# Supplementary material for: Benchmarking vibrational spectra: 5000 accurate eigenstates of acetonitrile using tree tensor network states
Source: arXiv:2504.05382 ancillary file (2025-04-14)
Supplement: Supplementary file 1 [file SI.pdf]

# Supporting information for: “Benchmarking Vibrational Spectra: 5000 Accurate Eigenstates of Acetonitrile Using Tree Tensor Network States”

Henrik R. Larsson

Department of Chemistry and Biochemistry, University of California, Merced, CA 95343, USA

## S1. COMPUTATIONAL DETAILS

We use the tree shown in Fig. 1 of the main paper for the final TTNS computations, which uses mode combination of the degenerate mode. Note that during the initial course of the optimizations for the CSC states, we used the tree from Ref. [1], which, compared to the tree from Fig. 1, does not make use of mode combination. The trees were converted to a tree with mode combination to avoid possible subtle numerical issues due to degeneracies. The mode combination fully treats the degenerate modes on equal footing. The mode numbering in Fig. 1 of the main paper follows Table 3 in Ref. [2]: The first four modes are non-degenerate and are ordered by decreasing frequency. This is followed by pairs of degenerate modes ( $\{5, 6\}$ ,  $\{7, 8\}$ , etc.), also ordered by decreasing frequency.

### A. DMRG simulation parameters

The DMRG sweeps abort once a relative energy convergence tolerance of  $10^{-10}$  is reached. The DMRG eigenvalue problem is solved using Davidson’s algorithm,<sup>3</sup> as implemented in PySCF.<sup>4</sup> We use eigenvalue convergence tolerances that are gradually decreased after some sweeps from  $10^{-7}$  to  $10^{-12}$ . In the state-shifted Hamiltonian,

$$\hat{H} + \sum_I (E_I + S) |I\rangle \langle I|, \quad (\text{S1})$$

we set  $S = 8499 \text{ cm}^{-1}$ . We adapt the bond dimension  $D$  for each tensor using a singular value decomposition (SVD) threshold of  $\epsilon = 10^{-3}$ , which is gradually decreased to  $\epsilon = 10^{-6}$  after some sweeps. To avoid oscillations of the bond dimensions during the sweeps, after the bond dimension adaption we increase  $D$  to  $D+2$ .<sup>1</sup> For the CSC PES, the initial guess is based on the previously converged state. Random noise is added in the first sweeps with magnitudes that start at  $10^{-2}$  and are decreased to  $10^{-6}$  during the course of the optimization, before the noise is turned off. For the USC (AC) PES, the initial guess is based on the converged CSC (USC) states.  $S$  is then set to  $99 \text{ cm}^{-1}$ , noise is turned off and the eigenvalue convergence tolerances and SVD thresholds  $\epsilon$  are set to tighter values in the beginning of the optimization. The computations make use of a code with hybrid distributed/shared-memory parallelization. We used one to four nodes with 36 to 64 cores.

Note that our algorithm does not necessarily return eigenstates ordered by energy. To ensure that we computed the lowest 1000/5000 states, we computed 100 to 200 additional states (so up to  $\sim 5200$  in total) using various initial guesses based on randomized TTNSs, symmetry-projected states, and

highly-excited variational self-consistent field states. While the chance is low that we missed some states just below the 5000 mark, we cannot fully rule out this possibility.

### B. States from the generalized eigenvalue problem

Solving the generalized eigenvalue problem in the basis of TTNSs,  $\{|I\rangle\}_I$  leads to eigenstates that are linear combinations of TTNSs. To fit them to a final TTNS for each eigenstate, we use all states  $|I\rangle$  whose eigenvalue coefficients is larger than  $10^{-2}$  and fit them with an adaptive bond dimension using an SVD threshold of  $\epsilon = 10^{-7}$ . The differences between the energies from the generalized eigenvalue problem and that of the fitted states was less than  $0.0008 \text{ cm}^{-1}$ , throughout. Note that the fitted states were just used for computing the entanglement entropy, the DVR error (see Section S2 A for a justification), for symmetry assignments, and for plotting selected states.

## S2. SYMMETRY ASSIGNMENT

We assign the symmetry of each state by applying the character projection operator<sup>5,6</sup>

$$\hat{P}^{(\mu)} = \frac{d_\mu}{h} \sum_R \chi^{(\mu)}(R)^* \hat{O}_R, \quad (\text{S2})$$

where  $R$  sums over all possible symmetry operations of irrep  $\mu$  with dimension  $d_\mu$ .  $\chi$  is the character and  $\hat{O}_R$  the operator for the symmetry transformation, as given in Ref. [7]. Applying  $\hat{P}^{(\mu)}$  onto a TTNS  $|I\rangle$  leads to a linear combination of TTNSs. We fit this linear combination and then compute the norm of  $\hat{P}^{(\mu)}|I\rangle$  to assign the irrep.

### A. Error estimate

Assuming that the individual errors are independent, we estimate the total error as

$$\Delta E_{\text{est}} = \sqrt{\Delta E_{\text{DVR}}^2 + \max(\Delta E_{D,1}, \Delta E_{D,2})^2 + \Delta E_{\text{deg}}^2}, \quad (\text{S3})$$

where  $\Delta E_{\text{DVR}}$  is the error of the DVR basis (see main text),  $\Delta E_{D,i}$  the error due to finite bond dimension (estimated using two individual procedures that lead to very similar errors; see main text and below), and  $\Delta E_{\text{deg}}$  the degeneracy error of states in  $E$  irreps. Note that  $\Delta E_{\text{deg}}$  is indirectly included in

the other error estimates and thus not an independent error. However,  $\Delta E_{\text{deg}}$  has a negligible influence on the total error (see Figs. S1 to S3), so we chose to include it in Eq. (S3).  $\Delta E_{\text{DVR}}$  was calculated from the linearly-combined states of the generalized eigenvalue problem in Section S1 B. For the CSC PES we also computed it by solving a generalized eigenvalue problem in the basis of TTNSs converted to the fully variational Harmonic oscillator basis, which led to a similar value of  $\Delta E_{\text{DVR}}$ .

### B. Bond dimension error estimates

Using a linear regression of the energy  $E$  as a function of  $1/D_{\text{max}}$  and two data points,  $E_1$  and  $E_2$  with  $E_1 < E_2$ ,<sup>8</sup> the lower bound is given as

$$E_{\text{low}} = E_1 - \frac{E_2 - E_1}{1/D_2 - 1/D_1} \frac{1}{D_1}, \quad (\text{S4})$$

which results in the error estimate

$$\Delta E_D = E_1 - E_{\text{low}} = \frac{E_2 - E_1}{1/D_2 - 1/D_1} \frac{1}{D_1}. \quad (\text{S5})$$

Defining  $x = \frac{D_2}{D_1}$ , Eq. (S5) leads to

$$\Delta E_D = (E_2 - E_1) \frac{x}{1 - x}. \quad (\text{S6})$$

Hence,  $\Delta E_D$  simply is a scaled energy difference. In this work we use  $x = 80\%$ , which leads to  $\Delta E_D = 4(E_2 - E_1)$ . If the estimates are close to the DMRG relative convergence tolerance of  $10^{-10}$ , the energy of the TTNS with  $D_2$  can be smaller than that of the original TTNS with  $D_1$ . In those few cases we used  $x = 50\%$ .

### C. Parameters for first procedure

For our first procedure, which is based on DMRG optimization, for each state  $|I\rangle$  we first perform a re-optimization with an SVD threshold of  $\epsilon = 10^{-13}$  (without an additional offset) but a maximum allowed bond dimension value that corresponds to  $D_{\text{max}}$  of  $|I\rangle$ . This allows all bonds with  $D$  below  $D_{\text{max}}$  to grow until  $D_{\text{max}}$  to get the best energy estimate  $E_1$ . After this optimization,  $D_{\text{max}}$  is reduced to  $0.8D_{\text{max}}$  (rounded to integer values) to get the second-best estimate  $E_2$ , and thereafter, for additional tests (see above), to  $0.5D_{\text{max}}$ . The energies  $E_1$  and  $E_2$  together with the respective  $D_{\text{max}}$  values are used to evaluate the error  $\Delta E_{D,1}$  in Eq. (S6). During these DMRG optimizations, all other states  $|J\rangle$  with  $J \neq I$  are shifted using Eq. (S1). Note that we shift the states obtained from the final DMRG optimization without re-optimization or truncation.

### D. Parameters for second procedure

For our second estimate  $\Delta E_{D,2}$ , we first compress each state  $|I\rangle$  using singular value decomposition, reducing  $D_{\text{max}}$

to  $0.8D_{\text{max}}$ , and, in another step to  $0.5D_{\text{max}}$ . For these sets of compressed states, we solve the generalized eigenvalue problem and then use Eq. (S6) to get  $\Delta E_{D,2}$ . We only used the  $0.5D_{\text{max}}$  data in rare cases where the energy does not decrease upon compression (see discussion below Eq. (S6)).

## S3. ADDITIONAL DATA

Table S1 compiles selected literature on computations of  $\text{CH}_3\text{CN}$  that are based on the PES from Ref. [2]. The maximum bond dimensions of the eigenstates are shown in Fig. S4. Fig. S5 shows that the error of the energies from Ref. [9] is determined by the finite Harmonic oscillator basis. Our TTNS computation with the same basis gives the same error, showing that the basis-set error is dominating.

Tabs. S2 to S4 lists all reported states together with additional data and the difference of the excitation energies to literature values. We compare excitation energies and thus assume that the zero-point energy has been computed accurately throughout, which is a reasonable assumption, as the ground state is simple. Note further that we report an error *estimate* that is automatically calculated for each state. This leads to some small inconsistencies. For example, states 11/12 in Table S2 are degenerate, but we show the energy of state 11 with a smaller error than that of state 12, which has an additional rounding error for the last digit.

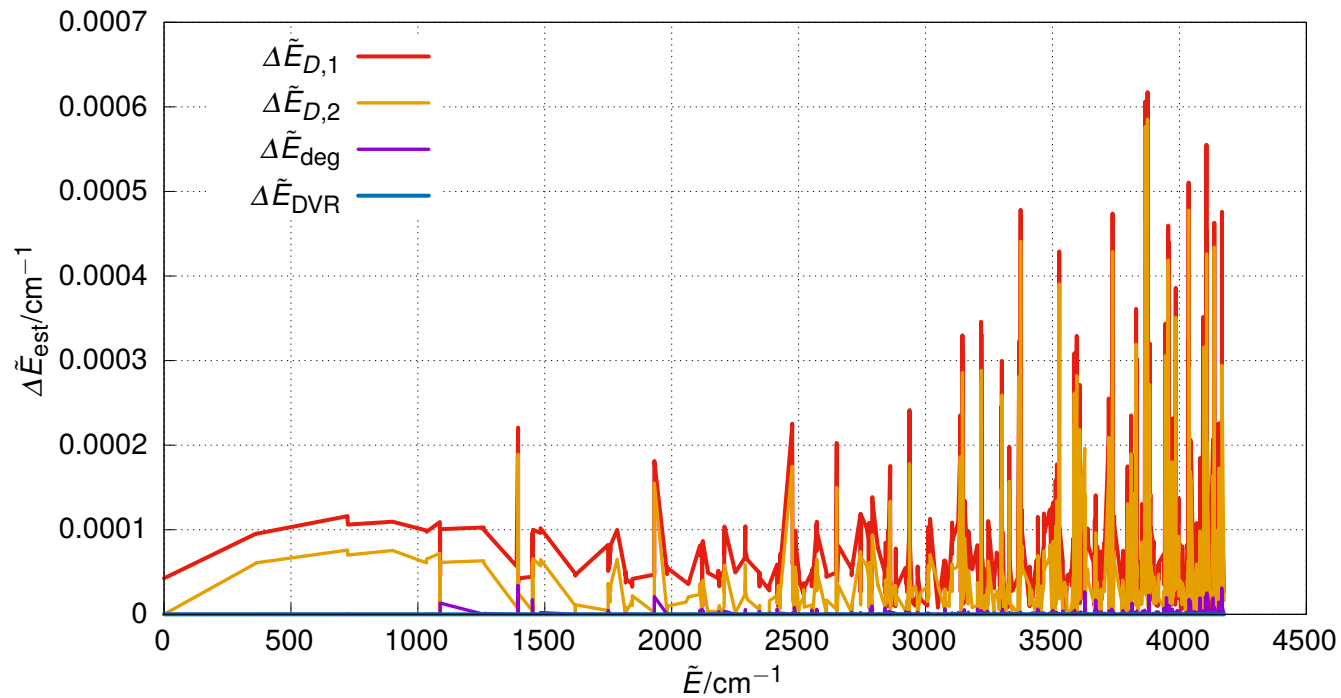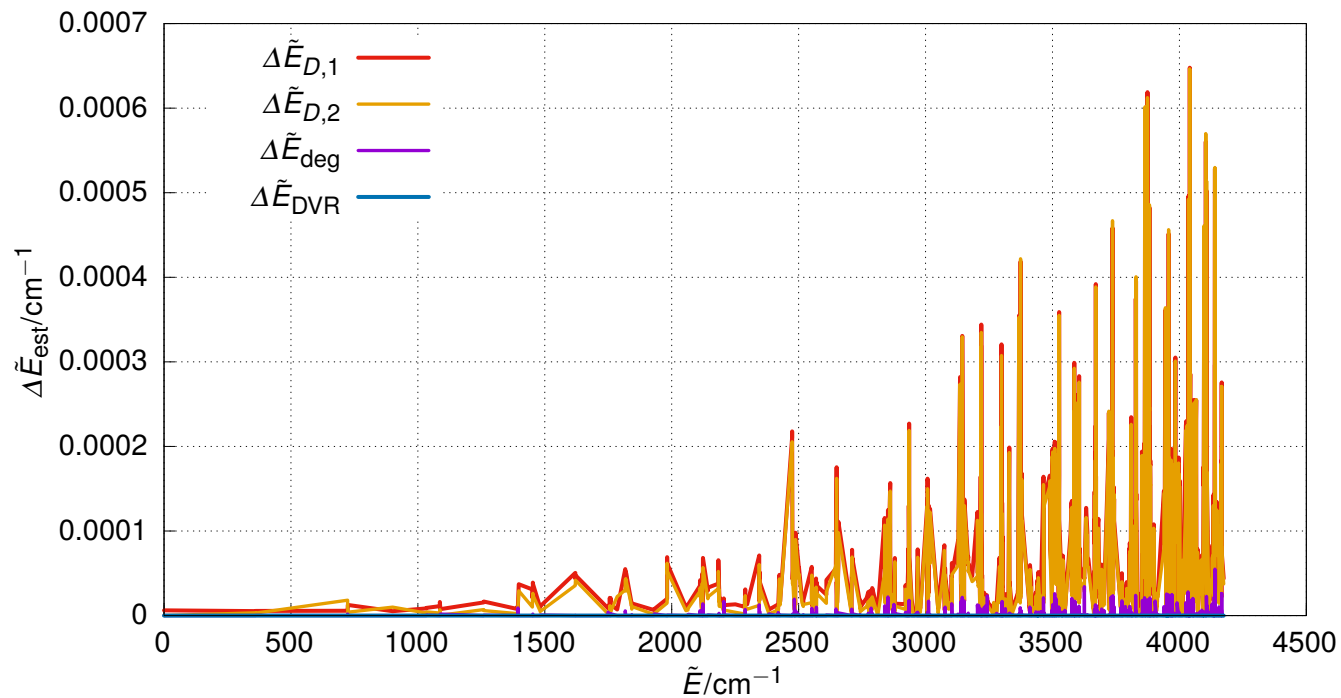

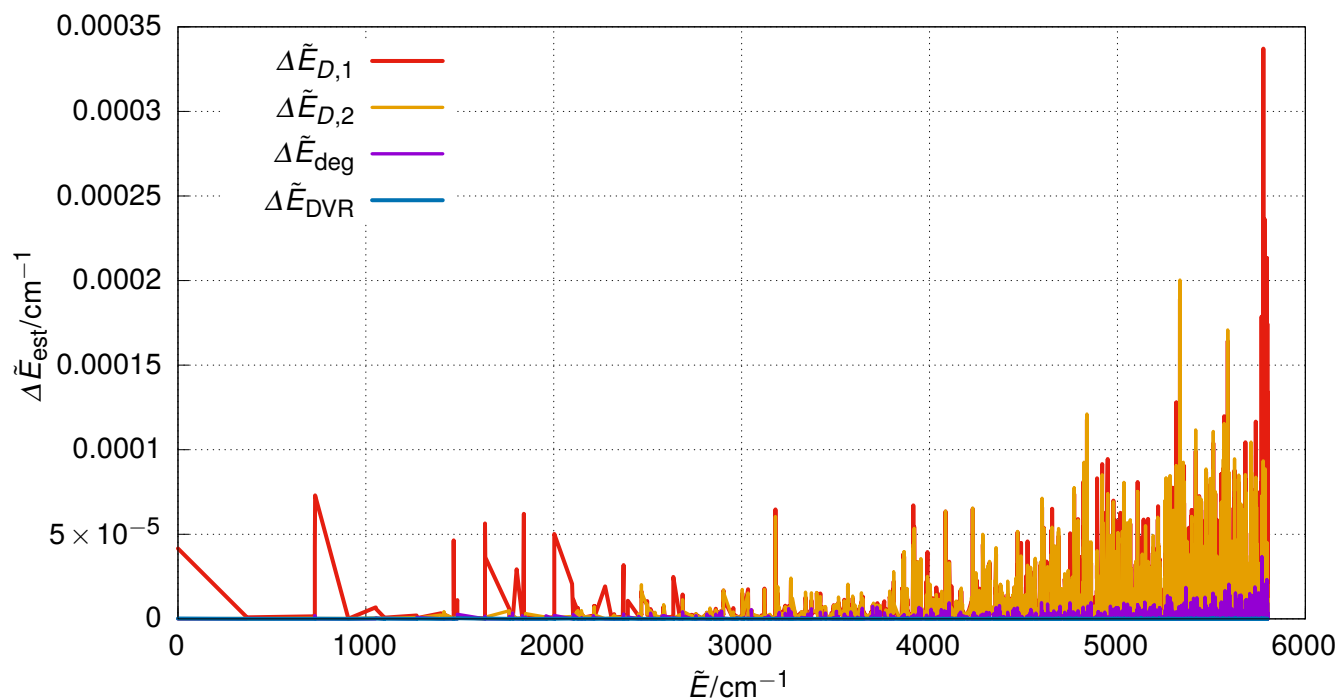

FIG. S3. Same as Fig. S1 but for the CSC PES. Note the different ordinate range.

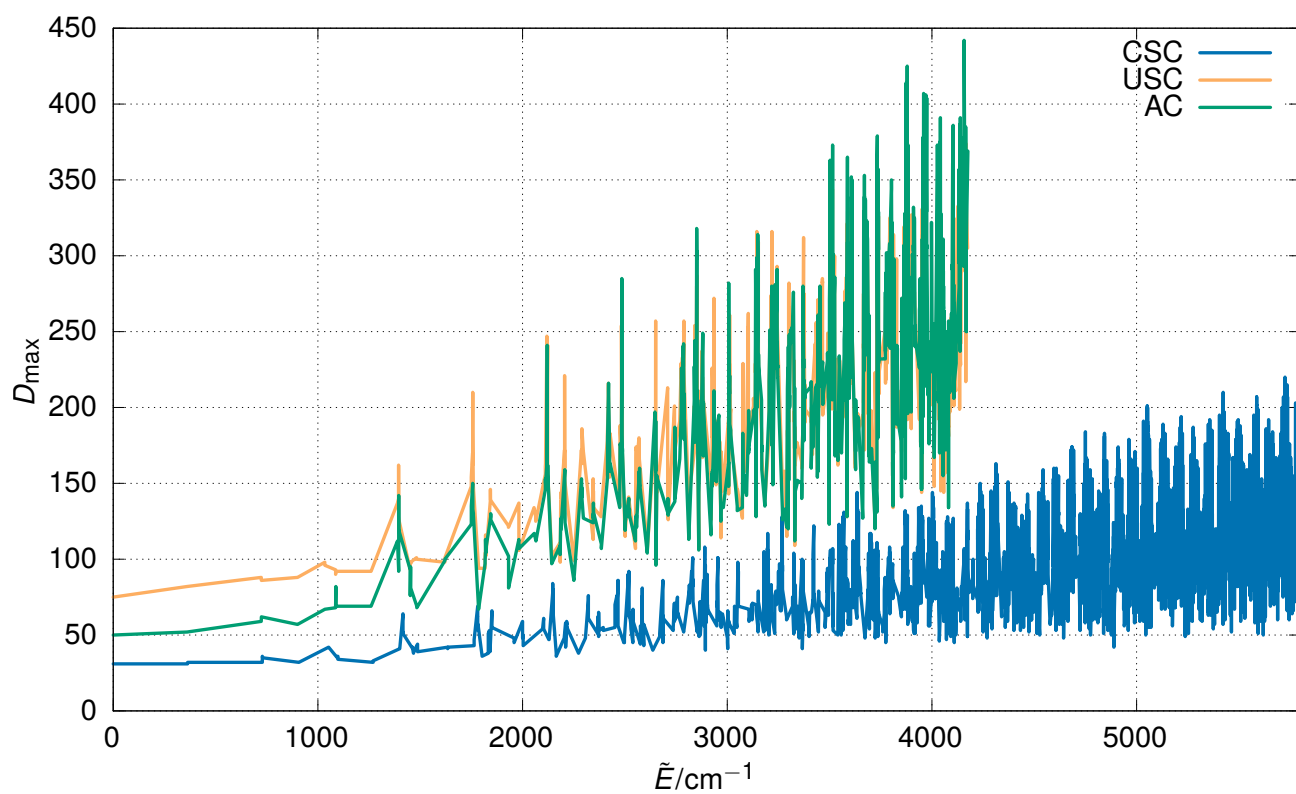

FIG. S4. Final bond dimensions of each state for the three used PESs.

TABLE S1. Selected literature results for eigenstate computations of acetonitrile based on the PES from Ref. [2]. Note that this only lists the number of states and not the estimated accuracy, which is difficult to assess, as different PESs and different error estimates are used.

| Reference | Year | Reference of PES          | number of states computed |
|-----------|------|---------------------------|---------------------------|
| 2         | 2005 | 2                         | 164                       |
| 10        | 2011 | 11                        | 40                        |
| 11        | 2011 | 11 (AC version)           | 201                       |
| 12        | 2014 | 11                        | 70                        |
| 13        | 2015 | 13                        | 10,000                    |
| 14        | 2015 | 11                        | 84                        |
| 15        | 2016 | 11                        | 50                        |
| 16        | 2016 | 11                        | 120                       |
| 17        | 2016 | 11                        | 60                        |
| 18        | 2016 | 11                        | 32                        |
| 19        | 2016 | 11                        | 84                        |
| 20        | 2016 | 11                        | 69                        |
| 21        | 2017 | 11                        | 120                       |
| 22        | 2017 | 22                        | 33                        |
| 9         | 2017 | 11                        | 239                       |
| 23        | 2017 | 11                        | 69                        |
| 24        | 2019 | 11                        | 15                        |
| 1         | 2019 | 11                        | 83                        |
| 25        | 2019 | 11                        | 20                        |
| 26        | 2019 | 11                        | 84                        |
| 27        | 2020 | 11                        | 69                        |
| 28        | 2021 | 11                        | 70                        |
| 29        | 2021 | 11                        | 51                        |
| 30        | 2021 | 30 (2 versions: USC, CSC) | 1000                      |
| 31        | 2023 | 11                        | 84                        |
| 32        | 2023 | 11                        | 51                        |
| 33        | 2023 | 11                        | 70                        |
| 34        | 2024 | 11                        | 239                       |
| 35        | 2024 | 11                        | 239                       |
| 36        | 2024 | 11                        | 84                        |
| this work | 2025 | 11                        | 1000                      |
| this work | 2025 | 30                        | 5000                      |

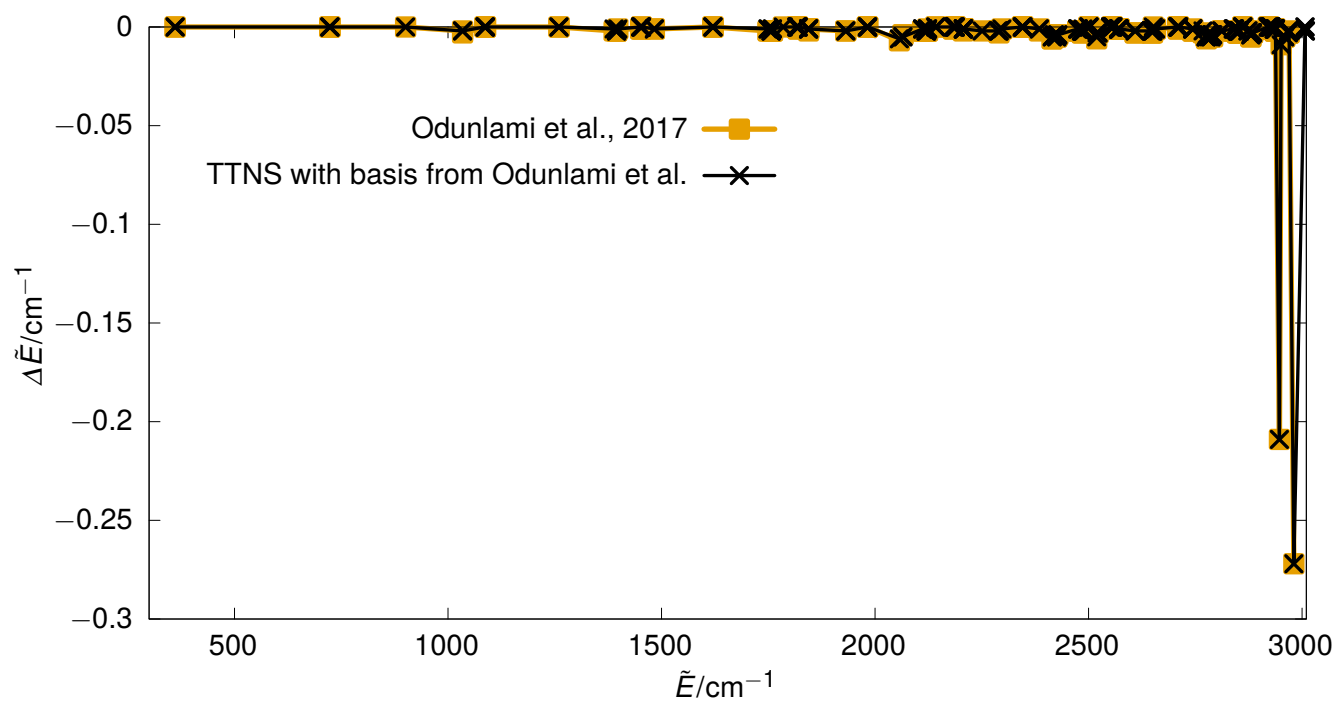

FIG. S5. Comparison of the literature error of Ref. [9] with TTNS computations using the same basis. The reference energies are our TTNS computations with the large basis (42 DVR functions in each mode).

## REFERENCES

- <sup>1</sup>H. R. Larsson, J. Chem. Phys. **151**, 204102 (2019).
- <sup>2</sup>D. Begue, P. Carbonniere, and C. Pouchan, J. Phys. Chem. A **109**, 4611 (2005).
- <sup>3</sup>E. R. Davidson, J. Comput. Phys. **17**, 87 (1975).
- <sup>4</sup>Q. Sun, T. C. Berkelbach, N. S. Blunt, G. H. Booth, S. Guo, Z. Li, J. Liu, J. D. McClain, E. R. Sayfutyarova, S. Sharma, S. Wouters, and G. K.-L. Chan, WIREs Comput Mol Sci **8**, 1340 (2018).
- <sup>5</sup>P. R. Bunker and P. Jensen, *Molecular Symmetry and Spectroscopy* (NRC Research Press, 2006).
- <sup>6</sup>T. Mathea and G. Rauhut, J. Chem. Phys. **152**, 194112 (2020).
- <sup>7</sup>L. Henry and G. Amat, J. Mol. Spectrosc. **5**, 319 (1961).
- <sup>8</sup>L. Tagliacozzo, G. Evenbly, and G. Vidal, Phys. Rev. B **80**, 235127 (2009).
- <sup>9</sup>M. Odunlami, V. Le Bris, D. Bégué, I. Baraille, and O. Coulaud, J. Chem. Phys. **146**, 214108 (2017).
- <sup>10</sup>G. Avila and T. Carrington, in *Quantum Dynamic Imaging*, edited by A. D. Bandrauk and M. Ivanov (Springer New York, New York, NY, 2011) pp. 1–12.
- <sup>11</sup>G. Avila and T. Carrington, J. Chem. Phys. **134**, 054126 (2011).
- <sup>12</sup>A. Leclerc and T. Carrington, J. Chem. Phys. **140**, 174111 (2014).
- <sup>13</sup>T. Halverson and B. Poirier, Chem. Phys. Lett. **624**, 37 (2015).
- <sup>14</sup>P. S. Thomas and T. Carrington, J. Phys. Chem. A **119**, 13074 (2015).
- <sup>15</sup>J. Brown and T. Carrington, J. Chem. Phys. **145**, 144104 (2016).
- <sup>16</sup>R. Garnier, M. Odunlami, V. Le Bris, D. Bégué, I. Baraille, and O. Coulaud, J. Chem. Phys. **144**, 204123 (2016).
- <sup>17</sup>A. Leclerc and T. Carrington, Chem. Phys. Lett. **644**, 183 (2016).
- <sup>18</sup>A. Leclerc, P. S. Thomas, and T. Carrington, Mol. Phys. , 1 (2016).
- <sup>19</sup>M. Rakhuba and I. Oseledets, J. Chem. Phys. **145**, 124101 (2016).
- <sup>20</sup>R. Wodraszka and T. Carrington, J. Chem. Phys. **145**, 044110 (2016).
- <sup>21</sup>G. Avila and T. Carrington, Chem. Phys. **482**, 3 (2017).
- <sup>22</sup>A. Baiardi, C. J. Stein, V. Barone, and M. Reiher, J. Chem. Theory Comput. **13**, 3764 (2017).
- <sup>23</sup>R. Wodraszka and T. Carrington, J. Chem. Phys. **146**, 194105 (2017).
- <sup>24</sup>R. Garnier, Comput. Phys. Commun. **234**, 263 (2019).
- <sup>25</sup>E. Lesko, M. Ardiansyah, and K. R. Brorsen, J. Chem. Phys. **151**, 164103 (2019).
- <sup>26</sup>M. Rakhuba, A. Novikov, and I. Oseledets, J. Comput. Phys. **396**, 718 (2019).
- <sup>27</sup>R. Wodraszka and T. Carrington, J. Chem. Phys. **152**, 164117 (2020).
- <sup>28</sup>J. H. Fetherolf and T. C. Berkelbach, J. Chem. Phys. **154**, 074104 (2021).
- <sup>29</sup>S. D. Kallullathil and T. Carrington, J. Chem. Phys. **155**, 234105 (2021).
- <sup>30</sup>J. Sarka and B. Poirier, J. Chem. Theory Comput. **17**, 7732 (2021).
- <sup>31</sup>S. D. Kallullathil and T. Carrington, Jr., J. Chem. Phys. **158**, 214102 (2023).
- <sup>32</sup>J. Simmons and T. Carrington, J. Chem. Phys. **158**, 144115 (2023).
- <sup>33</sup>H. K. Tran and T. C. Berkelbach, J. Chem. Phys. **159**, 194101 (2023).
- <sup>34</sup>H. Hoppe and U. Manthe, J. Chem. Phys. **160**, 034104 (2024).
- <sup>35</sup>M. Rey and T. Carrington, Jr., J. Chem. Phys. **161**, 044102 (2024).
- <sup>36</sup>Q. Zhang, R.-S. Wang, and L. Wang, J. Chem. Phys. **161**, 024103 (2024).

TABLE S2: Eigenstate data for the Avila/Carrington (AC) PES variant. Shown are the state number, the assigned irrep, the max. bond dimension, the entanglement entropy, the excitation energy (zero-point energy for state 0) and the differences of excitation energies,  $\Delta$ , from selected literature values to ours. For our energies, the digit in parentheses denotes our error estimate. Note that all literature energies are reported with only up to 3 places after the decimal point. Further, note that our error estimates of the excitation energies do not include that of the zero-point energy, which is negligible.

| State | $\Gamma_{C_{3v}}$ | $D_{\max}$ | $S_{vN}$ | $\tilde{E}/\text{cm}^{-1}$ | $\Delta\text{Ref. [11]}$ | $\Delta\text{Ref. [9]}$ | $\Delta\text{Ref. [34]}$ | $\Delta\text{Ref. [35]}$ | $\Delta\text{Ref. [1]}$ |
|-------|-------------------|------------|----------|----------------------------|--------------------------|-------------------------|--------------------------|--------------------------|-------------------------|
| 0     | $A_1$             | 50         | 0.053    | 9837.40670(4)              |                          |                         |                          |                          |                         |
| 1     | $E$               | 52         | 0.057    | 360.99009(9)               | -0.001                   | 0.000                   | -0.001                   | 0.000                    | -0.000                  |
| 2     | $E$               | 52         | 0.057    | 360.99009(9)               | -0.001                   | 0.000                   | -0.001                   | 0.000                    | -0.000                  |
| 3     | $E$               | 59         | 0.064    | 723.1793(1)                | -0.002                   | 0.000                   | -0.002                   | 0.000                    | -0.000                  |
| 4     | $E$               | 59         | 0.064    | 723.1793(1)                | -0.002                   | 0.000                   | -0.002                   | 0.000                    | -0.000                  |
| 5     | $A_1$             | 62         | 0.15     | 723.8254(1)                | -0.002                   | 0.000                   | -0.002                   | 0.000                    | -0.000                  |
| 6     | $A_1$             | 57         | 0.17     | 900.6572(1)                | -0.005                   | 0.000                   | -0.012                   | -0.001                   | -0.002                  |
| 7     | $E$               | 67         | 0.093    | 1034.12350(9)              | -0.003                   | -0.002                  | -0.006                   | -0.001                   | -0.000                  |
| 8     | $E$               | 67         | 0.094    | 1034.12350(9)              | -0.003                   | -0.003                  | -0.006                   | -0.001                   | -0.000                  |
| 9     | $A_1$             | 68         | 0.072    | 1086.5518(1)               | -0.002                   | -0.000                  | -0.002                   | -0.000                   | -0.000                  |
| 10    | $A_2$             | 70         | 0.072    | 1086.55209(9)              | -0.002                   | 0.000                   | -0.002                   | -0.001                   | -0.000                  |
| 11    | $E$               | 82         | 0.22     | 1087.77414(4)              | -0.002                   | 0.000                   | -0.002                   | -0.001                   | 0.000                   |
| 12    | $E$               | 69         | 0.22     | 1087.7742(1)               | -0.002                   | 0.000                   | -0.002                   | -0.001                   | -0.000                  |
| 13    | $E$               | 69         | 0.26     | 1259.8069(1)               | -0.015                   | -0.000                  | -0.015                   | -0.001                   | -0.002                  |
| 14    | $E$               | 69         | 0.26     | 1259.8069(1)               | -0.015                   | -0.000                  | -0.015                   | -0.001                   | -0.002                  |
| 15    | $A_1$             | 112        | 3.9      | 1388.96724(5)              | -0.006                   | -0.002                  | -0.015                   | -0.001                   | -0.000                  |
| 16    | $E$               | 92         | 2.1      | 1394.6792(2)               | -0.010                   | -0.002                  | -0.008                   | -0.001                   | -0.000                  |
| 17    | $E$               | 142        | 2.1      | 1394.6792(1)               | -0.010                   | -0.002                  | -0.008                   | -0.001                   | -0.000                  |
| 18    | $A_2$             | 120        | 2.1      | 1394.89789(3)              | -0.009                   | -0.002                  | -0.009                   | -0.001                   | -0.000                  |
| 19    | $A_1$             | 118        | 4.2      | 1397.68001(4)              | -0.007                   | -0.001                  | -0.013                   | -0.001                   | -0.000                  |
| 20    | $E$               | 93         | 0.081    | 1451.09246(4)              | -0.009                   | -0.001                  | -0.003                   | -0.001                   | -0.000                  |
| 21    | $E$               | 76         | 0.081    | 1451.09248(9)              | -0.009                   | -0.001                  | -0.003                   | -0.001                   | -0.000                  |
| 22    | $E$               | 93         | 0.31     | 1452.81789(4)              | -0.009                   | -0.000                  | -0.003                   | -0.001                   | -0.000                  |
| 23    | $E$               | 95         | 0.31     | 1452.81789(4)              | -0.009                   | -0.000                  | -0.003                   | -0.001                   | -0.000                  |
| 24    | $A_1$             | 81         | 0.37     | 1453.3935(1)               | -0.010                   | -0.001                  | -0.003                   | -0.001                   | -0.000                  |
| 25    | $E$               | 69         | 0.14     | 1483.21943(9)              | -0.010                   | -0.001                  | -0.008                   | -0.001                   | -0.000                  |
| 26    | $E$               | 68         | 0.14     | 1483.2194(1)               | -0.010                   | -0.001                  | -0.008                   | -0.001                   | -0.000                  |
| 27    | $E$               | 99         | 0.35     | 1620.19580(4)              | -0.026                   | -0.000                  | -0.018                   | -0.001                   | -0.003                  |
| 28    | $E$               | 100        | 0.35     | 1620.19580(4)              | -0.026                   | -0.000                  | -0.018                   | -0.001                   | -0.003                  |
| 29    | $A_1$             | 100        | 0.57     | 1620.73965(4)              | -0.027                   | -0.000                  | -0.017                   | -0.001                   | -0.004                  |
| 30    | $E$               | 123        | 3.8      | 1749.51845(8)              | -0.012                   | -0.002                  | -0.019                   | -0.002                   | -0.000                  |
| 31    | $E$               | 135        | 3.8      | 1749.51846(5)              | -0.012                   | -0.002                  | -0.019                   | -0.002                   | -0.000                  |
| 32    | $A_1$             | 150        | 2.2      | 1756.41218(6)              | -0.014                   | -0.002                  | -0.009                   | -0.002                   | -0.000                  |
| 33    | $A_2$             | 149        | 2.2      | 1756.41220(6)              | -0.014                   | -0.002                  | -0.010                   | -0.002                   | -0.000                  |
| 34    | $E$               | 136        | 1.5      | 1757.11852(6)              | -0.014                   | -0.002                  | -0.009                   | -0.001                   | -0.000                  |
| 35    | $E$               | 133        | 1.5      | 1757.11852(7)              | -0.014                   | -0.002                  | -0.009                   | -0.001                   | -0.000                  |
| 36    | $E$               | 130        | 4.2      | 1759.76002(7)              | -0.012                   | -0.002                  | -0.016                   | -0.001                   | -0.000                  |
| 37    | $E$               | 129        | 4.2      | 1759.76002(8)              | -0.012                   | -0.002                  | -0.016                   | -0.001                   | -0.000                  |
| 38    | $A_1$             | 67         | 0.41     | 1785.0980(1)               | -0.109                   | -0.000                  | -0.078                   | -0.006                   | -0.079                  |
| 39    | $E$               | 97         | 0.091    | 1816.78583(5)              | -0.013                   | -0.000                  | -0.003                   | -0.001                   | -0.000                  |
| 40    | $E$               | 99         | 0.091    | 1816.78583(4)              | -0.013                   | -0.000                  | -0.003                   | -0.001                   | -0.000                  |
| 41    | $A_1$             | 105        | 0.39     | 1818.93759(5)              | -0.014                   | -0.000                  | -0.004                   | -0.001                   | -0.000                  |
| 42    | $A_2$             | 113        | 0.39     | 1818.93877(3)              | -0.013                   | -0.000                  | -0.004                   | -0.001                   | -0.000                  |
| 43    | $E$               | 104        | 0.5      | 1820.01540(4)              | -0.016                   | -0.001                  | -0.005                   | -0.002                   | -0.000                  |
| 44    | $E$               | 106        | 0.5      | 1820.01540(4)              | -0.016                   | -0.001                  | -0.005                   | -0.002                   | -0.000                  |
| 45    | $A_2$             | 128        | 2.2      | 1844.24446(3)              | -0.014                   | -0.001                  | -0.010                   | -0.002                   | -0.000                  |
| 46    | $E$               | 129        | 2.1      | 1844.31646(3)              | -0.014                   | -0.001                  | -0.010                   | -0.002                   | -0.000                  |
| 47    | $E$               | 130        | 2.1      | 1844.31646(3)              | -0.014                   | -0.002                  | -0.010                   | -0.002                   | -0.000                  |
| 48    | $A_1$             | 126        | 2.2      | 1844.67609(4)              | -0.014                   | -0.001                  | -0.010                   | -0.001                   | -0.000                  |
| 49    | $E$               | 102        | 0.26     | 1931.51133(4)              | -0.036                   | -0.002                  | -0.028                   | -0.003                   | -0.003                  |
| 50    | $E$               | 81         | 0.26     | 1931.5114(1)               | -0.036                   | -0.002                  | -0.028                   | -0.003                   | -0.003                  |
| 51    | $A_1$             | 113        | 0.43     | 1981.81121(4)              | -0.038                   | 0.000                   | -0.020                   | -0.002                   | -0.004                  |

Continued on next page.



TABLE S2 – States on Avila/Carrington AC PES; continued from previous page.

| State | $\Gamma_{C_{3v}}$ | $D_{\max}$ | $S_{vN}$ | $\tilde{E}/\text{cm}^{-1}$ | $\Delta\text{Ref. [11]}$ | $\Delta\text{Ref. [9]}$ | $\Delta\text{Ref. [34]}$ | $\Delta\text{Ref. [35]}$ | $\Delta\text{Ref. [1]}$ |
|-------|-------------------|------------|----------|----------------------------|--------------------------|-------------------------|--------------------------|--------------------------|-------------------------|
| 52    | $A_2$             | 111        | 0.43     | 1981.81162(5)              | -0.037                   | -0.000                  | -0.020                   | -0.001                   | -0.004                  |
| 53    | $E$               | 108        | 0.84     | 1982.81155(5)              | -0.045                   | -0.000                  | -0.021                   | -0.002                   | -0.006                  |
| 54    | $E$               | 107        | 0.84     | 1982.81155(5)              | -0.045                   | -0.000                  | -0.021                   | -0.002                   | -0.006                  |
| 55    | $A_1$             | 117        | 0.22     | 2057.04417(3)              | -0.024                   | -0.007                  | -0.047                   | -0.003                   | -0.000                  |
| 56    | $E$               | 112        | 0.18     | 2065.26457(3)              | -0.021                   | -0.004                  | -0.035                   | -0.002                   | -0.000                  |
| 57    | $E$               | 112        | 0.18     | 2065.26457(3)              | -0.021                   | -0.004                  | -0.035                   | -0.002                   | -0.000                  |
| 58    | $E$               | 146        | 3.8      | 2111.36331(8)              | -0.017                   | -0.002                  | -0.022                   | -0.002                   | -0.000                  |
| 59    | $E$               | 153        | 3.8      | 2111.36332(7)              | -0.017                   | -0.002                  | -0.023                   | -0.002                   | -0.000                  |
| 60    | $A_1$             | 150        | 3.9      | 2112.28046(7)              | -0.017                   | -0.002                  | -0.023                   | -0.002                   | -0.001                  |
| 61    | $E$               | 164        | 2.3      | 2119.30706(7)              | -0.020                   | -0.002                  | -0.011                   | -0.002                   | -0.000                  |
| 62    | $E$               | 179        | 2.3      | 2119.30706(4)              | -0.020                   | -0.002                  | -0.011                   | -0.002                   | -0.000                  |
| 63    | $E$               | 241        | 2.3      | 2120.52057(3)              | -0.020                   | -0.002                  | -0.011                   | -0.001                   | -0.000                  |
| 64    | $E$               | 183        | 2.3      | 2120.52057(3)              | -0.020                   | -0.002                  | -0.011                   | -0.001                   | -0.000                  |
| 65    | $A_2$             | 146        | 2.3      | 2120.88878(8)              | -0.021                   | -0.002                  | -0.011                   | -0.002                   | -0.000                  |
| 66    | $E$               | 153        | 4.3      | 2122.81601(8)              | -0.018                   | -0.002                  | -0.018                   | -0.002                   | -0.000                  |
| 67    | $E$               | 162        | 4.3      | 2122.81602(6)              | -0.018                   | -0.002                  | -0.019                   | -0.002                   | -0.000                  |
| 68    | $A_1$             | 156        | 4.4      | 2123.28164(8)              | -0.019                   | -0.001                  | -0.018                   | -0.001                   | -0.001                  |
| 69    | $E$               | 97         | 0.58     | 2142.34823(5)              | -0.266                   | 0.000                   | -0.079                   | -0.007                   | -0.096                  |
| 70    | $E$               | 97         | 0.58     | 2142.34823(4)              | -0.266                   | 0.000                   | -0.079                   | -0.007                   | -0.096                  |
| 71    | $A_1$             | 109        | 0.1      | 2183.61730(4)              | -0.018                   | -0.001                  | -0.004                   | -0.002                   | -0.000                  |
| 72    | $A_2$             | 103        | 0.1      | 2183.61730(5)              | -0.018                   | -0.001                  | -0.004                   | -0.002                   | -0.000                  |
| 73    | $E$               | 124        | 0.47     | 2186.11660(3)              | -0.021                   | -0.000                  | -0.005                   | -0.001                   | -0.000                  |
| 74    | $E$               | 119        | 0.47     | 2186.11660(4)              | -0.021                   | -0.000                  | -0.005                   | -0.001                   | -0.000                  |
| 75    | $E$               | 127        | 0.64     | 2187.61783(3)              | -0.024                   | -0.000                  | -0.006                   | -0.001                   | -0.001                  |
| 76    | $E$               | 127        | 0.64     | 2187.61783(3)              | -0.024                   | -0.000                  | -0.006                   | -0.001                   | -0.001                  |
| 77    | $A_1$             | 121        | 0.69     | 2188.11851(4)              | -0.025                   | -0.000                  | -0.006                   | -0.001                   | -0.001                  |
| 78    | $A_1$             | 159        | 2.2      | 2206.60723(5)              | -0.019                   | -0.001                  | -0.011                   | -0.002                   | -0.000                  |
| 79    | $A_2$             | 139        | 2.2      | 2206.61448(9)              | -0.019                   | -0.002                  | -0.011                   | -0.002                   | -0.001                  |
| 80    | $E$               | 138        | 2.2      | 2206.75735(7)              | -0.019                   | -0.001                  | -0.011                   | -0.002                   | -0.000                  |
| 81    | $E$               | 134        | 2.2      | 2206.75735(8)              | -0.019                   | -0.001                  | -0.011                   | -0.002                   | -0.000                  |
| 82    | $E$               | 130        | 1.2      | 2207.54053(8)              | -0.018                   | -0.001                  | -0.010                   | -0.001                   | -0.000                  |
| 83    | $E$               | 124        | 1.1      | 2207.5405(1)               | -0.018                   | -0.001                  | -0.010                   | -0.001                   | -0.000                  |
| 84    | $A_1$             | 86         | 1.6      | 2250.70817(4)              | -0.038                   | -0.002                  | -0.155                   | -0.002                   |                         |
| 85    | $A_1$             | 153        | 4.2      | 2287.84401(6)              | -0.095                   | -0.002                  | -0.082                   | -0.003                   |                         |
| 86    | $E$               | 141        | 2.4      | 2290.1158(1)               | -0.106                   | -0.002                  | -0.033                   | -0.003                   |                         |
| 87    | $E$               | 147        | 2.4      | 2290.11580(8)              | -0.106                   | -0.002                  | -0.034                   | -0.003                   |                         |
| 88    | $A_2$             | 140        | 2.3      | 2290.27836(7)              | -0.106                   | -0.003                  | -0.033                   | -0.003                   |                         |
| 89    | $A_1$             | 127        | 3.4      | 2297.12893(6)              | -0.060                   | -0.001                  | -0.271                   | -0.005                   |                         |
| 90    | $E$               | 124        | 0.52     | 2344.64186(4)              | -0.106                   | -0.000                  | -0.023                   | -0.002                   |                         |
| 91    | $E$               | 130        | 0.52     | 2344.64186(4)              | -0.106                   | -0.000                  | -0.023                   | -0.002                   |                         |
| 92    | $E$               | 127        | 1.1      | 2346.00564(4)              | -0.121                   | -0.000                  | -0.028                   | -0.002                   |                         |
| 93    | $E$               | 137        | 1.1      | 2346.00564(3)              | -0.121                   | -0.000                  | -0.028                   | -0.002                   |                         |
| 94    | $A_1$             | 131        | 1.3      | 2346.46073(4)              | -0.127                   | -0.000                  | -0.031                   | -0.003                   |                         |
| 95    | $E$               | 110        | 0.26     | 2384.78934(2)              | -0.084                   | -0.001                  | -0.028                   | -0.004                   |                         |
| 96    | $E$               | 107        | 0.26     | 2384.78935(3)              | -0.084                   | -0.002                  | -0.028                   | -0.004                   |                         |
| 97    | $E$               | 154        | 3.3      | 2414.95730(5)              | -0.065                   | -0.006                  | -0.057                   | -0.004                   |                         |
| 98    | $E$               | 178        | 3.3      | 2414.95731(2)              | -0.065                   | -0.006                  | -0.057                   | -0.004                   |                         |
| 99    | $E$               | 216        | 4.0      | 2420.07836(3)              | -0.057                   | -0.005                  | -0.054                   | -0.004                   |                         |
| 100   | $E$               | 212        | 4.0      | 2420.07836(3)              | -0.057                   | -0.005                  | -0.054                   | -0.004                   |                         |
| 101   | $A_1$             | 171        | 2.3      | 2425.36855(4)              | -0.074                   | -0.005                  | -0.050                   | -0.003                   |                         |
| 102   | $A_2$             | 158        | 2.3      | 2425.40344(4)              | -0.075                   | -0.005                  | -0.050                   | -0.003                   |                         |
| 103   | $E$               | 158        | 4.3      | 2427.90577(7)              | -0.057                   | -0.004                  | -0.049                   | -0.003                   |                         |
| 104   | $E$               | 163        | 4.3      | 2427.90577(5)              | -0.057                   | -0.004                  | -0.050                   | -0.003                   |                         |
| 105   | $A_1$             | 134        | 3.8      | 2474.4681(2)               | -0.037                   | -0.002                  | -0.026                   | -0.002                   |                         |
| 106   | $A_2$             | 135        | 3.8      | 2474.4685(2)               | -0.037                   | -0.002                  | -0.027                   | -0.003                   |                         |
| 107   | $E$               | 172        | 3.9      | 2476.13517(6)              | -0.038                   | -0.002                  | -0.031                   | -0.002                   |                         |
| 108   | $E$               | 176        | 3.9      | 2476.13517(6)              | -0.038                   | -0.002                  | -0.031                   | -0.002                   |                         |
| 109   | $E$               | 173        | 2.3      | 2483.34870(8)              | -0.065                   | -0.002                  | -0.012                   | -0.002                   |                         |
| 110   | $E$               | 192        | 2.3      | 2483.34871(5)              | -0.065                   | -0.002                  | -0.012                   | -0.002                   |                         |

Continued on next page.

TABLE S2 – States on Avila/Carrington AC PES; continued from previous page.

| State | $\Gamma_{C_{3v}}$ | $D_{\max}$ | $S_{vN}$ | $\tilde{E}/\text{cm}^{-1}$ | $\Delta\text{Ref. [11]}$ | $\Delta\text{Ref. [9]}$ | $\Delta\text{Ref. [34]}$ | $\Delta\text{Ref. [35]}$ | $\Delta\text{Ref. [1]}$ |
|-------|-------------------|------------|----------|----------------------------|--------------------------|-------------------------|--------------------------|--------------------------|-------------------------|
| 111   | $A_1$             | 229        | 2.5      | 2485.02438(3)              | -0.067                   | -0.003                  | -0.016                   | -0.003                   |                         |
| 112   | $A_2$             | 285        | 2.5      | 2485.02520(3)              | -0.067                   | -0.003                  | -0.016                   | -0.003                   |                         |
| 113   | $E$               | 185        | 1.8      | 2485.80368(4)              | -0.067                   | -0.002                  | -0.017                   | -0.002                   |                         |
| 114   | $E$               | 182        | 1.9      | 2485.80369(5)              | -0.067                   | -0.002                  | -0.017                   | -0.002                   |                         |
| 115   | $A_1$             | 171        | 4.3      | 2486.90991(9)              | -0.048                   | -0.002                  | -0.022                   | -0.002                   |                         |
| 116   | $A_2$             | 173        | 4.3      | 2486.91045(9)              | -0.048                   | -0.002                  | -0.022                   | -0.003                   |                         |
| 117   | $E$               | 171        | 4.4      | 2487.73834(9)              | -0.053                   | -0.002                  | -0.026                   | -0.003                   |                         |
| 118   | $E$               | 173        | 4.4      | 2487.73834(8)              | -0.053                   | -0.002                  | -0.026                   | -0.003                   |                         |
| 119   | $E$               | 121        | 0.75     | 2500.89781(4)              | -0.366                   | -0.000                  | -0.094                   | -0.010                   |                         |
| 120   | $E$               | 119        | 0.75     | 2500.89781(5)              | -0.366                   | -0.000                  | -0.094                   | -0.010                   |                         |
| 121   | $A_1$             | 124        | 1.1      | 2501.28717(4)              | -0.399                   | 0.000                   | -0.122                   | -0.012                   |                         |
| 122   | $A_1$             | 140        | 2.3      | 2519.07539(2)              | -0.068                   | -0.006                  | -0.135                   | -0.004                   |                         |
| 123   | $A_2$             | 128        | 2.2      | 2519.76881(3)              | -0.065                   | -0.003                  | -0.120                   | -0.003                   |                         |
| 124   | $E$               | 133        | 2.2      | 2522.04763(2)              | -0.066                   | -0.003                  | -0.125                   | -0.003                   |                         |
| 125   | $E$               | 129        | 2.2      | 2522.04763(3)              | -0.066                   | -0.003                  | -0.125                   | -0.003                   |                         |
| 126   | $E$               | 112        | 0.12     | 2551.57241(4)              | -0.058                   | -0.001                  | -0.005                   | -0.003                   |                         |
| 127   | $E$               | 122        | 0.12     | 2551.57242(3)              | -0.058                   | -0.001                  | -0.005                   | -0.003                   |                         |
| 128   | $E$               | 127        | 0.56     | 2554.33468(5)              | -0.063                   | -0.000                  | -0.007                   | -0.002                   |                         |
| 129   | $E$               | 128        | 0.56     | 2554.33468(5)              | -0.063                   | -0.000                  | -0.007                   | -0.002                   |                         |
| 130   | $A_1$             | 127        | 0.78     | 2556.17659(5)              | -0.068                   | -0.000                  | -0.009                   | -0.002                   |                         |
| 131   | $A_2$             | 129        | 0.78     | 2556.17963(4)              | -0.068                   | -0.000                  | -0.009                   | -0.002                   |                         |
| 132   | $E$               | 121        | 0.88     | 2557.10040(5)              | -0.071                   | -0.001                  | -0.011                   | -0.003                   |                         |
| 133   | $E$               | 123        | 0.88     | 2557.10040(4)              | -0.071                   | -0.001                  | -0.011                   | -0.003                   |                         |
| 134   | $E$               | 158        | 2.2      | 2570.0867(1)               | -0.058                   | -0.001                  | -0.012                   | -0.002                   |                         |
| 135   | $E$               | 158        | 2.2      | 2570.0867(1)               | -0.058                   | -0.001                  | -0.012                   | -0.002                   |                         |
| 136   | $E$               | 151        | 2.3      | 2570.3936(1)               | -0.058                   | -0.001                  | -0.013                   | -0.002                   |                         |
| 137   | $E$               | 156        | 2.3      | 2570.39364(9)              | -0.058                   | -0.001                  | -0.013                   | -0.002                   |                         |
| 138   | $A_2$             | 148        | 2.4      | 2571.17174(9)              | -0.059                   | -0.001                  | -0.014                   | -0.002                   |                         |
| 139   | $E$               | 148        | 2.3      | 2571.5739(1)               | -0.059                   | -0.001                  | -0.014                   | -0.002                   |                         |
| 140   | $E$               | 160        | 2.3      | 2571.57390(7)              | -0.059                   | -0.001                  | -0.014                   | -0.002                   |                         |
| 141   | $A_1$             | 150        | 2.4      | 2572.01277(9)              | -0.059                   | -0.001                  | -0.014                   | -0.002                   |                         |
| 142   | $E$               | 104        | 1.6      | 2609.19437(5)              | -0.062                   | -0.003                  | -0.218                   | -0.003                   |                         |
| 143   | $E$               | 105        | 1.6      | 2609.19437(4)              | -0.062                   | -0.003                  | -0.219                   | -0.003                   |                         |
| 144   | $E$               | 197        | 4.5      | 2646.93648(4)              | -0.137                   | -0.003                  | -0.125                   | -0.005                   |                         |
| 145   | $E$               | 196        | 4.5      | 2646.93648(5)              | -0.137                   | -0.003                  | -0.125                   | -0.005                   |                         |
| 146   | $A_1$             | 158        | 2.6      | 2649.9412(2)               | -0.143                   | -0.003                  | -0.049                   | -0.005                   |                         |
| 147   | $A_2$             | 158        | 2.6      | 2649.9430(2)               | -0.143                   | -0.002                  | -0.048                   | -0.004                   |                         |
| 148   | $E$               | 190        | 1.8      | 2650.49993(4)              | -0.147                   | -0.002                  | -0.055                   | -0.005                   |                         |
| 149   | $E$               | 191        | 1.8      | 2650.49994(4)              | -0.147                   | -0.002                  | -0.056                   | -0.005                   |                         |
| 150   | $A_1$             | 96         | 0.77     | 2651.59271(3)              | -1.460                   | -0.000                  | -1.301                   | -0.084                   |                         |
| 151   | $E$               | 155        | 3.8      | 2656.65601(7)              | -0.137                   | -0.001                  | -0.339                   | -0.007                   |                         |
| 152   | $E$               | 154        | 3.8      | 2656.65601(8)              | -0.137                   | -0.001                  | -0.340                   | -0.007                   |                         |
| 153   | $E$               | 131        | 0.62     | 2708.67591(5)              | -0.145                   | -0.000                  | -0.028                   | -0.004                   |                         |
| 154   | $E$               | 136        | 0.62     | 2708.67592(4)              | -0.145                   | -0.000                  | -0.028                   | -0.004                   |                         |
| 155   | $A_1$             | 140        | 1.4      | 2710.30435(5)              | -0.178                   | -0.001                  | -0.041                   | -0.005                   |                         |
| 156   | $A_2$             | 135        | 1.4      | 2710.30609(5)              | -0.178                   | -0.001                  | -0.041                   | -0.004                   |                         |
| 157   | $E$               | 129        | 1.6      | 2711.12078(6)              | -0.197                   | -0.000                  | -0.049                   | -0.004                   |                         |
| 158   | $E$               | 130        | 1.6      | 2711.12078(5)              | -0.197                   | -0.000                  | -0.049                   | -0.004                   |                         |
| 159   | $A_2$             | 138        | 2.4      | 2743.9151(1)               | -0.113                   | -0.001                  | -0.044                   | -0.005                   |                         |
| 160   | $E$               | 177        | 2.4      | 2743.96435(3)              | -0.114                   | -0.002                  | -0.045                   | -0.005                   |                         |
| 161   | $E$               | 187        | 2.4      | 2743.96435(2)              | -0.114                   | -0.002                  | -0.045                   | -0.005                   |                         |
| 162   | $A_1$             | 140        | 2.4      | 2744.3545(1)               | -0.114                   | -0.002                  | -0.046                   | -0.005                   |                         |
| 163   | $A_1$             | 166        | 4.6      | 2768.0139(1)               | -0.041                   | -0.003                  | -0.925                   | -0.005                   |                         |
| 164   | $E$               | 196        | 4.3      | 2775.07172(8)              | -0.090                   | -0.005                  | -0.081                   | -0.005                   |                         |
| 165   | $E$               | 197        | 4.3      | 2775.07172(8)              | -0.090                   | -0.005                  | -0.082                   | -0.005                   |                         |
| 166   | $A_1$             | 226        | 5.2      | 2776.51235(5)              | -0.080                   | -0.006                  | -0.417                   | -0.006                   |                         |
| 167   | $A_2$             | 185        | 5.0      | 2777.3522(1)               | -0.078                   | -0.004                  | -0.086                   | -0.005                   |                         |
| 168   | $A_1$             | 211        | 6.0      | 2781.93486(9)              | -0.085                   | -0.005                  | -0.203                   | -0.005                   |                         |
| 169   | $E$               | 240        | 5.1      | 2782.22752(3)              | -0.085                   | -0.004                  | -0.083                   | -0.004                   |                         |

Continued on next page.

TABLE S2 – States on Avila/Carrington AC PES; continued from previous page.

| State | $\Gamma_{C_{3v}}$ | $D_{\max}$ | $S_{vN}$ | $\tilde{E}/\text{cm}^{-1}$ | $\Delta\text{Ref. [11]}$ | $\Delta\text{Ref. [9]}$ | $\Delta\text{Ref. [34]}$ | $\Delta\text{Ref. [35]}$ | $\Delta\text{Ref. [1]}$ |
|-------|-------------------|------------|----------|----------------------------|--------------------------|-------------------------|--------------------------|--------------------------|-------------------------|
| 170   | $E$               | 207        | 5.1      | 2782.22753(8)              | -0.085                   | -0.004                  | -0.083                   | -0.004                   |                         |
| 171   | $E$               | 242        | 2.4      | 2786.66126(2)              | -0.091                   | -0.005                  | -0.077                   | -0.005                   |                         |
| 172   | $E$               | 242        | 2.4      | 2786.66126(2)              | -0.091                   | -0.005                  | -0.077                   | -0.005                   |                         |
| 173   | $E$               | 179        | 3.5      | 2789.0217(1)               | -0.087                   | -0.004                  | -0.081                   | -0.005                   |                         |
| 174   | $E$               | 209        | 3.5      | 2789.02174(6)              | -0.087                   | -0.004                  | -0.081                   | -0.005                   |                         |
| 175   | $A_2$             | 181        | 5.0      | 2790.2146(1)               | -0.083                   | -0.004                  | -0.090                   | -0.004                   |                         |
| 176   | $A_1$             | 192        | 5.8      | 2790.6624(1)               | -0.081                   | -0.005                  | -0.140                   | -0.005                   |                         |
| 177   | $E$               | 114        | 0.56     | 2812.02159(7)              | -0.478                   | -0.002                  | -0.199                   | -0.021                   |                         |
| 178   | $E$               | 113        | 0.56     | 2812.02160(7)              | -0.478                   | -0.002                  | -0.200                   | -0.021                   |                         |
| 179   | $E$               | 205        | 3.8      | 2838.80123(5)              | -0.069                   | -0.002                  | -0.032                   | -0.003                   |                         |
| 180   | $E$               | 227        | 3.8      | 2838.80124(3)              | -0.069                   | -0.002                  | -0.032                   | -0.003                   |                         |
| 181   | $E$               | 200        | 4.0      | 2841.08717(6)              | -0.072                   | -0.002                  | -0.044                   | -0.003                   |                         |
| 182   | $E$               | 244        | 4.0      | 2841.08718(2)              | -0.072                   | -0.002                  | -0.044                   | -0.003                   |                         |
| 183   | $A_1$             | 177        | 4.0      | 2841.86718(8)              | -0.073                   | -0.002                  | -0.049                   | -0.004                   |                         |
| 184   | $A_1$             | 182        | 2.4      | 2848.52231(8)              | -0.082                   | -0.003                  | -0.017                   | -0.004                   |                         |
| 185   | $A_2$             | 199        | 2.4      | 2848.52232(5)              | -0.082                   | -0.003                  | -0.017                   | -0.004                   |                         |
| 186   | $E$               | 315        | 2.7      | 2850.57683(3)              | -0.087                   | -0.003                  | -0.024                   | -0.004                   |                         |
| 187   | $E$               | 318        | 2.7      | 2850.57683(3)              | -0.087                   | -0.003                  | -0.024                   | -0.004                   |                         |
| 188   | $E$               | 298        | 2.7      | 2851.76259(3)              | -0.089                   | -0.002                  | -0.029                   | -0.004                   |                         |
| 189   | $E$               | 299        | 2.7      | 2851.76259(3)              | -0.089                   | -0.002                  | -0.030                   | -0.004                   |                         |
| 190   | $E$               | 301        | 4.3      | 2852.07901(3)              | -0.076                   | -0.002                  | -0.027                   | -0.004                   |                         |
| 191   | $E$               | 303        | 4.3      | 2852.07901(3)              | -0.076                   | -0.002                  | -0.027                   | -0.004                   |                         |
| 192   | $A_2$             | 189        | 2.7      | 2852.14317(7)              | -0.090                   | -0.003                  | -0.032                   | -0.004                   |                         |
| 193   | $E$               | 211        | 4.7      | 2853.16435(8)              | -0.085                   | -0.002                  | -0.038                   | -0.004                   |                         |
| 194   | $E$               | 202        | 4.7      | 2853.16435(9)              | -0.085                   | -0.003                  | -0.038                   | -0.004                   |                         |
| 195   | $A_1$             | 201        | 4.8      | 2853.52341(7)              | -0.088                   | -0.003                  | -0.043                   | -0.005                   |                         |
| 196   | $A_1$             | 106        | 0.91     | 2860.7398(1)               |                          | -0.000                  | -0.119                   | -0.012                   |                         |
| 197   | $A_2$             | 111        | 0.91     | 2860.7404(1)               |                          | -0.001                  | -0.120                   | -0.012                   |                         |
| 198   | $E$               | 137        | 1.6      | 2861.40255(4)              |                          | -0.000                  | -0.176                   | -0.016                   |                         |
| 199   | $E$               | 144        | 1.6      | 2861.40255(4)              |                          | -0.000                  | -0.176                   | -0.016                   |                         |
| 200   | $E$               | 205        | 3.4      | 2873.29754(3)              | -0.067                   | -0.002                  | -0.301                   | -0.004                   |                         |
| 201   | $E$               | 191        | 3.4      | 2873.29754(2)              | -0.067                   | -0.002                  | -0.303                   | -0.004                   |                         |
| 202   | $E$               | 249        | 3.3      | 2880.04588(3)              |                          | -0.005                  | -0.195                   | -0.005                   |                         |
| 203   | $E$               | 249        | 3.3      | 2880.04588(3)              |                          | -0.005                  | -0.195                   | -0.005                   |                         |
| 204   | $E$               | 248        | 3.8      | 2881.22786(3)              |                          | -0.003                  | -0.195                   | -0.004                   |                         |
| 205   | $E$               | 235        | 3.8      | 2881.22786(3)              |                          | -0.003                  | -0.195                   | -0.004                   |                         |
| 206   | $A_1$             | 176        | 3.4      | 2882.64056(7)              |                          | -0.003                  | -0.179                   | -0.004                   |                         |
| 207   | $A_2$             | 168        | 3.2      | 2882.69461(7)              |                          | -0.003                  | -0.167                   | -0.004                   |                         |
| 208   | $E$               | 203        | 4.7      | 2884.11886(2)              |                          | -0.003                  | -0.209                   | -0.005                   |                         |
| 209   | $E$               | 198        | 4.7      | 2884.11886(3)              |                          | -0.003                  | -0.210                   | -0.005                   |                         |
| 210   | $E$               | 116        | 0.13     | 2920.63704(5)              |                          | 0.000                   | -0.007                   | -0.004                   |                         |
| 211   | $E$               | 120        | 0.13     | 2920.63704(4)              |                          | -0.001                  | -0.008                   | -0.004                   |                         |
| 212   | $A_1$             | 148        | 0.66     | 2923.57377(4)              |                          | -0.000                  | -0.010                   | -0.004                   |                         |
| 213   | $A_2$             | 151        | 0.66     | 2923.57377(3)              |                          | -0.000                  | -0.010                   | -0.004                   |                         |
| 214   | $E$               | 148        | 0.93     | 2925.67303(4)              |                          | -0.001                  | -0.014                   | -0.005                   |                         |
| 215   | $E$               | 156        | 0.93     | 2925.67303(3)              |                          | -0.001                  | -0.014                   | -0.005                   |                         |
| 216   | $E$               | 155        | 1.1      | 2926.93317(2)              |                          | -0.001                  | -0.018                   | -0.005                   |                         |
| 217   | $E$               | 158        | 1.1      | 2926.93317(2)              |                          | -0.001                  | -0.018                   | -0.005                   |                         |
| 218   | $A_1$             | 151        | 1.1      | 2927.35331(3)              |                          | -0.001                  | -0.019                   | -0.005                   |                         |
| 219   | $E$               | 179        | 2.2      | 2934.72857(9)              |                          | -0.001                  | -0.016                   | -0.003                   |                         |
| 220   | $E$               | 182        | 2.2      | 2934.72858(8)              |                          | -0.001                  | -0.016                   | -0.003                   |                         |
| 221   | $A_1$             | 211        | 2.4      | 2935.18311(6)              |                          | -0.001                  | -0.017                   | -0.003                   |                         |
| 222   | $A_2$             | 159        | 2.4      | 2935.1847(1)               |                          | -0.001                  | -0.017                   | -0.003                   |                         |
| 223   | $E$               | 173        | 2.4      | 2936.54088(9)              |                          | -0.001                  | -0.025                   | -0.003                   |                         |
| 224   | $E$               | 170        | 2.4      | 2936.54089(9)              |                          | -0.001                  | -0.025                   | -0.003                   |                         |
| 225   | $A_1$             | 152        | 2.4      | 2936.7003(2)               |                          | -0.002                  | -0.023                   | -0.004                   |                         |
| 226   | $A_2$             | 155        | 2.4      | 2936.7222(1)               |                          | -0.002                  | -0.022                   | -0.004                   |                         |
| 227   | $E$               | 169        | 1.7      | 2937.64249(8)              |                          | -0.002                  | -0.025                   | -0.004                   |                         |
| 228   | $E$               | 167        | 1.8      | 2937.64249(8)              |                          | -0.002                  | -0.026                   | -0.004                   |                         |

Continued on next page.

TABLE S2 – States on Avila/Carrington AC PES; continued from previous page.

| State | $\Gamma_{C_{3v}}$ | $D_{\max}$ | $S_{vN}$ | $\tilde{E}/\text{cm}^{-1}$ | $\Delta\text{Ref. [11]}$ | $\Delta\text{Ref. [9]}$ | $\Delta\text{Ref. [34]}$ | $\Delta\text{Ref. [35]}$ | $\Delta\text{Ref. [1]}$ |
|-------|-------------------|------------|----------|----------------------------|--------------------------|-------------------------|--------------------------|--------------------------|-------------------------|
| 229   | $A_1$             | 151        | 2.6      | 2946.99773(2)              | −0.054                   | −0.209                  | −0.515                   | −0.004                   |                         |
| 230   | $A_1$             | 188        | 0.92     | 2950.90903(3)              |                          | −0.009                  | −0.147                   | −0.013                   |                         |
| 231   | $E$               | 195        | 0.41     | 2959.28048(3)              |                          | −0.005                  | −0.202                   | −0.010                   |                         |
| 232   | $E$               | 192        | 0.41     | 2959.28048(3)              |                          | −0.005                  | −0.204                   | −0.010                   |                         |
| 233   | $E$               | 135        | 0.4      | 2967.87591(2)              | −0.083                   | −0.002                  | −0.555                   | −0.005                   |                         |
| 234   | $E$               | 128        | 0.4      | 2967.87591(3)              | −0.083                   | −0.003                  | −0.556                   | −0.005                   |                         |
| 235   | $E$               | 125        | 1.6      | 2968.89893(5)              |                          | −0.003                  | −0.297                   | −0.003                   |                         |
| 236   | $E$               | 130        | 1.6      | 2968.89893(4)              |                          | −0.003                  | −0.298                   | −0.003                   |                         |
| 237   | $A_1$             | 134        | 1.7      | 2969.54144(4)              |                          | −0.003                  | −0.354                   | −0.004                   |                         |
| 238   | $A_1$             | 134        | 2.2      | 2980.73725(2)              | −0.037                   | −0.272                  | −0.556                   | −0.004                   |                         |
| 239   | $E$               | 164        | 1.0      | 3006.92123(3)              |                          |                         | −0.480                   |                          |                         |
| 240   | $E$               | 148        | 1.0      | 3006.92123(2)              |                          |                         |                          |                          |                         |
| 241   | $E$               | 268        | 4.8      | 3007.21587(2)              |                          |                         |                          |                          |                         |
| 242   | $E$               | 282        | 4.8      | 3007.21587(2)              |                          |                         |                          |                          |                         |
| 243   | $A_1$             | 226        | 5.0      | 3008.04235(6)              |                          |                         |                          |                          |                         |
| 244   | $E$               | 209        | 2.7      | 3010.9785(1)               |                          |                         |                          |                          |                         |
| 245   | $E$               | 212        | 2.7      | 3010.97852(9)              |                          |                         |                          |                          |                         |
| 246   | $E$               | 221        | 3.0      | 3011.91664(6)              |                          |                         |                          |                          |                         |
| 247   | $E$               | 218        | 3.0      | 3011.91664(6)              |                          |                         |                          |                          |                         |
| 248   | $A_2$             | 189        | 3.0      | 3012.19325(9)              |                          |                         |                          |                          |                         |
| 249   | $E$               | 185        | 4.1      | 3017.3563(1)               |                          |                         |                          |                          |                         |
| 250   | $E$               | 184        | 4.1      | 3017.3563(1)               |                          |                         |                          |                          |                         |
| 251   | $A_1$             | 182        | 4.3      | 3017.6305(1)               |                          |                         |                          |                          |                         |
| 252   | $E$               | 135        | 0.51     | 3048.77422(3)              |                          |                         |                          |                          |                         |
| 253   | $E$               | 132        | 0.51     | 3048.77422(3)              |                          |                         |                          |                          |                         |
| 254   | $A_2$             | 134        | 0.72     | 3073.90300(6)              |                          |                         |                          |                          |                         |
| 255   | $A_1$             | 139        | 0.72     | 3073.90300(5)              |                          |                         |                          |                          |                         |
| 256   | $E$               | 155        | 1.6      | 3075.69380(5)              |                          |                         |                          |                          |                         |
| 257   | $E$               | 183        | 1.6      | 3075.69381(2)              |                          |                         |                          |                          |                         |
| 258   | $E$               | 145        | 2.0      | 3076.76888(5)              |                          |                         |                          |                          |                         |
| 259   | $E$               | 144        | 2.0      | 3076.76888(6)              |                          |                         |                          |                          |                         |
| 260   | $E$               | 146        | 0.52     | 3077.00981(3)              |                          |                         |                          |                          |                         |
| 261   | $E$               | 147        | 0.52     | 3077.00981(3)              |                          |                         |                          |                          |                         |
| 262   | $A_1$             | 144        | 2.1      | 3077.12735(6)              |                          |                         |                          |                          |                         |
| 263   | $A_1$             | 155        | 0.35     | 3092.89276(2)              |                          |                         |                          |                          |                         |
| 264   | $A_2$             | 142        | 0.25     | 3093.87802(4)              |                          |                         |                          |                          |                         |
| 265   | $A_1$             | 189        | 2.5      | 3104.37289(9)              |                          |                         |                          |                          |                         |
| 266   | $A_2$             | 198        | 2.5      | 3104.38114(7)              |                          |                         |                          |                          |                         |
| 267   | $E$               | 170        | 2.5      | 3104.5448(1)               |                          |                         |                          |                          |                         |
| 268   | $E$               | 173        | 2.5      | 3104.5448(1)               |                          |                         |                          |                          |                         |
| 269   | $E$               | 172        | 1.7      | 3105.25917(9)              |                          |                         |                          |                          |                         |
| 270   | $E$               | 174        | 1.7      | 3105.25917(8)              |                          |                         |                          |                          |                         |
| 271   | $E$               | 195        | 4.6      | 3128.1919(1)               |                          |                         |                          |                          |                         |
| 272   | $E$               | 198        | 4.6      | 3128.1919(1)               |                          |                         |                          |                          |                         |
| 273   | $A_1$             | 199        | 4.5      | 3136.5650(2)               |                          |                         |                          |                          |                         |
| 274   | $A_2$             | 194        | 4.5      | 3136.5706(2)               |                          |                         |                          |                          |                         |
| 275   | $E$               | 274        | 5.0      | 3138.34895(3)              |                          |                         |                          |                          |                         |
| 276   | $E$               | 291        | 5.0      | 3138.34895(2)              |                          |                         |                          |                          |                         |
| 277   | $E$               | 271        | 6.0      | 3139.40511(5)              |                          |                         |                          |                          |                         |
| 278   | $E$               | 274        | 6.0      | 3139.40511(4)              |                          |                         |                          |                          |                         |
| 279   | $A_1$             | 128        | 2.9      | 3140.88241(5)              |                          |                         |                          |                          |                         |
| 280   | $E$               | 282        | 5.2      | 3145.07954(4)              |                          |                         |                          |                          |                         |
| 281   | $E$               | 299        | 5.2      | 3145.07954(3)              |                          |                         |                          |                          |                         |
| 282   | $A_1$             | 202        | 5.4      | 3145.2003(3)               |                          |                         |                          |                          |                         |
| 283   | $A_2$             | 200        | 5.4      | 3145.2123(3)               |                          |                         |                          |                          |                         |
| 284   | $E$               | 284        | 2.5      | 3149.07562(3)              |                          |                         |                          |                          |                         |
| 285   | $E$               | 314        | 2.5      | 3149.07562(1)              |                          |                         |                          |                          |                         |
| 286   | $A_1$             | 263        | 4.8      | 3151.27343(6)              |                          |                         |                          |                          |                         |
| 287   | $A_2$             | 232        | 4.7      | 3151.3280(1)               |                          |                         |                          |                          |                         |

Continued on next page.

TABLE S2 – States on Avila/Carrington AC PES; continued from previous page.

| State | $\Gamma_{C_{3v}}$ | $D_{\max}$ | $S_{vN}$ | $\tilde{E}/\text{cm}^{-1}$ | $\Delta\text{Ref. [11]}$ | $\Delta\text{Ref. [9]}$ | $\Delta\text{Ref. [34]}$ | $\Delta\text{Ref. [35]}$ | $\Delta\text{Ref. [1]}$ |
|-------|-------------------|------------|----------|----------------------------|--------------------------|-------------------------|--------------------------|--------------------------|-------------------------|
| 288   | $E$               | 222        | 4.7      | 3152.7912(1)               |                          |                         |                          |                          |                         |
| 289   | $E$               | 235        | 4.8      | 3152.79124(8)              |                          |                         |                          |                          |                         |
| 290   | $E$               | 227        | 5.8      | 3153.6400(1)               |                          |                         |                          |                          |                         |
| 291   | $E$               | 227        | 5.8      | 3153.6400(1)               |                          |                         |                          |                          |                         |
| 292   | $A_1$             | 205        | 3.4      | 3167.52121(4)              |                          |                         |                          |                          |                         |
| 293   | $E$               | 171        | 2.8      | 3168.63059(9)              |                          |                         |                          |                          |                         |
| 294   | $E$               | 175        | 2.8      | 3168.63059(8)              |                          |                         |                          |                          |                         |
| 295   | $A_2$             | 159        | 2.7      | 3168.71994(9)              |                          |                         |                          |                          |                         |
| 296   | $A_1$             | 135        | 3.2      | 3183.70542(5)              |                          |                         |                          |                          |                         |
| 297   | $E$               | 198        | 3.8      | 3204.33446(8)              |                          |                         |                          |                          |                         |
| 298   | $E$               | 217        | 3.8      | 3204.33447(5)              |                          |                         |                          |                          |                         |
| 299   | $A_1$             | 240        | 4.0      | 3207.12483(4)              |                          |                         |                          |                          |                         |
| 300   | $A_2$             | 251        | 4.0      | 3207.12628(3)              |                          |                         |                          |                          |                         |
| 301   | $E$               | 210        | 4.0      | 3208.56083(5)              |                          |                         |                          |                          |                         |
| 302   | $E$               | 218        | 4.0      | 3208.56083(4)              |                          |                         |                          |                          |                         |
| 303   | $E$               | 212        | 2.4      | 3214.81336(5)              |                          |                         |                          |                          |                         |
| 304   | $E$               | 212        | 2.4      | 3214.81336(5)              |                          |                         |                          |                          |                         |
| 305   | $E$               | 280        | 3.1      | 3217.11049(4)              |                          |                         |                          |                          |                         |
| 306   | $E$               | 271        | 3.1      | 3217.11049(4)              |                          |                         |                          |                          |                         |
| 307   | $E$               | 206        | 4.3      | 3218.36720(8)              |                          |                         |                          |                          |                         |
| 308   | $E$               | 221        | 4.3      | 3218.36720(6)              |                          |                         |                          |                          |                         |
| 309   | $A_1$             | 192        | 3.2      | 3218.6558(2)               |                          |                         |                          |                          |                         |
| 310   | $A_2$             | 175        | 3.2      | 3218.6610(3)               |                          |                         |                          |                          |                         |
| 311   | $E$               | 240        | 2.2      | 3219.44365(3)              |                          |                         |                          |                          |                         |
| 312   | $E$               | 235        | 2.2      | 3219.44365(3)              |                          |                         |                          |                          |                         |
| 313   | $A_1$             | 179        | 4.7      | 3219.6147(3)               |                          |                         |                          |                          |                         |
| 314   | $A_2$             | 178        | 4.7      | 3219.6158(3)               |                          |                         |                          |                          |                         |
| 315   | $E$               | 230        | 4.9      | 3220.18891(6)              |                          |                         |                          |                          |                         |
| 316   | $E$               | 229        | 4.8      | 3220.18891(6)              |                          |                         |                          |                          |                         |
| 317   | $E$               | 160        | 1.1      | 3221.86959(4)              |                          |                         |                          |                          |                         |
| 318   | $E$               | 153        | 1.1      | 3221.86959(5)              |                          |                         |                          |                          |                         |
| 319   | $E$               | 158        | 2.0      | 3222.68042(5)              |                          |                         |                          |                          |                         |
| 320   | $E$               | 163        | 2.0      | 3222.68042(5)              |                          |                         |                          |                          |                         |
| 321   | $A_1$             | 149        | 2.2      | 3222.95191(6)              |                          |                         |                          |                          |                         |
| 322   | $E$               | 281        | 5.4      | 3233.81436(2)              |                          |                         |                          |                          |                         |
| 323   | $E$               | 256        | 5.4      | 3233.81436(3)              |                          |                         |                          |                          |                         |
| 324   | $A_2$             | 253        | 5.2      | 3233.91767(3)              |                          |                         |                          |                          |                         |
| 325   | $A_1$             | 247        | 5.2      | 3234.33990(4)              |                          |                         |                          |                          |                         |
| 326   | $E$               | 268        | 3.7      | 3242.02632(2)              |                          |                         |                          |                          |                         |
| 327   | $E$               | 278        | 3.7      | 3242.02632(2)              |                          |                         |                          |                          |                         |
| 328   | $A_1$             | 272        | 3.8      | 3242.75315(2)              |                          |                         |                          |                          |                         |
| 329   | $A_2$             | 291        | 3.8      | 3243.67674(3)              |                          |                         |                          |                          |                         |
| 330   | $E$               | 290        | 5.1      | 3243.74221(2)              |                          |                         |                          |                          |                         |
| 331   | $E$               | 270        | 5.1      | 3243.74221(3)              |                          |                         |                          |                          |                         |
| 332   | $E$               | 225        | 3.4      | 3244.46170(5)              |                          |                         |                          |                          |                         |
| 333   | $E$               | 243        | 3.4      | 3244.46170(3)              |                          |                         |                          |                          |                         |
| 334   | $E$               | 226        | 4.7      | 3246.19059(6)              |                          |                         |                          |                          |                         |
| 335   | $E$               | 228        | 4.7      | 3246.19059(5)              |                          |                         |                          |                          |                         |
| 336   | $A_2$             | 220        | 5.4      | 3246.52014(9)              |                          |                         |                          |                          |                         |
| 337   | $A_1$             | 220        | 5.6      | 3246.7462(1)               |                          |                         |                          |                          |                         |
| 338   | $E$               | 131        | 0.51     | 3269.88358(3)              |                          |                         |                          |                          |                         |
| 339   | $E$               | 126        | 0.51     | 3269.88358(4)              |                          |                         |                          |                          |                         |
| 340   | $E$               | 133        | 1.9      | 3279.98357(7)              |                          |                         |                          |                          |                         |
| 341   | $E$               | 130        | 1.9      | 3279.98357(7)              |                          |                         |                          |                          |                         |
| 342   | $A_2$             | 121        | 0.15     | 3290.79731(5)              |                          |                         |                          |                          |                         |
| 343   | $A_1$             | 123        | 0.15     | 3290.79731(5)              |                          |                         |                          |                          |                         |
| 344   | $E$               | 210        | 0.76     | 3293.81482(3)              |                          |                         |                          |                          |                         |
| 345   | $E$               | 212        | 0.76     | 3293.81482(3)              |                          |                         |                          |                          |                         |
| 346   | $E$               | 226        | 1.1      | 3296.07843(3)              |                          |                         |                          |                          |                         |

Continued on next page.

TABLE S2 – States on Avila/Carrington AC PES; continued from previous page.

| State | $\Gamma_{C_{3v}}$ | $D_{\max}$ | $S_{vN}$ | $\tilde{E}/\text{cm}^{-1}$ | $\Delta\text{Ref. [11]}$ | $\Delta\text{Ref. [9]}$ | $\Delta\text{Ref. [34]}$ | $\Delta\text{Ref. [35]}$ | $\Delta\text{Ref. [1]}$ |
|-------|-------------------|------------|----------|----------------------------|--------------------------|-------------------------|--------------------------|--------------------------|-------------------------|
| 347   | $E$               | 225        | 1.1      | 3296.07843(3)              |                          |                         |                          |                          |                         |
| 348   | $A_1$             | 122        | 1.3      | 3297.5844(2)               |                          |                         |                          |                          |                         |
| 349   | $A_2$             | 120        | 1.3      | 3297.5904(2)               |                          |                         |                          |                          |                         |
| 350   | $E$               | 240        | 1.3      | 3298.34180(3)              |                          |                         |                          |                          |                         |
| 351   | $E$               | 208        | 1.3      | 3298.34180(3)              |                          |                         |                          |                          |                         |
| 352   | $A_2$             | 152        | 2.2      | 3300.5214(3)               |                          |                         |                          |                          |                         |
| 353   | $A_1$             | 152        | 2.2      | 3300.5214(3)               |                          |                         |                          |                          |                         |
| 354   | $E$               | 215        | 2.4      | 3301.12075(6)              |                          |                         |                          |                          |                         |
| 355   | $E$               | 207        | 2.4      | 3301.12076(7)              |                          |                         |                          |                          |                         |
| 356   | $E$               | 215        | 1.5      | 3302.92110(9)              |                          |                         |                          |                          |                         |
| 357   | $E$               | 248        | 1.5      | 3302.92111(5)              |                          |                         |                          |                          |                         |
| 358   | $E$               | 217        | 1.5      | 3302.93617(8)              |                          |                         |                          |                          |                         |
| 359   | $E$               | 211        | 1.5      | 3302.93617(8)              |                          |                         |                          |                          |                         |
| 360   | $A_2$             | 201        | 2.7      | 3303.55008(7)              |                          |                         |                          |                          |                         |
| 361   | $E$               | 208        | 2.7      | 3304.32338(8)              |                          |                         |                          |                          |                         |
| 362   | $E$               | 206        | 2.7      | 3304.32338(8)              |                          |                         |                          |                          |                         |
| 363   | $A_1$             | 200        | 2.7      | 3304.77339(8)              |                          |                         |                          |                          |                         |
| 364   | $E$               | 245        | 4.3      | 3307.81250(3)              |                          |                         |                          |                          |                         |
| 365   | $E$               | 243        | 4.3      | 3307.81250(3)              |                          |                         |                          |                          |                         |
| 366   | $E$               | 242        | 4.5      | 3308.72630(3)              |                          |                         |                          |                          |                         |
| 367   | $E$               | 251        | 4.5      | 3308.72630(2)              |                          |                         |                          |                          |                         |
| 368   | $E$               | 248        | 4.5      | 3315.16229(3)              |                          |                         |                          |                          |                         |
| 369   | $E$               | 247        | 4.5      | 3315.16229(3)              |                          |                         |                          |                          |                         |
| 370   | $A_1$             | 253        | 2.7      | 3317.32238(2)              |                          |                         |                          |                          |                         |
| 371   | $A_2$             | 248        | 2.6      | 3317.34403(2)              |                          |                         |                          |                          |                         |
| 372   | $E$               | 276        | 4.0      | 3323.37873(3)              |                          |                         |                          |                          |                         |
| 373   | $E$               | 276        | 4.0      | 3323.37873(3)              |                          |                         |                          |                          |                         |
| 374   | $A_1$             | 173        | 2.4      | 3329.06505(5)              |                          |                         |                          |                          |                         |
| 375   | $A_2$             | 183        | 2.4      | 3329.08593(3)              |                          |                         |                          |                          |                         |
| 376   | $E$               | 213        | 2.5      | 3329.35777(2)              |                          |                         |                          |                          |                         |
| 377   | $E$               | 206        | 2.5      | 3329.35777(2)              |                          |                         |                          |                          |                         |
| 378   | $A_1$             | 112        | 1.6      | 3329.8058(2)               |                          |                         |                          |                          |                         |
| 379   | $A_2$             | 115        | 1.6      | 3329.8061(1)               |                          |                         |                          |                          |                         |
| 380   | $E$               | 147        | 1.7      | 3331.01805(5)              |                          |                         |                          |                          |                         |
| 381   | $E$               | 144        | 1.7      | 3331.01805(6)              |                          |                         |                          |                          |                         |
| 382   | $E$               | 150        | 2.3      | 3341.82856(2)              |                          |                         |                          |                          |                         |
| 383   | $E$               | 152        | 2.3      | 3341.82857(2)              |                          |                         |                          |                          |                         |
| 384   | $E$               | 150        | 1.3      | 3363.64466(4)              |                          |                         |                          |                          |                         |
| 385   | $E$               | 147        | 1.3      | 3363.64466(4)              |                          |                         |                          |                          |                         |
| 386   | $A_1$             | 140        | 1.8      | 3363.78908(5)              |                          |                         |                          |                          |                         |
| 387   | $A_1$             | 184        | 5.0      | 3368.7162(3)               |                          |                         |                          |                          |                         |
| 388   | $A_2$             | 183        | 5.0      | 3368.7172(3)               |                          |                         |                          |                          |                         |
| 389   | $E$               | 280        | 5.2      | 3370.15656(3)              |                          |                         |                          |                          |                         |
| 390   | $E$               | 277        | 5.2      | 3370.15656(3)              |                          |                         |                          |                          |                         |
| 391   | $E$               | 226        | 2.9      | 3373.2141(1)               |                          |                         |                          |                          |                         |
| 392   | $E$               | 232        | 2.9      | 3373.21406(9)              |                          |                         |                          |                          |                         |
| 393   | $A_1$             | 178        | 3.4      | 3374.4417(4)               |                          |                         |                          |                          |                         |
| 394   | $A_2$             | 179        | 3.4      | 3374.4478(4)               |                          |                         |                          |                          |                         |
| 395   | $E$               | 211        | 2.7      | 3375.0323(1)               |                          |                         |                          |                          |                         |
| 396   | $E$               | 218        | 2.7      | 3375.03231(9)              |                          |                         |                          |                          |                         |
| 397   | $A_1$             | 212        | 4.4      | 3379.2375(1)               |                          |                         |                          |                          |                         |
| 398   | $A_2$             | 206        | 4.4      | 3379.2382(1)               |                          |                         |                          |                          |                         |
| 399   | $E$               | 209        | 4.7      | 3379.6721(1)               |                          |                         |                          |                          |                         |
| 400   | $E$               | 209        | 4.7      | 3379.67206(9)              |                          |                         |                          |                          |                         |
| 401   | $E$               | 214        | 2.6      | 3409.95161(3)              |                          |                         |                          |                          |                         |
| 402   | $E$               | 214        | 2.6      | 3409.95161(3)              |                          |                         |                          |                          |                         |
| 403   | $A_1$             | 217        | 2.6      | 3410.09763(3)              |                          |                         |                          |                          |                         |
| 404   | $A_2$             | 160        | 2.6      | 3410.11370(5)              |                          |                         |                          |                          |                         |
| 405   | $A_1$             | 195        | 2.5      | 3417.37702(2)              |                          |                         |                          |                          |                         |

Continued on next page.

TABLE S2 – States on Avila/Carrington AC PES; continued from previous page.

| State | $\Gamma_{C_{3v}}$ | $D_{\max}$ | $S_{vN}$ | $\tilde{E}/\text{cm}^{-1}$ | $\Delta\text{Ref. [11]}$ | $\Delta\text{Ref. [9]}$ | $\Delta\text{Ref. [34]}$ | $\Delta\text{Ref. [35]}$ | $\Delta\text{Ref. [1]}$ |
|-------|-------------------|------------|----------|----------------------------|--------------------------|-------------------------|--------------------------|--------------------------|-------------------------|
| 406   | $A_2$             | 191        | 2.4      | 3418.02119(2)              |                          |                         |                          |                          |                         |
| 407   | $E$               | 174        | 2.4      | 3420.28693(3)              |                          |                         |                          |                          |                         |
| 408   | $E$               | 186        | 2.4      | 3420.28693(1)              |                          |                         |                          |                          |                         |
| 409   | $A_1$             | 213        | 4.6      | 3431.29328(4)              |                          |                         |                          |                          |                         |
| 410   | $E$               | 209        | 3.5      | 3435.81800(5)              |                          |                         |                          |                          |                         |
| 411   | $E$               | 215        | 3.5      | 3435.81801(5)              |                          |                         |                          |                          |                         |
| 412   | $A_2$             | 199        | 2.6      | 3437.15740(6)              |                          |                         |                          |                          |                         |
| 413   | $E$               | 154        | 0.81     | 3440.31312(4)              |                          |                         |                          |                          |                         |
| 414   | $E$               | 154        | 0.81     | 3440.31312(4)              |                          |                         |                          |                          |                         |
| 415   | $E$               | 165        | 1.9      | 3442.15513(5)              |                          |                         |                          |                          |                         |
| 416   | $E$               | 186        | 1.9      | 3442.15513(3)              |                          |                         |                          |                          |                         |
| 417   | $A_1$             | 182        | 4.0      | 3442.2076(1)               |                          |                         |                          |                          |                         |
| 418   | $A_1$             | 158        | 2.4      | 3443.37954(7)              |                          |                         |                          |                          |                         |
| 419   | $A_2$             | 165        | 2.4      | 3443.38416(5)              |                          |                         |                          |                          |                         |
| 420   | $E$               | 256        | 3.9      | 3443.54262(3)              |                          |                         |                          |                          |                         |
| 421   | $E$               | 261        | 3.9      | 3443.54262(3)              |                          |                         |                          |                          |                         |
| 422   | $E$               | 158        | 2.6      | 3443.99482(5)              |                          |                         |                          |                          |                         |
| 423   | $E$               | 168        | 2.6      | 3443.99483(4)              |                          |                         |                          |                          |                         |
| 424   | $E$               | 280        | 2.6      | 3453.00851(3)              |                          |                         |                          |                          |                         |
| 425   | $E$               | 279        | 2.6      | 3453.00851(3)              |                          |                         |                          |                          |                         |
| 426   | $E$               | 220        | 4.2      | 3455.73513(4)              |                          |                         |                          |                          |                         |
| 427   | $E$               | 214        | 4.2      | 3455.73513(5)              |                          |                         |                          |                          |                         |
| 428   | $E$               | 230        | 2.6      | 3466.01450(8)              |                          |                         |                          |                          |                         |
| 429   | $E$               | 225        | 2.6      | 3466.01450(9)              |                          |                         |                          |                          |                         |
| 430   | $E$               | 208        | 2.7      | 3466.3589(1)               |                          |                         |                          |                          |                         |
| 431   | $E$               | 210        | 2.7      | 3466.3589(1)               |                          |                         |                          |                          |                         |
| 432   | $A_2$             | 202        | 3.0      | 3466.9173(1)               |                          |                         |                          |                          |                         |
| 433   | $E$               | 214        | 2.9      | 3467.3405(1)               |                          |                         |                          |                          |                         |
| 434   | $E$               | 212        | 2.9      | 3467.3405(1)               |                          |                         |                          |                          |                         |
| 435   | $A_1$             | 207        | 3.0      | 3467.76955(9)              |                          |                         |                          |                          |                         |
| 436   | $E$               | 231        | 4.7      | 3489.7156(1)               |                          |                         |                          |                          |                         |
| 437   | $E$               | 236        | 4.7      | 3489.7156(1)               |                          |                         |                          |                          |                         |
| 438   | $A_1$             | 228        | 4.6      | 3490.7793(1)               |                          |                         |                          |                          |                         |
| 439   | $E$               | 180        | 3.1      | 3497.53098(4)              |                          |                         |                          |                          |                         |
| 440   | $E$               | 160        | 3.1      | 3497.53098(4)              |                          |                         |                          |                          |                         |
| 441   | $A_1$             | 123        | 1.3      | 3498.05874(3)              |                          |                         |                          |                          |                         |
| 442   | $E$               | 262        | 4.5      | 3499.3252(1)               |                          |                         |                          |                          |                         |
| 443   | $E$               | 271        | 4.5      | 3499.3252(1)               |                          |                         |                          |                          |                         |
| 444   | $E$               | 291        | 5.8      | 3501.34850(8)              |                          |                         |                          |                          |                         |
| 445   | $E$               | 314        | 5.8      | 3501.34850(6)              |                          |                         |                          |                          |                         |
| 446   | $A_1$             | 269        | 5.9      | 3502.0799(1)               |                          |                         |                          |                          |                         |
| 447   | $E$               | 334        | 6.3      | 3502.50128(3)              |                          |                         |                          |                          |                         |
| 448   | $E$               | 363        | 6.3      | 3502.50128(2)              |                          |                         |                          |                          |                         |
| 449   | $A_2$             | 250        | 5.2      | 3503.1503(1)               |                          |                         |                          |                          |                         |
| 450   | $E$               | 345        | 5.2      | 3509.09177(4)              |                          |                         |                          |                          |                         |
| 451   | $E$               | 347        | 5.2      | 3509.09177(4)              |                          |                         |                          |                          |                         |
| 452   | $A_1$             | 318        | 5.9      | 3509.28239(5)              |                          |                         |                          |                          |                         |
| 453   | $E$               | 345        | 5.8      | 3509.30699(3)              |                          |                         |                          |                          |                         |
| 454   | $E$               | 327        | 5.8      | 3509.30699(5)              |                          |                         |                          |                          |                         |
| 455   | $A_2$             | 210        | 2.6      | 3512.6139(1)               |                          |                         |                          |                          |                         |
| 456   | $A_1$             | 205        | 2.6      | 3512.6140(1)               |                          |                         |                          |                          |                         |
| 457   | $E$               | 373        | 4.5      | 3514.73439(2)              |                          |                         |                          |                          |                         |
| 458   | $E$               | 365        | 4.5      | 3514.73439(3)              |                          |                         |                          |                          |                         |
| 459   | $E$               | 248        | 3.8      | 3516.3087(1)               |                          |                         |                          |                          |                         |
| 460   | $E$               | 253        | 3.8      | 3516.3087(1)               |                          |                         |                          |                          |                         |
| 461   | $A_2$             | 301        | 5.4      | 3517.18454(6)              |                          |                         |                          |                          |                         |
| 462   | $A_1$             | 262        | 6.0      | 3517.3972(1)               |                          |                         |                          |                          |                         |
| 463   | $E$               | 249        | 5.8      | 3517.6106(1)               |                          |                         |                          |                          |                         |
| 464   | $E$               | 252        | 5.8      | 3517.6106(1)               |                          |                         |                          |                          |                         |

Continued on next page.

TABLE S2 – States on Avila/Carrington AC PES; continued from previous page.

| State | $\Gamma_{C_{3v}}$ | $D_{\max}$ | $S_{vN}$ | $\tilde{E}/\text{cm}^{-1}$ | $\Delta\text{Ref. [11]}$ | $\Delta\text{Ref. [9]}$ | $\Delta\text{Ref. [34]}$ | $\Delta\text{Ref. [35]}$ | $\Delta\text{Ref. [1]}$ |
|-------|-------------------|------------|----------|----------------------------|--------------------------|-------------------------|--------------------------|--------------------------|-------------------------|
| 465   | $E$               | 282        | 3.7      | 3525.01535(2)              |                          |                         |                          |                          |                         |
| 466   | $E$               | 286        | 3.7      | 3525.01535(2)              |                          |                         |                          |                          |                         |
| 467   | $A_1$             | 168        | 3.1      | 3526.5280(4)               |                          |                         |                          |                          |                         |
| 468   | $A_2$             | 168        | 3.1      | 3526.5320(3)               |                          |                         |                          |                          |                         |
| 469   | $E$               | 197        | 2.4      | 3526.8644(1)               |                          |                         |                          |                          |                         |
| 470   | $E$               | 197        | 2.3      | 3526.8644(1)               |                          |                         |                          |                          |                         |
| 471   | $E$               | 165        | 3.4      | 3540.66807(6)              |                          |                         |                          |                          |                         |
| 472   | $E$               | 175        | 3.4      | 3540.66808(4)              |                          |                         |                          |                          |                         |
| 473   | $E$               | 233        | 0.63     | 3547.29160(3)              |                          |                         |                          |                          |                         |
| 474   | $E$               | 234        | 0.63     | 3547.29160(3)              |                          |                         |                          |                          |                         |
| 475   | $E$               | 215        | 2.4      | 3552.57597(3)              |                          |                         |                          |                          |                         |
| 476   | $E$               | 213        | 2.4      | 3552.57597(3)              |                          |                         |                          |                          |                         |
| 477   | $A_2$             | 171        | 2.2      | 3557.43267(3)              |                          |                         |                          |                          |                         |
| 478   | $A_1$             | 170        | 2.5      | 3558.21396(4)              |                          |                         |                          |                          |                         |
| 479   | $A_1$             | 235        | 3.8      | 3571.04358(4)              |                          |                         |                          |                          |                         |
| 480   | $A_2$             | 245        | 3.8      | 3571.04359(4)              |                          |                         |                          |                          |                         |
| 481   | $E$               | 256        | 4.1      | 3574.23278(5)              |                          |                         |                          |                          |                         |
| 482   | $E$               | 269        | 4.1      | 3574.23278(4)              |                          |                         |                          |                          |                         |
| 483   | $E$               | 263        | 4.2      | 3576.20691(3)              |                          |                         |                          |                          |                         |
| 484   | $E$               | 267        | 4.2      | 3576.20691(3)              |                          |                         |                          |                          |                         |
| 485   | $A_1$             | 224        | 4.2      | 3576.87789(5)              |                          |                         |                          |                          |                         |
| 486   | $E$               | 204        | 2.5      | 3582.20741(9)              |                          |                         |                          |                          |                         |
| 487   | $E$               | 206        | 2.5      | 3582.20741(8)              |                          |                         |                          |                          |                         |
| 488   | $E$               | 161        | 1.2      | 3584.28176(7)              |                          |                         |                          |                          |                         |
| 489   | $E$               | 165        | 1.2      | 3584.28176(5)              |                          |                         |                          |                          |                         |
| 490   | $A_1$             | 287        | 3.7      | 3584.55082(5)              |                          |                         |                          |                          |                         |
| 491   | $A_2$             | 283        | 3.7      | 3584.55083(6)              |                          |                         |                          |                          |                         |
| 492   | $A_1$             | 129        | 2.4      | 3585.1055(2)               |                          |                         |                          |                          |                         |
| 493   | $A_2$             | 128        | 2.4      | 3585.1080(2)               |                          |                         |                          |                          |                         |
| 494   | $E$               | 186        | 2.8      | 3585.52083(4)              |                          |                         |                          |                          |                         |
| 495   | $E$               | 194        | 2.8      | 3585.52083(3)              |                          |                         |                          |                          |                         |
| 496   | $A_2^*$           | 169        | 4.3      | 3585.8252(3)               |                          |                         |                          |                          |                         |
| 497   | $A_1^*$           | 172        | 4.3      | 3585.8252(3)               |                          |                         |                          |                          |                         |
| 498   | $E$               | 293        | 4.3      | 3586.29367(6)              |                          |                         |                          |                          |                         |
| 499   | $E$               | 294        | 4.3      | 3586.29367(6)              |                          |                         |                          |                          |                         |
| 500   | $E$               | 365        | 4.6      | 3587.24300(2)              |                          |                         |                          |                          |                         |
| 501   | $E$               | 289        | 4.6      | 3587.24300(5)              |                          |                         |                          |                          |                         |
| 502   | $E$               | 278        | 4.6      | 3587.43454(3)              |                          |                         |                          |                          |                         |
| 503   | $E$               | 262        | 4.6      | 3587.43454(5)              |                          |                         |                          |                          |                         |
| 504   | $E$               | 309        | 4.7      | 3587.93771(4)              |                          |                         |                          |                          |                         |
| 505   | $E$               | 305        | 4.7      | 3587.93771(4)              |                          |                         |                          |                          |                         |
| 506   | $A_1$             | 244        | 5.2      | 3587.96357(7)              |                          |                         |                          |                          |                         |
| 507   | $A_2$             | 233        | 3.1      | 3588.00758(6)              |                          |                         |                          |                          |                         |
| 508   | $A_1$             | 209        | 5.5      | 3595.6929(3)               |                          |                         |                          |                          |                         |
| 509   | $A_2$             | 206        | 5.4      | 3595.6996(2)               |                          |                         |                          |                          |                         |
| 510   | $E$               | 301        | 5.2      | 3596.08000(4)              |                          |                         |                          |                          |                         |
| 511   | $E$               | 300        | 5.2      | 3596.08000(4)              |                          |                         |                          |                          |                         |
| 512   | $E$               | 275        | 4.2      | 3596.94168(5)              |                          |                         |                          |                          |                         |
| 513   | $E$               | 285        | 4.2      | 3596.94168(4)              |                          |                         |                          |                          |                         |
| 514   | $A_1$             | 279        | 3.9      | 3605.14399(7)              |                          |                         |                          |                          |                         |
| 515   | $A_2$             | 277        | 3.9      | 3605.14533(6)              |                          |                         |                          |                          |                         |
| 516   | $E$               | 347        | 4.0      | 3606.35194(2)              |                          |                         |                          |                          |                         |
| 517   | $E$               | 352        | 4.0      | 3606.35194(2)              |                          |                         |                          |                          |                         |
| 518   | $A_1$             | 220        | 5.6      | 3607.2657(2)               |                          |                         |                          |                          |                         |
| 519   | $A_2$             | 222        | 5.5      | 3607.2701(2)               |                          |                         |                          |                          |                         |
| 520   | $E$               | 309        | 3.5      | 3607.41538(3)              |                          |                         |                          |                          |                         |
| 521   | $E$               | 339        | 3.5      | 3607.41538(1)              |                          |                         |                          |                          |                         |
| 522   | $E$               | 335        | 4.1      | 3607.52519(3)              |                          |                         |                          |                          |                         |
| 523   | $E$               | 329        | 4.2      | 3607.52519(2)              |                          |                         |                          |                          |                         |

Continued on next page.



TABLE S2 – States on Avila/Carrington AC PES; continued from previous page.

| State | $\Gamma_{C_{3v}}$ | $D_{\max}$ | $S_{vN}$ | $\tilde{E}/\text{cm}^{-1}$ | $\Delta\text{Ref. [11]}$ | $\Delta\text{Ref. [9]}$ | $\Delta\text{Ref. [34]}$ | $\Delta\text{Ref. [35]}$ | $\Delta\text{Ref. [1]}$ |
|-------|-------------------|------------|----------|----------------------------|--------------------------|-------------------------|--------------------------|--------------------------|-------------------------|
| 524   | $A_1$             | 277        | 5.4      | 3609.29053(9)              |                          |                         |                          |                          |                         |
| 525   | $A_2$             | 281        | 5.2      | 3609.40645(7)              |                          |                         |                          |                          |                         |
| 526   | $E$               | 333        | 5.4      | 3609.99586(2)              |                          |                         |                          |                          |                         |
| 527   | $E$               | 350        | 5.4      | 3609.99586(2)              |                          |                         |                          |                          |                         |
| 528   | $E$               | 257        | 5.4      | 3610.3070(1)               |                          |                         |                          |                          |                         |
| 529   | $E$               | 248        | 5.4      | 3610.3070(1)               |                          |                         |                          |                          |                         |
| 530   | $A_2$             | 159        | 2.7      | 3627.0503(2)               |                          |                         |                          |                          |                         |
| 531   | $E$               | 182        | 2.7      | 3627.07906(7)              |                          |                         |                          |                          |                         |
| 532   | $E$               | 171        | 2.7      | 3627.0791(1)               |                          |                         |                          |                          |                         |
| 533   | $A_1$             | 205        | 2.7      | 3627.49720(4)              |                          |                         |                          |                          |                         |
| 534   | $A_1$             | 185        | 6.2      | 3632.80956(9)              |                          |                         |                          |                          |                         |
| 535   | $E$               | 192        | 4.0      | 3638.02306(9)              |                          |                         |                          |                          |                         |
| 536   | $E$               | 194        | 4.0      | 3638.02306(9)              |                          |                         |                          |                          |                         |
| 537   | $A_2$             | 180        | 3.9      | 3638.1525(1)               |                          |                         |                          |                          |                         |
| 538   | $A_1$             | 192        | 6.1      | 3641.43973(8)              |                          |                         |                          |                          |                         |
| 539   | $E$               | 127        | 0.16     | 3662.03960(6)              |                          |                         |                          |                          |                         |
| 540   | $E$               | 128        | 0.16     | 3662.03960(6)              |                          |                         |                          |                          |                         |
| 541   | $E$               | 223        | 0.91     | 3665.03583(3)              |                          |                         |                          |                          |                         |
| 542   | $E$               | 238        | 0.91     | 3665.03583(2)              |                          |                         |                          |                          |                         |
| 543   | $A_1$             | 329        | 4.3      | 3666.68645(3)              |                          |                         |                          |                          |                         |
| 544   | $E$               | 245        | 2.4      | 3666.7940(1)               |                          |                         |                          |                          |                         |
| 545   | $E$               | 247        | 2.4      | 3666.7940(1)               |                          |                         |                          |                          |                         |
| 546   | $A_1$             | 281        | 1.3      | 3667.36638(3)              |                          |                         |                          |                          |                         |
| 547   | $A_2$             | 267        | 1.3      | 3667.36639(3)              |                          |                         |                          |                          |                         |
| 548   | $E$               | 241        | 2.2      | 3667.44896(4)              |                          |                         |                          |                          |                         |
| 549   | $E$               | 293        | 2.2      | 3667.44896(1)              |                          |                         |                          |                          |                         |
| 550   | $E$               | 224        | 2.5      | 3668.19382(8)              |                          |                         |                          |                          |                         |
| 551   | $E$               | 229        | 2.5      | 3668.19383(8)              |                          |                         |                          |                          |                         |
| 552   | $E$               | 234        | 1.5      | 3669.03054(3)              |                          |                         |                          |                          |                         |
| 553   | $E$               | 271        | 1.5      | 3669.03054(2)              |                          |                         |                          |                          |                         |
| 554   | $E$               | 324        | 2.5      | 3670.01070(2)              |                          |                         |                          |                          |                         |
| 555   | $E$               | 322        | 2.5      | 3670.01070(2)              |                          |                         |                          |                          |                         |
| 556   | $E$               | 265        | 3.5      | 3670.2110(1)               |                          |                         |                          |                          |                         |
| 557   | $E$               | 353        | 3.5      | 3670.21104(9)              |                          |                         |                          |                          |                         |
| 558   | $A_1$             | 280        | 4.2      | 3670.30006(9)              |                          |                         |                          |                          |                         |
| 559   | $A_2$             | 307        | 2.8      | 3670.36073(3)              |                          |                         |                          |                          |                         |
| 560   | $A_1$             | 339        | 4.2      | 3670.41050(3)              |                          |                         |                          |                          |                         |
| 561   | $E$               | 270        | 2.8      | 3670.86728(3)              |                          |                         |                          |                          |                         |
| 562   | $E$               | 304        | 2.7      | 3670.86728(1)              |                          |                         |                          |                          |                         |
| 563   | $A_1$             | 336        | 4.5      | 3671.39998(3)              |                          |                         |                          |                          |                         |
| 564   | $E$               | 258        | 2.8      | 3671.45903(5)              |                          |                         |                          |                          |                         |
| 565   | $E$               | 263        | 2.8      | 3671.45903(5)              |                          |                         |                          |                          |                         |
| 566   | $A_1$             | 305        | 3.2      | 3671.99053(7)              |                          |                         |                          |                          |                         |
| 567   | $A_2$             | 318        | 2.8      | 3672.02222(2)              |                          |                         |                          |                          |                         |
| 568   | $A_2$             | 302        | 5.6      | 3672.32811(6)              |                          |                         |                          |                          |                         |
| 569   | $A_1$             | 311        | 8.1      | 3672.33160(8)              |                          |                         |                          |                          |                         |
| 570   | $E$               | 235        | 2.3      | 3672.88720(6)              |                          |                         |                          |                          |                         |
| 571   | $E$               | 234        | 2.4      | 3672.88720(7)              |                          |                         |                          |                          |                         |
| 572   | $E$               | 290        | 1.5      | 3673.75724(3)              |                          |                         |                          |                          |                         |
| 573   | $E$               | 285        | 1.4      | 3673.75724(3)              |                          |                         |                          |                          |                         |
| 574   | $E$               | 291        | 4.4      | 3675.16889(6)              |                          |                         |                          |                          |                         |
| 575   | $E$               | 337        | 4.4      | 3675.16890(3)              |                          |                         |                          |                          |                         |
| 576   | $E$               | 279        | 2.9      | 3676.58987(8)              |                          |                         |                          |                          |                         |
| 577   | $E$               | 285        | 2.9      | 3676.58987(7)              |                          |                         |                          |                          |                         |
| 578   | $A_1$             | 308        | 6.9      | 3677.86713(4)              |                          |                         |                          |                          |                         |
| 579   | $E$               | 304        | 5.6      | 3681.76541(3)              |                          |                         |                          |                          |                         |
| 580   | $E$               | 323        | 5.6      | 3681.76541(2)              |                          |                         |                          |                          |                         |
| 581   | $A_2$             | 315        | 5.8      | 3683.03726(3)              |                          |                         |                          |                          |                         |
| 582   | $A_1$             | 311        | 7.0      | 3685.49862(3)              |                          |                         |                          |                          |                         |

Continued on next page.

TABLE S2 – States on Avila/Carrington AC PES; continued from previous page.

| State | $\Gamma_{C_{3v}}$ | $D_{\max}$ | $S_{vN}$ | $\tilde{E}/\text{cm}^{-1}$ | $\Delta\text{Ref. [11]}$ | $\Delta\text{Ref. [9]}$ | $\Delta\text{Ref. [34]}$ | $\Delta\text{Ref. [35]}$ | $\Delta\text{Ref. [1]}$ |
|-------|-------------------|------------|----------|----------------------------|--------------------------|-------------------------|--------------------------|--------------------------|-------------------------|
| 583   | $E$               | 208        | 2.4      | 3691.47006(7)              |                          |                         |                          |                          |                         |
| 584   | $E$               | 222        | 2.4      | 3691.47006(4)              |                          |                         |                          |                          |                         |
| 585   | $E$               | 168        | 1.6      | 3691.90016(6)              |                          |                         |                          |                          |                         |
| 586   | $E$               | 174        | 1.6      | 3691.90016(5)              |                          |                         |                          |                          |                         |
| 587   | $A_1$             | 261        | 2.6      | 3692.03303(2)              |                          |                         |                          |                          |                         |
| 588   | $A_2$             | 208        | 2.6      | 3692.03785(7)              |                          |                         |                          |                          |                         |
| 589   | $E$               | 225        | 0.63     | 3692.39257(2)              |                          |                         |                          |                          |                         |
| 590   | $E$               | 226        | 0.63     | 3692.39257(2)              |                          |                         |                          |                          |                         |
| 591   | $E$               | 170        | 1.8      | 3693.60604(6)              |                          |                         |                          |                          |                         |
| 592   | $E$               | 168        | 1.8      | 3693.60604(6)              |                          |                         |                          |                          |                         |
| 593   | $A_1$             | 164        | 1.9      | 3694.17526(6)              |                          |                         |                          |                          |                         |
| 594   | $E$               | 168        | 2.3      | 3704.11760(7)              |                          |                         |                          |                          |                         |
| 595   | $E$               | 164        | 2.3      | 3704.11760(8)              |                          |                         |                          |                          |                         |
| 596   | $A_1$             | 173        | 2.4      | 3704.76761(7)              |                          |                         |                          |                          |                         |
| 597   | $A_1$             | 125        | 1.5      | 3721.7666(2)               |                          |                         |                          |                          |                         |
| 598   | $A_2$             | 120        | 1.5      | 3721.7674(2)               |                          |                         |                          |                          |                         |
| 599   | $E$               | 154        | 2.4      | 3721.88957(6)              |                          |                         |                          |                          |                         |
| 600   | $E$               | 164        | 2.4      | 3721.88957(4)              |                          |                         |                          |                          |                         |
| 601   | $E$               | 137        | 1.5      | 3731.32108(3)              |                          |                         |                          |                          |                         |
| 602   | $E$               | 131        | 1.5      | 3731.32108(5)              |                          |                         |                          |                          |                         |
| 603   | $E$               | 294        | 5.1      | 3731.43689(5)              |                          |                         |                          |                          |                         |
| 604   | $E$               | 365        | 5.1      | 3731.43690(1)              |                          |                         |                          |                          |                         |
| 605   | $E$               | 379        | 5.7      | 3733.32858(2)              |                          |                         |                          |                          |                         |
| 606   | $E$               | 294        | 5.7      | 3733.32858(6)              |                          |                         |                          |                          |                         |
| 607   | $A_1$             | 275        | 5.8      | 3733.97926(6)              |                          |                         |                          |                          |                         |
| 608   | $A_2$             | 186        | 3.0      | 3736.6383(4)               |                          |                         |                          |                          |                         |
| 609   | $A_1$             | 180        | 3.0      | 3736.6383(4)               |                          |                         |                          |                          |                         |
| 610   | $E$               | 357        | 3.8      | 3738.03389(3)              |                          |                         |                          |                          |                         |
| 611   | $E$               | 314        | 3.8      | 3738.03389(5)              |                          |                         |                          |                          |                         |
| 612   | $E$               | 304        | 3.9      | 3738.89446(4)              |                          |                         |                          |                          |                         |
| 613   | $E$               | 329        | 3.9      | 3738.89446(2)              |                          |                         |                          |                          |                         |
| 614   | $A_2$             | 229        | 3.9      | 3739.1895(1)               |                          |                         |                          |                          |                         |
| 615   | $E$               | 232        | 4.6      | 3742.3132(1)               |                          |                         |                          |                          |                         |
| 616   | $E$               | 234        | 4.6      | 3742.3132(1)               |                          |                         |                          |                          |                         |
| 617   | $E$               | 244        | 5.1      | 3742.7937(1)               |                          |                         |                          |                          |                         |
| 618   | $E$               | 250        | 5.1      | 3742.7937(1)               |                          |                         |                          |                          |                         |
| 619   | $A_1$             | 232        | 5.2      | 3742.9249(1)               |                          |                         |                          |                          |                         |
| 620   | $A_2$             | 232        | 2.7      | 3772.32933(3)              |                          |                         |                          |                          |                         |
| 621   | $A_1$             | 234        | 2.7      | 3772.32983(3)              |                          |                         |                          |                          |                         |
| 622   | $E$               | 276        | 3.0      | 3772.60869(2)              |                          |                         |                          |                          |                         |
| 623   | $E$               | 254        | 3.0      | 3772.60869(3)              |                          |                         |                          |                          |                         |
| 624   | $E$               | 237        | 1.7      | 3773.10527(3)              |                          |                         |                          |                          |                         |
| 625   | $E$               | 247        | 1.7      | 3773.10527(2)              |                          |                         |                          |                          |                         |
| 626   | $E$               | 269        | 5.8      | 3774.01682(4)              |                          |                         |                          |                          |                         |
| 627   | $E$               | 275        | 5.9      | 3774.01683(4)              |                          |                         |                          |                          |                         |
| 628   | $E$               | 271        | 4.0      | 3776.40480(3)              |                          |                         |                          |                          |                         |
| 629   | $E$               | 289        | 3.9      | 3776.40480(4)              |                          |                         |                          |                          |                         |
| 630   | $E$               | 258        | 4.1      | 3778.04704(3)              |                          |                         |                          |                          |                         |
| 631   | $E$               | 302        | 4.1      | 3778.04704(3)              |                          |                         |                          |                          |                         |
| 632   | $A_1$             | 241        | 3.7      | 3778.85564(7)              |                          |                         |                          |                          |                         |
| 633   | $A_2$             | 281        | 3.6      | 3778.90530(2)              |                          |                         |                          |                          |                         |
| 634   | $E$               | 253        | 4.8      | 3782.31577(3)              |                          |                         |                          |                          |                         |
| 635   | $E$               | 250        | 4.8      | 3782.31577(3)              |                          |                         |                          |                          |                         |
| 636   | $E$               | 285        | 6.1      | 3788.03617(4)              |                          |                         |                          |                          |                         |
| 637   | $E$               | 295        | 6.1      | 3788.03617(3)              |                          |                         |                          |                          |                         |
| 638   | $E$               | 308        | 6.3      | 3793.27889(3)              |                          |                         |                          |                          |                         |
| 639   | $E$               | 300        | 6.3      | 3793.27890(4)              |                          |                         |                          |                          |                         |
| 640   | $A_1$             | 239        | 4.4      | 3795.8978(1)               |                          |                         |                          |                          |                         |
| 641   | $A_2$             | 274        | 4.3      | 3795.96095(6)              |                          |                         |                          |                          |                         |

Continued on next page.

TABLE S2 – States on Avila/Carrington AC PES; continued from previous page.

| State | $\Gamma_{C_{3v}}$ | $D_{\max}$ | $S_{vN}$ | $\tilde{E}/\text{cm}^{-1}$ | $\Delta\text{Ref. [11]}$ | $\Delta\text{Ref. [9]}$ | $\Delta\text{Ref. [34]}$ | $\Delta\text{Ref. [35]}$ | $\Delta\text{Ref. [1]}$ |
|-------|-------------------|------------|----------|----------------------------|--------------------------|-------------------------|--------------------------|--------------------------|-------------------------|
| 642   | $E$               | 314        | 3.3      | 3797.90645(2)              |                          |                         |                          |                          |                         |
| 643   | $E$               | 326        | 3.3      | 3797.90645(2)              |                          |                         |                          |                          |                         |
| 644   | $E$               | 344        | 5.3      | 3802.30049(2)              |                          |                         |                          |                          |                         |
| 645   | $E$               | 350        | 5.3      | 3802.30049(2)              |                          |                         |                          |                          |                         |
| 646   | $A_1$             | 280        | 5.5      | 3804.67065(6)              |                          |                         |                          |                          |                         |
| 647   | $A_2$             | 287        | 5.4      | 3804.87125(5)              |                          |                         |                          |                          |                         |
| 648   | $E$               | 299        | 6.6      | 3805.16010(5)              |                          |                         |                          |                          |                         |
| 649   | $E$               | 322        | 6.6      | 3805.16011(3)              |                          |                         |                          |                          |                         |
| 650   | $E$               | 155        | 0.92     | 3807.89690(5)              |                          |                         |                          |                          |                         |
| 651   | $E$               | 164        | 0.92     | 3807.89690(4)              |                          |                         |                          |                          |                         |
| 652   | $A_1$             | 135        | 2.1      | 3809.6732(2)               |                          |                         |                          |                          |                         |
| 653   | $A_2$             | 144        | 2.1      | 3809.6732(1)               |                          |                         |                          |                          |                         |
| 654   | $E$               | 185        | 2.7      | 3810.93609(5)              |                          |                         |                          |                          |                         |
| 655   | $E$               | 179        | 2.7      | 3810.93609(6)              |                          |                         |                          |                          |                         |
| 656   | $E$               | 169        | 3.0      | 3811.69151(6)              |                          |                         |                          |                          |                         |
| 657   | $E$               | 172        | 3.0      | 3811.69152(6)              |                          |                         |                          |                          |                         |
| 658   | $A_1$             | 170        | 3.0      | 3811.94290(6)              |                          |                         |                          |                          |                         |
| 659   | $E$               | 239        | 2.7      | 3813.8517(1)               |                          |                         |                          |                          |                         |
| 660   | $E$               | 298        | 2.7      | 3813.85170(8)              |                          |                         |                          |                          |                         |
| 661   | $A_1$             | 225        | 3.4      | 3815.8541(1)               |                          |                         |                          |                          |                         |
| 662   | $A_2$             | 222        | 3.1      | 3816.6230(1)               |                          |                         |                          |                          |                         |
| 663   | $E$               | 240        | 5.5      | 3818.0913(1)               |                          |                         |                          |                          |                         |
| 664   | $E$               | 235        | 5.6      | 3818.0913(1)               |                          |                         |                          |                          |                         |
| 665   | $A_1$             | 189        | 0.9      | 3827.07303(5)              |                          |                         |                          |                          |                         |
| 666   | $E$               | 240        | 2.7      | 3828.8648(1)               |                          |                         |                          |                          |                         |
| 667   | $E$               | 241        | 2.7      | 3828.8648(1)               |                          |                         |                          |                          |                         |
| 668   | $A_1$             | 193        | 2.9      | 3829.3712(3)               |                          |                         |                          |                          |                         |
| 669   | $A_2$             | 196        | 2.9      | 3829.3747(3)               |                          |                         |                          |                          |                         |
| 670   | $E$               | 239        | 3.2      | 3830.32672(9)              |                          |                         |                          |                          |                         |
| 671   | $E$               | 234        | 3.2      | 3830.3267(1)               |                          |                         |                          |                          |                         |
| 672   | $A_1$             | 209        | 3.2      | 3830.5414(3)               |                          |                         |                          |                          |                         |
| 673   | $A_2$             | 210        | 3.2      | 3830.5650(2)               |                          |                         |                          |                          |                         |
| 674   | $E$               | 239        | 2.8      | 3831.38947(8)              |                          |                         |                          |                          |                         |
| 675   | $E$               | 230        | 2.8      | 3831.3895(1)               |                          |                         |                          |                          |                         |
| 676   | $E$               | 191        | 0.79     | 3835.72221(4)              |                          |                         |                          |                          |                         |
| 677   | $E$               | 190        | 0.79     | 3835.72221(4)              |                          |                         |                          |                          |                         |
| 678   | $A_1$             | 178        | 2.5      | 3849.50030(2)              |                          |                         |                          |                          |                         |
| 679   | $E$               | 141        | 1.6      | 3851.53297(6)              |                          |                         |                          |                          |                         |
| 680   | $E$               | 144        | 1.6      | 3851.53297(5)              |                          |                         |                          |                          |                         |
| 681   | $A_1$             | 254        | 4.7      | 3852.5391(1)               |                          |                         |                          |                          |                         |
| 682   | $A_2$             | 272        | 4.7      | 3852.53963(9)              |                          |                         |                          |                          |                         |
| 683   | $E$               | 254        | 4.5      | 3854.4771(1)               |                          |                         |                          |                          |                         |
| 684   | $E$               | 264        | 4.5      | 3854.47711(8)              |                          |                         |                          |                          |                         |
| 685   | $E$               | 183        | 3.2      | 3855.45963(6)              |                          |                         |                          |                          |                         |
| 686   | $E$               | 181        | 3.2      | 3855.45963(6)              |                          |                         |                          |                          |                         |
| 687   | $A_1$             | 184        | 3.3      | 3855.99563(6)              |                          |                         |                          |                          |                         |
| 688   | $E$               | 291        | 4.6      | 3863.2878(1)               |                          |                         |                          |                          |                         |
| 689   | $E$               | 307        | 4.6      | 3863.28785(9)              |                          |                         |                          |                          |                         |
| 690   | $A_1$             | 236        | 6.1      | 3865.4974(5)               |                          |                         |                          |                          |                         |
| 691   | $A_2$             | 231        | 6.1      | 3865.5103(6)               |                          |                         |                          |                          |                         |
| 692   | $A_1$             | 242        | 6.5      | 3866.6525(4)               |                          |                         |                          |                          |                         |
| 693   | $E$               | 302        | 5.8      | 3866.65455(9)              |                          |                         |                          |                          |                         |
| 694   | $E$               | 298        | 5.8      | 3866.6546(1)               |                          |                         |                          |                          |                         |
| 695   | $A_2$             | 234        | 6.5      | 3866.6567(5)               |                          |                         |                          |                          |                         |
| 696   | $E$               | 328        | 5.5      | 3868.00367(6)              |                          |                         |                          |                          |                         |
| 697   | $E$               | 319        | 5.5      | 3868.00367(8)              |                          |                         |                          |                          |                         |
| 698   | $E$               | 157        | 0.55     | 3870.22894(3)              |                          |                         |                          |                          |                         |
| 699   | $E$               | 153        | 0.55     | 3870.22894(5)              |                          |                         |                          |                          |                         |
| 700   | $E$               | 414        | 5.0      | 3873.90105(2)              |                          |                         |                          |                          |                         |

Continued on next page.

TABLE S2 – States on Avila/Carrington AC PES; continued from previous page.

| State | $\Gamma_{C_{3v}}$ | $D_{\max}$ | $S_{vN}$ | $\tilde{E}/\text{cm}^{-1}$ | $\Delta\text{Ref. [11]}$ | $\Delta\text{Ref. [9]}$ | $\Delta\text{Ref. [34]}$ | $\Delta\text{Ref. [35]}$ | $\Delta\text{Ref. [1]}$ |
|-------|-------------------|------------|----------|----------------------------|--------------------------|-------------------------|--------------------------|--------------------------|-------------------------|
| 701   | $E$               | 410        | 5.0      | 3873.90105(2)              |                          |                         |                          |                          |                         |
| 702   | $A_1$             | 237        | 5.9      | 3874.4565(6)               |                          |                         |                          |                          |                         |
| 703   | $A_2$             | 241        | 5.9      | 3874.4688(5)               |                          |                         |                          |                          |                         |
| 704   | $E$               | 321        | 5.4      | 3874.56496(7)              |                          |                         |                          |                          |                         |
| 705   | $E$               | 326        | 5.4      | 3874.56496(6)              |                          |                         |                          |                          |                         |
| 706   | $E$               | 293        | 2.7      | 3877.26150(5)              |                          |                         |                          |                          |                         |
| 707   | $E$               | 279        | 2.7      | 3877.26150(6)              |                          |                         |                          |                          |                         |
| 708   | $E$               | 425        | 4.1      | 3879.31107(2)              |                          |                         |                          |                          |                         |
| 709   | $E$               | 290        | 4.1      | 3879.3111(1)               |                          |                         |                          |                          |                         |
| 710   | $A_1$             | 283        | 5.2      | 3880.8457(1)               |                          |                         |                          |                          |                         |
| 711   | $A_2$             | 281        | 5.0      | 3880.9326(1)               |                          |                         |                          |                          |                         |
| 712   | $A_1$             | 196        | 2.4      | 3881.95235(2)              |                          |                         |                          |                          |                         |
| 713   | $E$               | 280        | 5.1      | 3881.9862(1)               |                          |                         |                          |                          |                         |
| 714   | $E$               | 278        | 5.1      | 3881.9862(1)               |                          |                         |                          |                          |                         |
| 715   | $A_1$             | 227        | 5.9      | 3882.5284(3)               |                          |                         |                          |                          |                         |
| 716   | $A_2$             | 231        | 5.9      | 3882.5285(2)               |                          |                         |                          |                          |                         |
| 717   | $E$               | 301        | 6.0      | 3882.5549(1)               |                          |                         |                          |                          |                         |
| 718   | $E$               | 299        | 6.0      | 3882.5549(1)               |                          |                         |                          |                          |                         |
| 719   | $E$               | 373        | 4.2      | 3883.73409(2)              |                          |                         |                          |                          |                         |
| 720   | $E$               | 373        | 4.2      | 3883.73409(2)              |                          |                         |                          |                          |                         |
| 721   | $A_1$             | 275        | 4.6      | 3884.17384(7)              |                          |                         |                          |                          |                         |
| 722   | $E$               | 244        | 3.3      | 3885.7154(1)               |                          |                         |                          |                          |                         |
| 723   | $E$               | 245        | 3.3      | 3885.7154(1)               |                          |                         |                          |                          |                         |
| 724   | $E$               | 265        | 3.8      | 3886.22433(8)              |                          |                         |                          |                          |                         |
| 725   | $E$               | 265        | 3.8      | 3886.22433(8)              |                          |                         |                          |                          |                         |
| 726   | $A_2$             | 235        | 3.8      | 3886.3909(1)               |                          |                         |                          |                          |                         |
| 727   | $E$               | 199        | 3.7      | 3898.90242(7)              |                          |                         |                          |                          |                         |
| 728   | $E$               | 197        | 3.7      | 3898.90242(8)              |                          |                         |                          |                          |                         |
| 729   | $A_1$             | 248        | 3.9      | 3899.07868(3)              |                          |                         |                          |                          |                         |
| 730   | $A_1$             | 286        | 5.8      | 3901.81097(2)              |                          |                         |                          |                          |                         |
| 731   | $A_2$             | 280        | 5.8      | 3902.89384(2)              |                          |                         |                          |                          |                         |
| 732   | $E$               | 298        | 5.7      | 3904.60814(2)              |                          |                         |                          |                          |                         |
| 733   | $E$               | 301        | 5.7      | 3904.60814(2)              |                          |                         |                          |                          |                         |
| 734   | $A_2$             | 293        | 5.0      | 3908.51363(2)              |                          |                         |                          |                          |                         |
| 735   | $A_1$             | 307        | 4.8      | 3909.11285(2)              |                          |                         |                          |                          |                         |
| 736   | $E$               | 303        | 5.8      | 3909.85801(3)              |                          |                         |                          |                          |                         |
| 737   | $E$               | 332        | 5.8      | 3909.85802(2)              |                          |                         |                          |                          |                         |
| 738   | $E$               | 295        | 3.9      | 3912.90610(2)              |                          |                         |                          |                          |                         |
| 739   | $E$               | 298        | 3.9      | 3912.90610(2)              |                          |                         |                          |                          |                         |
| 740   | $A_1$             | 325        | 5.5      | 3914.49338(3)              |                          |                         |                          |                          |                         |
| 741   | $A_2$             | 322        | 5.8      | 3915.04928(3)              |                          |                         |                          |                          |                         |
| 742   | $E$               | 240        | 3.6      | 3917.92541(6)              |                          |                         |                          |                          |                         |
| 743   | $E$               | 254        | 3.6      | 3917.92541(4)              |                          |                         |                          |                          |                         |
| 744   | $E$               | 245        | 5.2      | 3919.85724(6)              |                          |                         |                          |                          |                         |
| 745   | $E$               | 244        | 5.2      | 3919.85724(6)              |                          |                         |                          |                          |                         |
| 746   | $E$               | 226        | 3.8      | 3938.90669(7)              |                          |                         |                          |                          |                         |
| 747   | $E$               | 264        | 3.8      | 3938.90669(3)              |                          |                         |                          |                          |                         |
| 748   | $E$               | 271        | 4.2      | 3942.38830(5)              |                          |                         |                          |                          |                         |
| 749   | $E$               | 285        | 4.2      | 3942.38830(4)              |                          |                         |                          |                          |                         |
| 750   | $A_1$             | 181        | 4.3      | 3944.7868(3)               |                          |                         |                          |                          |                         |
| 751   | $A_2$             | 177        | 4.3      | 3944.7906(3)               |                          |                         |                          |                          |                         |
| 752   | $E$               | 243        | 4.3      | 3946.02069(5)              |                          |                         |                          |                          |                         |
| 753   | $E$               | 269        | 4.3      | 3946.02069(3)              |                          |                         |                          |                          |                         |
| 754   | $A_2$             | 174        | 1.4      | 3947.97272(6)              |                          |                         |                          |                          |                         |
| 755   | $A_1$             | 254        | 1.4      | 3947.97272(1)              |                          |                         |                          |                          |                         |
| 756   | $E$               | 192        | 2.7      | 3948.66996(6)              |                          |                         |                          |                          |                         |
| 757   | $E$               | 189        | 2.7      | 3948.66996(6)              |                          |                         |                          |                          |                         |
| 758   | $E$               | 146        | 3.2      | 3949.0883(1)               |                          |                         |                          |                          |                         |
| 759   | $E$               | 184        | 3.2      | 3949.0884(1)               |                          |                         |                          |                          |                         |

Continued on next page.

TABLE S2 – States on Avila/Carrington AC PES; continued from previous page.

| State | $\Gamma_{C_{3v}}$ | $D_{\max}$ | $S_{vN}$ | $\tilde{E}/\text{cm}^{-1}$ | $\Delta\text{Ref. [11]}$ | $\Delta\text{Ref. [9]}$ | $\Delta\text{Ref. [34]}$ | $\Delta\text{Ref. [35]}$ | $\Delta\text{Ref. [1]}$ |
|-------|-------------------|------------|----------|----------------------------|--------------------------|-------------------------|--------------------------|--------------------------|-------------------------|
| 760   | $A_1$             | 146        | 3.4      | 3949.2279(2)               |                          |                         |                          |                          |                         |
| 761   | $E$               | 202        | 1.6      | 3950.45168(2)              |                          |                         |                          |                          |                         |
| 762   | $E$               | 203        | 1.6      | 3950.45168(2)              |                          |                         |                          |                          |                         |
| 763   | $A_2$             | 171        | 2.6      | 3950.6918(2)               |                          |                         |                          |                          |                         |
| 764   | $A_1$             | 170        | 2.6      | 3950.6918(2)               |                          |                         |                          |                          |                         |
| 765   | $E$               | 304        | 4.2      | 3952.88063(5)              |                          |                         |                          |                          |                         |
| 766   | $E$               | 311        | 4.2      | 3952.88063(5)              |                          |                         |                          |                          |                         |
| 767   | $E$               | 261        | 4.3      | 3954.44369(7)              |                          |                         |                          |                          |                         |
| 768   | $E$               | 268        | 4.3      | 3954.44369(6)              |                          |                         |                          |                          |                         |
| 769   | $E$               | 314        | 4.8      | 3954.60733(6)              |                          |                         |                          |                          |                         |
| 770   | $E$               | 313        | 4.8      | 3954.60733(6)              |                          |                         |                          |                          |                         |
| 771   | $A_1$             | 194        | 5.2      | 3955.8089(4)               |                          |                         |                          |                          |                         |
| 772   | $A_2$             | 215        | 5.2      | 3955.8252(3)               |                          |                         |                          |                          |                         |
| 773   | $E$               | 311        | 4.5      | 3956.06365(4)              |                          |                         |                          |                          |                         |
| 774   | $E$               | 378        | 4.5      | 3956.06365(1)              |                          |                         |                          |                          |                         |
| 775   | $E$               | 357        | 4.9      | 3956.46318(3)              |                          |                         |                          |                          |                         |
| 776   | $E$               | 293        | 4.9      | 3956.46318(3)              |                          |                         |                          |                          |                         |
| 777   | $A_1$             | 194        | 4.3      | 3957.0011(4)               |                          |                         |                          |                          |                         |
| 778   | $A_2$             | 203        | 4.3      | 3957.0027(3)               |                          |                         |                          |                          |                         |
| 779   | $E$               | 286        | 3.4      | 3957.39658(3)              |                          |                         |                          |                          |                         |
| 780   | $E$               | 344        | 3.3      | 3957.39658(1)              |                          |                         |                          |                          |                         |
| 781   | $E$               | 292        | 5.5      | 3958.8656(1)               |                          |                         |                          |                          |                         |
| 782   | $E$               | 329        | 5.5      | 3958.86561(9)              |                          |                         |                          |                          |                         |
| 783   | $E$               | 407        | 5.2      | 3959.40237(2)              |                          |                         |                          |                          |                         |
| 784   | $E$               | 321        | 5.2      | 3959.40238(7)              |                          |                         |                          |                          |                         |
| 785   | $A_2$             | 331        | 5.4      | 3960.48560(4)              |                          |                         |                          |                          |                         |
| 786   | $E$               | 349        | 5.5      | 3960.78212(5)              |                          |                         |                          |                          |                         |
| 787   | $E$               | 351        | 5.5      | 3960.78212(5)              |                          |                         |                          |                          |                         |
| 788   | $A_1$             | 329        | 5.4      | 3961.32103(4)              |                          |                         |                          |                          |                         |
| 789   | $E$               | 243        | 1.1      | 3967.32354(3)              |                          |                         |                          |                          |                         |
| 790   | $E$               | 245        | 1.1      | 3967.32354(3)              |                          |                         |                          |                          |                         |
| 791   | $E$               | 381        | 4.0      | 3969.40092(2)              |                          |                         |                          |                          |                         |
| 792   | $E$               | 374        | 4.0      | 3969.40092(2)              |                          |                         |                          |                          |                         |
| 793   | $E$               | 406        | 4.5      | 3970.97720(2)              |                          |                         |                          |                          |                         |
| 794   | $E$               | 333        | 4.5      | 3970.97721(7)              |                          |                         |                          |                          |                         |
| 795   | $A_1$             | 219        | 3.8      | 3971.5115(2)               |                          |                         |                          |                          |                         |
| 796   | $A_2$             | 214        | 3.6      | 3971.5138(2)               |                          |                         |                          |                          |                         |
| 797   | $A_1$             | 319        | 4.4      | 3971.56683(5)              |                          |                         |                          |                          |                         |
| 798   | $E$               | 329        | 5.7      | 3971.79129(8)              |                          |                         |                          |                          |                         |
| 799   | $E$               | 324        | 5.6      | 3971.79129(8)              |                          |                         |                          |                          |                         |
| 800   | $E$               | 320        | 5.2      | 3972.43982(8)              |                          |                         |                          |                          |                         |
| 801   | $E$               | 369        | 5.2      | 3972.43982(4)              |                          |                         |                          |                          |                         |
| 802   | $A_2$             | 361        | 4.3      | 3972.57544(2)              |                          |                         |                          |                          |                         |
| 803   | $E$               | 329        | 5.0      | 3973.61362(9)              |                          |                         |                          |                          |                         |
| 804   | $E$               | 344        | 5.0      | 3973.61362(7)              |                          |                         |                          |                          |                         |
| 805   | $E$               | 402        | 5.5      | 3974.51602(2)              |                          |                         |                          |                          |                         |
| 806   | $E$               | 404        | 5.5      | 3974.51602(2)              |                          |                         |                          |                          |                         |
| 807   | $E$               | 321        | 5.1      | 3974.88612(7)              |                          |                         |                          |                          |                         |
| 808   | $E$               | 316        | 5.1      | 3974.88612(8)              |                          |                         |                          |                          |                         |
| 809   | $A_2$             | 305        | 5.4      | 3975.00477(9)              |                          |                         |                          |                          |                         |
| 810   | $A_1$             | 307        | 5.9      | 3975.3046(1)               |                          |                         |                          |                          |                         |
| 811   | $E$               | 208        | 2.9      | 3981.22481(2)              |                          |                         |                          |                          |                         |
| 812   | $E$               | 209        | 2.9      | 3981.22481(2)              |                          |                         |                          |                          |                         |
| 813   | $A_1$             | 243        | 0.68     | 3983.33459(3)              |                          |                         |                          |                          |                         |
| 814   | $A_2$             | 232        | 0.51     | 3984.49467(3)              |                          |                         |                          |                          |                         |
| 815   | $A_1$             | 176        | 2.9      | 3985.5663(3)               |                          |                         |                          |                          |                         |
| 816   | $A_2$             | 178        | 2.9      | 3985.5757(2)               |                          |                         |                          |                          |                         |
| 817   | $E$               | 218        | 2.9      | 3985.72959(8)              |                          |                         |                          |                          |                         |
| 818   | $E$               | 213        | 2.8      | 3985.72959(9)              |                          |                         |                          |                          |                         |

Continued on next page.

TABLE S2 – States on Avila/Carrington AC PES; continued from previous page.

| State | $\Gamma_{C_{3v}}$ | $D_{\max}$ | $S_{vN}$ | $\tilde{E}/\text{cm}^{-1}$ | $\Delta\text{Ref. [11]}$ | $\Delta\text{Ref. [9]}$ | $\Delta\text{Ref. [34]}$ | $\Delta\text{Ref. [35]}$ | $\Delta\text{Ref. [1]}$ |
|-------|-------------------|------------|----------|----------------------------|--------------------------|-------------------------|--------------------------|--------------------------|-------------------------|
| 819   | $E$               | 233        | 2.5      | 3986.37717(7)              |                          |                         |                          |                          |                         |
| 820   | $E$               | 233        | 2.5      | 3986.37717(7)              |                          |                         |                          |                          |                         |
| 821   | $E$               | 223        | 6.1      | 3990.9039(1)               |                          |                         |                          |                          |                         |
| 822   | $E$               | 233        | 6.1      | 3990.90387(9)              |                          |                         |                          |                          |                         |
| 823   | $A_1$             | 244        | 4.0      | 3997.2610(1)               |                          |                         |                          |                          |                         |
| 824   | $A_2$             | 234        | 4.0      | 3997.2613(1)               |                          |                         |                          |                          |                         |
| 825   | $E$               | 322        | 3.3      | 3997.84976(2)              |                          |                         |                          |                          |                         |
| 826   | $E$               | 316        | 3.3      | 3997.84976(2)              |                          |                         |                          |                          |                         |
| 827   | $E$               | 234        | 6.1      | 4000.93393(8)              |                          |                         |                          |                          |                         |
| 828   | $E$               | 245        | 6.1      | 4000.93393(6)              |                          |                         |                          |                          |                         |
| 829   | $E$               | 255        | 2.7      | 4005.89745(3)              |                          |                         |                          |                          |                         |
| 830   | $E$               | 254        | 2.7      | 4005.89745(3)              |                          |                         |                          |                          |                         |
| 831   | $A_2$             | 173        | 2.6      | 4010.71296(5)              |                          |                         |                          |                          |                         |
| 832   | $A_1$             | 255        | 2.8      | 4011.14436(3)              |                          |                         |                          |                          |                         |
| 833   | $A_1$             | 167        | 4.2      | 4011.34338(8)              |                          |                         |                          |                          |                         |
| 834   | $E$               | 210        | 2.4      | 4015.39943(3)              |                          |                         |                          |                          |                         |
| 835   | $E$               | 205        | 2.4      | 4015.39943(2)              |                          |                         |                          |                          |                         |
| 836   | $E$               | 356        | 5.5      | 4026.51270(5)              |                          |                         |                          |                          |                         |
| 837   | $E$               | 373        | 5.5      | 4026.51271(4)              |                          |                         |                          |                          |                         |
| 838   | $A_1$             | 359        | 3.0      | 4026.70588(4)              |                          |                         |                          |                          |                         |
| 839   | $A_2$             | 356        | 2.9      | 4026.71090(4)              |                          |                         |                          |                          |                         |
| 840   | $A_1$             | 265        | 4.0      | 4027.69747(5)              |                          |                         |                          |                          |                         |
| 841   | $A_2$             | 283        | 3.3      | 4028.38540(2)              |                          |                         |                          |                          |                         |
| 842   | $E$               | 265        | 3.4      | 4028.41062(5)              |                          |                         |                          |                          |                         |
| 843   | $E$               | 281        | 3.4      | 4028.41062(3)              |                          |                         |                          |                          |                         |
| 844   | $E$               | 368        | 7.6      | 4030.87116(8)              |                          |                         |                          |                          |                         |
| 845   | $E$               | 364        | 7.6      | 4030.87116(8)              |                          |                         |                          |                          |                         |
| 846   | $E$               | 358        | 6.7      | 4033.81776(7)              |                          |                         |                          |                          |                         |
| 847   | $E$               | 344        | 6.7      | 4033.81776(9)              |                          |                         |                          |                          |                         |
| 848   | $E$               | 228        | 0.19     | 4034.35034(3)              |                          |                         |                          |                          |                         |
| 849   | $E$               | 230        | 0.19     | 4034.35034(3)              |                          |                         |                          |                          |                         |
| 850   | $A_2$             | 353        | 2.9      | 4034.47611(2)              |                          |                         |                          |                          |                         |
| 851   | $A_1$             | 288        | 2.9      | 4034.47619(5)              |                          |                         |                          |                          |                         |
| 852   | $E$               | 208        | 2.2      | 4035.49933(9)              |                          |                         |                          |                          |                         |
| 853   | $E$               | 203        | 2.2      | 4035.4993(1)               |                          |                         |                          |                          |                         |
| 854   | $E$               | 272        | 2.9      | 4035.70877(4)              |                          |                         |                          |                          |                         |
| 855   | $E$               | 272        | 2.9      | 4035.70877(4)              |                          |                         |                          |                          |                         |
| 856   | $A_1$             | 263        | 6.1      | 4036.1943(5)               |                          |                         |                          |                          |                         |
| 857   | $A_2$             | 266        | 6.1      | 4036.2313(4)               |                          |                         |                          |                          |                         |
| 858   | $A_1$             | 296        | 2.9      | 4036.33418(4)              |                          |                         |                          |                          |                         |
| 859   | $A_2$             | 291        | 2.9      | 4036.33419(4)              |                          |                         |                          |                          |                         |
| 860   | $E$               | 310        | 3.1      | 4037.0381(1)               |                          |                         |                          |                          |                         |
| 861   | $E$               | 338        | 3.1      | 4037.03812(7)              |                          |                         |                          |                          |                         |
| 862   | $A_1^*$           | 174        | 1.5      | 4037.2716(2)               |                          |                         |                          |                          |                         |
| 863   | $A_2^*$           | 170        | 1.5      | 4037.2716(3)               |                          |                         |                          |                          |                         |
| 864   | $E^-$             | 366        | 6.7      | 4037.37339(5)              |                          |                         |                          |                          |                         |
| 865   | $E$               | 340        | 6.7      | 4037.37339(7)              |                          |                         |                          |                          |                         |
| 866   | $A_2$             | 375        | 2.7      | 4038.51341(2)              |                          |                         |                          |                          |                         |
| 867   | $A_1$             | 331        | 2.8      | 4038.51353(3)              |                          |                         |                          |                          |                         |
| 868   | $E$               | 263        | 3.4      | 4038.7465(1)               |                          |                         |                          |                          |                         |
| 869   | $E$               | 369        | 3.3      | 4038.74652(9)              |                          |                         |                          |                          |                         |
| 870   | $E$               | 322        | 2.1      | 4039.57103(2)              |                          |                         |                          |                          |                         |
| 871   | $E$               | 337        | 2.1      | 4039.57103(2)              |                          |                         |                          |                          |                         |
| 872   | $E$               | 260        | 3.3      | 4040.2322(1)               |                          |                         |                          |                          |                         |
| 873   | $E$               | 271        | 3.3      | 4040.23217(9)              |                          |                         |                          |                          |                         |
| 874   | $E$               | 371        | 3.1      | 4040.64564(2)              |                          |                         |                          |                          |                         |
| 875   | $E$               | 294        | 3.1      | 4040.64565(8)              |                          |                         |                          |                          |                         |
| 876   | $A_2$             | 344        | 3.2      | 4040.73584(2)              |                          |                         |                          |                          |                         |
| 877   | $E$               | 321        | 2.3      | 4041.25452(2)              |                          |                         |                          |                          |                         |

Continued on next page.

TABLE S2 – States on Avila/Carrington AC PES; continued from previous page.

| State | $\Gamma_{C_{3v}}$ | $D_{\max}$ | $S_{vN}$ | $\tilde{E}/\text{cm}^{-1}$ | $\Delta\text{Ref. [11]}$ | $\Delta\text{Ref. [9]}$ | $\Delta\text{Ref. [34]}$ | $\Delta\text{Ref. [35]}$ | $\Delta\text{Ref. [1]}$ |
|-------|-------------------|------------|----------|----------------------------|--------------------------|-------------------------|--------------------------|--------------------------|-------------------------|
| 878   | $E$               | 236        | 2.3      | 4041.25453(6)              |                          |                         |                          |                          |                         |
| 879   | $A_1$             | 307        | 6.4      | 4041.2971(2)               |                          |                         |                          |                          |                         |
| 880   | $A_2$             | 391        | 6.4      | 4041.31144(5)              |                          |                         |                          |                          |                         |
| 881   | $E$               | 257        | 3.4      | 4041.9146(1)               |                          |                         |                          |                          |                         |
| 882   | $E$               | 274        | 3.4      | 4041.91465(9)              |                          |                         |                          |                          |                         |
| 883   | $A_1$             | 251        | 4.5      | 4042.1957(1)               |                          |                         |                          |                          |                         |
| 884   | $A_2$             | 251        | 2.0      | 4042.40913(4)              |                          |                         |                          |                          |                         |
| 885   | $A_1$             | 264        | 4.3      | 4042.51094(9)              |                          |                         |                          |                          |                         |
| 886   | $E$               | 211        | 2.0      | 4042.96983(3)              |                          |                         |                          |                          |                         |
| 887   | $E$               | 199        | 2.0      | 4042.96984(4)              |                          |                         |                          |                          |                         |
| 888   | $E$               | 328        | 5.7      | 4043.05177(9)              |                          |                         |                          |                          |                         |
| 889   | $E$               | 281        | 5.7      | 4043.0518(2)               |                          |                         |                          |                          |                         |
| 890   | $E$               | 274        | 7.2      | 4045.6685(2)               |                          |                         |                          |                          |                         |
| 891   | $E$               | 273        | 7.2      | 4045.6685(2)               |                          |                         |                          |                          |                         |
| 892   | $A_1$             | 155        | 3.7      | 4054.69079(3)              |                          |                         |                          |                          |                         |
| 893   | $E$               | 273        | 2.7      | 4055.04309(3)              |                          |                         |                          |                          |                         |
| 894   | $E$               | 311        | 2.7      | 4055.04309(1)              |                          |                         |                          |                          |                         |
| 895   | $E$               | 243        | 1.9      | 4055.16791(2)              |                          |                         |                          |                          |                         |
| 896   | $E$               | 218        | 1.9      | 4055.16791(3)              |                          |                         |                          |                          |                         |
| 897   | $E$               | 290        | 2.7      | 4055.89290(3)              |                          |                         |                          |                          |                         |
| 898   | $E$               | 267        | 2.7      | 4055.89290(5)              |                          |                         |                          |                          |                         |
| 899   | $A_1$             | 266        | 2.7      | 4056.50642(3)              |                          |                         |                          |                          |                         |
| 900   | $A_2$             | 265        | 2.7      | 4056.56060(3)              |                          |                         |                          |                          |                         |
| 901   | $E$               | 280        | 2.8      | 4056.81740(3)              |                          |                         |                          |                          |                         |
| 902   | $E$               | 261        | 2.8      | 4056.81740(4)              |                          |                         |                          |                          |                         |
| 903   | $A_1$             | 241        | 1.9      | 4057.28711(2)              |                          |                         |                          |                          |                         |
| 904   | $A_2$             | 232        | 1.9      | 4057.28832(4)              |                          |                         |                          |                          |                         |
| 905   | $E$               | 224        | 2.0      | 4058.34969(3)              |                          |                         |                          |                          |                         |
| 906   | $E$               | 264        | 2.0      | 4058.34970(1)              |                          |                         |                          |                          |                         |
| 907   | $A_1$             | 172        | 2.4      | 4067.5878(1)               |                          |                         |                          |                          |                         |
| 908   | $A_2$             | 178        | 2.4      | 4067.58883(8)              |                          |                         |                          |                          |                         |
| 909   | $E$               | 227        | 2.7      | 4068.80841(5)              |                          |                         |                          |                          |                         |
| 910   | $E$               | 233        | 2.7      | 4068.80841(4)              |                          |                         |                          |                          |                         |
| 911   | $A_2$             | 217        | 2.5      | 4069.27793(3)              |                          |                         |                          |                          |                         |
| 912   | $E$               | 231        | 3.2      | 4070.28938(3)              |                          |                         |                          |                          |                         |
| 913   | $E$               | 250        | 3.2      | 4070.28938(3)              |                          |                         |                          |                          |                         |
| 914   | $A_1$             | 238        | 3.6      | 4072.28555(3)              |                          |                         |                          |                          |                         |
| 915   | $A_1$             | 182        | 3.2      | 4081.19541(5)              |                          |                         |                          |                          |                         |
| 916   | $E$               | 134        | 3.0      | 4081.2141(1)               |                          |                         |                          |                          |                         |
| 917   | $E$               | 215        | 3.0      | 4081.2141(1)               |                          |                         |                          |                          |                         |
| 918   | $E$               | 257        | 1.8      | 4081.29391(2)              |                          |                         |                          |                          |                         |
| 919   | $E$               | 234        | 1.8      | 4081.29391(2)              |                          |                         |                          |                          |                         |
| 920   | $A_1$             | 210        | 2.4      | 4087.54567(4)              |                          |                         |                          |                          |                         |
| 921   | $A_2$             | 221        | 3.5      | 4089.81345(3)              |                          |                         |                          |                          |                         |
| 922   | $E$               | 228        | 3.5      | 4089.91784(3)              |                          |                         |                          |                          |                         |
| 923   | $E$               | 223        | 3.5      | 4089.91785(4)              |                          |                         |                          |                          |                         |
| 924   | $A_1$             | 230        | 3.5      | 4090.25199(2)              |                          |                         |                          |                          |                         |
| 925   | $E$               | 223        | 1.2      | 4094.1627(3)               |                          |                         |                          |                          |                         |
| 926   | $E$               | 233        | 1.2      | 4094.16275(2)              |                          |                         |                          |                          |                         |
| 927   | $E$               | 251        | 5.2      | 4095.3667(2)               |                          |                         |                          |                          |                         |
| 928   | $E$               | 262        | 5.2      | 4095.3667(1)               |                          |                         |                          |                          |                         |
| 929   | $A_1$             | 236        | 5.9      | 4097.5690(2)               |                          |                         |                          |                          |                         |
| 930   | $A_2$             | 228        | 5.9      | 4097.5731(3)               |                          |                         |                          |                          |                         |
| 931   | $E$               | 294        | 6.0      | 4098.70564(7)              |                          |                         |                          |                          |                         |
| 932   | $E$               | 291        | 6.0      | 4098.70564(7)              |                          |                         |                          |                          |                         |
| 933   | $E$               | 361        | 3.2      | 4101.24136(2)              |                          |                         |                          |                          |                         |
| 934   | $E$               | 295        | 3.2      | 4101.24136(5)              |                          |                         |                          |                          |                         |
| 935   | $E$               | 382        | 4.4      | 4102.63917(3)              |                          |                         |                          |                          |                         |
| 936   | $E$               | 279        | 4.4      | 4102.6392(1)               |                          |                         |                          |                          |                         |

Continued on next page.

TABLE S2 – States on Avila/Carrington AC PES; continued from previous page.

| State | $\Gamma_{C_{3v}}$ | $D_{\max}$ | $S_{vN}$ | $\tilde{E}/\text{cm}^{-1}$ | $\Delta\text{Ref. [11]}$ | $\Delta\text{Ref. [9]}$ | $\Delta\text{Ref. [34]}$ | $\Delta\text{Ref. [35]}$ | $\Delta\text{Ref. [1]}$ |
|-------|-------------------|------------|----------|----------------------------|--------------------------|-------------------------|--------------------------|--------------------------|-------------------------|
| 937   | $A_1$             | 386        | 4.7      | 4103.66151(3)              |                          |                         |                          |                          |                         |
| 938   | $A_2$             | 299        | 4.7      | 4103.6780(1)               |                          |                         |                          |                          |                         |
| 939   | $E$               | 357        | 3.8      | 4104.26566(2)              |                          |                         |                          |                          |                         |
| 940   | $E$               | 271        | 3.8      | 4104.26567(8)              |                          |                         |                          |                          |                         |
| 941   | $E$               | 265        | 4.8      | 4106.5994(5)               |                          |                         |                          |                          |                         |
| 942   | $E$               | 281        | 4.8      | 4106.59936(5)              |                          |                         |                          |                          |                         |
| 943   | $A_1$             | 220        | 5.5      | 4107.0313(3)               |                          |                         |                          |                          |                         |
| 944   | $A_2$             | 206        | 5.5      | 4107.0331(4)               |                          |                         |                          |                          |                         |
| 945   | $E$               | 269        | 5.6      | 4107.13144(8)              |                          |                         |                          |                          |                         |
| 946   | $E$               | 214        | 5.6      | 4107.1315(2)               |                          |                         |                          |                          |                         |
| 947   | $E$               | 229        | 0.45     | 4118.48606(3)              |                          |                         |                          |                          |                         |
| 948   | $E$               | 241        | 0.45     | 4118.48606(3)              |                          |                         |                          |                          |                         |
| 949   | $E$               | 279        | 6.7      | 4132.6466(2)               |                          |                         |                          |                          |                         |
| 950   | $E$               | 357        | 6.7      | 4132.6466(1)               |                          |                         |                          |                          |                         |
| 951   | $A_2$             | 295        | 6.9      | 4133.2116(1)               |                          |                         |                          |                          |                         |
| 952   | $A_1$             | 344        | 8.0      | 4133.53440(8)              |                          |                         |                          |                          |                         |
| 953   | $A_1$             | 305        | 5.1      | 4134.17003(7)              |                          |                         |                          |                          |                         |
| 954   | $E$               | 356        | 3.2      | 4135.87409(2)              |                          |                         |                          |                          |                         |
| 955   | $E$               | 260        | 3.2      | 4135.87410(8)              |                          |                         |                          |                          |                         |
| 956   | $E$               | 305        | 7.9      | 4136.1077(1)               |                          |                         |                          |                          |                         |
| 957   | $E$               | 345        | 7.9      | 4136.10770(9)              |                          |                         |                          |                          |                         |
| 958   | $E$               | 306        | 8.3      | 4136.5364(1)               |                          |                         |                          |                          |                         |
| 959   | $E$               | 311        | 8.3      | 4136.5364(1)               |                          |                         |                          |                          |                         |
| 960   | $E$               | 270        | 0.97     | 4136.73592(3)              |                          |                         |                          |                          |                         |
| 961   | $E$               | 247        | 0.95     | 4136.73592(2)              |                          |                         |                          |                          |                         |
| 962   | $A_1$             | 299        | 7.6      | 4137.1585(1)               |                          |                         |                          |                          |                         |
| 963   | $E$               | 273        | 4.2      | 4137.3165(1)               |                          |                         |                          |                          |                         |
| 964   | $E$               | 306        | 4.1      | 4137.31648(8)              |                          |                         |                          |                          |                         |
| 965   | $A_1$             | 237        | 6.4      | 4137.4162(4)               |                          |                         |                          |                          |                         |
| 966   | $A_2$             | 244        | 5.1      | 4137.4277(3)               |                          |                         |                          |                          |                         |
| 967   | $A_2$             | 317        | 6.6      | 4138.1738(1)               |                          |                         |                          |                          |                         |
| 968   | $E$               | 387        | 5.2      | 4138.64374(3)              |                          |                         |                          |                          |                         |
| 969   | $E$               | 380        | 5.3      | 4138.64374(3)              |                          |                         |                          |                          |                         |
| 970   | $E$               | 309        | 4.3      | 4138.72353(9)              |                          |                         |                          |                          |                         |
| 971   | $E$               | 391        | 4.4      | 4138.72354(5)              |                          |                         |                          |                          |                         |
| 972   | $E$               | 317        | 6.6      | 4141.93436(8)              |                          |                         |                          |                          |                         |
| 973   | $E$               | 328        | 6.6      | 4141.93436(7)              |                          |                         |                          |                          |                         |
| 974   | $A_2$             | 323        | 6.6      | 4142.34970(7)              |                          |                         |                          |                          |                         |
| 975   | $A_1$             | 335        | 6.6      | 4142.68303(6)              |                          |                         |                          |                          |                         |
| 976   | $E$               | 317        | 7.0      | 4147.8083(1)               |                          |                         |                          |                          |                         |
| 977   | $E$               | 324        | 7.0      | 4147.8084(1)               |                          |                         |                          |                          |                         |
| 978   | $A_1$             | 321        | 8.3      | 4148.2123(1)               |                          |                         |                          |                          |                         |
| 979   | $A_2$             | 373        | 6.0      | 4149.54441(2)              |                          |                         |                          |                          |                         |
| 980   | $E$               | 337        | 7.0      | 4154.91672(7)              |                          |                         |                          |                          |                         |
| 981   | $E$               | 378        | 7.0      | 4154.91674(5)              |                          |                         |                          |                          |                         |
| 982   | $A_1$             | 293        | 8.0      | 4155.0260(2)               |                          |                         |                          |                          |                         |
| 983   | $E$               | 391        | 4.7      | 4157.26618(2)              |                          |                         |                          |                          |                         |
| 984   | $E$               | 442        | 4.7      | 4157.26618(1)              |                          |                         |                          |                          |                         |
| 985   | $E$               | 377        | 4.9      | 4159.43864(4)              |                          |                         |                          |                          |                         |
| 986   | $E$               | 352        | 4.9      | 4159.43864(6)              |                          |                         |                          |                          |                         |
| 987   | $A_2$             | 350        | 4.8      | 4160.59090(6)              |                          |                         |                          |                          |                         |
| 988   | $A_1$             | 360        | 7.5      | 4162.88645(7)              |                          |                         |                          |                          |                         |
| 989   | $E$               | 366        | 6.1      | 4164.86063(7)              |                          |                         |                          |                          |                         |
| 990   | $E$               | 385        | 6.1      | 4164.86063(4)              |                          |                         |                          |                          |                         |
| 991   | $A_2$             | 363        | 7.7      | 4165.42752(7)              |                          |                         |                          |                          |                         |
| 992   | $E$               | 295        | 3.5      | 4165.87216(2)              |                          |                         |                          |                          |                         |
| 993   | $E$               | 290        | 3.5      | 4165.87216(2)              |                          |                         |                          |                          |                         |
| 994   | $E$               | 332        | 5.9      | 4166.9102(1)               |                          |                         |                          |                          |                         |
| 995   | $E$               | 302        | 5.9      | 4166.9103(1)               |                          |                         |                          |                          |                         |

Continued on next page.



TABLE S2 – States on Avila/Carrington AC PES; continued from previous page.

| State | $\Gamma_{C_{3v}}$ | $D_{\max}$ | $S_{vN}$ | $\tilde{E}/\text{cm}^{-1}$ | $\Delta\text{Ref. [11]}$ | $\Delta\text{Ref. [9]}$ | $\Delta\text{Ref. [34]}$ | $\Delta\text{Ref. [35]}$ | $\Delta\text{Ref. [1]}$ |
|-------|-------------------|------------|----------|----------------------------|--------------------------|-------------------------|--------------------------|--------------------------|-------------------------|
| 996   | $A_1$             | 282        | 8.0      | 4167.4886(1)               |                          |                         |                          |                          |                         |
| 997   | $E$               | 250        | 7.3      | 4167.4936(4)               |                          |                         |                          |                          |                         |
| 998   | $E$               | 305        | 7.3      | 4167.4936(2)               |                          |                         |                          |                          |                         |
| 999   | $A_2$             | 369        | 2.9      | 4175.78635(2)              |                          |                         |                          |                          |                         |

TABLE S3: Same as Table S2 but for the USC PES variant from Sarka and Poirier.

| State | $\Gamma_{C_{3v}}$ | $D_{\max}$ | $S_{vN}$ | $\tilde{E}/\text{cm}^{-1}$ | $\Delta\text{Ref. [30]}$ |
|-------|-------------------|------------|----------|----------------------------|--------------------------|
| 0     | $A_1$             | 75         | 0.053    | 9836.852699(6)             | −0.029                   |
| 1     | $E$               | 82         | 0.057    | 361.001402(5)              | −0.001                   |
| 2     | $E$               | 82         | 0.057    | 361.001403(5)              | −0.001                   |
| 3     | $E$               | 88         | 0.064    | 723.20616(1)               | −0.001                   |
| 4     | $E$               | 87         | 0.064    | 723.20616(1)               | −0.001                   |
| 5     | $A_1$             | 86         | 0.14     | 723.85771(1)               | −0.001                   |
| 6     | $A_1$             | 88         | 0.17     | 900.66522(1)               | −0.002                   |
| 7     | $E$               | 98         | 0.093    | 1033.577242(8)             | −0.003                   |
| 8     | $E$               | 96         | 0.094    | 1033.577243(9)             | −0.004                   |
| 9     | $A_1$             | 93         | 0.071    | 1086.59826(1)              | −0.002                   |
| 10    | $A_2$             | 90         | 0.071    | 1086.59858(1)              | −0.002                   |
| 11    | $E$               | 92         | 0.22     | 1087.83174(1)              | −0.001                   |
| 12    | $E$               | 92         | 0.22     | 1087.831742(7)             | −0.003                   |
| 13    | $E$               | 92         | 0.26     | 1259.83201(1)              | −0.004                   |
| 14    | $E$               | 92         | 0.26     | 1259.83201(1)              | −0.004                   |
| 15    | $A_1$             | 137        | 4.0      | 1388.721837(8)             | −0.039                   |
| 16    | $E$               | 140        | 2.1      | 1394.16149(1)              | −0.005                   |
| 17    | $E$               | 162        | 2.1      | 1394.16150(1)              | −0.027                   |
| 18    | $A_2$             | 128        | 2.1      | 1394.39400(1)              | −0.004                   |
| 19    | $A_1$             | 125        | 4.2      | 1397.39020(3)              | −0.037                   |
| 20    | $E$               | 93         | 0.08     | 1451.16273(3)              | −0.003                   |
| 21    | $E$               | 96         | 0.08     | 1451.16273(2)              | −0.020                   |
| 22    | $E$               | 98         | 0.3      | 1452.90497(2)              | −0.003                   |
| 23    | $E$               | 97         | 0.3      | 1452.90497(3)              | −0.069                   |
| 24    | $A_1$             | 98         | 0.36     | 1453.48615(3)              | −0.066                   |
| 25    | $E$               | 101        | 0.14     | 1481.677027(9)             | −0.003                   |
| 26    | $E$               | 100        | 0.14     | 1481.67703(1)              | −0.145                   |
| 27    | $E$               | 98         | 0.34     | 1620.24228(5)              | −0.006                   |
| 28    | $E$               | 99         | 0.34     | 1620.24228(4)              | −0.086                   |
| 29    | $A_1$             | 101        | 0.57     | 1620.79205(4)              | −0.118                   |
| 30    | $E$               | 148        | 3.9      | 1749.299275(8)             | −0.039                   |
| 31    | $E$               | 154        | 3.9      | 1749.29928(1)              | −0.168                   |
| 32    | $A_2$             | 170        | 2.2      | 1755.93223(1)              | −0.028                   |
| 33    | $A_1$             | 162        | 2.2      | 1755.93263(2)              | −0.053                   |
| 34    | $E$               | 210        | 1.5      | 1756.679427(5)             | −0.014                   |
| 35    | $E$               | 184        | 1.5      | 1756.67943(1)              | −0.026                   |
| 36    | $E$               | 147        | 4.1      | 1759.47961(2)              | −0.032                   |
| 37    | $E$               | 148        | 4.1      | 1759.47961(1)              | −0.162                   |
| 38    | $A_1$             | 94         | 0.41     | 1785.11325(2)              | −0.198                   |
| 39    | $E$               | 94         | 0.091    | 1816.88397(5)              | −0.016                   |
| 40    | $E$               | 104        | 0.091    | 1816.88397(4)              | −0.051                   |
| 41    | $A_1$             | 104        | 0.39     | 1819.05826(5)              | −0.058                   |
| 42    | $A_2$             | 116        | 0.39     | 1819.05967(3)              | −0.090                   |
| 43    | $E$               | 105        | 0.5      | 1820.14756(3)              | −0.024                   |
| 44    | $E$               | 102        | 0.5      | 1820.14756(5)              | −0.133                   |
| 45    | $A_2$             | 139        | 2.2      | 1842.72206(1)              | −0.031                   |
| 46    | $E$               | 146        | 2.1      | 1842.78988(1)              | −0.076                   |
| 47    | $E$               | 145        | 2.1      | 1842.78989(1)              | −0.126                   |

Continued on next page.

TABLE S3 – States on Sarka/Poirier USC PES; continued from previous page.

| State | $\Gamma_{C_{3v}}$ | $D_{\max}$ | $S_{vN}$ | $\tilde{E}/\text{cm}^{-1}$ | $\Delta\text{Ref. [30]}$ |
|-------|-------------------|------------|----------|----------------------------|--------------------------|
| 48    | $A_1$             | 139        | 2.2      | 1843.14864(1)              | −0.126                   |
| 49    | $E$               | 122        | 0.26     | 1930.985015(6)             | −0.008                   |
| 50    | $E$               | 121        | 0.26     | 1930.985017(8)             | −0.201                   |
| 51    | $A_1$             | 137        | 0.43     | 1981.88323(2)              | −0.050                   |
| 52    | $A_2$             | 106        | 0.43     | 1981.88372(6)              | −0.147                   |
| 53    | $E$               | 107        | 0.84     | 1982.89560(5)              | −0.067                   |
| 54    | $E$               | 106        | 0.84     | 1982.89560(6)              | −0.158                   |
| 55    | $A_1$             | 134        | 0.22     | 2055.97326(1)              | −0.105                   |
| 56    | $E$               | 128        | 0.18     | 2064.18564(1)              | −0.010                   |
| 57    | $E$               | 125        | 0.18     | 2064.18564(1)              | −0.108                   |
| 58    | $E$               | 156        | 3.9      | 2111.17285(3)              | −0.103                   |
| 59    | $E$               | 161        | 3.9      | 2111.17285(3)              | −0.164                   |
| 60    | $A_1$             | 163        | 4.0      | 2112.09717(4)              | −0.117                   |
| 61    | $E$               | 247        | 2.3      | 2118.874379(8)             | −0.050                   |
| 62    | $E$               | 198        | 2.3      | 2118.87438(2)              | −0.082                   |
| 63    | $E$               | 162        | 2.3      | 2120.15698(4)              | −0.010                   |
| 64    | $E$               | 172        | 2.3      | 2120.15699(4)              | −0.053                   |
| 65    | $A_2$             | 215        | 2.3      | 2120.550586(9)             | −0.035                   |
| 66    | $E$               | 241        | 4.3      | 2122.555035(9)             | −0.091                   |
| 67    | $E$               | 165        | 4.3      | 2122.55505(4)              | −0.149                   |
| 68    | $A_1$             | 157        | 4.4      | 2123.02138(6)              | −0.114                   |
| 69    | $E$               | 103        | 0.58     | 2142.38638(3)              | −0.204                   |
| 70    | $E$               | 102        | 0.58     | 2142.38638(3)              | −0.205                   |
| 71    | $A_1$             | 111        | 0.1      | 2183.74737(3)              | −0.042                   |
| 72    | $A_2$             | 98         | 0.1      | 2183.74738(6)              | −0.086                   |
| 73    | $E$               | 138        | 0.47     | 2186.27530(2)              | −0.097                   |
| 74    | $E$               | 126        | 0.47     | 2186.27530(3)              | −0.102                   |
| 75    | $E$               | 135        | 0.64     | 2187.79381(2)              | −0.075                   |
| 76    | $E$               | 144        | 0.64     | 2187.79381(1)              | −0.090                   |
| 77    | $A_1$             | 140        | 0.69     | 2188.30027(2)              | −0.117                   |
| 78    | $A_1$             | 172        | 2.2      | 2205.10049(1)              | −0.062                   |
| 79    | $A_2$             | 171        | 2.2      | 2205.10803(2)              | −0.059                   |
| 80    | $E$               | 160        | 2.2      | 2205.25760(1)              | −0.127                   |
| 81    | $E$               | 221        | 2.2      | 2205.25761(1)              | −0.132                   |
| 82    | $E$               | 153        | 1.1      | 2206.038433(9)             | −0.027                   |
| 83    | $E$               | 152        | 1.1      | 2206.03843(1)              | −0.182                   |
| 84    | $A_1$             | 99         | 1.6      | 2250.70463(1)              | −0.202                   |
| 85    | $A_1$             | 172        | 4.1      | 2287.40905(1)              | −0.121                   |
| 86    | $E$               | 163        | 2.4      | 2289.63197(3)              | −0.069                   |
| 87    | $E$               | 180        | 2.4      | 2289.63198(2)              | −0.114                   |
| 88    | $A_2$             | 186        | 2.3      | 2289.82337(1)              | −0.153                   |
| 89    | $A_1$             | 171        | 3.3      | 2297.05753(1)              | −0.188                   |
| 90    | $E$               | 113        | 0.52     | 2344.74369(7)              | −0.103                   |
| 91    | $E$               | 153        | 0.52     | 2344.74370(6)              | −0.183                   |
| 92    | $E$               | 125        | 1.1      | 2346.12568(5)              | −0.103                   |
| 93    | $E$               | 145        | 1.1      | 2346.12569(4)              | −0.119                   |
| 94    | $A_1$             | 134        | 1.3      | 2346.58687(4)              | −0.154                   |
| 95    | $E$               | 128        | 0.26     | 2383.254336(7)             | −0.008                   |
| 96    | $E$               | 131        | 0.26     | 2383.254338(7)             | −0.205                   |
| 97    | $E$               | 178        | 3.1      | 2414.04094(1)              | −0.066                   |
| 98    | $E$               | 181        | 3.2      | 2414.04094(1)              | −0.167                   |
| 99    | $E$               | 206        | 4.0      | 2419.284062(7)             | −0.092                   |
| 100   | $E$               | 216        | 4.0      | 2419.28407(1)              | −0.137                   |
| 101   | $A_1$             | 160        | 2.3      | 2424.34874(4)              | −0.062                   |
| 102   | $A_2$             | 154        | 2.3      | 2424.36326(4)              | −0.096                   |
| 103   | $E$               | 183        | 4.3      | 2427.00777(1)              | −0.077                   |
| 104   | $E$               | 183        | 4.3      | 2427.00777(1)              | −0.124                   |
| 105   | $A_2$             | 136        | 3.9      | 2474.3123(2)               | −0.141                   |
| 106   | $A_1$             | 135        | 3.9      | 2474.3123(2)               | −0.172                   |

Continued on next page.

TABLE S3 – States on Sarka/Poirier USC PES; continued from previous page.

| State | $\Gamma_{C_{3v}}$ | $D_{\max}$ | $S_{vN}$ | $\tilde{E}/\text{cm}^{-1}$ | $\Delta\text{Ref. [30]}$ |
|-------|-------------------|------------|----------|----------------------------|--------------------------|
| 107   | $E$               | 180        | 3.9      | 2475.98878(5)              | −0.079                   |
| 108   | $E$               | 188        | 3.9      | 2475.98878(4)              | −0.185                   |
| 109   | $E$               | 168        | 2.3      | 2482.97205(8)              | −0.083                   |
| 110   | $E$               | 254        | 2.3      | 2482.97207(7)              | −0.100                   |
| 111   | $A_2$             | 200        | 2.5      | 2484.74174(5)              | −0.051                   |
| 112   | $A_1$             | 259        | 2.5      | 2484.74249(1)              | −0.092                   |
| 113   | $E$               | 255        | 1.8      | 2485.579766(7)             | −0.055                   |
| 114   | $E$               | 217        | 1.9      | 2485.57977(2)              | −0.131                   |
| 115   | $A_1$             | 266        | 4.3      | 2486.68016(1)              | −0.126                   |
| 116   | $A_2$             | 266        | 4.3      | 2486.68087(1)              | −0.152                   |
| 117   | $E$               | 185        | 4.4      | 2487.50750(6)              | −0.071                   |
| 118   | $E$               | 170        | 4.4      | 2487.50750(9)              | −0.175                   |
| 119   | $E$               | 115        | 0.74     | 2500.96313(5)              | −0.212                   |
| 120   | $E$               | 118        | 0.74     | 2500.96313(5)              | −0.214                   |
| 121   | $A_1$             | 118        | 1.1      | 2501.35897(5)              | −0.215                   |
| 122   | $A_2$             | 138        | 2.2      | 2513.05879(2)              | −0.086                   |
| 123   | $E$               | 141        | 2.2      | 2518.42936(1)              | −0.041                   |
| 124   | $E$               | 138        | 2.2      | 2518.42936(1)              | −0.088                   |
| 125   | $A_1$             | 140        | 2.3      | 2518.51250(1)              | −0.179                   |
| 126   | $E$               | 107        | 0.11     | 2551.73847(5)              | −0.077                   |
| 127   | $E$               | 136        | 0.11     | 2551.73848(4)              | −0.122                   |
| 128   | $E$               | 174        | 0.56     | 2554.53549(1)              | −0.108                   |
| 129   | $E$               | 172        | 0.56     | 2554.53549(1)              | −0.119                   |
| 130   | $A_1$             | 173        | 0.78     | 2556.40032(1)              | −0.076                   |
| 131   | $A_2$             | 167        | 0.78     | 2556.40429(1)              | −0.133                   |
| 132   | $E$               | 153        | 0.87     | 2557.33635(1)              | −0.056                   |
| 133   | $E$               | 163        | 0.87     | 2557.33635(1)              | −0.178                   |
| 134   | $E$               | 180        | 2.2      | 2568.60421(4)              | −0.080                   |
| 135   | $E$               | 180        | 2.2      | 2568.60421(3)              | −0.081                   |
| 136   | $E$               | 180        | 2.3      | 2568.92016(3)              | −0.121                   |
| 137   | $E$               | 175        | 2.3      | 2568.92017(3)              | −0.141                   |
| 138   | $A_2$             | 161        | 2.4      | 2569.70939(3)              | −0.078                   |
| 139   | $E$               | 170        | 2.4      | 2570.10228(3)              | −0.086                   |
| 140   | $E$               | 177        | 2.4      | 2570.10229(4)              | −0.120                   |
| 141   | $A_1$             | 166        | 2.4      | 2570.54219(3)              | −0.128                   |
| 142   | $E$               | 110        | 1.6      | 2609.20380(2)              | −0.205                   |
| 143   | $E$               | 106        | 1.6      | 2609.20380(4)              | −0.215                   |
| 144   | $E$               | 181        | 4.4      | 2646.55675(5)              | −0.116                   |
| 145   | $E$               | 187        | 4.4      | 2646.55676(6)              | −0.158                   |
| 146   | $A_1$             | 159        | 2.6      | 2649.5095(1)               | −0.117                   |
| 147   | $A_2$             | 155        | 2.6      | 2649.5109(1)               | −0.168                   |
| 148   | $E$               | 257        | 1.8      | 2650.127865(9)             | −0.193                   |
| 149   | $E$               | 197        | 1.8      | 2650.12787(4)              | −0.194                   |
| 150   | $A_1$             | 103        | 0.77     | 2651.61438(1)              | −0.252                   |
| 151   | $E$               | 158        | 3.7      | 2656.58262(5)              | −0.190                   |
| 152   | $E$               | 144        | 3.7      | 2656.5826(1)               | −0.196                   |
| 153   | $E$               | 213        | 0.62     | 2708.811678(5)             | −0.148                   |
| 154   | $E$               | 136        | 0.62     | 2708.81169(4)              | −0.205                   |
| 155   | $A_1$             | 137        | 1.4      | 2710.46457(5)              | −0.111                   |
| 156   | $A_2$             | 128        | 1.4      | 2710.46670(7)              | −0.153                   |
| 157   | $E$               | 130        | 1.6      | 2711.29358(5)              | −0.111                   |
| 158   | $E$               | 126        | 1.6      | 2711.29359(6)              | −0.201                   |
| 159   | $A_2$             | 201        | 2.4      | 2742.40366(1)              | −0.031                   |
| 160   | $E$               | 184        | 2.4      | 2742.45072(1)              | −0.085                   |
| 161   | $E$               | 186        | 2.4      | 2742.45072(1)              | −0.195                   |
| 162   | $A_1$             | 171        | 2.4      | 2742.840222(9)             | −0.133                   |
| 163   | $A_1$             | 191        | 4.9      | 2767.75543(2)              | −0.184                   |
| 164   | $E$               | 225        | 4.2      | 2774.21567(2)              | −0.127                   |
| 165   | $E$               | 229        | 4.2      | 2774.21567(1)              | −0.150                   |

Continued on next page.

TABLE S3 – States on Sarka/Poirier USC PES; continued from previous page.

| State | $\Gamma_{C_{3v}}$ | $D_{\max}$ | $S_{vN}$ | $\tilde{E}/\text{cm}^{-1}$ | $\Delta\text{Ref. [30]}$ |
|-------|-------------------|------------|----------|----------------------------|--------------------------|
| 166   | $A_1$             | 219        | 5.0      | 2775.79207(1)              | −0.143                   |
| 167   | $A_2$             | 224        | 5.1      | 2776.691421(7)             | −0.183                   |
| 168   | $A_1$             | 233        | 6.1      | 2781.26252(2)              | −0.122                   |
| 169   | $E$               | 230        | 5.1      | 2781.52627(1)              | −0.135                   |
| 170   | $E$               | 229        | 5.1      | 2781.52627(2)              | −0.160                   |
| 171   | $E$               | 241        | 2.4      | 2785.69486(1)              | −0.101                   |
| 172   | $E$               | 227        | 2.4      | 2785.69487(1)              | −0.118                   |
| 173   | $E$               | 257        | 3.6      | 2788.15773(1)              | −0.127                   |
| 174   | $E$               | 226        | 3.6      | 2788.15773(2)              | −0.146                   |
| 175   | $A_2$             | 219        | 5.1      | 2789.37651(1)              | −0.155                   |
| 176   | $A_1$             | 217        | 5.9      | 2789.86922(3)              | −0.123                   |
| 177   | $E$               | 140        | 0.56     | 2811.513404(5)             | −0.215                   |
| 178   | $E$               | 140        | 0.56     | 2811.513404(5)             | −0.232                   |
| 179   | $E$               | 170        | 3.9      | 2838.6861(1)               | −0.169                   |
| 180   | $E$               | 201        | 3.9      | 2838.6862(1)               | −0.181                   |
| 181   | $E$               | 193        | 4.0      | 2840.98322(7)              | −0.126                   |
| 182   | $E$               | 254        | 4.0      | 2840.98323(7)              | −0.182                   |
| 183   | $A_1$             | 188        | 4.1      | 2841.76530(6)              | −0.153                   |
| 184   | $A_1$             | 186        | 2.4      | 2848.21044(7)              | −0.121                   |
| 185   | $A_2$             | 212        | 2.4      | 2848.21045(6)              | −0.122                   |
| 186   | $E$               | 280        | 2.7      | 2850.37227(2)              | −0.117                   |
| 187   | $E$               | 204        | 2.7      | 2850.3723(1)               | −0.124                   |
| 188   | $E$               | 287        | 2.7      | 2851.65448(1)              | −0.113                   |
| 189   | $E$               | 213        | 2.7      | 2851.65449(5)              | −0.121                   |
| 190   | $E$               | 277        | 4.3      | 2851.89989(1)              | −0.155                   |
| 191   | $E$               | 175        | 4.3      | 2851.8999(1)               | −0.162                   |
| 192   | $A_2$             | 188        | 2.7      | 2852.07617(8)              | −0.128                   |
| 193   | $E$               | 256        | 4.6      | 2852.97949(3)              | −0.113                   |
| 194   | $E$               | 246        | 4.6      | 2852.97949(4)              | −0.163                   |
| 195   | $A_1$             | 207        | 4.8      | 2853.32941(6)              | −0.151                   |
| 196   | $A_1$             | 108        | 0.91     | 2860.8365(1)               | −0.224                   |
| 197   | $A_2$             | 114        | 0.91     | 2860.8372(1)               | −0.228                   |
| 198   | $E$               | 178        | 1.6      | 2861.51251(1)              | −0.221                   |
| 199   | $E$               | 177        | 1.6      | 2861.51251(1)              | −0.238                   |
| 200   | $E$               | 211        | 4.3      | 2870.63771(1)              | −0.076                   |
| 201   | $E$               | 180        | 4.3      | 2870.63772(3)              | −0.194                   |
| 202   | $E$               | 214        | 4.5      | 2875.20543(1)              | −0.101                   |
| 203   | $E$               | 237        | 4.5      | 2875.20544(1)              | −0.141                   |
| 204   | $A_1$             | 174        | 3.4      | 2879.07056(6)              | −0.085                   |
| 205   | $A_2$             | 167        | 3.2      | 2879.10966(6)              | −0.117                   |
| 206   | $E$               | 220        | 2.3      | 2879.265299(9)             | −0.064                   |
| 207   | $E$               | 217        | 2.3      | 2879.26530(1)              | −0.206                   |
| 208   | $E$               | 208        | 4.5      | 2881.27584(1)              | −0.056                   |
| 209   | $E$               | 208        | 4.5      | 2881.27584(1)              | −0.190                   |
| 210   | $E$               | 154        | 0.13     | 2920.84313(1)              | −0.115                   |
| 211   | $E$               | 126        | 0.13     | 2920.84313(3)              | −0.154                   |
| 212   | $A_1$             | 157        | 0.66     | 2923.82081(3)              | −0.121                   |
| 213   | $A_2$             | 158        | 0.66     | 2923.82081(2)              | −0.125                   |
| 214   | $E$               | 161        | 0.93     | 2925.94975(2)              | −0.111                   |
| 215   | $E$               | 226        | 0.93     | 2925.94976(2)              | −0.144                   |
| 216   | $E$               | 219        | 1.1      | 2927.227853(5)             | −0.102                   |
| 217   | $E$               | 196        | 1.1      | 2927.227854(9)             | −0.131                   |
| 218   | $A_1$             | 180        | 1.1      | 2927.65399(1)              | −0.155                   |
| 219   | $E$               | 187        | 2.2      | 2933.27429(8)              | −0.094                   |
| 220   | $E$               | 205        | 2.2      | 2933.27430(7)              | −0.110                   |
| 221   | $A_1$             | 214        | 2.4      | 2933.74057(4)              | −0.132                   |
| 222   | $A_2$             | 157        | 2.4      | 2933.7422(1)               | −0.156                   |
| 223   | $E$               | 272        | 2.4      | 2935.11681(1)              | −0.088                   |
| 224   | $E$               | 182        | 2.4      | 2935.11683(5)              | −0.180                   |

Continued on next page.

TABLE S3 – States on Sarka/Poirier USC PES; continued from previous page.

| State | $\Gamma_{C_{3v}}$ | $D_{\max}$ | $S_{vN}$ | $\tilde{E}/\text{cm}^{-1}$ | $\Delta\text{Ref. [30]}$ |
|-------|-------------------|------------|----------|----------------------------|--------------------------|
| 225   | $A_1$             | 152        | 2.4      | 2935.2625(2)               | −0.143                   |
| 226   | $A_2$             | 157        | 2.4      | 2935.2863(1)               | −0.144                   |
| 227   | $E$               | 173        | 1.8      | 2936.21178(7)              | −0.056                   |
| 228   | $E$               | 174        | 1.7      | 2936.21178(6)              | −0.203                   |
| 229   | $A_1$             | 149        | 2.5      | 2945.14843(1)              | −0.301                   |
| 230   | $A_1$             | 191        | 0.83     | 2949.864849(7)             | −0.136                   |
| 231   | $E$               | 178        | 0.42     | 2958.232306(7)             | −0.138                   |
| 232   | $E$               | 179        | 0.42     | 2958.232307(6)             | −0.217                   |
| 233   | $E$               | 177        | 0.4      | 2964.847196(4)             | −0.138                   |
| 234   | $E$               | 156        | 0.4      | 2964.84720(1)              | −0.184                   |
| 235   | $E$               | 121        | 1.6      | 2968.92573(6)              | −0.219                   |
| 236   | $E$               | 114        | 1.6      | 2968.92574(7)              | −0.231                   |
| 237   | $A_1$             | 171        | 1.7      | 2969.57418(1)              | −0.232                   |
| 238   | $A_1$             | 145        | 2.2      | 2979.452351(8)             | −0.423                   |
| 239   | $E$               | 194        | 4.7      | 3006.8965(1)               | −0.153                   |
| 240   | $E$               | 193        | 4.7      | 3006.8965(1)               | −0.187                   |
| 241   | $E$               | 143        | 1.0      | 3006.97145(1)              | −0.275                   |
| 242   | $E$               | 185        | 1.0      | 3006.97145(1)              | −0.333                   |
| 243   | $A_1$             | 185        | 5.0      | 3007.7106(1)               | −0.193                   |
| 244   | $E$               | 211        | 2.7      | 3010.6077(1)               | −0.156                   |
| 245   | $E$               | 229        | 2.7      | 3010.60768(9)              | −0.212                   |
| 246   | $E$               | 188        | 3.0      | 3011.6340(1)               | −0.209                   |
| 247   | $E$               | 261        | 3.0      | 3011.6340(1)               | −0.222                   |
| 248   | $A_2$             | 192        | 3.0      | 3011.95088(9)              | −0.201                   |
| 249   | $E$               | 199        | 4.0      | 3017.29250(6)              | −0.202                   |
| 250   | $E$               | 195        | 4.0      | 3017.29251(7)              | −0.223                   |
| 251   | $A_1$             | 177        | 4.2      | 3017.5752(1)               | −0.229                   |
| 252   | $E$               | 144        | 0.53     | 3049.672333(8)             | −0.310                   |
| 253   | $E$               | 146        | 0.53     | 3049.672334(8)             | −0.497                   |
| 254   | $A_2$             | 127        | 0.71     | 3074.07686(8)              | −0.184                   |
| 255   | $A_1$             | 133        | 0.71     | 3074.07686(7)              | −0.223                   |
| 256   | $E$               | 193        | 0.55     | 3075.461513(6)             | −0.068                   |
| 257   | $E$               | 185        | 0.55     | 3075.461514(7)             | −0.220                   |
| 258   | $E$               | 156        | 1.6      | 3075.89894(4)              | −0.133                   |
| 259   | $E$               | 184        | 1.6      | 3075.89895(4)              | −0.198                   |
| 260   | $E$               | 229        | 2.0      | 3076.992956(7)             | −0.149                   |
| 261   | $E$               | 145        | 2.0      | 3076.99297(5)              | −0.179                   |
| 262   | $A_1$             | 156        | 2.1      | 3077.35776(4)              | −0.208                   |
| 263   | $A_1$             | 169        | 0.35     | 3091.30514(1)              | −0.084                   |
| 264   | $A_2$             | 158        | 0.25     | 3092.26367(2)              | −0.172                   |
| 265   | $A_1$             | 262        | 2.5      | 3102.88483(2)              | −0.087                   |
| 266   | $A_2$             | 216        | 2.5      | 3102.89340(4)              | −0.162                   |
| 267   | $E$               | 190        | 2.5      | 3103.06133(4)              | −0.189                   |
| 268   | $E$               | 253        | 2.5      | 3103.06134(3)              | −0.226                   |
| 269   | $E$               | 179        | 1.7      | 3103.77569(6)              | −0.080                   |
| 270   | $E$               | 182        | 1.7      | 3103.77569(4)              | −0.251                   |
| 271   | $E$               | 201        | 4.8      | 3127.94905(8)              | −0.188                   |
| 272   | $E$               | 206        | 4.8      | 3127.94905(7)              | −0.270                   |
| 273   | $A_1$             | 189        | 4.4      | 3135.7756(2)               | −0.161                   |
| 274   | $A_2$             | 192        | 4.4      | 3135.7806(2)               | −0.168                   |
| 275   | $E$               | 229        | 4.9      | 3137.65580(8)              | −0.111                   |
| 276   | $E$               | 223        | 4.9      | 3137.6558(1)               | −0.232                   |
| 277   | $E$               | 240        | 6.0      | 3138.85286(6)              | −0.190                   |
| 278   | $E$               | 279        | 6.0      | 3138.85287(5)              | −0.205                   |
| 279   | $A_1$             | 170        | 2.9      | 3140.88468(1)              | −0.265                   |
| 280   | $E$               | 316        | 5.2      | 3144.53564(2)              | −0.131                   |
| 281   | $E$               | 236        | 5.3      | 3144.53566(7)              | −0.171                   |
| 282   | $A_1$             | 201        | 5.4      | 3144.6030(3)               | −0.175                   |
| 283   | $A_2$             | 200        | 5.5      | 3144.6141(3)               | −0.174                   |

Continued on next page.

TABLE S3 – States on Sarka/Poirier USC PES; continued from previous page.

| State | $\Gamma_{C_{3v}}$ | $D_{\max}$ | $S_{vN}$ | $\tilde{E}/\text{cm}^{-1}$ | $\Delta\text{Ref. [30]}$ |
|-------|-------------------|------------|----------|----------------------------|--------------------------|
| 284   | $E$               | 239        | 2.5      | 3148.18676(4)              | −0.127                   |
| 285   | $E$               | 241        | 2.5      | 3148.18677(3)              | −0.161                   |
| 286   | $A_1$             | 253        | 4.9      | 3150.48803(7)              | −0.143                   |
| 287   | $A_2$             | 290        | 4.8      | 3150.49893(3)              | −0.169                   |
| 288   | $E$               | 309        | 4.8      | 3152.03055(1)              | −0.151                   |
| 289   | $E$               | 241        | 4.8      | 3152.03057(4)              | −0.169                   |
| 290   | $E$               | 229        | 5.8      | 3152.8978(1)               | −0.139                   |
| 291   | $E$               | 222        | 5.8      | 3152.8978(1)               | −0.211                   |
| 292   | $A_1$             | 186        | 3.4      | 3167.04252(6)              | −0.266                   |
| 293   | $E$               | 183        | 2.8      | 3168.17834(7)              | −0.239                   |
| 294   | $E$               | 183        | 2.8      | 3168.17834(6)              | −0.268                   |
| 295   | $A_2$             | 167        | 2.7      | 3168.31043(6)              | −0.240                   |
| 296   | $A_1$             | 139        | 3.2      | 3183.70622(4)              | −0.281                   |
| 297   | $E$               | 180        | 3.8      | 3204.2669(1)               | −0.194                   |
| 298   | $E$               | 217        | 3.8      | 3204.2669(1)               | −0.196                   |
| 299   | $A_1$             | 233        | 4.1      | 3207.07112(5)              | −0.166                   |
| 300   | $A_2$             | 245        | 4.1      | 3207.07153(4)              | −0.209                   |
| 301   | $E$               | 221        | 4.1      | 3208.50868(4)              | −0.112                   |
| 302   | $E$               | 180        | 4.1      | 3208.5087(1)               | −0.245                   |
| 303   | $E$               | 274        | 2.5      | 3214.57483(1)              | −0.147                   |
| 304   | $E$               | 226        | 2.5      | 3214.57484(4)              | −0.161                   |
| 305   | $E$               | 208        | 3.3      | 3216.9652(1)               | −0.146                   |
| 306   | $E$               | 220        | 3.3      | 3216.9652(1)               | −0.170                   |
| 307   | $E$               | 316        | 4.3      | 3218.27358(1)              | −0.175                   |
| 308   | $E$               | 275        | 4.3      | 3218.27358(2)              | −0.177                   |
| 309   | $A_1$             | 177        | 3.5      | 3218.6234(3)               | −0.141                   |
| 310   | $A_2$             | 232        | 3.5      | 3218.62531(9)              | −0.155                   |
| 311   | $E$               | 282        | 2.3      | 3219.52692(1)              | −0.086                   |
| 312   | $E$               | 242        | 2.2      | 3219.52693(3)              | −0.151                   |
| 313   | $A_1$             | 179        | 4.7      | 3219.5342(3)               | −0.189                   |
| 314   | $A_2$             | 175        | 4.7      | 3219.5349(3)               | −0.217                   |
| 315   | $E$               | 204        | 4.9      | 3220.0578(1)               | −0.123                   |
| 316   | $E$               | 215        | 4.9      | 3220.0578(1)               | −0.221                   |
| 317   | $E$               | 165        | 1.1      | 3222.00212(3)              | −0.241                   |
| 318   | $E$               | 215        | 1.1      | 3222.00212(3)              | −0.252                   |
| 319   | $E$               | 176        | 2.0      | 3222.83305(3)              | −0.251                   |
| 320   | $E$               | 164        | 2.0      | 3222.83306(4)              | −0.264                   |
| 321   | $A_1$             | 214        | 2.2      | 3223.11128(1)              | −0.278                   |
| 322   | $A_2$             | 226        | 5.8      | 3231.16605(2)              | −0.170                   |
| 323   | $E$               | 246        | 5.8      | 3231.17228(1)              | −0.211                   |
| 324   | $E$               | 264        | 5.8      | 3231.17229(2)              | −0.217                   |
| 325   | $A_1$             | 266        | 5.4      | 3232.48865(2)              | −0.182                   |
| 326   | $E$               | 271        | 5.2      | 3237.59137(2)              | −0.147                   |
| 327   | $E$               | 250        | 5.2      | 3237.59139(2)              | −0.160                   |
| 328   | $A_2$             | 258        | 4.9      | 3237.87851(1)              | −0.165                   |
| 329   | $E$               | 246        | 3.4      | 3240.93400(2)              | −0.141                   |
| 330   | $E$               | 250        | 3.4      | 3240.93400(2)              | −0.146                   |
| 331   | $E$               | 255        | 3.6      | 3241.47354(2)              | −0.101                   |
| 332   | $E$               | 247        | 3.6      | 3241.47355(1)              | −0.137                   |
| 333   | $A_1$             | 261        | 3.7      | 3241.68010(2)              | −0.171                   |
| 334   | $E$               | 293        | 5.6      | 3243.41539(2)              | −0.141                   |
| 335   | $E$               | 252        | 5.6      | 3243.41542(2)              | −0.181                   |
| 336   | $A_2$             | 240        | 5.6      | 3243.49486(1)              | −0.176                   |
| 337   | $A_1$             | 255        | 6.1      | 3244.11474(1)              | −0.178                   |
| 338   | $E$               | 154        | 0.51     | 3268.354152(8)             | −0.233                   |
| 339   | $E$               | 155        | 0.51     | 3268.35415(1)              | −0.291                   |
| 340   | $E$               | 157        | 1.9      | 3279.433678(5)             | −0.226                   |
| 341   | $E$               | 158        | 1.9      | 3279.43368(1)              | −0.262                   |
| 342   | $A_2$             | 115        | 0.14     | 3291.04747(6)              | −0.153                   |

Continued on next page.

TABLE S3 – States on Sarka/Poirier USC PES; continued from previous page.

| State | $\Gamma_{C_{3v}}$ | $D_{\max}$ | $S_{vN}$ | $\tilde{E}/\text{cm}^{-1}$ | $\Delta\text{Ref. [30]}$ |
|-------|-------------------|------------|----------|----------------------------|--------------------------|
| 343   | $A_1$             | 120        | 0.14     | 3291.04747(5)              | −0.186                   |
| 344   | $E$               | 185        | 0.77     | 3294.11164(2)              | −0.130                   |
| 345   | $E$               | 182        | 0.77     | 3294.11164(2)              | −0.148                   |
| 346   | $E$               | 178        | 1.1      | 3296.41133(3)              | −0.151                   |
| 347   | $E$               | 191        | 1.1      | 3296.41133(2)              | −0.155                   |
| 348   | $A_1$             | 124        | 1.3      | 3297.9400(1)               | −0.136                   |
| 349   | $A_2$             | 120        | 1.3      | 3297.9483(2)               | −0.156                   |
| 350   | $E$               | 177        | 1.4      | 3298.71080(3)              | −0.091                   |
| 351   | $E$               | 192        | 1.4      | 3298.71080(3)              | −0.261                   |
| 352   | $A_1^*$           | 153        | 2.2      | 3299.1000(3)               | −0.115                   |
| 353   | $A_2^*$           | 154        | 2.2      | 3299.1000(3)               | −0.143                   |
| 354   | $E$               | 203        | 2.4      | 3299.71461(8)              | −0.153                   |
| 355   | $E$               | 277        | 2.4      | 3299.71462(8)              | −0.179                   |
| 356   | $E$               | 282        | 2.2      | 3301.52652(2)              | −0.121                   |
| 357   | $E$               | 243        | 2.2      | 3301.52653(6)              | −0.129                   |
| 358   | $E$               | 266        | 2.3      | 3301.55198(3)              | −0.203                   |
| 359   | $E$               | 191        | 2.3      | 3301.5520(1)               | −0.226                   |
| 360   | $A_2$             | 191        | 2.7      | 3302.1781(1)               | −0.183                   |
| 361   | $E$               | 245        | 2.7      | 3302.93856(4)              | −0.117                   |
| 362   | $E$               | 208        | 2.7      | 3302.93857(9)              | −0.155                   |
| 363   | $A_1$             | 240        | 2.7      | 3303.39197(3)              | −0.181                   |
| 364   | $E$               | 233        | 3.9      | 3306.284421(7)             | −0.277                   |
| 365   | $E$               | 241        | 4.0      | 3306.284424(7)             | −0.317                   |
| 366   | $E$               | 233        | 3.6      | 3307.47196(1)              | −0.173                   |
| 367   | $E$               | 240        | 3.6      | 3307.47196(2)              | −0.227                   |
| 368   | $E$               | 250        | 4.4      | 3314.30225(2)              | −0.178                   |
| 369   | $E$               | 235        | 4.4      | 3314.30226(1)              | −0.232                   |
| 370   | $A_1$             | 247        | 2.7      | 3316.351162(9)             | −0.202                   |
| 371   | $A_2$             | 248        | 2.6      | 3316.36380(1)              | −0.194                   |
| 372   | $E$               | 220        | 3.9      | 3322.72405(2)              | −0.217                   |
| 373   | $E$               | 220        | 3.9      | 3322.72405(2)              | −0.267                   |
| 374   | $A_1$             | 210        | 2.4      | 3326.06169(1)              | −0.178                   |
| 375   | $A_2$             | 231        | 2.4      | 3326.074935(6)             | −0.183                   |
| 376   | $E$               | 191        | 2.5      | 3326.36657(2)              | −0.181                   |
| 377   | $E$               | 197        | 2.5      | 3326.36657(2)              | −0.196                   |
| 378   | $A_1$             | 109        | 1.6      | 3329.8544(2)               | −0.245                   |
| 379   | $A_2$             | 115        | 1.6      | 3329.8547(1)               | −0.247                   |
| 380   | $E$               | 187        | 1.7      | 3331.07849(2)              | −0.247                   |
| 381   | $E$               | 162        | 1.7      | 3331.07850(3)              | −0.263                   |
| 382   | $E$               | 174        | 2.2      | 3340.539827(6)             | −0.442                   |
| 383   | $E$               | 177        | 2.2      | 3340.539827(6)             | −0.446                   |
| 384   | $E$               | 164        | 1.3      | 3363.72774(2)              | −0.348                   |
| 385   | $E$               | 160        | 1.3      | 3363.72774(3)              | −0.366                   |
| 386   | $A_1$             | 171        | 1.8      | 3363.87937(2)              | −0.423                   |
| 387   | $A_1$             | 182        | 4.9      | 3368.4632(3)               | −0.196                   |
| 388   | $A_2$             | 178        | 4.9      | 3368.4640(3)               | −0.244                   |
| 389   | $E$               | 210        | 5.2      | 3369.8815(1)               | −0.170                   |
| 390   | $E$               | 204        | 5.2      | 3369.8815(1)               | −0.279                   |
| 391   | $E$               | 312        | 2.9      | 3372.91325(2)              | −0.204                   |
| 392   | $E$               | 238        | 2.9      | 3372.91325(8)              | −0.251                   |
| 393   | $A_1$             | 182        | 3.4      | 3374.2540(4)               | −0.227                   |
| 394   | $A_2$             | 184        | 3.4      | 3374.2587(3)               | −0.235                   |
| 395   | $E$               | 226        | 2.7      | 3374.92537(7)              | −0.228                   |
| 396   | $E$               | 275        | 2.7      | 3374.92537(6)              | −0.244                   |
| 397   | $A_1$             | 190        | 4.3      | 3379.1957(1)               | −0.235                   |
| 398   | $A_2$             | 215        | 4.3      | 3379.19653(9)              | −0.257                   |
| 399   | $E$               | 200        | 4.6      | 3379.6445(1)               | −0.229                   |
| 400   | $E$               | 199        | 4.6      | 3379.6445(1)               | −0.293                   |
| 401   | $E$               | 193        | 2.6      | 3410.815756(6)             | −0.370                   |

Continued on next page.

TABLE S3 – States on Sarka/Poirier USC PES; continued from previous page.

| State | $\Gamma_{C_{3v}}$ | $D_{\max}$ | $S_{vN}$ | $\tilde{E}/\text{cm}^{-1}$ | $\Delta\text{Ref. [30]}$ |
|-------|-------------------|------------|----------|----------------------------|--------------------------|
| 402   | $E$               | 190        | 2.6      | 3410.81577(2)              | −0.376                   |
| 403   | $A_2$             | 200        | 3.9      | 3410.961968(8)             | −0.453                   |
| 404   | $A_1$             | 188        | 2.7      | 3410.99312(1)              | −0.514                   |
| 405   | $A_2$             | 173        | 3.8      | 3411.34859(6)              | −0.258                   |
| 406   | $E$               | 169        | 2.4      | 3416.69017(3)              | −0.074                   |
| 407   | $E$               | 194        | 2.4      | 3416.69017(3)              | −0.233                   |
| 408   | $A_1$             | 212        | 2.5      | 3416.827614(6)             | −0.309                   |
| 409   | $A_1$             | 242        | 4.7      | 3429.92365(1)              | −0.228                   |
| 410   | $E$               | 227        | 3.5      | 3434.36728(2)              | −0.162                   |
| 411   | $E$               | 256        | 3.5      | 3434.36728(2)              | −0.223                   |
| 412   | $A_2$             | 233        | 2.6      | 3435.77749(1)              | −0.162                   |
| 413   | $E$               | 159        | 0.81     | 3440.52920(4)              | −0.215                   |
| 414   | $E$               | 181        | 0.81     | 3440.52920(3)              | −0.243                   |
| 415   | $A_1$             | 239        | 4.0      | 3440.93448(1)              | −0.235                   |
| 416   | $E$               | 271        | 3.9      | 3442.368397(9)             | −0.217                   |
| 417   | $E$               | 263        | 3.9      | 3442.368399(9)             | −0.221                   |
| 418   | $E$               | 177        | 1.9      | 3442.40939(4)              | −0.197                   |
| 419   | $E$               | 204        | 1.9      | 3442.40940(3)              | −0.235                   |
| 420   | $A_1$             | 250        | 2.4      | 3443.658865(8)             | −0.204                   |
| 421   | $A_2$             | 177        | 2.4      | 3443.66489(4)              | −0.200                   |
| 422   | $E$               | 159        | 2.6      | 3444.28783(5)              | −0.164                   |
| 423   | $E$               | 179        | 2.6      | 3444.28784(4)              | −0.327                   |
| 424   | $E$               | 261        | 2.6      | 3451.49143(1)              | −0.133                   |
| 425   | $E$               | 254        | 2.6      | 3451.49143(1)              | −0.196                   |
| 426   | $E$               | 254        | 4.2      | 3454.24324(1)              | −0.180                   |
| 427   | $E$               | 237        | 4.2      | 3454.24324(2)              | −0.207                   |
| 428   | $E$               | 200        | 2.6      | 3464.5567(1)               | −0.157                   |
| 429   | $E$               | 281        | 2.6      | 3464.5567(1)               | −0.221                   |
| 430   | $E$               | 285        | 2.7      | 3464.90704(2)              | −0.224                   |
| 431   | $E$               | 282        | 2.7      | 3464.90704(2)              | −0.241                   |
| 432   | $A_2$             | 283        | 3.0      | 3465.47575(2)              | −0.218                   |
| 433   | $E$               | 204        | 2.9      | 3465.8932(1)               | −0.148                   |
| 434   | $E$               | 198        | 2.9      | 3465.8932(1)               | −0.207                   |
| 435   | $A_1$             | 195        | 3.0      | 3466.3246(1)               | −0.236                   |
| 436   | $E$               | 219        | 4.8      | 3489.4970(1)               | −0.271                   |
| 437   | $E$               | 220        | 4.8      | 3489.4970(1)               | −0.302                   |
| 438   | $A_1$             | 249        | 4.8      | 3490.56774(7)              | −0.285                   |
| 439   | $E$               | 170        | 3.1      | 3497.55196(5)              | −0.293                   |
| 440   | $E$               | 204        | 3.1      | 3497.55197(4)              | −0.334                   |
| 441   | $A_1$             | 182        | 1.3      | 3498.085601(7)             | −0.727                   |
| 442   | $E$               | 241        | 4.5      | 3498.6120(1)               | −0.203                   |
| 443   | $E$               | 244        | 4.5      | 3498.6120(1)               | −0.390                   |
| 444   | $E$               | 246        | 5.7      | 3500.6967(2)               | −0.207                   |
| 445   | $E$               | 249        | 5.7      | 3500.6967(1)               | −0.223                   |
| 446   | $A_1$             | 244        | 5.8      | 3501.4578(1)               | −0.259                   |
| 447   | $E$               | 279        | 6.3      | 3502.05357(9)              | −0.221                   |
| 448   | $E$               | 245        | 6.3      | 3502.0536(1)               | −0.227                   |
| 449   | $A_2$             | 276        | 5.2      | 3502.69388(8)              | −0.220                   |
| 450   | $E$               | 259        | 5.2      | 3508.5966(1)               | −0.208                   |
| 451   | $E$               | 341        | 5.2      | 3508.5966(1)               | −0.209                   |
| 452   | $E$               | 270        | 5.8      | 3508.9063(1)               | −0.195                   |
| 453   | $E$               | 249        | 5.8      | 3508.9063(2)               | −0.204                   |
| 454   | $A_1$             | 248        | 6.0      | 3508.9198(2)               | −0.264                   |
| 455   | $A_2$             | 199        | 2.7      | 3511.8164(2)               | −0.172                   |
| 456   | $A_1$             | 204        | 2.7      | 3511.8164(1)               | −0.198                   |
| 457   | $E$               | 344        | 4.5      | 3514.01413(4)              | −0.168                   |
| 458   | $E$               | 259        | 4.5      | 3514.0142(1)               | −0.212                   |
| 459   | $E$               | 268        | 3.9      | 3515.63856(7)              | −0.195                   |
| 460   | $E$               | 282        | 3.9      | 3515.63856(7)              | −0.216                   |

Continued on next page.



TABLE S3 – States on Sarka/Poirier USC PES; continued from previous page.

| State | $\Gamma_{C_{3v}}$ | $D_{\max}$ | $S_{vN}$ | $\tilde{E}/\text{cm}^{-1}$ | $\Delta\text{Ref. [30]}$ |
|-------|-------------------|------------|----------|----------------------------|--------------------------|
| 461   | $A_2$             | 289        | 5.4      | 3516.54120(8)              | −0.186                   |
| 462   | $A_1$             | 261        | 6.1      | 3516.7387(1)               | −0.201                   |
| 463   | $E$               | 237        | 5.8      | 3516.9415(1)               | −0.228                   |
| 464   | $E$               | 236        | 5.8      | 3516.9415(1)               | −0.231                   |
| 465   | $E$               | 300        | 3.7      | 3524.58727(1)              | −0.289                   |
| 466   | $E$               | 216        | 3.7      | 3524.58728(9)              | −0.372                   |
| 467   | $A_1$             | 196        | 3.1      | 3526.1412(1)               | −0.297                   |
| 468   | $A_2$             | 169        | 3.1      | 3526.1449(3)               | −0.306                   |
| 469   | $E$               | 193        | 2.3      | 3526.5562(1)               | −0.267                   |
| 470   | $E$               | 190        | 2.4      | 3526.5562(1)               | −0.298                   |
| 471   | $E$               | 201        | 1.4      | 3539.59958(1)              | −0.207                   |
| 472   | $E$               | 232        | 1.5      | 3539.599581(8)             | −0.247                   |
| 473   | $E$               | 170        | 3.4      | 3540.68771(5)              | −0.313                   |
| 474   | $E$               | 162        | 3.4      | 3540.68771(7)              | −0.387                   |
| 475   | $E$               | 191        | 2.4      | 3548.86012(1)              | −0.104                   |
| 476   | $E$               | 231        | 2.4      | 3548.86013(1)              | −0.289                   |
| 477   | $A_2$             | 191        | 2.2      | 3551.73318(1)              | −0.187                   |
| 478   | $A_1$             | 184        | 2.5      | 3552.57421(2)              | −0.196                   |
| 479   | $A_1$             | 200        | 3.8      | 3571.03035(9)              | −0.222                   |
| 480   | $A_2$             | 199        | 3.8      | 3571.03035(9)              | −0.224                   |
| 481   | $E$               | 208        | 4.2      | 3574.2363(1)               | −0.215                   |
| 482   | $E$               | 204        | 4.2      | 3574.2363(1)               | −0.243                   |
| 483   | $E$               | 277        | 4.3      | 3576.21237(2)              | −0.199                   |
| 484   | $E$               | 195        | 4.3      | 3576.2124(1)               | −0.232                   |
| 485   | $A_1$             | 249        | 4.3      | 3576.88193(3)              | −0.246                   |
| 486   | $E$               | 286        | 2.5      | 3582.05080(1)              | −0.183                   |
| 487   | $E$               | 193        | 2.5      | 3582.0508(1)               | −0.203                   |
| 488   | $A_1$             | 321        | 4.0      | 3584.43962(3)              | −0.177                   |
| 489   | $A_2$             | 317        | 4.0      | 3584.43963(3)              | −0.193                   |
| 490   | $E$               | 264        | 1.2      | 3584.454096(6)             | −0.274                   |
| 491   | $E$               | 255        | 1.2      | 3584.454096(7)             | −0.286                   |
| 492   | $A_1$             | 128        | 2.4      | 3585.3051(2)               | −0.308                   |
| 493   | $A_2$             | 130        | 2.4      | 3585.3081(2)               | −0.312                   |
| 494   | $E$               | 203        | 2.8      | 3585.73348(2)              | −0.274                   |
| 495   | $E$               | 205        | 2.8      | 3585.73348(2)              | −0.341                   |
| 496   | $A_2^*$           | 172        | 4.3      | 3585.8579(3)               | −0.220                   |
| 497   | $A_1^*$           | 175        | 4.3      | 3585.8579(2)               | −0.338                   |
| 498   | $E$               | 248        | 4.6      | 3586.2399(1)               | −0.174                   |
| 499   | $E$               | 242        | 4.7      | 3586.2399(1)               | −0.217                   |
| 500   | $E$               | 226        | 4.5      | 3587.3765(1)               | −0.173                   |
| 501   | $E$               | 234        | 4.5      | 3587.3765(1)               | −0.199                   |
| 502   | $E$               | 225        | 5.0      | 3587.4156(1)               | −0.186                   |
| 503   | $E$               | 293        | 5.0      | 3587.4156(1)               | −0.218                   |
| 504   | $A_1$             | 286        | 5.2      | 3587.86931(3)              | −0.255                   |
| 505   | $E$               | 329        | 4.2      | 3588.13919(2)              | −0.132                   |
| 506   | $E$               | 230        | 4.2      | 3588.1392(1)               | −0.217                   |
| 507   | $A_2$             | 267        | 3.1      | 3588.32086(2)              | −0.212                   |
| 508   | $A_1$             | 218        | 5.8      | 3593.1108(2)               | −0.224                   |
| 509   | $A_2$             | 219        | 5.8      | 3593.1173(2)               | −0.250                   |
| 510   | $E$               | 258        | 5.6      | 3593.49495(3)              | −0.232                   |
| 511   | $E$               | 250        | 5.6      | 3593.49495(5)              | −0.254                   |
| 512   | $E$               | 253        | 5.0      | 3594.99709(5)              | −0.128                   |
| 513   | $E$               | 259        | 5.0      | 3594.99709(3)              | −0.333                   |
| 514   | $A_2$             | 264        | 5.3      | 3600.93266(3)              | −0.184                   |
| 515   | $A_1$             | 286        | 5.3      | 3600.93302(5)              | −0.209                   |
| 516   | $E$               | 259        | 4.8      | 3601.76594(8)              | −0.150                   |
| 517   | $E$               | 256        | 4.8      | 3601.76594(6)              | −0.209                   |
| 518   | $E$               | 315        | 3.5      | 3603.94729(2)              | −0.175                   |
| 519   | $E$               | 261        | 3.5      | 3603.94730(4)              | −0.185                   |

Continued on next page.

TABLE S3 – States on Sarka/Poirier USC PES; continued from previous page.

| State | $\Gamma_{C_{3v}}$ | $D_{\max}$ | $S_{vN}$ | $\tilde{E}/\text{cm}^{-1}$ | $\Delta\text{Ref. [30]}$ |
|-------|-------------------|------------|----------|----------------------------|--------------------------|
| 520   | $A_1$             | 223        | 4.6      | 3604.9185(2)               | −0.131                   |
| 521   | $A_2$             | 216        | 4.5      | 3604.9546(2)               | −0.155                   |
| 522   | $E$               | 257        | 3.1      | 3605.43290(6)              | −0.098                   |
| 523   | $E$               | 320        | 3.1      | 3605.43291(6)              | −0.223                   |
| 524   | $A_1$             | 305        | 6.2      | 3606.53926(8)              | −0.214                   |
| 525   | $A_2$             | 332        | 6.1      | 3606.60130(4)              | −0.192                   |
| 526   | $E$               | 263        | 5.6      | 3607.03129(4)              | −0.174                   |
| 527   | $E$               | 264        | 5.6      | 3607.03129(5)              | −0.214                   |
| 528   | $E$               | 263        | 5.6      | 3607.70883(4)              | −0.111                   |
| 529   | $E$               | 263        | 5.6      | 3607.70883(5)              | −0.333                   |
| 530   | $A_2$             | 160        | 2.7      | 3625.54780(4)              | −0.254                   |
| 531   | $E$               | 196        | 2.7      | 3625.57665(4)              | −0.302                   |
| 532   | $E$               | 163        | 2.7      | 3625.57668(5)              | −0.310                   |
| 533   | $A_1$             | 198        | 2.7      | 3625.99467(5)              | −0.339                   |
| 534   | $A_1$             | 178        | 6.2      | 3632.5196(1)               | −0.346                   |
| 535   | $E$               | 192        | 4.0      | 3637.50561(9)              | −0.259                   |
| 536   | $E$               | 196        | 4.0      | 3637.50561(9)              | −0.333                   |
| 537   | $A_2$             | 186        | 3.9      | 3637.65886(6)              | −0.265                   |
| 538   | $A_1$             | 186        | 6.1      | 3641.18741(6)              | −0.336                   |
| 539   | $E$               | 195        | 0.16     | 3662.337842(8)             | −0.188                   |
| 540   | $E$               | 194        | 0.16     | 3662.337842(7)             | −0.213                   |
| 541   | $E$               | 187        | 1.1      | 3665.37573(5)              | −0.153                   |
| 542   | $E$               | 258        | 1.1      | 3665.37574(4)              | −0.176                   |
| 543   | $A_1$             | 275        | 4.3      | 3665.80277(8)              | −0.188                   |
| 544   | $E$               | 239        | 2.6      | 3665.9074(1)               | −0.192                   |
| 545   | $E$               | 242        | 2.5      | 3665.9074(1)               | −0.303                   |
| 546   | $E$               | 203        | 2.2      | 3666.0633(1)               | −0.182                   |
| 547   | $E$               | 211        | 2.2      | 3666.06334(9)              | −0.242                   |
| 548   | $E$               | 218        | 2.6      | 3666.8390(1)               | −0.183                   |
| 549   | $E$               | 243        | 2.6      | 3666.8390(1)               | −0.207                   |
| 550   | $A_1$             | 212        | 1.5      | 3667.74603(4)              | −0.177                   |
| 551   | $A_2$             | 233        | 1.5      | 3667.74607(3)              | −0.194                   |
| 552   | $E$               | 245        | 3.3      | 3668.8260(1)               | −0.172                   |
| 553   | $E$               | 247        | 3.3      | 3668.8260(1)               | −0.177                   |
| 554   | $A_1$             | 246        | 3.1      | 3669.0270(1)               | −0.221                   |
| 555   | $A_2$             | 324        | 3.0      | 3669.03987(5)              | −0.225                   |
| 556   | $E$               | 248        | 3.3      | 3669.1070(1)               | −0.373                   |
| 557   | $E$               | 302        | 3.3      | 3669.1070(1)               | −0.379                   |
| 558   | $E$               | 285        | 2.0      | 3669.43458(2)              | −0.168                   |
| 559   | $E$               | 215        | 2.0      | 3669.43459(6)              | −0.209                   |
| 560   | $A_1$             | 293        | 3.3      | 3669.66814(4)              | −0.384                   |
| 561   | $E$               | 225        | 3.4      | 3670.1335(1)               | −0.183                   |
| 562   | $E$               | 221        | 3.4      | 3670.1335(1)               | −0.227                   |
| 563   | $E$               | 172        | 2.4      | 3670.4947(2)               | −0.124                   |
| 564   | $E$               | 191        | 2.4      | 3670.4947(2)               | −0.215                   |
| 565   | $A_1$             | 208        | 4.1      | 3670.5761(3)               | −0.222                   |
| 566   | $A_2$             | 230        | 2.8      | 3670.6904(1)               | −0.180                   |
| 567   | $A_1$             | 307        | 3.4      | 3670.89056(3)              | −0.239                   |
| 568   | $E$               | 203        | 2.5      | 3671.5707(1)               | −0.093                   |
| 569   | $E$               | 204        | 2.5      | 3671.5707(1)               | −0.243                   |
| 570   | $A_2$             | 275        | 5.5      | 3671.57531(7)              | −0.290                   |
| 571   | $A_1$             | 269        | 7.5      | 3671.7204(1)               | −0.325                   |
| 572   | $E$               | 196        | 1.6      | 3673.26482(7)              | −0.303                   |
| 573   | $E$               | 234        | 1.5      | 3673.26483(6)              | −0.592                   |
| 574   | $E$               | 313        | 4.3      | 3674.43340(4)              | −0.267                   |
| 575   | $E$               | 297        | 4.3      | 3674.43341(5)              | −0.322                   |
| 576   | $E$               | 265        | 2.9      | 3675.70055(5)              | −0.226                   |
| 577   | $E$               | 269        | 2.9      | 3675.70056(6)              | −0.281                   |
| 578   | $A_1$             | 247        | 7.1      | 3677.4351(1)               | −0.331                   |

Continued on next page.

TABLE S3 – States on Sarka/Poirier USC PES; continued from previous page.

| State | $\Gamma_{C_{3v}}$ | $D_{\max}$ | $S_{vN}$ | $\tilde{E}/\text{cm}^{-1}$ | $\Delta\text{Ref. [30]}$ |
|-------|-------------------|------------|----------|----------------------------|--------------------------|
| 579   | $E$               | 244        | 5.6      | 3681.1538(1)               | −0.274                   |
| 580   | $E$               | 245        | 5.6      | 3681.1538(1)               | −0.333                   |
| 581   | $A_2$             | 253        | 5.8      | 3682.41663(7)              | −0.259                   |
| 582   | $A_1$             | 298        | 6.9      | 3685.13044(3)              | −0.342                   |
| 583   | $E$               | 233        | 2.4      | 3688.48904(4)              | −0.199                   |
| 584   | $E$               | 246        | 2.4      | 3688.48904(2)              | −0.211                   |
| 585   | $A_1$             | 231        | 2.6      | 3689.08538(1)              | −0.201                   |
| 586   | $A_2$             | 260        | 2.6      | 3689.08561(1)              | −0.214                   |
| 587   | $E$               | 203        | 0.62     | 3689.434366(9)             | −0.180                   |
| 588   | $E$               | 205        | 0.62     | 3689.434369(8)             | −0.229                   |
| 589   | $E$               | 175        | 1.6      | 3691.97466(5)              | −0.274                   |
| 590   | $E$               | 206        | 1.6      | 3691.97467(4)              | −0.275                   |
| 591   | $E$               | 176        | 1.8      | 3693.69859(6)              | −0.276                   |
| 592   | $E$               | 239        | 1.8      | 3693.69859(5)              | −0.305                   |
| 593   | $A_1$             | 174        | 1.9      | 3694.27379(5)              | −0.301                   |
| 594   | $E$               | 198        | 2.3      | 3702.82906(1)              | −0.475                   |
| 595   | $E$               | 181        | 2.3      | 3702.82906(2)              | −0.482                   |
| 596   | $A_1$             | 193        | 2.4      | 3703.48407(2)              | −0.486                   |
| 597   | $A_1$             | 124        | 1.5      | 3721.8869(2)               | −0.425                   |
| 598   | $A_2$             | 121        | 1.5      | 3721.8879(2)               | −0.441                   |
| 599   | $E$               | 206        | 2.4      | 3722.02464(1)              | −0.466                   |
| 600   | $E$               | 223        | 2.4      | 3722.02464(1)              | −0.753                   |
| 601   | $E$               | 150        | 1.5      | 3729.763583(6)             | −0.239                   |
| 602   | $E$               | 146        | 1.5      | 3729.763587(7)             | −0.352                   |
| 603   | $E$               | 323        | 5.1      | 3731.25620(3)              | −0.257                   |
| 604   | $E$               | 230        | 5.1      | 3731.2562(1)               | −0.299                   |
| 605   | $E$               | 235        | 5.6      | 3733.1211(1)               | −0.263                   |
| 606   | $E$               | 244        | 5.6      | 3733.1211(1)               | −0.269                   |
| 607   | $A_1$             | 224        | 5.8      | 3733.7544(1)               | −0.323                   |
| 608   | $A_2$             | 187        | 3.0      | 3736.4163(4)               | −0.259                   |
| 609   | $A_1$             | 181        | 3.0      | 3736.4163(4)               | −0.292                   |
| 610   | $E$               | 323        | 3.9      | 3737.94095(4)              | −0.255                   |
| 611   | $E$               | 243        | 3.9      | 3737.9410(2)               | −0.275                   |
| 612   | $E$               | 326        | 4.0      | 3738.92164(3)              | −0.258                   |
| 613   | $E$               | 262        | 4.0      | 3738.92164(8)              | −0.292                   |
| 614   | $A_2$             | 223        | 3.8      | 3739.2710(1)               | −0.258                   |
| 615   | $E$               | 209        | 4.5      | 3742.3090(1)               | −0.282                   |
| 616   | $E$               | 226        | 4.5      | 3742.3091(1)               | −0.298                   |
| 617   | $E$               | 231        | 5.0      | 3742.8085(1)               | −0.283                   |
| 618   | $E$               | 231        | 5.0      | 3742.8085(1)               | −0.300                   |
| 619   | $A_1$             | 224        | 5.1      | 3742.9406(1)               | −0.350                   |
| 620   | $E$               | 249        | 3.8      | 3769.252356(9)             | −0.236                   |
| 621   | $E$               | 241        | 3.8      | 3769.25237(1)              | −0.280                   |
| 622   | $A_1$             | 236        | 2.9      | 3773.15188(4)              | −0.404                   |
| 623   | $A_2$             | 216        | 2.9      | 3773.16505(2)              | −0.401                   |
| 624   | $E$               | 271        | 7.9      | 3773.42683(2)              | −0.224                   |
| 625   | $E$               | 273        | 7.9      | 3773.42683(1)              | −0.421                   |
| 626   | $E$               | 265        | 8.1      | 3773.56543(4)              | −0.453                   |
| 627   | $E$               | 259        | 8.1      | 3773.56544(5)              | −0.468                   |
| 628   | $E$               | 218        | 1.7      | 3774.00709(1)              | −0.319                   |
| 629   | $E$               | 224        | 1.6      | 3774.00709(1)              | −0.583                   |
| 630   | $A_1$             | 262        | 3.9      | 3775.32373(1)              | −0.145                   |
| 631   | $A_2$             | 272        | 3.8      | 3775.36215(1)              | −0.200                   |
| 632   | $E$               | 267        | 2.6      | 3775.53113(2)              | −0.206                   |
| 633   | $E$               | 266        | 2.6      | 3775.53114(1)              | −0.378                   |
| 634   | $E$               | 229        | 4.3      | 3780.23389(1)              | −0.205                   |
| 635   | $E$               | 237        | 4.3      | 3780.233890(8)             | −0.376                   |
| 636   | $E$               | 269        | 6.2      | 3787.01032(2)              | −0.203                   |
| 637   | $E$               | 290        | 6.2      | 3787.01033(2)              | −0.436                   |

Continued on next page.

TABLE S3 – States on Sarka/Poirier USC PES; continued from previous page.

| State | $\Gamma_{C_{3v}}$ | $D_{\max}$ | $S_{vN}$ | $\tilde{E}/\text{cm}^{-1}$ | $\Delta\text{Ref. [30]}$ |
|-------|-------------------|------------|----------|----------------------------|--------------------------|
| 638   | $E$               | 281        | 6.2      | 3792.29387(4)              | −0.278                   |
| 639   | $E$               | 304        | 6.2      | 3792.29387(3)              | −0.346                   |
| 640   | $A_1$             | 325        | 4.4      | 3794.55632(2)              | −0.251                   |
| 641   | $A_2$             | 319        | 4.3      | 3794.61089(2)              | −0.252                   |
| 642   | $E$               | 287        | 3.4      | 3796.69834(1)              | −0.159                   |
| 643   | $E$               | 287        | 3.4      | 3796.69834(1)              | −0.282                   |
| 644   | $E$               | 317        | 5.2      | 3801.15132(3)              | −0.276                   |
| 645   | $E$               | 299        | 5.3      | 3801.15133(2)              | −0.344                   |
| 646   | $A_1$             | 269        | 5.5      | 3803.59447(8)              | −0.313                   |
| 647   | $A_2$             | 318        | 5.4      | 3803.81287(3)              | −0.256                   |
| 648   | $E$               | 289        | 6.6      | 3804.11598(4)              | −0.220                   |
| 649   | $E$               | 262        | 6.7      | 3804.11599(8)              | −0.379                   |
| 650   | $E$               | 144        | 0.92     | 3808.15932(8)              | −0.248                   |
| 651   | $E$               | 155        | 0.92     | 3808.15933(6)              | −0.268                   |
| 652   | $A_1$             | 138        | 2.1      | 3809.9809(2)               | −0.239                   |
| 653   | $A_2$             | 134        | 2.1      | 3809.9810(2)               | −0.276                   |
| 654   | $E$               | 187        | 2.7      | 3811.27678(5)              | −0.246                   |
| 655   | $E$               | 181        | 2.7      | 3811.27679(6)              | −0.269                   |
| 656   | $E$               | 207        | 2.9      | 3812.05220(2)              | −0.234                   |
| 657   | $E$               | 206        | 2.9      | 3812.05220(2)              | −0.290                   |
| 658   | $A_1$             | 211        | 3.0      | 3812.31027(2)              | −0.331                   |
| 659   | $E$               | 314        | 2.7      | 3812.42556(2)              | −0.234                   |
| 660   | $E$               | 309        | 2.7      | 3812.42556(2)              | −0.257                   |
| 661   | $A_1$             | 229        | 3.4      | 3814.4958(1)               | −0.277                   |
| 662   | $A_2$             | 251        | 3.2      | 3815.18827(5)              | −0.226                   |
| 663   | $E$               | 288        | 5.6      | 3816.69220(1)              | −0.227                   |
| 664   | $E$               | 291        | 5.6      | 3816.69220(1)              | −0.277                   |
| 665   | $A_1$             | 219        | 0.9      | 3826.063345(6)             | −0.442                   |
| 666   | $E$               | 298        | 2.7      | 3827.44148(3)              | −0.218                   |
| 667   | $E$               | 216        | 2.7      | 3827.4415(1)               | −0.269                   |
| 668   | $A_1$             | 193        | 2.9      | 3827.9555(3)               | −0.266                   |
| 669   | $A_2$             | 187        | 2.9      | 3827.9590(3)               | −0.266                   |
| 670   | $E$               | 210        | 3.2      | 3828.9290(1)               | −0.208                   |
| 671   | $E$               | 217        | 3.2      | 3828.9290(1)               | −0.268                   |
| 672   | $A_1$             | 196        | 3.2      | 3829.1340(4)               | −0.226                   |
| 673   | $A_2$             | 207        | 3.2      | 3829.1595(3)               | −0.227                   |
| 674   | $E$               | 215        | 2.8      | 3829.9906(1)               | −0.150                   |
| 675   | $E$               | 214        | 2.8      | 3829.9906(1)               | −0.341                   |
| 676   | $E$               | 201        | 0.78     | 3834.70366(1)              | −0.277                   |
| 677   | $E$               | 211        | 0.78     | 3834.703660(9)             | −0.438                   |
| 678   | $A_1$             | 199        | 2.4      | 3847.704709(6)             | −0.439                   |
| 679   | $E$               | 171        | 1.6      | 3851.59348(2)              | −1.045                   |
| 680   | $E$               | 193        | 1.6      | 3851.59348(2)              | −1.109                   |
| 681   | $A_1$             | 245        | 4.8      | 3852.3536(1)               | −0.356                   |
| 682   | $A_2$             | 237        | 4.8      | 3852.3538(1)               | −0.766                   |
| 683   | $E$               | 229        | 4.7      | 3854.3026(1)               | −0.267                   |
| 684   | $E$               | 272        | 4.7      | 3854.3026(1)               | −0.376                   |
| 685   | $E$               | 193        | 3.2      | 3855.50485(4)              | −0.360                   |
| 686   | $E$               | 191        | 3.2      | 3855.50485(5)              | −0.379                   |
| 687   | $A_1$             | 182        | 3.3      | 3856.04708(7)              | −0.369                   |
| 688   | $E$               | 258        | 4.5      | 3862.6611(2)               | −0.244                   |
| 689   | $E$               | 319        | 4.5      | 3862.6611(2)               | −0.267                   |
| 690   | $A_1$             | 234        | 6.0      | 3864.9010(5)               | −0.271                   |
| 691   | $A_2$             | 231        | 6.0      | 3864.9123(6)               | −0.297                   |
| 692   | $E$               | 253        | 5.7      | 3866.0773(2)               | −0.184                   |
| 693   | $E$               | 255        | 5.7      | 3866.0773(2)               | −0.387                   |
| 694   | $A_1$             | 233        | 6.5      | 3866.3150(5)               | −0.266                   |
| 695   | $A_2$             | 231        | 6.5      | 3866.3192(5)               | −0.270                   |
| 696   | $E$               | 191        | 0.54     | 3867.209833(8)             | −0.215                   |

Continued on next page.

TABLE S3 – States on Sarka/Poirier USC PES; continued from previous page.

| State | $\Gamma_{C_{3v}}$ | $D_{\max}$ | $S_{vN}$ | $\tilde{E}/\text{cm}^{-1}$ | $\Delta\text{Ref. [30]}$ |
|-------|-------------------|------------|----------|----------------------------|--------------------------|
| 697   | $E$               | 192        | 0.54     | 3867.209833(8)             | −0.245                   |
| 698   | $E$               | 261        | 5.5      | 3867.6860(2)               | −0.234                   |
| 699   | $E$               | 260        | 5.5      | 3867.6860(2)               | −0.290                   |
| 700   | $E$               | 268        | 5.0      | 3873.5003(2)               | −0.254                   |
| 701   | $E$               | 272        | 5.0      | 3873.5003(2)               | −0.269                   |
| 702   | $A_1$             | 238        | 5.9      | 3874.1840(5)               | −0.271                   |
| 703   | $A_2$             | 235        | 5.9      | 3874.1992(6)               | −0.269                   |
| 704   | $E$               | 338        | 5.5      | 3874.37562(5)              | −0.243                   |
| 705   | $E$               | 263        | 5.5      | 3874.3756(1)               | −0.345                   |
| 706   | $E$               | 250        | 2.8      | 3876.5687(1)               | −0.231                   |
| 707   | $E$               | 255        | 2.8      | 3876.56875(6)              | −0.239                   |
| 708   | $E$               | 344        | 4.1      | 3878.71256(7)              | −0.234                   |
| 709   | $E$               | 321        | 4.1      | 3878.7126(1)               | −0.245                   |
| 710   | $A_1$             | 267        | 5.2      | 3880.3419(1)               | −0.244                   |
| 711   | $A_2$             | 255        | 5.0      | 3880.3535(2)               | −0.248                   |
| 712   | $A_1$             | 192        | 2.4      | 3880.629317(7)             | −0.535                   |
| 713   | $E$               | 254        | 5.1      | 3881.4700(1)               | −0.220                   |
| 714   | $E$               | 254        | 5.1      | 3881.4700(1)               | −0.259                   |
| 715   | $A_1^*$           | 234        | 5.9      | 3881.9511(2)               | −0.217                   |
| 716   | $A_2^*$           | 211        | 5.9      | 3881.9511(4)               | −0.258                   |
| 717   | $E$               | 280        | 6.0      | 3882.0274(2)               | −0.285                   |
| 718   | $E$               | 282        | 6.0      | 3882.0274(2)               | −0.301                   |
| 719   | $E$               | 310        | 4.2      | 3883.36772(4)              | −0.380                   |
| 720   | $E$               | 234        | 4.2      | 3883.3677(1)               | −0.420                   |
| 721   | $A_1$             | 232        | 4.6      | 3883.7889(1)               | −0.430                   |
| 722   | $E$               | 232        | 3.3      | 3885.4031(1)               | −0.360                   |
| 723   | $E$               | 229        | 3.3      | 3885.4031(1)               | −0.393                   |
| 724   | $E$               | 226        | 3.7      | 3886.0239(1)               | −0.310                   |
| 725   | $E$               | 227        | 3.7      | 3886.0239(1)               | −0.373                   |
| 726   | $A_2$             | 236        | 3.7      | 3886.23924(9)              | −0.345                   |
| 727   | $A_2$             | 247        | 6.0      | 3894.63613(3)              | −0.249                   |
| 728   | $E$               | 262        | 5.1      | 3898.46072(4)              | −0.262                   |
| 729   | $E$               | 287        | 5.1      | 3898.46072(2)              | −0.267                   |
| 730   | $E$               | 186        | 3.7      | 3898.9457(1)               | −0.393                   |
| 731   | $E$               | 191        | 3.7      | 3898.9457(1)               | −0.486                   |
| 732   | $A_1$             | 197        | 3.9      | 3899.1313(1)               | −0.437                   |
| 733   | $A_1$             | 327        | 4.2      | 3900.234966(9)             | −0.288                   |
| 734   | $A_1$             | 281        | 5.9      | 3901.23796(2)              | −0.264                   |
| 735   | $A_2$             | 282        | 5.5      | 3903.86687(2)              | −0.254                   |
| 736   | $E$               | 275        | 5.7      | 3904.28707(2)              | −0.213                   |
| 737   | $E$               | 322        | 5.7      | 3904.28708(3)              | −0.288                   |
| 738   | $E$               | 278        | 4.4      | 3909.29575(2)              | −0.218                   |
| 739   | $E$               | 285        | 4.5      | 3909.29575(2)              | −0.228                   |
| 740   | $A_2$             | 312        | 5.1      | 3910.00929(1)              | −0.243                   |
| 741   | $A_1$             | 289        | 6.3      | 3912.04497(1)              | −0.241                   |
| 742   | $E$               | 267        | 3.6      | 3912.33451(2)              | −0.225                   |
| 743   | $E$               | 263        | 3.6      | 3912.33451(3)              | −0.226                   |
| 744   | $E$               | 276        | 5.5      | 3914.69152(2)              | −0.208                   |
| 745   | $E$               | 275        | 5.5      | 3914.69152(2)              | −0.261                   |
| 746   | $E$               | 192        | 3.8      | 3938.9545(1)               | −0.258                   |
| 747   | $E$               | 215        | 3.8      | 3938.9546(1)               | −0.263                   |
| 748   | $E$               | 212        | 4.2      | 3942.4582(1)               | −0.279                   |
| 749   | $E$               | 208        | 4.2      | 3942.4582(1)               | −0.281                   |
| 750   | $A_1$             | 175        | 4.4      | 3944.8603(3)               | −0.271                   |
| 751   | $A_2$             | 176        | 4.4      | 3944.8624(3)               | −0.274                   |
| 752   | $E$               | 201        | 4.4      | 3946.0888(1)               | −0.172                   |
| 753   | $E$               | 231        | 4.4      | 3946.0888(1)               | −0.373                   |
| 754   | $A_2^*$           | 186        | 1.4      | 3948.18992(4)              | −0.333                   |
| 755   | $A_1^*$           | 246        | 1.4      | 3948.18992(3)              | −0.337                   |

Continued on next page.

TABLE S3 – States on Sarka/Poirier USC PES; continued from previous page.

| State | $\Gamma_{C_{3v}}$ | $D_{\max}$ | $S_{vN}$ | $\tilde{E}/\text{cm}^{-1}$ | $\Delta\text{Ref. [30]}$ |
|-------|-------------------|------------|----------|----------------------------|--------------------------|
| 756   | $E$               | 199        | 2.7      | 3948.92148(5)              | −0.375                   |
| 757   | $E$               | 183        | 2.7      | 3948.92148(7)              | −0.413                   |
| 758   | $E$               | 150        | 3.2      | 3949.3608(1)               | −0.355                   |
| 759   | $E$               | 266        | 3.2      | 3949.3608(1)               | −0.508                   |
| 760   | $A_1$             | 144        | 3.4      | 3949.5074(2)               | −0.610                   |
| 761   | $A_2^*$           | 167        | 2.6      | 3950.6246(3)               | −0.225                   |
| 762   | $A_1^*$           | 166        | 2.6      | 3950.6246(3)               | −0.248                   |
| 763   | $E$               | 199        | 1.8      | 3951.20574(2)              | −0.342                   |
| 764   | $E$               | 210        | 1.8      | 3951.20574(1)              | −0.643                   |
| 765   | $E$               | 331        | 4.3      | 3952.80331(3)              | −0.217                   |
| 766   | $E$               | 247        | 4.3      | 3952.8033(1)               | −0.232                   |
| 767   | $E$               | 256        | 5.0      | 3954.5587(1)               | −0.235                   |
| 768   | $E$               | 260        | 5.0      | 3954.5587(1)               | −0.272                   |
| 769   | $E$               | 300        | 4.3      | 3954.61864(4)              | −0.258                   |
| 770   | $E$               | 265        | 4.3      | 3954.61864(7)              | −0.266                   |
| 771   | $A_1$             | 253        | 5.3      | 3955.7819(1)               | −0.249                   |
| 772   | $A_2$             | 259        | 5.3      | 3955.7950(1)               | −0.254                   |
| 773   | $E$               | 273        | 6.0      | 3956.3530(2)               | −0.250                   |
| 774   | $E$               | 316        | 6.0      | 3956.3531(2)               | −0.262                   |
| 775   | $E$               | 246        | 4.4      | 3956.3998(1)               | −0.218                   |
| 776   | $E$               | 280        | 4.4      | 3956.3998(1)               | −0.232                   |
| 777   | $E$               | 323        | 5.3      | 3956.43415(3)              | −0.217                   |
| 778   | $E$               | 265        | 5.3      | 3956.43416(7)              | −0.393                   |
| 779   | $E$               | 310        | 5.8      | 3957.0037(1)               | −0.271                   |
| 780   | $E$               | 294        | 5.8      | 3957.0037(1)               | −0.288                   |
| 781   | $A_2$             | 215        | 4.2      | 3957.4545(4)               | −0.209                   |
| 782   | $A_1$             | 202        | 4.1      | 3957.4608(4)               | −0.202                   |
| 783   | $A_2$             | 329        | 6.0      | 3957.85211(8)              | −0.244                   |
| 784   | $E$               | 254        | 3.2      | 3957.93106(8)              | −0.188                   |
| 785   | $E$               | 255        | 3.2      | 3957.93107(9)              | −0.288                   |
| 786   | $E$               | 286        | 5.8      | 3958.7248(1)               | −0.207                   |
| 787   | $E$               | 286        | 5.9      | 3958.7248(1)               | −0.310                   |
| 788   | $A_1$             | 269        | 5.5      | 3959.5854(1)               | −0.264                   |
| 789   | $E$               | 316        | 5.2      | 3965.32817(8)              | −0.223                   |
| 790   | $E$               | 335        | 5.2      | 3965.32817(7)              | −0.257                   |
| 791   | $E$               | 241        | 1.2      | 3965.89783(1)              | −0.117                   |
| 792   | $E$               | 238        | 1.2      | 3965.89783(2)              | −0.519                   |
| 793   | $E$               | 356        | 5.3      | 3966.65357(5)              | −0.185                   |
| 794   | $E$               | 283        | 5.3      | 3966.6536(1)               | −0.226                   |
| 795   | $A_2$             | 264        | 5.1      | 3967.05477(8)              | −0.222                   |
| 796   | $A_1$             | 224        | 3.6      | 3968.1131(1)               | −0.214                   |
| 797   | $A_2$             | 220        | 3.6      | 3968.1131(2)               | −0.227                   |
| 798   | $E$               | 347        | 5.0      | 3969.56440(7)              | −0.167                   |
| 799   | $E$               | 294        | 5.0      | 3969.5644(1)               | −0.215                   |
| 800   | $E$               | 331        | 4.3      | 3970.38482(6)              | −0.193                   |
| 801   | $E$               | 292        | 4.3      | 3970.38484(9)              | −0.246                   |
| 802   | $A_1$             | 334        | 4.1      | 3970.66069(3)              | −0.234                   |
| 803   | $E$               | 302        | 6.2      | 3970.7745(1)               | −0.238                   |
| 804   | $E$               | 308        | 6.2      | 3970.7745(1)               | −0.252                   |
| 805   | $E$               | 319        | 5.6      | 3971.61872(9)              | −0.218                   |
| 806   | $E$               | 275        | 5.6      | 3971.6187(1)               | −0.230                   |
| 807   | $A_2$             | 309        | 5.7      | 3972.06823(9)              | −0.211                   |
| 808   | $E$               | 287        | 6.2      | 3972.2540(1)               | −0.184                   |
| 809   | $E$               | 290        | 6.2      | 3972.2540(1)               | −0.308                   |
| 810   | $A_1$             | 280        | 6.4      | 3972.7436(1)               | −0.271                   |
| 811   | $E$               | 229        | 3.1      | 3977.954594(8)             | −0.381                   |
| 812   | $E$               | 240        | 3.1      | 3977.954597(8)             | −0.533                   |
| 813   | $A_1$             | 237        | 0.68     | 3981.791836(9)             | −0.405                   |
| 814   | $A_2$             | 240        | 0.51     | 3982.921925(6)             | −0.233                   |

Continued on next page.

TABLE S3 – States on Sarka/Poirier USC PES; continued from previous page.

| State | $\Gamma_{C_{3v}}$ | $D_{\max}$ | $S_{vN}$ | $\tilde{E}/\text{cm}^{-1}$ | $\Delta\text{Ref. [30]}$ |
|-------|-------------------|------------|----------|----------------------------|--------------------------|
| 815   | $A_1$             | 182        | 2.9      | 3984.0955(3)               | −0.311                   |
| 816   | $A_2$             | 181        | 2.9      | 3984.1054(2)               | −0.328                   |
| 817   | $E$               | 210        | 2.9      | 3984.2606(1)               | −0.323                   |
| 818   | $E$               | 205        | 2.8      | 3984.2606(1)               | −0.392                   |
| 819   | $E$               | 207        | 2.5      | 3984.9111(1)               | −0.322                   |
| 820   | $E$               | 203        | 2.5      | 3984.9111(1)               | −0.404                   |
| 821   | $E$               | 202        | 6.2      | 3990.6466(1)               | −0.373                   |
| 822   | $E$               | 231        | 6.2      | 3990.6466(1)               | −0.406                   |
| 823   | $A_1$             | 222        | 4.0      | 3996.7856(1)               | −0.325                   |
| 824   | $A_2$             | 220        | 4.0      | 3996.7859(1)               | −0.383                   |
| 825   | $E$               | 224        | 3.3      | 3997.4287(1)               | −0.313                   |
| 826   | $E$               | 216        | 3.3      | 3997.4287(1)               | −0.322                   |
| 827   | $E$               | 231        | 3.2      | 3998.65996(1)              | −0.247                   |
| 828   | $E$               | 245        | 3.2      | 3998.659960(7)             | −0.267                   |
| 829   | $E$               | 202        | 6.1      | 4000.6908(1)               | −0.365                   |
| 830   | $E$               | 202        | 6.1      | 4000.6908(1)               | −0.394                   |
| 831   | $A_2$             | 228        | 2.5      | 4004.167252(9)             | −0.207                   |
| 832   | $A_1$             | 249        | 2.7      | 4004.693583(5)             | −0.241                   |
| 833   | $A_1$             | 148        | 4.1      | 4011.34261(7)              | −0.600                   |
| 834   | $E$               | 218        | 2.8      | 4012.072861(9)             | −0.312                   |
| 835   | $E$               | 220        | 2.8      | 4012.072862(8)             | −0.534                   |
| 836   | $E$               | 270        | 5.4      | 4025.7247(2)               | −0.219                   |
| 837   | $E$               | 295        | 5.4      | 4025.7247(2)               | −0.325                   |
| 838   | $A_1$             | 265        | 3.0      | 4025.9333(2)               | −0.416                   |
| 839   | $A_2$             | 315        | 2.9      | 4025.93861(9)              | −0.482                   |
| 840   | $A_1$             | 204        | 4.0      | 4027.2389(1)               | −0.536                   |
| 841   | $E$               | 220        | 3.4      | 4027.9886(1)               | −0.431                   |
| 842   | $E$               | 286        | 3.4      | 4027.9886(1)               | −0.650                   |
| 843   | $A_2$             | 249        | 3.3      | 4028.01946(4)              | −0.785                   |
| 844   | $E$               | 317        | 7.5      | 4030.3674(1)               | −0.352                   |
| 845   | $E$               | 299        | 7.5      | 4030.3674(2)               | −0.380                   |
| 846   | $A_2$             | 240        | 2.7      | 4032.7358(1)               | −0.419                   |
| 847   | $A_1$             | 242        | 2.7      | 4032.7361(1)               | −0.442                   |
| 848   | $E$               | 363        | 7.2      | 4033.26522(7)              | −0.339                   |
| 849   | $E$               | 317        | 7.2      | 4033.2652(1)               | −0.387                   |
| 850   | $E$               | 323        | 4.2      | 4034.03609(5)              | −0.302                   |
| 851   | $E$               | 266        | 4.2      | 4034.0361(1)               | −0.337                   |
| 852   | $E$               | 231        | 2.2      | 4034.15281(6)              | −0.274                   |
| 853   | $E$               | 261        | 2.2      | 4034.15281(6)              | −0.319                   |
| 854   | $E$               | 194        | 0.2      | 4034.70177(1)              | −0.223                   |
| 855   | $E$               | 192        | 0.21     | 4034.70177(1)              | −0.241                   |
| 856   | $A_1$             | 308        | 2.6      | 4035.03208(3)              | −0.218                   |
| 857   | $A_2$             | 268        | 2.6      | 4035.03208(4)              | −0.239                   |
| 858   | $A_1$             | 265        | 5.9      | 4035.6010(4)               | −0.353                   |
| 859   | $A_2$             | 260        | 5.9      | 4035.6257(5)               | −0.338                   |
| 860   | $E$               | 273        | 3.1      | 4036.2497(1)               | −0.295                   |
| 861   | $E$               | 309        | 3.1      | 4036.2497(1)               | −0.373                   |
| 862   | $E$               | 316        | 6.8      | 4036.9641(1)               | −0.364                   |
| 863   | $E$               | 305        | 6.8      | 4036.9641(1)               | −0.387                   |
| 864   | $A_2$             | 208        | 2.9      | 4037.1934(4)               | −0.196                   |
| 865   | $A_1$             | 208        | 2.9      | 4037.1935(4)               | −0.202                   |
| 866   | $E$               | 265        | 3.0      | 4037.4873(1)               | −0.245                   |
| 867   | $E$               | 281        | 3.0      | 4037.4873(1)               | −0.252                   |
| 868   | $A_2$             | 291        | 1.3      | 4037.67489(1)              | −0.189                   |
| 869   | $A_1$             | 291        | 1.3      | 4037.67490(1)              | −0.214                   |
| 870   | $E$               | 250        | 3.1      | 4038.9814(1)               | −0.221                   |
| 871   | $E$               | 240        | 3.1      | 4038.9814(1)               | −0.242                   |
| 872   | $E$               | 255        | 3.2      | 4039.3422(1)               | −0.204                   |
| 873   | $E$               | 244        | 3.2      | 4039.3422(1)               | −0.246                   |

Continued on next page.

TABLE S3 – States on Sarka/Poirier USC PES; continued from previous page.

| State | $\Gamma_{C_{3v}}$ | $D_{\max}$ | $S_{vN}$ | $\tilde{E}/\text{cm}^{-1}$ | $\Delta\text{Ref. [30]}$ |
|-------|-------------------|------------|----------|----------------------------|--------------------------|
| 874   | $A_2$             | 218        | 3.2      | 4039.4861(1)               | −0.236                   |
| 875   | $E$               | 221        | 1.8      | 4040.02984(6)              | −0.225                   |
| 876   | $E$               | 214        | 1.8      | 4040.02985(7)              | −0.227                   |
| 877   | $E$               | 259        | 3.2      | 4040.6214(1)               | −0.172                   |
| 878   | $E$               | 250        | 3.2      | 4040.6214(1)               | −0.235                   |
| 879   | $A_1$             | 244        | 6.4      | 4040.7429(6)               | −0.352                   |
| 880   | $A_2$             | 247        | 6.3      | 4040.7456(5)               | −0.402                   |
| 881   | $A_1$             | 261        | 3.3      | 4041.0450(1)               | −0.304                   |
| 882   | $E$               | 205        | 1.9      | 4041.77498(7)              | −0.220                   |
| 883   | $E$               | 235        | 1.9      | 4041.77499(6)              | −0.268                   |
| 884   | $E$               | 271        | 5.7      | 4042.5226(2)               | −0.343                   |
| 885   | $E$               | 268        | 5.7      | 4042.5227(2)               | −0.348                   |
| 886   | $A_1$             | 147        | 2.0      | 4042.9248(2)               | −0.230                   |
| 887   | $A_2$             | 145        | 1.9      | 4042.9352(2)               | −0.233                   |
| 888   | $E$               | 225        | 1.9      | 4043.50574(2)              | −0.162                   |
| 889   | $E$               | 224        | 1.9      | 4043.50574(2)              | −0.432                   |
| 890   | $E$               | 266        | 7.2      | 4045.2938(2)               | −0.381                   |
| 891   | $E$               | 310        | 7.2      | 4045.2938(2)               | −0.412                   |
| 892   | $E$               | 271        | 2.4      | 4052.09350(3)              | −0.221                   |
| 893   | $E$               | 253        | 2.4      | 4052.09351(1)              | −0.238                   |
| 894   | $E$               | 276        | 2.7      | 4052.98913(4)              | −0.224                   |
| 895   | $E$               | 252        | 2.7      | 4052.98915(2)              | −0.238                   |
| 896   | $A_1$             | 242        | 2.7      | 4053.59373(4)              | −0.224                   |
| 897   | $A_2$             | 261        | 2.7      | 4053.63333(2)              | −0.216                   |
| 898   | $E$               | 243        | 2.8      | 4053.91300(5)              | −0.220                   |
| 899   | $E$               | 202        | 2.8      | 4053.9130(1)               | −0.227                   |
| 900   | $A_1$             | 188        | 3.7      | 4054.70558(1)              | −0.725                   |
| 901   | $E$               | 187        | 1.6      | 4055.27140(5)              | −0.314                   |
| 902   | $E$               | 187        | 1.6      | 4055.27140(5)              | −0.326                   |
| 903   | $A_1$             | 146        | 1.9      | 4057.4161(2)               | −0.326                   |
| 904   | $A_2$             | 144        | 1.9      | 4057.4175(2)               | −0.363                   |
| 905   | $E$               | 183        | 2.0      | 4058.49081(5)              | −0.307                   |
| 906   | $E$               | 182        | 2.0      | 4058.49081(5)              | −0.381                   |
| 907   | $A_1$             | 157        | 2.3      | 4066.3036(2)               | −0.515                   |
| 908   | $A_2$             | 164        | 2.3      | 4066.3045(1)               | −0.555                   |
| 909   | $E$               | 214        | 2.5      | 4067.54072(2)              | −0.507                   |
| 910   | $E$               | 215        | 2.5      | 4067.54073(3)              | −0.560                   |
| 911   | $A_1$             | 180        | 3.6      | 4071.34700(7)              | −0.305                   |
| 912   | $E$               | 202        | 3.1      | 4071.37669(1)              | −0.442                   |
| 913   | $E$               | 217        | 3.1      | 4071.37669(1)              | −0.700                   |
| 914   | $A_2$             | 197        | 2.4      | 4072.473794(6)             | −0.472                   |
| 915   | $A_1$             | 187        | 3.2      | 4081.38739(6)              | −0.492                   |
| 916   | $E$               | 181        | 3.0      | 4081.39857(6)              | −0.567                   |
| 917   | $E$               | 200        | 3.0      | 4081.39858(6)              | −0.653                   |
| 918   | $E$               | 187        | 1.8      | 4081.45610(5)              | −0.947                   |
| 919   | $E$               | 211        | 1.8      | 4081.45610(4)              | −1.184                   |
| 920   | $A_1$             | 217        | 2.6      | 4085.79114(3)              | −0.395                   |
| 921   | $A_2$             | 197        | 3.5      | 4088.27380(7)              | −0.283                   |
| 922   | $E$               | 206        | 3.5      | 4088.37687(6)              | −0.315                   |
| 923   | $E$               | 200        | 3.5      | 4088.37687(5)              | −0.381                   |
| 924   | $A_1$             | 216        | 3.5      | 4088.71320(5)              | −0.343                   |
| 925   | $E$               | 211        | 1.4      | 4092.29584(3)              | −0.217                   |
| 926   | $E$               | 259        | 1.4      | 4092.29584(2)              | −0.382                   |
| 927   | $E$               | 238        | 5.2      | 4095.2650(1)               | −0.328                   |
| 928   | $E$               | 245        | 5.2      | 4095.2650(1)               | −0.370                   |
| 929   | $A_1$             | 222        | 5.9      | 4097.4404(3)               | −0.326                   |
| 930   | $A_2$             | 213        | 5.9      | 4097.4440(4)               | −0.375                   |
| 931   | $E$               | 247        | 6.0      | 4098.5434(1)               | −0.276                   |
| 932   | $E$               | 253        | 6.0      | 4098.5434(1)               | −0.512                   |

Continued on next page.



TABLE S3 – States on Sarka/Poirier USC PES; continued from previous page.

| State | $\Gamma_{C_{3v}}$ | $D_{\max}$ | $S_{vN}$ | $\tilde{E}/\text{cm}^{-1}$ | $\Delta\text{Ref. [30]}$ |
|-------|-------------------|------------|----------|----------------------------|--------------------------|
| 933   | $E$               | 237        | 3.2      | 4101.1068(1)               | −0.317                   |
| 934   | $E$               | 244        | 3.2      | 4101.1068(1)               | −0.347                   |
| 935   | $E$               | 268        | 4.5      | 4102.6371(2)               | −0.309                   |
| 936   | $E$               | 268        | 4.5      | 4102.6371(2)               | −0.355                   |
| 937   | $A_1$             | 214        | 4.9      | 4103.8101(4)               | −0.338                   |
| 938   | $A_2$             | 207        | 4.8      | 4103.8225(5)               | −0.326                   |
| 939   | $E$               | 236        | 3.8      | 4104.5327(1)               | −0.298                   |
| 940   | $E$               | 229        | 3.8      | 4104.5327(1)               | −0.351                   |
| 941   | $E$               | 325        | 4.7      | 4106.65360(3)              | −0.340                   |
| 942   | $E$               | 229        | 4.7      | 4106.6536(1)               | −0.353                   |
| 943   | $A_1$             | 201        | 5.5      | 4107.1166(5)               | −0.326                   |
| 944   | $A_2$             | 218        | 5.5      | 4107.1186(3)               | −0.335                   |
| 945   | $E$               | 246        | 5.5      | 4107.2064(1)               | −0.401                   |
| 946   | $E$               | 225        | 5.5      | 4107.2064(1)               | −0.518                   |
| 947   | $E$               | 211        | 0.45     | 4116.36810(1)              | −0.203                   |
| 948   | $E$               | 221        | 0.45     | 4116.36810(1)              | −0.352                   |
| 949   | $E$               | 333        | 5.1      | 4128.44747(5)              | −0.287                   |
| 950   | $E$               | 298        | 5.1      | 4128.44748(6)              | −0.301                   |
| 951   | $A_2$             | 278        | 5.6      | 4128.76347(8)              | −0.310                   |
| 952   | $A_1$             | 296        | 6.9      | 4131.53445(8)              | −0.301                   |
| 953   | $A_2$             | 298        | 6.2      | 4133.45918(4)              | −0.262                   |
| 954   | $E$               | 288        | 6.3      | 4133.5746(1)               | −0.297                   |
| 955   | $E$               | 313        | 6.3      | 4133.5746(1)               | −0.347                   |
| 956   | $A_1$             | 249        | 3.7      | 4133.9655(1)               | −0.414                   |
| 957   | $E$               | 336        | 4.4      | 4135.16637(5)              | −0.295                   |
| 958   | $E$               | 292        | 4.4      | 4135.1664(1)               | −0.307                   |
| 959   | $E$               | 199        | 1.1      | 4135.21092(2)              | −0.300                   |
| 960   | $E$               | 239        | 1.1      | 4135.21092(2)              | −0.548                   |
| 961   | $E$               | 282        | 4.1      | 4135.7132(1)               | −0.312                   |
| 962   | $E$               | 303        | 4.1      | 4135.7132(1)               | −0.378                   |
| 963   | $A_1$             | 285        | 4.0      | 4135.8838(1)               | −0.390                   |
| 964   | $E$               | 281        | 3.3      | 4136.74781(7)              | −0.439                   |
| 965   | $E$               | 248        | 3.3      | 4136.7478(1)               | −0.448                   |
| 966   | $E$               | 238        | 3.0      | 4137.1641(1)               | −0.568                   |
| 967   | $E$               | 258        | 3.0      | 4137.1641(1)               | −0.582                   |
| 968   | $E$               | 234        | 3.2      | 4138.1141(1)               | −0.377                   |
| 969   | $E$               | 245        | 3.2      | 4138.1141(1)               | −0.402                   |
| 970   | $A_1$             | 293        | 3.3      | 4138.24529(5)              | −0.598                   |
| 971   | $A_2$             | 233        | 3.0      | 4138.27992(3)              | −0.636                   |
| 972   | $E$               | 228        | 6.4      | 4139.8884(5)               | −0.270                   |
| 973   | $E$               | 328        | 6.4      | 4139.8885(5)               | −0.302                   |
| 974   | $A_2$             | 242        | 6.4      | 4140.0055(3)               | −0.407                   |
| 975   | $A_1$             | 287        | 6.5      | 4140.6058(1)               | −0.333                   |
| 976   | $E$               | 306        | 7.1      | 4146.8591(1)               | −0.354                   |
| 977   | $E$               | 311        | 7.1      | 4146.85913(9)              | −0.458                   |
| 978   | $A_1$             | 307        | 8.4      | 4147.3346(1)               | −0.455                   |
| 979   | $A_2$             | 290        | 6.1      | 4148.85902(8)              | −0.456                   |
| 980   | $E$               | 336        | 6.9      | 4154.01343(9)              | −0.342                   |
| 981   | $E$               | 336        | 6.9      | 4154.01343(9)              | −0.395                   |
| 982   | $A_1$             | 324        | 8.1      | 4154.1314(1)               | −0.402                   |
| 983   | $E$               | 328        | 4.8      | 4156.03974(3)              | −0.326                   |
| 984   | $E$               | 337        | 4.8      | 4156.03975(3)              | −0.342                   |
| 985   | $E$               | 305        | 5.0      | 4158.3524(1)               | −0.258                   |
| 986   | $E$               | 327        | 5.0      | 4158.35238(9)              | −0.354                   |
| 987   | $A_2$             | 333        | 4.9      | 4159.62525(7)              | −0.278                   |
| 988   | $A_1$             | 359        | 7.4      | 4161.79450(9)              | −0.379                   |
| 989   | $E$               | 331        | 6.0      | 4163.89621(5)              | −0.371                   |
| 990   | $E$               | 331        | 6.1      | 4163.89622(7)              | −0.379                   |
| 991   | $A_2$             | 301        | 7.7      | 4164.5585(1)               | −0.370                   |

Continued on next page.

TABLE S3 – States on Sarka/Poirier USC PES; continued from previous page.

| State | $\Gamma_{C_{3v}}$ | $D_{\max}$ | $S_{vN}$ | $\tilde{E}/\text{cm}^{-1}$ | $\Delta\text{Ref. [30]}$ |
|-------|-------------------|------------|----------|----------------------------|--------------------------|
| 992   | $E$               | 286        | 3.6      | 4165.33671(2)              | −0.361                   |
| 993   | $E$               | 217        | 3.6      | 4165.33671(8)              | −0.506                   |
| 994   | $E$               | 374        | 6.0      | 4165.95681(6)              | −0.362                   |
| 995   | $E$               | 368        | 6.0      | 4165.95681(7)              | −0.367                   |
| 996   | $E$               | 282        | 7.3      | 4166.5559(2)               | −0.226                   |
| 997   | $E$               | 334        | 7.3      | 4166.5559(2)               | −0.402                   |
| 998   | $A_1$             | 340        | 8.1      | 4166.55882(7)              | −0.450                   |
| 999   | $A_2$             | 305        | 2.9      | 4174.47169(4)              | −0.272                   |

TABLE S4: Same as Table S2 but for the CSC PES variant from Sarka and Poirier.

| State | $\Gamma_{C_{3v}}$ | $D_{\max}$ | $S_{vN}$ | $\tilde{E}/\text{cm}^{-1}$ | $\Delta\text{Ref. [30]}$ |
|-------|-------------------|------------|----------|----------------------------|--------------------------|
| 0     | $A_1$             | 31         | 0.0068   | 9914.94354(4)              | −0.003                   |
| 1     | $E$               | 31         | 0.0072   | 363.470376(1)              | 0.000                    |
| 2     | $E$               | 32         | 0.0072   | 363.4703761(9)             | −0.001                   |
| 3     | $E$               | 32         | 0.0078   | 728.459540(1)              | −0.000                   |
| 4     | $E$               | 36         | 0.0078   | 728.45954(4)               | −0.000                   |
| 5     | $A_1$             | 35         | 0.02     | 729.92844(7)               | −0.001                   |
| 6     | $A_1$             | 32         | 0.021    | 907.0054301(2)             | 0.000                    |
| 7     | $E$               | 42         | 0.01     | 1052.365945(6)             | −0.000                   |
| 8     | $E$               | 42         | 0.01     | 1052.365945(6)             | −0.000                   |
| 9     | $A_1$             | 35         | 0.0086   | 1094.948924(1)             | −0.000                   |
| 10    | $A_2$             | 36         | 0.0086   | 1094.9489276(6)            | −0.001                   |
| 11    | $E$               | 36         | 0.031    | 1097.8546011(4)            | −0.000                   |
| 12    | $E$               | 34         | 0.031    | 1097.8546014(7)            | −0.001                   |
| 13    | $E$               | 32         | 0.033    | 1269.786754(2)             | −0.000                   |
| 14    | $E$               | 33         | 0.033    | 1269.7867551(9)            | −0.026                   |
| 15    | $A_1$             | 41         | 0.092    | 1399.868739(3)             | −0.030                   |
| 16    | $A_1$             | 64         | 2.1      | 1415.730861(1)             | −0.014                   |
| 17    | $E$               | 51         | 2.0      | 1415.821132(4)             | −0.002                   |
| 18    | $E$               | 52         | 2.0      | 1415.821133(3)             | −0.019                   |
| 19    | $A_2$             | 51         | 2.0      | 1415.860836(2)             | −0.001                   |
| 20    | $E$               | 41         | 0.0096   | 1462.9205551(6)            | −0.002                   |
| 21    | $E$               | 42         | 0.0096   | 1462.9205552(5)            | −0.004                   |
| 22    | $E$               | 38         | 0.043    | 1467.2317164(8)            | −0.002                   |
| 23    | $E$               | 40         | 0.043    | 1467.23172(4)              | −0.015                   |
| 24    | $A_1$             | 39         | 0.053    | 1468.668971(4)             | −0.012                   |
| 25    | $E$               | 44         | 0.013    | 1486.89343(1)              | −0.002                   |
| 26    | $E$               | 39         | 0.013    | 1486.893429(2)             | −0.030                   |
| 27    | $E$               | 42         | 0.046    | 1634.0955399(6)            | −0.018                   |
| 28    | $E$               | 41         | 0.046    | 1634.09554(5)              | −0.027                   |
| 29    | $A_1$             | 42         | 0.08     | 1635.56160(3)              | −0.019                   |
| 30    | $E$               | 43         | 0.1      | 1763.284885(5)             | −0.030                   |
| 31    | $E$               | 47         | 0.1      | 1763.284886(1)             | −0.038                   |
| 32    | $E$               | 69         | 2.1      | 1780.735475(2)             | −0.011                   |
| 33    | $E$               | 62         | 2.1      | 1780.735478(4)             | −0.015                   |
| 34    | $A_1$             | 62         | 2.0      | 1780.794560(2)             | −0.011                   |
| 35    | $A_2$             | 58         | 2.0      | 1780.794605(3)             | −0.020                   |
| 36    | $E$               | 53         | 0.096    | 1782.241121(2)             | −0.005                   |
| 37    | $E$               | 57         | 0.095    | 1782.241121(2)             | −0.018                   |
| 38    | $A_1$             | 36         | 0.053    | 1802.38504(2)              | −0.038                   |
| 39    | $E$               | 38         | 0.011    | 1832.3570026(8)            | −0.003                   |
| 40    | $E$               | 51         | 0.011    | 1832.357004(2)             | −0.012                   |
| 41    | $A_1$             | 53         | 0.056    | 1838.043086(1)             | −0.013                   |
| 42    | $A_2$             | 52         | 0.056    | 1838.043097(1)             | −0.019                   |
| 43    | $E$               | 40         | 0.075    | 1840.88673(6)              | −0.007                   |
| 44    | $E$               | 39         | 0.075    | 1840.886731(1)             | −0.024                   |

Continued on next page.

TABLE S4 – states on Sarka/Poirier CSC PES; continued from previous page

| State | $\Gamma_{C_{3v}}$ | $D_{\max}$ | $S_{vN}$ | $\tilde{E}/\text{cm}^{-1}$ | $\Delta\text{Ref. [30]}$ |
|-------|-------------------|------------|----------|----------------------------|--------------------------|
| 45    | $A_2$             | 66         | 2.0      | 1850.278499(1)             | −0.015                   |
| 46    | $E$               | 56         | 2.0      | 1850.377053(3)             | −0.018                   |
| 47    | $E$               | 56         | 2.0      | 1850.377054(3)             | −0.019                   |
| 48    | $A_1$             | 55         | 2.0      | 1850.485768(3)             | −0.023                   |
| 49    | $E$               | 48         | 0.027    | 1958.6764976(9)            | −0.002                   |
| 50    | $E$               | 45         | 0.027    | 1958.676499(2)             | −0.038                   |
| 51    | $A_1$             | 59         | 0.059    | 1999.913368(1)             | −0.029                   |
| 52    | $A_2$             | 48         | 0.059    | 1999.913371(1)             | −0.030                   |
| 53    | $E$               | 50         | 0.12     | 2002.812132(1)             | −0.012                   |
| 54    | $E$               | 43         | 0.12     | 2002.81213(5)              | −0.035                   |
| 55    | $A_1$             | 54         | 0.026    | 2097.53463(2)              | −0.019                   |
| 56    | $E$               | 61         | 0.019    | 2103.014437(1)             | −0.003                   |
| 57    | $E$               | 54         | 0.019    | 2103.01444(1)              | −0.020                   |
| 58    | $E$               | 47         | 0.11     | 2128.221847(4)             | −0.034                   |
| 59    | $E$               | 47         | 0.11     | 2128.221847(6)             | −0.038                   |
| 60    | $A_1$             | 47         | 0.12     | 2129.693729(1)             | −0.034                   |
| 61    | $E$               | 78         | 2.1      | 2147.180427(1)             | −0.015                   |
| 62    | $E$               | 84         | 2.1      | 2147.180427(2)             | −0.017                   |
| 63    | $E$               | 61         | 2.0      | 2147.267739(3)             | −0.018                   |
| 64    | $E$               | 62         | 2.0      | 2147.267739(5)             | −0.020                   |
| 65    | $A_1$             | 80         | 2.1      | 2149.977926(1)             | −0.018                   |
| 66    | $E$               | 63         | 2.1      | 2150.147635(2)             | −0.006                   |
| 67    | $E$               | 63         | 2.1      | 2150.147636(2)             | −0.021                   |
| 68    | $A_2$             | 63         | 2.0      | 2150.252436(2)             | −0.007                   |
| 69    | $E$               | 38         | 0.077    | 2164.4621942(9)            | −0.038                   |
| 70    | $E$               | 36         | 0.077    | 2164.462194(1)             | −0.039                   |
| 71    | $A_2$             | 48         | 0.012    | 2203.241376(1)             | −0.009                   |
| 72    | $A_1$             | 48         | 0.012    | 2203.2413768(6)            | −0.017                   |
| 73    | $E$               | 58         | 0.07     | 2210.272470(1)             | −0.018                   |
| 74    | $E$               | 42         | 0.07     | 2210.272472(2)             | −0.022                   |
| 75    | $E$               | 55         | 0.099    | 2214.492281(1)             | −0.014                   |
| 76    | $E$               | 52         | 0.099    | 2214.492281(2)             | −0.021                   |
| 77    | $E$               | 59         | 2.0      | 2215.375406(3)             | −0.005                   |
| 78    | $E$               | 57         | 2.0      | 2215.375406(7)             | −0.005                   |
| 79    | $A_1$             | 57         | 2.0      | 2215.379231(6)             | −0.032                   |
| 80    | $A_2$             | 58         | 2.0      | 2215.379390(7)             | −0.036                   |
| 81    | $A_1$             | 54         | 0.11     | 2215.899228(1)             | −0.020                   |
| 82    | $E$               | 55         | 0.12     | 2216.867929(2)             | −0.003                   |
| 83    | $E$               | 55         | 0.1      | 2216.867930(2)             | −0.034                   |
| 84    | $A_1$             | 38         | 0.13     | 2273.24002(1)              | −0.038                   |
| 85    | $A_1$             | 48         | 0.24     | 2307.0828278(8)            | −0.038                   |
| 86    | $A_1$             | 73         | 2.1      | 2321.352812(2)             | −0.016                   |
| 87    | $E$               | 76         | 2.0      | 2321.441019(2)             | −0.024                   |
| 88    | $E$               | 72         | 2.0      | 2321.441019(2)             | −0.031                   |
| 89    | $A_2$             | 61         | 2.0      | 2321.481456(1)             | −0.033                   |
| 90    | $E$               | 51         | 0.072    | 2367.222454(1)             | −0.033                   |
| 91    | $E$               | 62         | 0.072    | 2367.222455(1)             | −0.034                   |
| 92    | $E$               | 49         | 0.17     | 2371.52129(3)              | −0.021                   |
| 93    | $E$               | 65         | 0.17     | 2371.521294(3)             | −0.033                   |
| 94    | $A_1$             | 53         | 0.2      | 2372.954458(2)             | −0.026                   |
| 95    | $E$               | 55         | 0.028    | 2394.1615018(4)            | −0.003                   |
| 96    | $E$               | 53         | 0.028    | 2394.16150(1)              | −0.037                   |
| 97    | $E$               | 55         | 0.19     | 2451.436838(1)             | −0.030                   |
| 98    | $E$               | 70         | 0.19     | 2451.436840(3)             | −0.038                   |
| 99    | $E$               | 76         | 0.13     | 2460.962267(2)             | −0.021                   |
| 100   | $E$               | 70         | 0.13     | 2460.962267(2)             | −0.021                   |
| 101   | $E$               | 82         | 2.1      | 2466.407810(2)             | −0.010                   |
| 102   | $E$               | 86         | 2.1      | 2466.407810(2)             | −0.025                   |
| 103   | $A_1$             | 58         | 2.0      | 2466.45231(2)              | −0.014                   |

Continued on next page.

TABLE S4 – states on Sarka/Poirier CSC PES; continued from previous page

| State | $\Gamma_{C_{3v}}$ | $D_{\max}$ | $S_{vN}$ | $\tilde{E}/\text{cm}^{-1}$ | $\Delta\text{Ref. [30]}$ |
|-------|-------------------|------------|----------|----------------------------|--------------------------|
| 104   | $A_2$             | 56         | 2.0      | 2466.45611(1)              | −0.026                   |
| 105   | $A_1$             | 45         | 0.12     | 2494.660772(9)             | −0.036                   |
| 106   | $A_2$             | 46         | 0.12     | 2494.660775(9)             | −0.038                   |
| 107   | $E$               | 45         | 0.13     | 2497.57144(1)              | −0.033                   |
| 108   | $E$               | 48         | 0.13     | 2497.571439(8)             | −0.038                   |
| 109   | $A_1$             | 85         | 2.1      | 2515.105208(3)             | −0.018                   |
| 110   | $A_2$             | 90         | 2.1      | 2515.105208(2)             | −0.020                   |
| 111   | $E$               | 66         | 2.0      | 2515.222618(4)             | −0.020                   |
| 112   | $E$               | 73         | 2.0      | 2515.222621(6)             | −0.023                   |
| 113   | $E$               | 89         | 2.1      | 2519.425044(3)             | −0.014                   |
| 114   | $E$               | 92         | 2.1      | 2519.425044(3)             | −0.023                   |
| 115   | $A_1$             | 86         | 2.1      | 2519.505947(4)             | −0.014                   |
| 116   | $A_2$             | 91         | 2.1      | 2519.506071(3)             | −0.027                   |
| 117   | $E$               | 62         | 0.21     | 2520.928701(1)             | −0.015                   |
| 118   | $E$               | 65         | 0.2      | 2520.928702(2)             | −0.023                   |
| 119   | $E$               | 58         | 0.1      | 2528.077037(1)             | −0.038                   |
| 120   | $E$               | 58         | 0.1      | 2528.077037(1)             | −0.039                   |
| 121   | $A_1$             | 54         | 0.16     | 2529.538565(1)             | −0.038                   |
| 122   | $A_2$             | 45         | 2.0      | 2538.893031(3)             | −0.017                   |
| 123   | $E$               | 67         | 2.0      | 2539.768550(1)             | −0.016                   |
| 124   | $E$               | 65         | 2.0      | 2539.768550(2)             | −0.020                   |
| 125   | $A_1$             | 59         | 2.0      | 2540.181685(1)             | −0.021                   |
| 126   | $E$               | 44         | 0.014    | 2575.557279(1)             | −0.015                   |
| 127   | $E$               | 56         | 0.013    | 2575.557281(2)             | −0.023                   |
| 128   | $E$               | 54         | 2.0      | 2581.881809(1)             | −0.005                   |
| 129   | $E$               | 75         | 2.0      | 2581.881810(3)             | −0.005                   |
| 130   | $E$               | 63         | 2.0      | 2581.886770(2)             | −0.033                   |
| 131   | $E$               | 69         | 2.0      | 2581.886772(3)             | −0.035                   |
| 132   | $E$               | 53         | 0.084    | 2583.904157(2)             | −0.020                   |
| 133   | $E$               | 63         | 0.084    | 2583.904157(1)             | −0.021                   |
| 134   | $A_2$             | 63         | 2.0      | 2584.593601(6)             | −0.017                   |
| 135   | $E$               | 70         | 2.0      | 2584.803802(1)             | −0.019                   |
| 136   | $E$               | 81         | 2.0      | 2584.803804(2)             | −0.019                   |
| 137   | $A_1$             | 60         | 2.0      | 2585.002900(8)             | −0.022                   |
| 138   | $A_1$             | 51         | 0.12     | 2589.470506(3)             | −0.015                   |
| 139   | $A_2$             | 50         | 0.12     | 2589.470535(3)             | −0.025                   |
| 140   | $E$               | 43         | 0.14     | 2592.2542753(4)            | −0.011                   |
| 141   | $E$               | 57         | 0.14     | 2592.254277(2)             | −0.031                   |
| 142   | $E$               | 40         | 0.13     | 2636.267461(1)             | −0.039                   |
| 143   | $E$               | 40         | 0.13     | 2636.26746(2)              | −0.039                   |
| 144   | $E$               | 49         | 0.26     | 2669.809554(2)             | −0.037                   |
| 145   | $E$               | 51         | 0.26     | 2669.809554(2)             | −0.038                   |
| 146   | $E$               | 86         | 2.1      | 2685.675640(2)             | −0.026                   |
| 147   | $E$               | 68         | 2.1      | 2685.675644(4)             | −0.032                   |
| 148   | $A_1$             | 59         | 2.1      | 2685.73250(1)              | −0.031                   |
| 149   | $A_2$             | 63         | 2.1      | 2685.732572(9)             | −0.033                   |
| 150   | $A_1$             | 45         | 0.13     | 2685.761414(1)             | −0.041                   |
| 151   | $E$               | 57         | 0.16     | 2687.176998(3)             | −0.022                   |
| 152   | $E$               | 61         | 0.16     | 2687.176999(4)             | −0.039                   |
| 153   | $E$               | 53         | 0.087    | 2736.005598(2)             | −0.034                   |
| 154   | $E$               | 55         | 0.087    | 2736.005598(2)             | −0.036                   |
| 155   | $A_1$             | 71         | 0.22     | 2741.672494(1)             | −0.028                   |
| 156   | $A_2$             | 59         | 0.22     | 2741.672506(1)             | −0.032                   |
| 157   | $E$               | 64         | 0.27     | 2744.506603(1)             | −0.015                   |
| 158   | $E$               | 60         | 0.27     | 2744.506603(1)             | −0.037                   |
| 159   | $A_2$             | 75         | 2.0      | 2756.857330(1)             | −0.032                   |
| 160   | $E$               | 62         | 2.0      | 2756.956183(2)             | −0.017                   |
| 161   | $E$               | 65         | 2.0      | 2756.956185(3)             | −0.032                   |
| 162   | $A_1$             | 65         | 2.0      | 2757.065142(2)             | −0.023                   |

Continued on next page.

TABLE S4 – states on Sarka/Poirier CSC PES; continued from previous page

| State | $\Gamma_{C_{3v}}$ | $D_{\max}$ | $S_{vN}$ | $\tilde{E}/\text{cm}^{-1}$ | $\Delta\text{Ref. [30]}$ |
|-------|-------------------|------------|----------|----------------------------|--------------------------|
| 163   | $A_1$             | 52         | 0.077    | 2787.1286656(6)            | −0.038                   |
| 164   | $A_1$             | 80         | 2.3      | 2814.716060(3)             | −0.034                   |
| 165   | $E$               | 83         | 2.2      | 2814.836081(3)             | −0.034                   |
| 166   | $E$               | 79         | 2.2      | 2814.836084(3)             | −0.038                   |
| 167   | $A_2$             | 71         | 2.1      | 2814.886075(3)             | −0.038                   |
| 168   | $E$               | 92         | 0.19     | 2825.900123(2)             | −0.021                   |
| 169   | $E$               | 92         | 0.19     | 2825.900123(2)             | −0.021                   |
| 170   | $A_1$             | 88         | 0.22     | 2827.355838(3)             | −0.021                   |
| 171   | $A_2$             | 101        | 2.2      | 2831.309935(2)             | −0.021                   |
| 172   | $A_1$             | 93         | 2.2      | 2831.318193(2)             | −0.026                   |
| 173   | $E$               | 82         | 2.0      | 2831.411741(4)             | −0.020                   |
| 174   | $E$               | 87         | 2.0      | 2831.411743(6)             | −0.026                   |
| 175   | $E$               | 74         | 0.11     | 2832.828044(3)             | −0.021                   |
| 176   | $E$               | 72         | 0.11     | 2832.828045(5)             | −0.021                   |
| 177   | $E$               | 52         | 0.06     | 2853.329025(1)             | −0.039                   |
| 178   | $E$               | 55         | 0.06     | 2853.3290252(9)            | −0.039                   |
| 179   | $E$               | 49         | 0.12     | 2862.583421(6)             | −0.038                   |
| 180   | $E$               | 59         | 0.12     | 2862.583424(6)             | −0.039                   |
| 181   | $E$               | 72         | 0.15     | 2866.900969(1)             | −0.036                   |
| 182   | $E$               | 54         | 0.15     | 2866.900971(3)             | −0.038                   |
| 183   | $A_1$             | 50         | 0.15     | 2868.340340(3)             | −0.037                   |
| 184   | $E$               | 86         | 2.1      | 2884.493508(4)             | −0.019                   |
| 185   | $E$               | 74         | 2.1      | 2884.493512(4)             | −0.023                   |
| 186   | $A_2$             | 67         | 2.0      | 2884.641806(3)             | −0.023                   |
| 187   | $A_1$             | 71         | 2.0      | 2884.641808(3)             | −0.025                   |
| 188   | $E$               | 56         | 0.096    | 2886.895602(1)             | −0.030                   |
| 189   | $E$               | 64         | 0.096    | 2886.895605(4)             | −0.038                   |
| 190   | $E$               | 104        | 2.1      | 2890.193710(2)             | −0.021                   |
| 191   | $E$               | 108        | 2.1      | 2890.193710(1)             | −0.026                   |
| 192   | $E$               | 74         | 2.1      | 2890.298681(3)             | −0.022                   |
| 193   | $E$               | 95         | 2.1      | 2890.298685(6)             | −0.028                   |
| 194   | $A_1$             | 93         | 2.2      | 2892.865807(3)             | −0.022                   |
| 195   | $E$               | 96         | 2.1      | 2893.120273(2)             | −0.021                   |
| 196   | $E$               | 75         | 2.1      | 2893.120277(4)             | −0.024                   |
| 197   | $A_2$             | 40         | 0.13     | 2893.211480(4)             | −0.040                   |
| 198   | $A_1$             | 52         | 0.13     | 2893.211480(3)             | −0.040                   |
| 199   | $A_2$             | 66         | 2.1      | 2893.289192(4)             | −0.021                   |
| 200   | $E$               | 58         | 0.24     | 2896.099571(1)             | −0.038                   |
| 201   | $E$               | 68         | 0.24     | 2896.099571(1)             | −0.040                   |
| 202   | $E$               | 87         | 2.1      | 2902.336019(3)             | −0.020                   |
| 203   | $E$               | 90         | 2.1      | 2902.336019(2)             | −0.033                   |
| 204   | $E$               | 68         | 3.0      | 2903.23018(1)              | −0.016                   |
| 205   | $E$               | 69         | 3.0      | 2903.23018(1)              | −0.025                   |
| 206   | $A_1$             | 70         | 3.0      | 2903.23614(1)              | −0.022                   |
| 207   | $A_2$             | 64         | 3.0      | 2903.23705(1)              | −0.031                   |
| 208   | $E$               | 68         | 2.1      | 2903.64165(1)              | −0.019                   |
| 209   | $E$               | 67         | 2.1      | 2903.64165(1)              | −0.028                   |
| 210   | $E$               | 56         | 0.016    | 2949.288795(1)             | −0.021                   |
| 211   | $E$               | 61         | 0.015    | 2949.288795(2)             | −0.026                   |
| 212   | $E$               | 72         | 2.0      | 2949.866421(2)             | −0.008                   |
| 213   | $E$               | 69         | 2.0      | 2949.866421(3)             | −0.013                   |
| 214   | $A_2^*$           | 73         | 2.0      | 2949.878350(1)             | −0.034                   |
| 215   | $A_1^*$           | 83         | 2.0      | 2949.878352(2)             | −0.034                   |
| 216   | $E$               | 96         | 2.1      | 2954.152011(2)             | −0.014                   |
| 217   | $E$               | 95         | 2.1      | 2954.152011(2)             | −0.028                   |
| 218   | $A_1$             | 101        | 2.1      | 2954.192884(2)             | −0.028                   |
| 219   | $A_2$             | 92         | 2.1      | 2954.193049(2)             | −0.030                   |
| 220   | $E$               | 60         | 0.27     | 2955.668208(6)             | −0.012                   |
| 221   | $E$               | 65         | 0.28     | 2955.668209(4)             | −0.041                   |

Continued on next page.

TABLE S4 – states on Sarka/Poirier CSC PES; continued from previous page

| State | $\Gamma_{C_{3v}}$ | $D_{\max}$ | $S_{vN}$ | $\tilde{E}/\text{cm}^{-1}$ | $\Delta\text{Ref. [30]}$ |
|-------|-------------------|------------|----------|----------------------------|--------------------------|
| 222   | $A_1^*$           | 65         | 0.1      | 2958.922400(1)             | −0.022                   |
| 223   | $A_2^*$           | 65         | 0.1      | 2958.922400(1)             | −0.023                   |
| 224   | $E$               | 65         | 0.15     | 2965.806316(1)             | −0.023                   |
| 225   | $E$               | 60         | 0.15     | 2965.806316(2)             | −0.026                   |
| 226   | $A_1$             | 62         | 0.42     | 2969.337225(1)             | −0.030                   |
| 227   | $E$               | 60         | 0.17     | 2969.937777(1)             | −0.022                   |
| 228   | $E$               | 55         | 0.17     | 2969.937778(1)             | −0.023                   |
| 229   | $A_1$             | 62         | 0.18     | 2971.315117(1)             | −0.025                   |
| 230   | $E$               | 61         | 0.023    | 2976.3482601(7)            | −0.029                   |
| 231   | $E$               | 64         | 0.023    | 2976.348261(1)             | −0.031                   |
| 232   | $E$               | 48         | 0.14     | 3000.817046(1)             | −0.038                   |
| 233   | $E$               | 45         | 0.14     | 3000.817046(1)             | −0.041                   |
| 234   | $A_1$             | 41         | 0.15     | 3002.288339(1)             | −0.041                   |
| 235   | $A_1$             | 66         | 0.85     | 3002.7302004(8)            | −0.063                   |
| 236   | $A_1$             | 56         | 0.52     | 3003.16478(1)              | −0.025                   |
| 237   | $E$               | 59         | 0.037    | 3008.624095(2)             | −0.024                   |
| 238   | $E$               | 58         | 0.037    | 3008.624095(2)             | −0.038                   |
| 239   | $E$               | 51         | 0.28     | 3034.06587(1)              | −0.038                   |
| 240   | $E$               | 51         | 0.28     | 3034.06587(1)              | −0.041                   |
| 241   | $A_1$             | 69         | 0.31     | 3035.535233(1)             | −0.042                   |
| 242   | $E$               | 55         | 0.14     | 3047.120490(1)             | −0.042                   |
| 243   | $E$               | 58         | 0.14     | 3047.1204905(9)            | −0.053                   |
| 244   | $E$               | 91         | 2.1      | 3051.447928(4)             | −0.034                   |
| 245   | $E$               | 93         | 2.1      | 3051.447928(4)             | −0.034                   |
| 246   | $E$               | 74         | 2.1      | 3051.532664(3)             | −0.034                   |
| 247   | $E$               | 98         | 2.1      | 3051.532669(6)             | −0.035                   |
| 248   | $A_1$             | 88         | 2.2      | 3054.237092(5)             | −0.027                   |
| 249   | $E$               | 92         | 2.2      | 3054.406040(3)             | −0.030                   |
| 250   | $E$               | 90         | 2.2      | 3054.406040(3)             | −0.037                   |
| 251   | $A_2$             | 69         | 2.1      | 3054.511707(3)             | −0.036                   |
| 252   | $A_1$             | 67         | 0.1      | 3106.246177(1)             | −0.037                   |
| 253   | $A_2$             | 59         | 0.1      | 3106.246177(2)             | −0.038                   |
| 254   | $E$               | 65         | 0.27     | 3113.249641(1)             | −0.033                   |
| 255   | $E$               | 65         | 0.27     | 3113.249641(1)             | −0.033                   |
| 256   | $E$               | 66         | 0.35     | 3117.453005(1)             | −0.025                   |
| 257   | $E$               | 66         | 0.35     | 3117.453006(1)             | −0.035                   |
| 258   | $A_1$             | 70         | 0.37     | 3118.854331(1)             | −0.031                   |
| 259   | $E$               | 65         | 2.1      | 3121.274078(7)             | −0.025                   |
| 260   | $E$               | 69         | 2.1      | 3121.274078(5)             | −0.028                   |
| 261   | $A_1$             | 62         | 2.1      | 3121.27821(1)              | −0.036                   |
| 262   | $A_2$             | 60         | 2.1      | 3121.27823(1)              | −0.042                   |
| 263   | $E$               | 67         | 0.18     | 3122.763999(1)             | −0.019                   |
| 264   | $E$               | 71         | 0.17     | 3122.764000(1)             | −0.046                   |
| 265   | $E$               | 70         | 0.041    | 3140.886906(1)             | −0.012                   |
| 266   | $E$               | 66         | 0.041    | 3140.886908(2)             | −0.035                   |
| 267   | $E$               | 54         | 0.091    | 3150.492020(1)             | −0.038                   |
| 268   | $E$               | 52         | 0.091    | 3150.492021(2)             | −0.044                   |
| 269   | $A_1$             | 79         | 0.034    | 3151.857572(1)             | −0.013                   |
| 270   | $A_2$             | 72         | 0.027    | 3152.024697(1)             | −0.028                   |
| 271   | $A_1$             | 52         | 0.38     | 3178.045234(1)             | −0.045                   |
| 272   | $E$               | 99         | 2.3      | 3179.676387(4)             | −0.037                   |
| 273   | $E$               | 105        | 2.3      | 3179.676387(4)             | −0.040                   |
| 274   | $A_1$             | 69         | 2.2      | 3179.75704(4)              | −0.037                   |
| 275   | $A_2$             | 64         | 2.2      | 3179.75710(6)              | −0.040                   |
| 276   | $E$               | 85         | 0.28     | 3181.203845(2)             | −0.034                   |
| 277   | $E$               | 84         | 0.28     | 3181.203846(1)             | −0.041                   |
| 278   | $E$               | 53         | 0.02     | 3185.048206(1)             | −0.012                   |
| 279   | $E$               | 56         | 0.02     | 3185.048206(1)             | −0.103                   |
| 280   | $A_1$             | 72         | 0.22     | 3192.33294(1)              | −0.021                   |

Continued on next page.

TABLE S4 – states on Sarka/Poirier CSC PES; continued from previous page

| State | $\Gamma_{C_{3v}}$ | $D_{\max}$ | $S_{vN}$ | $\tilde{E}/\text{cm}^{-1}$ | $\Delta\text{Ref. [30]}$ |
|-------|-------------------|------------|----------|----------------------------|--------------------------|
| 281   | $A_2$             | 69         | 0.22     | 3192.33295(1)              | −0.022                   |
| 282   | $E$               | 96         | 0.3      | 3195.213522(2)             | −0.020                   |
| 283   | $E$               | 107        | 0.3      | 3195.213523(3)             | −0.024                   |
| 284   | $E$               | 106        | 2.2      | 3197.719112(5)             | −0.025                   |
| 285   | $E$               | 117        | 2.2      | 3197.719113(5)             | −0.027                   |
| 286   | $E$               | 96         | 2.0      | 3197.868503(4)             | −0.025                   |
| 287   | $E$               | 106        | 2.0      | 3197.868505(5)             | −0.027                   |
| 288   | $E$               | 100        | 2.1      | 3200.666962(5)             | −0.016                   |
| 289   | $E$               | 90         | 2.1      | 3200.666965(6)             | −0.028                   |
| 290   | $A_1$             | 88         | 2.1      | 3200.713632(6)             | −0.018                   |
| 291   | $A_2$             | 94         | 2.1      | 3200.721045(4)             | −0.029                   |
| 292   | $A_1$             | 50         | 0.52     | 3202.718115(1)             | −0.046                   |
| 293   | $A_1$             | 79         | 2.2      | 3215.302213(3)             | −0.043                   |
| 294   | $E$               | 79         | 2.1      | 3215.387669(2)             | −0.038                   |
| 295   | $E$               | 83         | 2.1      | 3215.387670(2)             | −0.043                   |
| 296   | $A_2$             | 65         | 2.1      | 3215.429010(1)             | −0.039                   |
| 297   | $E$               | 51         | 0.13     | 3231.972157(7)             | −0.039                   |
| 298   | $E$               | 76         | 0.13     | 3231.972160(7)             | −0.039                   |
| 299   | $A_1$             | 79         | 0.16     | 3237.665621(1)             | −0.037                   |
| 300   | $A_2$             | 74         | 0.16     | 3237.665633(1)             | −0.040                   |
| 301   | $E$               | 70         | 0.17     | 3240.512920(1)             | −0.035                   |
| 302   | $E$               | 71         | 0.17     | 3240.512920(1)             | −0.043                   |
| 303   | $A_2$             | 80         | 2.1      | 3250.225912(7)             | −0.038                   |
| 304   | $E$               | 92         | 2.1      | 3250.325234(1)             | −0.038                   |
| 305   | $E$               | 80         | 2.1      | 3250.325240(6)             | −0.040                   |
| 306   | $A_1$             | 82         | 2.1      | 3250.434435(3)             | −0.042                   |
| 307   | $E$               | 89         | 2.1      | 3255.328874(4)             | −0.022                   |
| 308   | $E$               | 97         | 2.1      | 3255.328874(3)             | −0.027                   |
| 309   | $E$               | 79         | 2.0      | 3255.508396(3)             | −0.025                   |
| 310   | $E$               | 73         | 2.0      | 3255.508398(4)             | −0.029                   |
| 311   | $E$               | 66         | 0.15     | 3259.848098(1)             | −0.040                   |
| 312   | $E$               | 68         | 0.15     | 3259.848098(1)             | −0.041                   |
| 313   | $A_1$             | 72         | 2.2      | 3262.37549(2)              | −0.027                   |
| 314   | $A_2$             | 73         | 2.2      | 3262.37550(2)              | −0.028                   |
| 315   | $E$               | 95         | 2.1      | 3262.509127(5)             | −0.028                   |
| 316   | $E$               | 77         | 2.1      | 3262.509131(7)             | −0.029                   |
| 317   | $E$               | 66         | 0.32     | 3264.128363(1)             | −0.041                   |
| 318   | $E$               | 78         | 0.32     | 3264.128363(1)             | −0.044                   |
| 319   | $A_1$             | 77         | 0.37     | 3265.555363(1)             | −0.043                   |
| 320   | $E$               | 88         | 2.2      | 3266.591724(9)             | −0.023                   |
| 321   | $E$               | 111        | 2.2      | 3266.591724(8)             | −0.024                   |
| 322   | $A_1$             | 75         | 2.1      | 3266.703611(4)             | −0.020                   |
| 323   | $A_2$             | 73         | 2.1      | 3266.703817(7)             | −0.030                   |
| 324   | $E$               | 108        | 2.1      | 3267.315263(2)             | −0.029                   |
| 325   | $E$               | 108        | 2.1      | 3267.315263(2)             | −0.035                   |
| 326   | $A_2$             | 128        | 3.5      | 3268.097387(2)             | −0.030                   |
| 327   | $E$               | 94         | 0.41     | 3268.109043(7)             | −0.024                   |
| 328   | $E$               | 85         | 0.41     | 3268.109043(6)             | −0.027                   |
| 329   | $A_1$             | 118        | 3.1      | 3268.178392(3)             | −0.029                   |
| 330   | $E$               | 120        | 3.1      | 3268.223021(2)             | −0.026                   |
| 331   | $E$               | 123        | 3.1      | 3268.223021(3)             | −0.030                   |
| 332   | $E$               | 106        | 2.1      | 3268.613959(3)             | −0.025                   |
| 333   | $E$               | 111        | 2.1      | 3268.613959(3)             | −0.026                   |
| 334   | $A_2$             | 120        | 2.6      | 3268.877563(3)             | −0.024                   |
| 335   | $E$               | 92         | 2.1      | 3269.681986(2)             | −0.024                   |
| 336   | $E$               | 96         | 2.1      | 3269.681987(4)             | −0.026                   |
| 337   | $A_1$             | 80         | 2.1      | 3270.08323(1)              | −0.026                   |
| 338   | $E$               | 62         | 0.059    | 3289.807175(1)             | −0.038                   |
| 339   | $E$               | 60         | 0.059    | 3289.8071750(9)            | −0.052                   |

Continued on next page.

TABLE S4 – states on Sarka/Poirier CSC PES; continued from previous page

| State | $\Gamma_{C_{3v}}$ | $D_{\max}$ | $S_{vN}$ | $\tilde{E}/\text{cm}^{-1}$ | $\Delta\text{Ref. [30]}$ |
|-------|-------------------|------------|----------|----------------------------|--------------------------|
| 340   | $A_2^*$           | 69         | 2.0      | 3319.315771(4)             | −0.013                   |
| 341   | $A_1^*$           | 70         | 2.0      | 3319.315772(3)             | −0.019                   |
| 342   | $E$               | 75         | 2.0      | 3319.334251(2)             | −0.033                   |
| 343   | $E$               | 70         | 2.0      | 3319.334252(4)             | −0.035                   |
| 344   | $A_1$             | 52         | 0.017    | 3324.420466(1)             | −0.027                   |
| 345   | $A_2$             | 52         | 0.017    | 3324.420466(2)             | −0.032                   |
| 346   | $E$               | 54         | 0.14     | 3324.9669088(8)            | −0.037                   |
| 347   | $E$               | 51         | 0.14     | 3324.9669094(9)            | −0.045                   |
| 348   | $E$               | 99         | 2.1      | 3324.995814(2)             | −0.023                   |
| 349   | $E$               | 89         | 2.1      | 3324.995814(2)             | −0.026                   |
| 350   | $E$               | 73         | 2.1      | 3325.016935(2)             | −0.035                   |
| 351   | $E$               | 104        | 2.1      | 3325.016936(2)             | −0.036                   |
| 352   | $A_2$             | 90         | 2.1      | 3327.559585(3)             | −0.030                   |
| 353   | $E$               | 74         | 2.1      | 3327.885896(2)             | −0.025                   |
| 354   | $E$               | 76         | 2.1      | 3327.885896(2)             | −0.030                   |
| 355   | $A_1$             | 83         | 2.1      | 3328.166027(1)             | −0.028                   |
| 356   | $E$               | 83         | 0.42     | 3332.836415(1)             | −0.031                   |
| 357   | $E$               | 78         | 0.42     | 3332.836416(1)             | −0.033                   |
| 358   | $E$               | 60         | 0.12     | 3335.312343(2)             | −0.022                   |
| 359   | $E$               | 54         | 0.12     | 3335.312343(3)             | −0.026                   |
| 360   | $A_2$             | 63         | 2.0      | 3339.844894(8)             | −0.031                   |
| 361   | $A_1$             | 63         | 2.0      | 3339.845370(9)             | −0.032                   |
| 362   | $E$               | 65         | 2.0      | 3339.85774(1)              | −0.033                   |
| 363   | $E$               | 63         | 2.0      | 3339.85774(1)              | −0.034                   |
| 364   | $E$               | 69         | 0.17     | 3343.485096(1)             | −0.026                   |
| 365   | $E$               | 68         | 0.17     | 3343.485096(2)             | −0.028                   |
| 366   | $A_1$             | 53         | 0.21     | 3348.935402(3)             | −0.027                   |
| 367   | $A_2$             | 49         | 0.21     | 3348.935467(1)             | −0.029                   |
| 368   | $E$               | 48         | 0.23     | 3351.661152(1)             | −0.014                   |
| 369   | $E$               | 62         | 0.23     | 3351.661154(3)             | −0.047                   |
| 370   | $E$               | 76         | 0.37     | 3357.953442(1)             | −0.037                   |
| 371   | $E$               | 78         | 0.36     | 3357.953442(1)             | −0.055                   |
| 372   | $E$               | 100        | 0.85     | 3365.881247(2)             | −0.026                   |
| 373   | $E$               | 93         | 0.86     | 3365.881247(5)             | −0.045                   |
| 374   | $E$               | 74         | 1.0      | 3366.226742(1)             | −0.065                   |
| 375   | $E$               | 68         | 1.0      | 3366.226745(4)             | −0.071                   |
| 376   | $A_1$             | 41         | 0.14     | 3366.870109(1)             | −0.042                   |
| 377   | $A_2$             | 41         | 0.14     | 3366.870111(2)             | −0.045                   |
| 378   | $E$               | 57         | 0.16     | 3369.780327(1)             | −0.041                   |
| 379   | $E$               | 53         | 0.16     | 3369.780327(1)             | −0.049                   |
| 380   | $E$               | 99         | 2.1      | 3371.328571(2)             | −0.030                   |
| 381   | $E$               | 68         | 2.1      | 3371.32858(1)              | −0.039                   |
| 382   | $A_1$             | 71         | 2.1      | 3371.36966(1)              | −0.036                   |
| 383   | $A_2$             | 79         | 2.1      | 3371.373474(5)             | −0.037                   |
| 384   | $A_1$             | 54         | 0.3      | 3399.833038(4)             | −0.041                   |
| 385   | $A_2$             | 49         | 0.3      | 3399.83304(1)              | −0.043                   |
| 386   | $E$               | 65         | 0.35     | 3402.737219(3)             | −0.041                   |
| 387   | $E$               | 64         | 0.35     | 3402.737219(3)             | −0.048                   |
| 388   | $E$               | 65         | 0.18     | 3410.029723(1)             | −0.050                   |
| 389   | $E$               | 65         | 0.18     | 3410.029723(1)             | −0.053                   |
| 390   | $A_1$             | 65         | 0.26     | 3411.484368(1)             | −0.051                   |
| 391   | $A_2^*$           | 73         | 2.2      | 3418.70893(1)              | −0.037                   |
| 392   | $A_1^*$           | 72         | 2.2      | 3418.70893(1)              | −0.038                   |
| 393   | $E$               | 78         | 2.1      | 3418.823594(4)             | −0.037                   |
| 394   | $E$               | 103        | 2.1      | 3418.823598(6)             | −0.039                   |
| 395   | $E$               | 122        | 2.2      | 3423.014909(2)             | −0.028                   |
| 396   | $E$               | 119        | 2.2      | 3423.014909(2)             | −0.040                   |
| 397   | $A_1$             | 98         | 2.2      | 3423.094717(7)             | −0.034                   |
| 398   | $A_2$             | 79         | 2.2      | 3423.094843(6)             | −0.040                   |

Continued on next page.



TABLE S4 – states on Sarka/Poirier CSC PES; continued from previous page

| State | $\Gamma_{C_{3v}}$ | $D_{\max}$ | $S_{vN}$ | $\tilde{E}/\text{cm}^{-1}$ | $\Delta\text{Ref. [30]}$ |
|-------|-------------------|------------|----------|----------------------------|--------------------------|
| 399   | $E$               | 72         | 0.36     | 3424.513958(7)             | −0.029                   |
| 400   | $E$               | 77         | 0.35     | 3424.513959(6)             | −0.044                   |
| 401   | $A_2$             | 52         | 2.0      | 3445.464311(7)             | −0.038                   |
| 402   | $E$               | 62         | 2.0      | 3446.341773(2)             | −0.030                   |
| 403   | $E$               | 79         | 2.0      | 3446.341777(5)             | −0.037                   |
| 404   | $A_1$             | 73         | 2.0      | 3446.758870(2)             | −0.034                   |
| 405   | $E$               | 65         | 0.12     | 3477.928123(1)             | −0.038                   |
| 406   | $E$               | 55         | 0.12     | 3477.928123(3)             | −0.040                   |
| 407   | $E$               | 72         | 0.33     | 3486.236852(2)             | −0.037                   |
| 408   | $E$               | 70         | 0.32     | 3486.236852(1)             | −0.039                   |
| 409   | $E$               | 79         | 2.1      | 3487.109165(3)             | −0.032                   |
| 410   | $E$               | 89         | 2.1      | 3487.109166(3)             | −0.034                   |
| 411   | $E$               | 91         | 2.1      | 3487.114259(2)             | −0.041                   |
| 412   | $E$               | 84         | 2.1      | 3487.114259(4)             | −0.046                   |
| 413   | $A_2$             | 78         | 2.1      | 3489.813429(8)             | −0.039                   |
| 414   | $E$               | 94         | 2.1      | 3490.024316(3)             | −0.030                   |
| 415   | $E$               | 89         | 2.1      | 3490.024317(2)             | −0.039                   |
| 416   | $A_1$             | 84         | 2.1      | 3490.223747(6)             | −0.035                   |
| 417   | $A_1$             | 70         | 0.43     | 3491.778593(1)             | −0.031                   |
| 418   | $A_2$             | 80         | 0.43     | 3491.778604(1)             | −0.042                   |
| 419   | $E$               | 63         | 0.48     | 3494.549856(3)             | −0.022                   |
| 420   | $E$               | 73         | 0.48     | 3494.549856(2)             | −0.053                   |
| 421   | $A_1$             | 77         | 0.44     | 3495.758464(5)             | −0.048                   |
| 422   | $E$               | 98         | 0.73     | 3501.224707(1)             | −0.036                   |
| 423   | $E$               | 98         | 0.73     | 3501.224708(1)             | −0.046                   |
| 424   | $A_1$             | 106        | 2.4      | 3504.198162(3)             | −0.033                   |
| 425   | $E$               | 91         | 2.5      | 3504.362270(5)             | −0.021                   |
| 426   | $E$               | 101        | 2.6      | 3504.362274(9)             | −0.040                   |
| 427   | $A_2$             | 98         | 2.0      | 3504.399106(3)             | −0.028                   |
| 428   | $E$               | 97         | 0.55     | 3515.242935(3)             | −0.015                   |
| 429   | $E$               | 107        | 0.59     | 3515.242936(3)             | −0.041                   |
| 430   | $E$               | 57         | 0.1      | 3515.376500(5)             | −0.044                   |
| 431   | $E$               | 56         | 0.1      | 3515.376501(3)             | −0.044                   |
| 432   | $E$               | 77         | 0.52     | 3515.42191(1)              | −0.030                   |
| 433   | $E$               | 78         | 0.54     | 3515.42191(1)              | −0.030                   |
| 434   | $A_1$             | 53         | 0.11     | 3516.848194(7)             | −0.045                   |
| 435   | $E$               | 50         | 0.4      | 3540.377368(1)             | −0.046                   |
| 436   | $E$               | 61         | 0.4      | 3540.377368(1)             | −0.054                   |
| 437   | $E$               | 123        | 2.3      | 3546.065112(1)             | −0.040                   |
| 438   | $E$               | 104        | 2.3      | 3546.065112(5)             | −0.041                   |
| 439   | $E$               | 106        | 2.2      | 3546.180251(5)             | −0.040                   |
| 440   | $E$               | 88         | 2.2      | 3546.18025(1)              | −0.041                   |
| 441   | $E$               | 70         | 2.0      | 3548.524217(1)             | −0.013                   |
| 442   | $E$               | 63         | 2.0      | 3548.524217(2)             | −0.017                   |
| 443   | $A_1$             | 73         | 2.0      | 3548.528228(1)             | −0.109                   |
| 444   | $A_2$             | 59         | 2.0      | 3548.533946(2)             | −0.113                   |
| 445   | $A_1$             | 97         | 2.3      | 3548.858001(8)             | −0.042                   |
| 446   | $E$               | 87         | 2.2      | 3549.063531(6)             | −0.039                   |
| 447   | $E$               | 96         | 2.2      | 3549.063533(7)             | −0.042                   |
| 448   | $A_2$             | 89         | 2.2      | 3549.183192(4)             | −0.039                   |
| 449   | $A_1$             | 50         | 0.16     | 3556.726828(1)             | −0.091                   |
| 450   | $E$               | 116        | 0.24     | 3560.244512(2)             | −0.023                   |
| 451   | $E$               | 117        | 0.24     | 3560.244512(2)             | −0.024                   |
| 452   | $E$               | 113        | 0.72     | 3564.503488(4)             | −0.025                   |
| 453   | $E$               | 128        | 0.7      | 3564.503488(4)             | −0.034                   |
| 454   | $E$               | 53         | 0.56     | 3564.74198(1)              | −0.046                   |
| 455   | $E$               | 53         | 0.56     | 3564.741981(4)             | −0.054                   |
| 456   | $E$               | 115        | 2.5      | 3565.620141(5)             | −0.029                   |
| 457   | $E$               | 118        | 2.5      | 3565.620141(4)             | −0.030                   |

Continued on next page.

TABLE S4 – states on Sarka/Poirier CSC PES; continued from previous page

| State | $\Gamma_{C_{3v}}$ | $D_{\max}$ | $S_{vN}$ | $\tilde{E}/\text{cm}^{-1}$ | $\Delta\text{Ref. [30]}$ |
|-------|-------------------|------------|----------|----------------------------|--------------------------|
| 458   | $A_1^*$           | 83         | 2.1      | 3565.80652(1)              | −0.029                   |
| 459   | $A_2^*$           | 77         | 2.1      | 3565.80652(2)              | −0.030                   |
| 460   | $A_1$             | 103        | 0.36     | 3565.950822(2)             | −0.031                   |
| 461   | $A_2$             | 131        | 2.2      | 3569.942698(2)             | −0.022                   |
| 462   | $A_1$             | 114        | 2.3      | 3569.970634(7)             | −0.034                   |
| 463   | $E$               | 97         | 2.1      | 3570.057708(5)             | −0.022                   |
| 464   | $E$               | 99         | 2.1      | 3570.057709(6)             | −0.034                   |
| 465   | $E$               | 88         | 0.19     | 3571.440699(8)             | −0.026                   |
| 466   | $E$               | 97         | 0.19     | 3571.440700(6)             | −0.031                   |
| 467   | $E$               | 108        | 2.2      | 3578.929573(1)             | −0.042                   |
| 468   | $E$               | 96         | 2.2      | 3578.929573(3)             | −0.043                   |
| 469   | $A_1$             | 95         | 2.1      | 3578.983616(4)             | −0.044                   |
| 470   | $A_2$             | 74         | 2.1      | 3578.983672(3)             | −0.044                   |
| 471   | $E$               | 75         | 0.25     | 3580.424497(6)             | −0.039                   |
| 472   | $E$               | 66         | 0.25     | 3580.424501(5)             | −0.049                   |
| 473   | $E$               | 81         | 0.25     | 3585.067562(2)             | −0.024                   |
| 474   | $E$               | 87         | 0.25     | 3585.067562(2)             | −0.045                   |
| 475   | $E$               | 84         | 2.0      | 3590.615449(2)             | −0.025                   |
| 476   | $E$               | 82         | 2.0      | 3590.615450(2)             | −0.031                   |
| 477   | $A_1$             | 57         | 2.0      | 3590.92522(1)              | −0.030                   |
| 478   | $A_2$             | 60         | 2.0      | 3590.930851(9)             | −0.029                   |
| 479   | $A_2$             | 57         | 0.13     | 3602.809907(5)             | −0.039                   |
| 480   | $A_1$             | 80         | 0.13     | 3602.809909(8)             | −0.041                   |
| 481   | $E$               | 77         | 0.18     | 3609.849104(1)             | −0.040                   |
| 482   | $E$               | 70         | 0.18     | 3609.849104(3)             | −0.043                   |
| 483   | $E$               | 72         | 0.2      | 3614.073730(2)             | −0.042                   |
| 484   | $E$               | 68         | 0.2      | 3614.073730(3)             | −0.042                   |
| 485   | $E$               | 99         | 2.1      | 3615.271163(4)             | −0.038                   |
| 486   | $E$               | 93         | 2.1      | 3615.271164(5)             | −0.041                   |
| 487   | $A_1$             | 112        | 2.1      | 3615.275293(3)             | −0.046                   |
| 488   | $A_2$             | 97         | 2.1      | 3615.275621(3)             | −0.048                   |
| 489   | $A_1$             | 79         | 0.23     | 3615.482438(1)             | −0.042                   |
| 490   | $E$               | 82         | 0.21     | 3616.767006(1)             | −0.035                   |
| 491   | $E$               | 85         | 0.21     | 3616.767007(2)             | −0.049                   |
| 492   | $A_1$             | 75         | 2.1      | 3627.595183(4)             | −0.028                   |
| 493   | $A_2$             | 73         | 2.1      | 3627.595185(7)             | −0.031                   |
| 494   | $E$               | 104        | 2.0      | 3627.805981(2)             | −0.029                   |
| 495   | $E$               | 92         | 2.0      | 3627.805981(4)             | −0.032                   |
| 496   | $E$               | 73         | 0.18     | 3627.970164(1)             | −0.043                   |
| 497   | $E$               | 67         | 0.18     | 3627.970164(2)             | −0.043                   |
| 498   | $A_1$             | 61         | 0.4      | 3633.608621(2)             | −0.044                   |
| 499   | $A_2$             | 61         | 0.41     | 3633.608636(3)             | −0.048                   |
| 500   | $A_1$             | 124        | 2.1      | 3633.789746(4)             | −0.034                   |
| 501   | $A_2$             | 115        | 2.1      | 3633.789752(4)             | −0.036                   |
| 502   | $E$               | 141        | 3.2      | 3634.619705(4)             | −0.030                   |
| 503   | $E$               | 144        | 3.2      | 3634.619705(3)             | −0.031                   |
| 504   | $E$               | 131        | 3.0      | 3634.708538(3)             | −0.029                   |
| 505   | $E$               | 128        | 3.0      | 3634.708538(3)             | −0.031                   |
| 506   | $A_2$             | 102        | 2.1      | 3635.089516(3)             | −0.028                   |
| 507   | $A_1$             | 107        | 2.1      | 3635.089516(3)             | −0.028                   |
| 508   | $E$               | 106        | 2.2      | 3635.957955(6)             | −0.030                   |
| 509   | $E$               | 107        | 2.2      | 3635.957955(7)             | −0.031                   |
| 510   | $A_1$             | 101        | 2.1      | 3636.121562(7)             | −0.030                   |
| 511   | $A_2$             | 101        | 2.1      | 3636.121562(8)             | −0.032                   |
| 512   | $E$               | 76         | 0.49     | 3636.428596(1)             | −0.040                   |
| 513   | $E$               | 91         | 0.49     | 3636.428596(2)             | −0.058                   |
| 514   | $E$               | 133        | 2.2      | 3636.662870(3)             | −0.027                   |
| 515   | $E$               | 122        | 2.2      | 3636.662871(3)             | −0.036                   |
| 516   | $A_1$             | 91         | 3.1      | 3637.60018(1)              | −0.026                   |

Continued on next page.

TABLE S4 – states on Sarka/Poirier CSC PES; continued from previous page

| State | $\Gamma_{C_{3v}}$ | $D_{\max}$ | $S_{vN}$ | $\tilde{E}/\text{cm}^{-1}$ | $\Delta\text{Ref. [30]}$ |
|-------|-------------------|------------|----------|----------------------------|--------------------------|
| 517   | $A_2$             | 105        | 3.1      | 3637.60234(1)              | −0.029                   |
| 518   | $E$               | 118        | 2.9      | 3637.623755(2)             | −0.018                   |
| 519   | $E$               | 122        | 2.9      | 3637.623756(3)             | −0.034                   |
| 520   | $E$               | 102        | 2.1      | 3637.998614(4)             | −0.021                   |
| 521   | $E$               | 92         | 2.1      | 3637.998618(8)             | −0.038                   |
| 522   | $E$               | 131        | 2.2      | 3641.533461(1)             | −0.024                   |
| 523   | $E$               | 114        | 2.2      | 3641.533461(4)             | −0.036                   |
| 524   | $E$               | 86         | 2.2      | 3641.660653(8)             | −0.024                   |
| 525   | $E$               | 93         | 2.2      | 3641.66066(1)              | −0.037                   |
| 526   | $A_1$             | 95         | 2.2      | 3644.085218(6)             | −0.033                   |
| 527   | $E$               | 83         | 2.2      | 3644.428455(9)             | −0.027                   |
| 528   | $E$               | 78         | 2.2      | 3644.42846(1)              | −0.035                   |
| 529   | $A_2$             | 92         | 2.2      | 3644.658203(5)             | −0.027                   |
| 530   | $A_2$             | 81         | 2.1      | 3651.798592(3)             | −0.044                   |
| 531   | $E$               | 77         | 2.1      | 3651.897782(2)             | −0.045                   |
| 532   | $E$               | 78         | 2.1      | 3651.897782(2)             | −0.048                   |
| 533   | $A_1$             | 77         | 2.1      | 3652.007008(3)             | −0.050                   |
| 534   | $A_1$             | 48         | 0.55     | 3673.002211(1)             | −0.051                   |
| 535   | $A_1$             | 78         | 2.2      | 3687.890982(3)             | −0.047                   |
| 536   | $E$               | 80         | 2.1      | 3687.978723(2)             | −0.040                   |
| 537   | $E$               | 68         | 2.1      | 3687.978724(2)             | −0.050                   |
| 538   | $A_2$             | 66         | 2.1      | 3688.018740(1)             | −0.041                   |
| 539   | $E$               | 104        | 2.0      | 3690.212962(2)             | −0.018                   |
| 540   | $E$               | 93         | 2.0      | 3690.212962(4)             | −0.026                   |
| 541   | $E$               | 92         | 2.0      | 3690.237985(3)             | −0.034                   |
| 542   | $E$               | 95         | 2.0      | 3690.237985(3)             | −0.035                   |
| 543   | $A_1$             | 54         | 0.54     | 3694.700861(2)             | −0.051                   |
| 544   | $A_1$             | 116        | 2.1      | 3697.248945(1)             | −0.024                   |
| 545   | $A_2$             | 117        | 2.1      | 3697.248946(1)             | −0.025                   |
| 546   | $E$               | 97         | 2.1      | 3697.258966(7)             | −0.040                   |
| 547   | $E$               | 76         | 2.1      | 3697.258973(9)             | −0.041                   |
| 548   | $E$               | 85         | 0.44     | 3697.855649(3)             | −0.032                   |
| 549   | $E$               | 85         | 0.45     | 3697.855649(4)             | −0.034                   |
| 550   | $A_1$             | 88         | 0.49     | 3699.314685(1)             | −0.032                   |
| 551   | $E$               | 65         | 0.021    | 3700.9372593(9)            | −0.031                   |
| 552   | $E$               | 74         | 0.019    | 3700.937260(1)             | −0.035                   |
| 553   | $E$               | 117        | 2.1      | 3701.405826(2)             | −0.025                   |
| 554   | $E$               | 103        | 2.1      | 3701.405826(3)             | −0.036                   |
| 555   | $A_1$             | 74         | 2.1      | 3701.500154(9)             | −0.031                   |
| 556   | $A_2$             | 73         | 2.1      | 3701.500424(7)             | −0.033                   |
| 557   | $E$               | 85         | 0.47     | 3702.970549(5)             | −0.015                   |
| 558   | $E$               | 86         | 0.48     | 3702.970549(5)             | −0.047                   |
| 559   | $E$               | 111        | 2.0      | 3704.860615(1)             | −0.033                   |
| 560   | $E$               | 102        | 2.0      | 3704.860616(2)             | −0.034                   |
| 561   | $A_2$             | 80         | 2.0      | 3704.880357(7)             | −0.034                   |
| 562   | $A_1$             | 92         | 2.1      | 3704.894945(4)             | −0.035                   |
| 563   | $E$               | 71         | 0.057    | 3706.344347(6)             | −0.032                   |
| 564   | $E$               | 81         | 0.059    | 3706.344349(8)             | −0.035                   |
| 565   | $E$               | 66         | 0.13     | 3713.059191(1)             | −0.026                   |
| 566   | $E$               | 60         | 0.13     | 3713.059191(2)             | −0.029                   |
| 567   | $A_1$             | 106        | 2.5      | 3720.540947(3)             | −0.047                   |
| 568   | $E$               | 90         | 2.4      | 3720.661646(8)             | −0.044                   |
| 569   | $E$               | 85         | 2.4      | 3720.661653(7)             | −0.048                   |
| 570   | $A_2$             | 88         | 2.3      | 3720.715460(5)             | −0.048                   |
| 571   | $A_2$             | 49         | 0.2      | 3722.492442(9)             | −0.029                   |
| 572   | $A_1$             | 48         | 0.2      | 3722.492442(7)             | −0.035                   |
| 573   | $E$               | 63         | 0.25     | 3729.233195(2)             | −0.032                   |
| 574   | $E$               | 67         | 0.25     | 3729.233195(3)             | −0.035                   |
| 575   | $E$               | 107        | 0.36     | 3730.146375(4)             | −0.038                   |

Continued on next page.

TABLE S4 – states on Sarka/Poirier CSC PES; continued from previous page

| State | $\Gamma_{C_{3v}}$ | $D_{\max}$ | $S_{vN}$ | $\tilde{E}/\text{cm}^{-1}$ | $\Delta\text{Ref. [30]}$ |
|-------|-------------------|------------|----------|----------------------------|--------------------------|
| 576   | $E$               | 107        | 0.37     | 3730.146376(2)             | −0.045                   |
| 577   | $E$               | 80         | 0.52     | 3731.209093(3)             | −0.070                   |
| 578   | $E$               | 87         | 0.53     | 3731.209093(2)             | −0.073                   |
| 579   | $A_1$             | 111        | 0.4      | 3731.597512(3)             | −0.037                   |
| 580   | $A_1$             | 76         | 0.53     | 3732.677858(3)             | −0.070                   |
| 581   | $E$               | 68         | 0.27     | 3733.278739(1)             | −0.030                   |
| 582   | $E$               | 68         | 0.28     | 3733.278739(2)             | −0.033                   |
| 583   | $E$               | 59         | 0.14     | 3734.408578(1)             | −0.044                   |
| 584   | $E$               | 54         | 0.14     | 3734.408578(2)             | −0.046                   |
| 585   | $A_1$             | 68         | 0.28     | 3734.627435(1)             | −0.034                   |
| 586   | $A_2$             | 106        | 2.2      | 3735.549163(2)             | −0.042                   |
| 587   | $A_1$             | 102        | 2.2      | 3735.557189(2)             | −0.039                   |
| 588   | $E$               | 103        | 2.1      | 3735.645600(3)             | −0.038                   |
| 589   | $E$               | 89         | 2.1      | 3735.645605(9)             | −0.042                   |
| 590   | $E$               | 49         | 0.11     | 3735.943159(1)             | −0.041                   |
| 591   | $E$               | 51         | 0.11     | 3735.943160(1)             | −0.067                   |
| 592   | $E$               | 87         | 0.19     | 3737.060951(3)             | −0.038                   |
| 593   | $E$               | 84         | 0.19     | 3737.060951(4)             | −0.040                   |
| 594   | $E$               | 63         | 0.17     | 3738.726174(1)             | −0.046                   |
| 595   | $E$               | 66         | 0.17     | 3738.726174(1)             | −0.047                   |
| 596   | $A_1$             | 64         | 0.18     | 3740.165576(1)             | −0.046                   |
| 597   | $E$               | 56         | 0.13     | 3759.43552(1)              | −0.038                   |
| 598   | $E$               | 52         | 0.13     | 3759.435526(3)             | −0.056                   |
| 599   | $E$               | 64         | 0.32     | 3767.092971(6)             | −0.045                   |
| 600   | $E$               | 80         | 0.32     | 3767.092972(5)             | −0.045                   |
| 601   | $E$               | 88         | 0.4      | 3771.398625(1)             | −0.044                   |
| 602   | $E$               | 73         | 0.4      | 3771.398626(2)             | −0.045                   |
| 603   | $A_1$             | 64         | 0.42     | 3772.834043(5)             | −0.046                   |
| 604   | $A_1$             | 49         | 0.22     | 3774.471568(5)             | −0.056                   |
| 605   | $A_2$             | 45         | 0.22     | 3774.471569(3)             | −0.060                   |
| 606   | $E$               | 71         | 0.38     | 3777.343739(1)             | −0.047                   |
| 607   | $E$               | 75         | 0.38     | 3777.343739(1)             | −0.075                   |
| 608   | $E$               | 97         | 2.2      | 3787.442633(5)             | −0.040                   |
| 609   | $E$               | 101        | 2.2      | 3787.442634(5)             | −0.041                   |
| 610   | $A_1$             | 74         | 2.1      | 3787.58815(1)              | −0.041                   |
| 611   | $A_2$             | 71         | 2.1      | 3787.58816(1)              | −0.042                   |
| 612   | $E$               | 102        | 2.3      | 3793.122103(9)             | −0.038                   |
| 613   | $E$               | 105        | 2.3      | 3793.122104(8)             | −0.040                   |
| 614   | $E$               | 89         | 2.3      | 3793.22571(1)              | −0.041                   |
| 615   | $E$               | 108        | 2.3      | 3793.22571(1)              | −0.041                   |
| 616   | $E$               | 75         | 0.24     | 3794.369075(1)             | −0.038                   |
| 617   | $E$               | 64         | 0.24     | 3794.369077(2)             | −0.058                   |
| 618   | $A_1$             | 100        | 2.4      | 3795.782933(6)             | −0.038                   |
| 619   | $E$               | 84         | 2.3      | 3796.03803(1)              | −0.040                   |
| 620   | $E$               | 90         | 2.3      | 3796.03804(1)              | −0.042                   |
| 621   | $A_2$             | 79         | 2.3      | 3796.208266(2)             | −0.040                   |
| 622   | $E$               | 97         | 2.1      | 3808.217635(4)             | −0.037                   |
| 623   | $E$               | 94         | 2.1      | 3808.217637(3)             | −0.038                   |
| 624   | $E$               | 76         | 3.0      | 3809.11400(2)              | −0.035                   |
| 625   | $E$               | 78         | 3.0      | 3809.11400(2)              | −0.039                   |
| 626   | $A_1$             | 75         | 3.1      | 3809.11886(2)              | −0.036                   |
| 627   | $A_2$             | 74         | 3.0      | 3809.11972(1)              | −0.040                   |
| 628   | $E$               | 78         | 2.1      | 3809.528889(7)             | −0.031                   |
| 629   | $E$               | 86         | 2.1      | 3809.528890(9)             | −0.047                   |
| 630   | $E$               | 75         | 0.12     | 3837.920379(1)             | −0.038                   |
| 631   | $E$               | 74         | 0.12     | 3837.920379(1)             | −0.058                   |
| 632   | $E$               | 62         | 0.14     | 3851.035896(2)             | −0.041                   |
| 633   | $E$               | 74         | 0.14     | 3851.035896(1)             | −0.041                   |
| 634   | $E$               | 72         | 2.1      | 3854.43129(1)              | −0.037                   |

Continued on next page.

TABLE S4 – states on Sarka/Poirier CSC PES; continued from previous page

| State | $\Gamma_{C_{3v}}$ | $D_{\max}$ | $S_{vN}$ | $\tilde{E}/\text{cm}^{-1}$ | $\Delta\text{Ref. [30]}$ |
|-------|-------------------|------------|----------|----------------------------|--------------------------|
| 635   | $E$               | 78         | 2.1      | 3854.43129(1)              | −0.039                   |
| 636   | $A_1$             | 70         | 2.1      | 3854.44297(1)              | −0.044                   |
| 637   | $A_2$             | 70         | 2.1      | 3854.44297(1)              | −0.046                   |
| 638   | $E$               | 108        | 2.2      | 3858.704162(3)             | −0.035                   |
| 639   | $E$               | 91         | 2.2      | 3858.704162(9)             | −0.038                   |
| 640   | $A_1$             | 67         | 2.2      | 3858.74553(3)              | −0.038                   |
| 641   | $A_2$             | 69         | 2.2      | 3858.74569(2)              | −0.041                   |
| 642   | $E$               | 107        | 0.49     | 3859.110235(2)             | −0.049                   |
| 643   | $E$               | 96         | 0.49     | 3859.110237(4)             | −0.051                   |
| 644   | $E$               | 83         | 0.42     | 3860.216968(5)             | −0.022                   |
| 645   | $E$               | 87         | 0.43     | 3860.216968(5)             | −0.051                   |
| 646   | $A_2$             | 74         | 0.37     | 3860.619570(1)             | −0.041                   |
| 647   | $A_1$             | 76         | 0.38     | 3860.619570(1)             | −0.044                   |
| 648   | $E$               | 90         | 2.4      | 3864.57202(1)              | −0.042                   |
| 649   | $E$               | 83         | 2.4      | 3864.57202(4)              | −0.043                   |
| 650   | $A_1$             | 86         | 2.6      | 3864.60488(3)              | −0.045                   |
| 651   | $A_2$             | 88         | 2.6      | 3864.60969(2)              | −0.044                   |
| 652   | $E$               | 74         | 0.51     | 3867.468134(2)             | −0.039                   |
| 653   | $E$               | 77         | 0.51     | 3867.468135(1)             | −0.047                   |
| 654   | $E$               | 132        | 2.3      | 3869.188892(3)             | −0.030                   |
| 655   | $E$               | 126        | 2.3      | 3869.188892(3)             | −0.032                   |
| 656   | $A_1$             | 123        | 2.6      | 3869.294069(4)             | −0.034                   |
| 657   | $A_2$             | 131        | 2.6      | 3869.294347(2)             | −0.043                   |
| 658   | $E$               | 119        | 0.45     | 3870.711451(2)             | −0.014                   |
| 659   | $E$               | 116        | 0.45     | 3870.711452(2)             | −0.047                   |
| 660   | $E$               | 76         | 0.59     | 3871.578517(1)             | −0.036                   |
| 661   | $E$               | 67         | 0.59     | 3871.578517(3)             | −0.043                   |
| 662   | $A_1$             | 70         | 0.61     | 3872.948853(2)             | −0.039                   |
| 663   | $A_1$             | 72         | 0.43     | 3876.87628(1)              | −0.036                   |
| 664   | $E$               | 127        | 1.3      | 3880.125986(2)             | −0.030                   |
| 665   | $E$               | 129        | 1.3      | 3880.125986(2)             | −0.041                   |
| 666   | $E$               | 90         | 1.2      | 3880.34481(1)              | −0.030                   |
| 667   | $E$               | 90         | 1.2      | 3880.34481(1)              | −0.032                   |
| 668   | $A_1$             | 93         | 0.17     | 3881.614952(8)             | −0.030                   |
| 669   | $A_2$             | 57         | 0.12     | 3881.76330(1)              | −0.047                   |
| 670   | $A_1$             | 58         | 0.11     | 3881.76331(1)              | −0.049                   |
| 671   | $A_2$             | 88         | 0.17     | 3881.781074(7)             | −0.032                   |
| 672   | $E$               | 69         | 0.038    | 3883.877712(1)             | −0.034                   |
| 673   | $E$               | 65         | 0.038    | 3883.877713(2)             | −0.037                   |
| 674   | $E$               | 61         | 0.13     | 3884.673998(4)             | −0.044                   |
| 675   | $E$               | 59         | 0.13     | 3884.673998(4)             | −0.050                   |
| 676   | $A_1$             | 82         | 0.084    | 3897.084031(2)             | −0.052                   |
| 677   | $E$               | 68         | 0.073    | 3902.543038(2)             | −0.040                   |
| 678   | $E$               | 68         | 0.073    | 3902.543040(2)             | −0.052                   |
| 679   | $E$               | 59         | 0.42     | 3904.240480(1)             | −0.051                   |
| 680   | $E$               | 68         | 0.42     | 3904.240480(1)             | −0.056                   |
| 681   | $A_1$             | 71         | 0.45     | 3905.708772(1)             | −0.051                   |
| 682   | $A_1$             | 53         | 0.45     | 3909.845546(1)             | −0.074                   |
| 683   | $A_1$             | 53         | 2.0      | 3913.51924(5)              | −0.019                   |
| 684   | $A_2$             | 56         | 2.0      | 3913.51960(4)              | −0.019                   |
| 685   | $E$               | 54         | 2.0      | 3913.53255(4)              | −0.106                   |
| 686   | $E$               | 51         | 2.0      | 3913.53255(6)              | −0.122                   |
| 687   | $A_1$             | 104        | 2.3      | 3913.936166(7)             | −0.043                   |
| 688   | $A_2$             | 99         | 2.3      | 3913.936167(8)             | −0.044                   |
| 689   | $E$               | 98         | 2.2      | 3914.08704(1)              | −0.043                   |
| 690   | $E$               | 98         | 2.2      | 3914.08704(1)              | −0.044                   |
| 691   | $E$               | 62         | 0.034    | 3914.995211(1)             | −0.012                   |
| 692   | $E$               | 75         | 0.034    | 3914.995211(1)             | −0.115                   |
| 693   | $E$               | 51         | 0.22     | 3917.356531(2)             | −0.097                   |

Continued on next page.

TABLE S4 – states on Sarka/Poirier CSC PES; continued from previous page

| State | $\Gamma_{C_{3v}}$ | $D_{\max}$ | $S_{vN}$ | $\tilde{E}/\text{cm}^{-1}$ | $\Delta\text{Ref. [30]}$ |
|-------|-------------------|------------|----------|----------------------------|--------------------------|
| 694   | $E$               | 69         | 0.22     | 3917.356531(1)             | −0.141                   |
| 695   | $E$               | 94         | 2.3      | 3918.27182(1)              | −0.041                   |
| 696   | $E$               | 101        | 2.3      | 3918.27182(1)              | −0.044                   |
| 697   | $A_1$             | 89         | 2.2      | 3918.37606(5)              | −0.043                   |
| 698   | $A_2$             | 80         | 2.2      | 3918.37621(5)              | −0.043                   |
| 699   | $E$               | 88         | 0.41     | 3919.799587(7)             | −0.036                   |
| 700   | $E$               | 98         | 0.39     | 3919.799588(7)             | −0.046                   |
| 701   | $E$               | 80         | 0.59     | 3928.305756(2)             | −0.050                   |
| 702   | $E$               | 58         | 0.59     | 3928.30576(1)              | −0.056                   |
| 703   | $E$               | 105        | 0.25     | 3929.618464(4)             | −0.026                   |
| 704   | $E$               | 108        | 0.25     | 3929.618465(4)             | −0.032                   |
| 705   | $A_1$             | 69         | 0.63     | 3929.770989(3)             | −0.051                   |
| 706   | $A_1$             | 124        | 3.2      | 3934.821099(6)             | −0.033                   |
| 707   | $A_2$             | 134        | 3.2      | 3934.821109(6)             | −0.034                   |
| 708   | $E$               | 128        | 2.1      | 3935.208343(2)             | −0.032                   |
| 709   | $E$               | 115        | 2.1      | 3935.208344(4)             | −0.034                   |
| 710   | $A_1$             | 107        | 1.9      | 3935.38862(3)              | −0.032                   |
| 711   | $A_2$             | 94         | 1.9      | 3935.38865(3)              | −0.037                   |
| 712   | $E$               | 128        | 0.48     | 3938.083982(2)             | −0.024                   |
| 713   | $E$               | 109        | 0.47     | 3938.083983(5)             | −0.047                   |
| 714   | $A_2$             | 71         | 2.2      | 3938.104117(9)             | −0.038                   |
| 715   | $E$               | 74         | 2.2      | 3938.976710(7)             | −0.037                   |
| 716   | $E$               | 92         | 2.2      | 3938.976713(9)             | −0.047                   |
| 717   | $A_1$             | 75         | 2.2      | 3939.37640(1)              | −0.049                   |
| 718   | $E$               | 120        | 2.4      | 3940.686445(7)             | −0.031                   |
| 719   | $E$               | 119        | 2.4      | 3940.686447(8)             | −0.037                   |
| 720   | $E$               | 121        | 2.1      | 3940.832042(6)             | −0.031                   |
| 721   | $E$               | 122        | 2.1      | 3940.832042(7)             | −0.036                   |
| 722   | $E$               | 108        | 2.2      | 3943.567896(6)             | −0.027                   |
| 723   | $E$               | 101        | 2.2      | 3943.567899(6)             | −0.033                   |
| 724   | $A_1$             | 90         | 2.2      | 3943.61299(1)              | −0.035                   |
| 725   | $A_2$             | 86         | 2.2      | 3943.62382(2)              | −0.032                   |
| 726   | $E$               | 98         | 2.2      | 3944.017401(5)             | −0.047                   |
| 727   | $E$               | 94         | 2.2      | 3944.017401(7)             | −0.048                   |
| 728   | $E$               | 79         | 2.1      | 3944.098856(4)             | −0.048                   |
| 729   | $E$               | 102        | 2.1      | 3944.098863(9)             | −0.050                   |
| 730   | $A_1$             | 87         | 2.4      | 3946.79407(1)              | −0.052                   |
| 731   | $E$               | 106        | 2.3      | 3946.962023(3)             | −0.043                   |
| 732   | $E$               | 98         | 2.3      | 3946.962023(5)             | −0.054                   |
| 733   | $A_2$             | 71         | 2.2      | 3947.068750(6)             | −0.044                   |
| 734   | $A_2$             | 135        | 2.4      | 3948.385569(3)             | −0.035                   |
| 735   | $E$               | 115        | 2.4      | 3948.508553(6)             | −0.036                   |
| 736   | $E$               | 109        | 2.3      | 3948.508554(9)             | −0.037                   |
| 737   | $A_1$             | 104        | 2.3      | 3948.63911(1)              | −0.039                   |
| 738   | $A_1$             | 126        | 3.3      | 3953.996671(3)             | −0.034                   |
| 739   | $E$               | 89         | 3.0      | 3954.04741(2)              | −0.025                   |
| 740   | $E$               | 128        | 3.0      | 3954.04742(2)              | −0.037                   |
| 741   | $A_2$             | 84         | 3.3      | 3954.04800(3)              | −0.039                   |
| 742   | $E$               | 107        | 2.8      | 3954.363748(7)             | −0.025                   |
| 743   | $E$               | 102        | 2.8      | 3954.363749(8)             | −0.036                   |
| 744   | $E$               | 113        | 2.9      | 3954.380976(5)             | −0.037                   |
| 745   | $E$               | 106        | 2.9      | 3954.380976(7)             | −0.038                   |
| 746   | $E$               | 75         | 0.13     | 3975.080136(1)             | −0.042                   |
| 747   | $E$               | 81         | 0.13     | 3975.080137(1)             | −0.042                   |
| 748   | $E$               | 86         | 2.1      | 3981.727830(4)             | −0.039                   |
| 749   | $E$               | 104        | 2.1      | 3981.727831(4)             | −0.040                   |
| 750   | $E$               | 93         | 2.1      | 3981.732083(5)             | −0.050                   |
| 751   | $E$               | 89         | 2.1      | 3981.732084(7)             | −0.051                   |
| 752   | $E$               | 80         | 0.19     | 3983.435660(2)             | −0.044                   |

Continued on next page.

TABLE S4 – states on Sarka/Poirier CSC PES; continued from previous page

| State | $\Gamma_{C_{3v}}$ | $D_{\max}$ | $S_{vN}$ | $\tilde{E}/\text{cm}^{-1}$ | $\Delta\text{Ref. [30]}$ |
|-------|-------------------|------------|----------|----------------------------|--------------------------|
| 753   | $E$               | 56         | 0.19     | 3983.43566(2)              | −0.045                   |
| 754   | $A_2$             | 90         | 2.1      | 3984.44333(1)              | −0.041                   |
| 755   | $E$               | 127        | 2.1      | 3984.654582(1)             | −0.041                   |
| 756   | $E$               | 95         | 2.1      | 3984.654585(5)             | −0.043                   |
| 757   | $A_1$             | 92         | 2.1      | 3984.854174(3)             | −0.045                   |
| 758   | $A_1$             | 56         | 0.22     | 3989.00769(4)              | −0.043                   |
| 759   | $A_2$             | 57         | 0.22     | 3989.00772(2)              | −0.048                   |
| 760   | $E$               | 81         | 0.23     | 3991.794287(1)             | −0.038                   |
| 761   | $E$               | 63         | 0.23     | 3991.794288(6)             | −0.056                   |
| 762   | $A_1^*$           | 74         | 0.21     | 3997.561530(1)             | −0.045                   |
| 763   | $A_2^*$           | 78         | 0.21     | 3997.561530(1)             | −0.047                   |
| 764   | $E$               | 97         | 2.1      | 4001.276692(3)             | −0.031                   |
| 765   | $E$               | 104        | 2.1      | 4001.276692(2)             | −0.035                   |
| 766   | $A_2$             | 74         | 2.0      | 4001.518693(5)             | −0.032                   |
| 767   | $A_1$             | 72         | 2.0      | 4001.518695(4)             | −0.035                   |
| 768   | $E$               | 121        | 2.1      | 4001.744491(6)             | −0.038                   |
| 769   | $E$               | 121        | 2.1      | 4001.744492(6)             | −0.038                   |
| 770   | $E$               | 132        | 3.2      | 4002.566812(4)             | −0.033                   |
| 771   | $E$               | 144        | 3.2      | 4002.566813(3)             | −0.033                   |
| 772   | $A_2$             | 84         | 3.0      | 4002.67592(1)              | −0.033                   |
| 773   | $A_1$             | 85         | 3.0      | 4002.67592(2)              | −0.033                   |
| 774   | $E$               | 126        | 2.1      | 4003.046724(3)             | −0.031                   |
| 775   | $E$               | 116        | 2.1      | 4003.046724(5)             | −0.032                   |
| 776   | $E$               | 83         | 0.49     | 4004.524553(1)             | −0.050                   |
| 777   | $E$               | 83         | 0.49     | 4004.524553(1)             | −0.055                   |
| 778   | $E$               | 141        | 2.3      | 4006.045036(3)             | −0.032                   |
| 779   | $E$               | 141        | 2.3      | 4006.045036(3)             | −0.037                   |
| 780   | $A_2$             | 139        | 3.7      | 4006.696662(3)             | −0.034                   |
| 781   | $A_1$             | 133        | 3.1      | 4006.911004(2)             | −0.036                   |
| 782   | $E$               | 124        | 3.1      | 4006.972306(8)             | −0.030                   |
| 783   | $E$               | 135        | 3.1      | 4006.972306(7)             | −0.036                   |
| 784   | $E$               | 127        | 2.2      | 4007.349302(2)             | −0.032                   |
| 785   | $E$               | 128        | 2.2      | 4007.349302(3)             | −0.035                   |
| 786   | $A_2$             | 134        | 3.0      | 4007.719704(4)             | −0.030                   |
| 787   | $E$               | 102        | 2.3      | 4008.414094(4)             | −0.032                   |
| 788   | $E$               | 120        | 2.3      | 4008.414100(7)             | −0.032                   |
| 789   | $E$               | 86         | 0.62     | 4008.703819(1)             | −0.051                   |
| 790   | $E$               | 88         | 0.62     | 4008.703819(1)             | −0.057                   |
| 791   | $A_1$             | 94         | 2.1      | 4008.790906(8)             | −0.034                   |
| 792   | $A_1$             | 81         | 0.67     | 4010.097148(2)             | −0.054                   |
| 793   | $E$               | 122        | 2.2      | 4010.926002(2)             | −0.032                   |
| 794   | $E$               | 100        | 2.2      | 4010.926003(8)             | −0.035                   |
| 795   | $E$               | 125        | 2.1      | 4011.120043(2)             | −0.034                   |
| 796   | $E$               | 92         | 2.1      | 4011.120045(8)             | −0.037                   |
| 797   | $E$               | 94         | 2.1      | 4015.521607(3)             | −0.041                   |
| 798   | $E$               | 99         | 2.1      | 4015.521607(3)             | −0.041                   |
| 799   | $A_1$             | 74         | 2.1      | 4015.525939(6)             | −0.054                   |
| 800   | $A_2$             | 77         | 2.1      | 4015.525973(4)             | −0.060                   |
| 801   | $E$               | 80         | 0.27     | 4017.007311(3)             | −0.040                   |
| 802   | $E$               | 74         | 0.25     | 4017.007314(2)             | −0.057                   |
| 803   | $A_1$             | 98         | 2.2      | 4017.82270(1)              | −0.031                   |
| 804   | $A_2$             | 108        | 2.2      | 4017.822705(7)             | −0.038                   |
| 805   | $E$               | 110        | 2.2      | 4017.975225(5)             | −0.032                   |
| 806   | $E$               | 91         | 2.2      | 4017.975229(6)             | −0.041                   |
| 807   | $E$               | 98         | 2.3      | 4021.932913(8)             | −0.028                   |
| 808   | $E$               | 111        | 2.3      | 4021.932914(7)             | −0.038                   |
| 809   | $A_1$             | 89         | 2.2      | 4022.08514(1)              | −0.032                   |
| 810   | $A_2$             | 88         | 2.2      | 4022.085459(5)             | −0.036                   |
| 811   | $E$               | 93         | 0.63     | 4022.255373(1)             | −0.032                   |

Continued on next page.

TABLE S4 – states on Sarka/Poirier CSC PES; continued from previous page

| State | $\Gamma_{C_{3v}}$ | $D_{\max}$ | $S_{vN}$ | $\tilde{E}/\text{cm}^{-1}$ | $\Delta\text{Ref. [30]}$ |
|-------|-------------------|------------|----------|----------------------------|--------------------------|
| 812   | $E$               | 92         | 0.63     | 4022.255373(1)             | −0.034                   |
| 813   | $E$               | 88         | 0.54     | 4023.479608(5)             | −0.030                   |
| 814   | $E$               | 89         | 0.54     | 4023.479608(5)             | −0.034                   |
| 815   | $E$               | 84         | 2.1      | 4029.381477(2)             | −0.029                   |
| 816   | $E$               | 93         | 2.1      | 4029.381478(1)             | −0.041                   |
| 817   | $A_2$             | 87         | 2.0      | 4029.716302(1)             | −0.033                   |
| 818   | $A_1$             | 92         | 2.0      | 4029.734772(1)             | −0.035                   |
| 819   | $E$               | 50         | 0.57     | 4035.969891(5)             | −0.052                   |
| 820   | $E$               | 46         | 0.57     | 4035.96989(1)              | −0.054                   |
| 821   | $E$               | 83         | 0.068    | 4045.808551(3)             | −0.013                   |
| 822   | $E$               | 93         | 0.07     | 4045.808552(4)             | −0.062                   |
| 823   | $E$               | 72         | 0.53     | 4052.3955519(6)            | −0.062                   |
| 824   | $E$               | 81         | 0.53     | 4052.395554(2)             | −0.080                   |
| 825   | $E$               | 79         | 2.2      | 4052.455476(3)             | −0.046                   |
| 826   | $E$               | 83         | 2.2      | 4052.455478(4)             | −0.050                   |
| 827   | $A_1$             | 65         | 2.2      | 4052.51214(1)              | −0.047                   |
| 828   | $A_2$             | 105        | 2.2      | 4052.51219(1)              | −0.053                   |
| 829   | $E$               | 73         | 0.22     | 4053.961885(2)             | −0.041                   |
| 830   | $E$               | 74         | 0.23     | 4053.961886(1)             | −0.052                   |
| 831   | $A_1$             | 93         | 0.056    | 4056.758391(1)             | −0.046                   |
| 832   | $A_2$             | 83         | 0.047    | 4056.928883(2)             | −0.035                   |
| 833   | $E$               | 66         | 0.58     | 4057.379034(4)             | −0.053                   |
| 834   | $E$               | 59         | 0.58     | 4057.379035(5)             | −0.054                   |
| 835   | $E$               | 96         | 2.0      | 4062.541620(4)             | −0.025                   |
| 836   | $E$               | 80         | 2.0      | 4062.541625(6)             | −0.031                   |
| 837   | $A_2$             | 77         | 2.0      | 4062.573303(4)             | −0.037                   |
| 838   | $A_1$             | 93         | 2.0      | 4062.573308(5)             | −0.039                   |
| 839   | $A_2$             | 71         | 0.45     | 4064.37541(1)              | −0.035                   |
| 840   | $A_1$             | 72         | 0.45     | 4064.37542(1)              | −0.036                   |
| 841   | $E$               | 88         | 0.54     | 4067.261631(3)             | −0.032                   |
| 842   | $E$               | 104        | 0.54     | 4067.261632(3)             | −0.034                   |
| 843   | $E$               | 83         | 2.1      | 4070.901475(6)             | −0.023                   |
| 844   | $E$               | 78         | 2.1      | 4070.901476(8)             | −0.025                   |
| 845   | $A_2^*$           | 80         | 2.1      | 4070.903619(4)             | −0.047                   |
| 846   | $A_1^*$           | 80         | 2.1      | 4070.903620(5)             | −0.047                   |
| 847   | $A_1$             | 47         | 1.0      | 4070.9164867(5)            | −0.061                   |
| 848   | $E$               | 93         | 2.0      | 4071.376077(5)             | −0.035                   |
| 849   | $E$               | 124        | 2.0      | 4071.376079(5)             | −0.037                   |
| 850   | $E$               | 96         | 2.1      | 4071.421485(3)             | −0.036                   |
| 851   | $E$               | 125        | 2.1      | 4071.421489(6)             | −0.037                   |
| 852   | $A_2$             | 112        | 2.1      | 4074.297763(7)             | −0.033                   |
| 853   | $A_1$             | 77         | 2.1      | 4074.298733(4)             | −0.034                   |
| 854   | $E$               | 83         | 2.1      | 4074.313577(7)             | −0.034                   |
| 855   | $E$               | 85         | 2.1      | 4074.313578(7)             | −0.036                   |
| 856   | $E$               | 124        | 2.1      | 4076.432270(2)             | −0.031                   |
| 857   | $E$               | 93         | 2.1      | 4076.432273(4)             | −0.036                   |
| 858   | $E$               | 128        | 2.1      | 4076.489519(1)             | −0.036                   |
| 859   | $E$               | 99         | 2.1      | 4076.489520(7)             | −0.040                   |
| 860   | $E$               | 66         | 0.021    | 4078.824566(1)             | −0.036                   |
| 861   | $E$               | 62         | 0.021    | 4078.824566(1)             | −0.038                   |
| 862   | $A_2$             | 101        | 2.2      | 4078.864030(3)             | −0.037                   |
| 863   | $E$               | 93         | 2.2      | 4079.310757(5)             | −0.034                   |
| 864   | $E$               | 79         | 2.2      | 4079.310762(5)             | −0.036                   |
| 865   | $A_1$             | 84         | 2.2      | 4079.662996(2)             | −0.038                   |
| 866   | $E$               | 123        | 2.4      | 4084.821684(3)             | −0.048                   |
| 867   | $E$               | 112        | 2.4      | 4084.821684(6)             | −0.048                   |
| 868   | $A_1$             | 80         | 2.4      | 4084.90086(3)              | −0.050                   |
| 869   | $A_2$             | 73         | 2.4      | 4084.90093(6)              | −0.052                   |
| 870   | $E$               | 87         | 0.49     | 4086.347015(8)             | −0.041                   |

Continued on next page.



TABLE S4 – states on Sarka/Poirier CSC PES; continued from previous page

| State | $\Gamma_{C_{3v}}$ | $D_{\max}$ | $S_{vN}$ | $\tilde{E}/\text{cm}^{-1}$ | $\Delta\text{Ref. [30]}$ |
|-------|-------------------|------------|----------|----------------------------|--------------------------|
| 871   | $E$               | 94         | 0.49     | 4086.347019(9)             | −0.058                   |
| 872   | $A_1$             | 51         | 1.2      | 4086.551489(2)             | −0.065                   |
| 873   | $A_2$             | 49         | 0.15     | 4092.14852(1)              | −0.031                   |
| 874   | $A_1$             | 50         | 0.15     | 4092.148521(8)             | −0.034                   |
| 875   | $E$               | 66         | 0.038    | 4092.356304(1)             | −0.012                   |
| 876   | $E$               | 59         | 0.039    | 4092.356304(2)             | −0.121                   |
| 877   | $A_1$             | 86         | 0.35     | 4095.90680(2)              | −0.046                   |
| 878   | $A_2$             | 93         | 0.35     | 4095.906809(7)             | −0.049                   |
| 879   | $A_1$             | 94         | 2.3      | 4097.200424(2)             | −0.059                   |
| 880   | $E$               | 88         | 2.2      | 4097.282114(3)             | −0.060                   |
| 881   | $E$               | 73         | 2.2      | 4097.282118(4)             | −0.071                   |
| 882   | $A_2$             | 85         | 2.1      | 4097.324464(3)             | −0.065                   |
| 883   | $A_1$             | 63         | 0.47     | 4097.698844(6)             | −0.073                   |
| 884   | $A_2$             | 61         | 0.47     | 4097.698846(5)             | −0.077                   |
| 885   | $E$               | 113        | 0.44     | 4098.778145(8)             | −0.031                   |
| 886   | $E$               | 114        | 0.44     | 4098.778146(9)             | −0.057                   |
| 887   | $E$               | 88         | 0.49     | 4100.604341(2)             | −0.069                   |
| 888   | $E$               | 77         | 0.49     | 4100.604342(3)             | −0.085                   |
| 889   | $E$               | 124        | 2.3      | 4101.284675(4)             | −0.044                   |
| 890   | $E$               | 113        | 2.3      | 4101.284677(5)             | −0.044                   |
| 891   | $E$               | 103        | 2.1      | 4101.427821(5)             | −0.044                   |
| 892   | $E$               | 124        | 2.1      | 4101.427827(8)             | −0.045                   |
| 893   | $E$               | 75         | 0.23     | 4102.814147(2)             | −0.035                   |
| 894   | $E$               | 76         | 0.23     | 4102.814147(1)             | −0.037                   |
| 895   | $E$               | 57         | 0.14     | 4103.414945(1)             | −0.049                   |
| 896   | $E$               | 52         | 0.14     | 4103.414946(2)             | −0.050                   |
| 897   | $E$               | 127        | 2.3      | 4104.222310(4)             | −0.039                   |
| 898   | $E$               | 88         | 2.3      | 4104.22232(1)              | −0.046                   |
| 899   | $A_1$             | 86         | 2.2      | 4104.26698(2)              | −0.047                   |
| 900   | $A_2$             | 90         | 2.2      | 4104.27444(3)              | −0.042                   |
| 901   | $A_1$             | 45         | 0.19     | 4109.109098(3)             | −0.047                   |
| 902   | $A_2$             | 49         | 0.19     | 4109.109111(3)             | −0.051                   |
| 903   | $E$               | 74         | 0.29     | 4110.817150(3)             | −0.036                   |
| 904   | $E$               | 74         | 0.29     | 4110.8171508(9)            | −0.040                   |
| 905   | $E$               | 64         | 0.2      | 4111.956781(1)             | −0.045                   |
| 906   | $E$               | 71         | 0.2      | 4111.956781(1)             | −0.054                   |
| 907   | $A_1$             | 53         | 0.32     | 4116.15423(1)              | −0.033                   |
| 908   | $A_2$             | 50         | 0.32     | 4116.15435(1)              | −0.038                   |
| 909   | $E$               | 59         | 0.34     | 4118.823394(7)             | −0.019                   |
| 910   | $E$               | 71         | 0.34     | 4118.823394(3)             | −0.057                   |
| 911   | $A_2$             | 71         | 2.1      | 4122.377482(1)             | −0.047                   |
| 912   | $E$               | 81         | 2.1      | 4122.476394(1)             | −0.049                   |
| 913   | $E$               | 75         | 2.1      | 4122.476394(1)             | −0.049                   |
| 914   | $A_1$             | 74         | 2.1      | 4122.585282(1)             | −0.051                   |
| 915   | $E$               | 66         | 0.33     | 4135.828234(6)             | −0.048                   |
| 916   | $E$               | 68         | 0.33     | 4135.828234(6)             | −0.049                   |
| 917   | $E$               | 74         | 0.26     | 4140.429295(1)             | −0.066                   |
| 918   | $E$               | 59         | 0.26     | 4140.429295(3)             | −0.071                   |
| 919   | $A_1$             | 60         | 0.45     | 4141.50289(1)              | −0.049                   |
| 920   | $A_2$             | 67         | 0.45     | 4141.502897(5)             | −0.050                   |
| 921   | $E$               | 82         | 0.49     | 4144.340827(2)             | −0.043                   |
| 922   | $E$               | 76         | 0.49     | 4144.340828(2)             | −0.061                   |
| 923   | $E$               | 76         | 0.5      | 4144.682188(1)             | −0.071                   |
| 924   | $E$               | 80         | 0.5      | 4144.682189(1)             | −0.075                   |
| 925   | $A_1$             | 80         | 0.57     | 4146.100101(1)             | −0.073                   |
| 926   | $A_2$             | 100        | 2.3      | 4157.009620(1)             | −0.047                   |
| 927   | $E$               | 105        | 2.3      | 4157.109291(3)             | −0.048                   |
| 928   | $E$               | 101        | 2.3      | 4157.109293(2)             | −0.051                   |
| 929   | $A_1$             | 93         | 2.3      | 4157.218876(2)             | −0.050                   |

Continued on next page.

TABLE S4 – states on Sarka/Poirier CSC PES; continued from previous page

| State | $\Gamma_{C_{3v}}$ | $D_{\max}$ | $S_{vN}$ | $\tilde{E}/\text{cm}^{-1}$ | $\Delta\text{Ref. [30]}$ |
|-------|-------------------|------------|----------|----------------------------|--------------------------|
| 930   | $E$               | 102        | 2.2      | 4157.632915(5)             | −0.043                   |
| 931   | $E$               | 105        | 2.2      | 4157.632915(5)             | −0.045                   |
| 932   | $E$               | 107        | 2.1      | 4157.809703(5)             | −0.043                   |
| 933   | $E$               | 85         | 2.1      | 4157.80971(1)              | −0.045                   |
| 934   | $A_1$             | 60         | 0.072    | 4161.221925(2)             | −0.052                   |
| 935   | $A_1$             | 86         | 2.4      | 4164.650296(9)             | −0.044                   |
| 936   | $A_2$             | 89         | 2.4      | 4164.65030(1)              | −0.046                   |
| 937   | $E$               | 87         | 2.3      | 4164.78244(1)              | −0.045                   |
| 938   | $E$               | 106        | 2.3      | 4164.78245(1)              | −0.048                   |
| 939   | $E$               | 107        | 2.4      | 4168.848614(9)             | −0.033                   |
| 940   | $E$               | 102        | 2.4      | 4168.84861(1)              | −0.049                   |
| 941   | $A_1$             | 85         | 2.4      | 4168.96047(1)              | −0.042                   |
| 942   | $A_2$             | 84         | 2.4      | 4168.96071(1)              | −0.048                   |
| 943   | $E$               | 106        | 0.64     | 4170.361346(3)             | −0.035                   |
| 944   | $E$               | 104        | 0.64     | 4170.361346(6)             | −0.052                   |
| 945   | $E$               | 121        | 2.2      | 4172.515367(5)             | −0.039                   |
| 946   | $E$               | 123        | 2.2      | 4172.515367(4)             | −0.043                   |
| 947   | $A_2$             | 132        | 3.5      | 4173.299629(5)             | −0.043                   |
| 948   | $A_1$             | 137        | 3.1      | 4173.381248(2)             | −0.041                   |
| 949   | $E$               | 135        | 3.1      | 4173.423649(4)             | −0.040                   |
| 950   | $E$               | 135        | 3.1      | 4173.423649(5)             | −0.044                   |
| 951   | $E$               | 49         | 0.13     | 4173.453487(1)             | −0.042                   |
| 952   | $E$               | 76         | 0.13     | 4173.453489(2)             | −0.068                   |
| 953   | $E$               | 121        | 2.1      | 4173.819541(4)             | −0.044                   |
| 954   | $E$               | 122        | 2.1      | 4173.819541(4)             | −0.047                   |
| 955   | $A_2$             | 133        | 2.7      | 4174.075063(2)             | −0.044                   |
| 956   | $E$               | 113        | 2.2      | 4174.880778(5)             | −0.041                   |
| 957   | $E$               | 119        | 2.2      | 4174.880779(4)             | −0.043                   |
| 958   | $A_1$             | 94         | 2.1      | 4175.285844(8)             | −0.043                   |
| 959   | $A_1$             | 89         | 0.075    | 4176.844061(3)             | −0.041                   |
| 960   | $E$               | 78         | 0.068    | 4182.415117(2)             | −0.026                   |
| 961   | $E$               | 80         | 0.068    | 4182.415119(3)             | −0.041                   |
| 962   | $E$               | 88         | 0.045    | 4199.143582(2)             | −0.027                   |
| 963   | $E$               | 74         | 0.045    | 4199.143584(3)             | −0.037                   |
| 964   | $A_1$             | 92         | 2.2      | 4201.140075(1)             | −0.047                   |
| 965   | $E$               | 100        | 2.1      | 4201.267523(3)             | −0.049                   |
| 966   | $E$               | 97         | 2.1      | 4201.267524(2)             | −0.049                   |
| 967   | $A_2$             | 83         | 2.1      | 4201.310603(2)             | −0.052                   |
| 968   | $A_2$             | 73         | 2.1      | 4223.22736(1)              | −0.041                   |
| 969   | $A_1$             | 75         | 2.1      | 4223.22737(1)              | −0.043                   |
| 970   | $E$               | 120        | 2.1      | 4223.245531(2)             | −0.048                   |
| 971   | $E$               | 113        | 2.1      | 4223.245531(3)             | −0.048                   |
| 972   | $E$               | 116        | 0.53     | 4223.983802(5)             | −0.051                   |
| 973   | $E$               | 128        | 0.53     | 4223.983803(5)             | −0.052                   |
| 974   | $A_1$             | 122        | 0.56     | 4225.451392(5)             | −0.053                   |
| 975   | $A_1$             | 65         | 0.16     | 4225.554479(2)             | −0.044                   |
| 976   | $A_2$             | 72         | 0.16     | 4225.554479(1)             | −0.045                   |
| 977   | $E$               | 99         | 2.2      | 4228.887882(6)             | −0.036                   |
| 978   | $E$               | 117        | 2.2      | 4228.887883(4)             | −0.039                   |
| 979   | $E$               | 102        | 2.2      | 4228.909450(4)             | −0.047                   |
| 980   | $E$               | 100        | 2.2      | 4228.909451(4)             | −0.047                   |
| 981   | $E$               | 66         | 0.41     | 4229.073795(1)             | −0.044                   |
| 982   | $E$               | 74         | 0.41     | 4229.073796(2)             | −0.063                   |
| 983   | $A_2$             | 137        | 2.5      | 4229.407647(5)             | −0.046                   |
| 984   | $A_1$             | 135        | 2.5      | 4229.423013(6)             | −0.045                   |
| 985   | $E$               | 99         | 2.6      | 4229.51818(6)              | −0.046                   |
| 986   | $E$               | 126        | 2.6      | 4229.51819(6)              | −0.047                   |
| 987   | $E$               | 116        | 0.48     | 4230.948854(4)             | −0.042                   |
| 988   | $E$               | 114        | 0.48     | 4230.948855(6)             | −0.053                   |

Continued on next page.

TABLE S4 – states on Sarka/Poirier CSC PES; continued from previous page

| State | $\Gamma_{C_{3v}}$ | $D_{\max}$ | $S_{vN}$ | $\tilde{E}/\text{cm}^{-1}$ | $\Delta\text{Ref. [30]}$ |
|-------|-------------------|------------|----------|----------------------------|--------------------------|
| 989   | $A_2$             | 95         | 2.3      | 4231.441698(7)             | −0.041                   |
| 990   | $E$               | 91         | 2.3      | 4231.76903(1)              | −0.039                   |
| 991   | $E$               | 101        | 2.3      | 4231.76903(1)              | −0.042                   |
| 992   | $A_1$             | 95         | 2.3      | 4232.049631(2)             | −0.044                   |
| 993   | $A_2$             | 78         | 2.0      | 4235.559938(1)             | −0.056                   |
| 994   | $E$               | 131        | 2.4      | 4235.586177(2)             | −0.034                   |
| 995   | $E$               | 135        | 2.4      | 4235.586180(4)             | −0.036                   |
| 996   | $E$               | 129        | 2.5      | 4235.711353(3)             | −0.041                   |
| 997   | $E$               | 150        | 2.5      | 4235.711357(5)             | −0.047                   |
| 998   | $E$               | 78         | 2.0      | 4236.060255(1)             | −0.064                   |
| 999   | $E$               | 81         | 2.0      | 4236.060255(1)             | −0.066                   |
| 1000  | $E$               | 78         | 0.43     | 4236.382160(1)             |                          |
| 1001  | $E$               | 77         | 0.43     | 4236.382160(2)             |                          |
| 1002  | $A_1$             | 80         | 2.0      | 4236.611610(1)             |                          |
| 1003  | $A_1$             | 145        | 2.5      | 4238.261876(4)             |                          |
| 1004  | $E$               | 138        | 2.3      | 4238.562605(2)             |                          |
| 1005  | $E$               | 126        | 2.3      | 4238.562608(5)             |                          |
| 1006  | $A_2$             | 126        | 2.2      | 4238.760076(9)             |                          |
| 1007  | $E$               | 93         | 0.45     | 4239.686617(2)             |                          |
| 1008  | $E$               | 96         | 0.45     | 4239.686617(1)             |                          |
| 1009  | $E$               | 80         | 0.6      | 4244.507245(1)             |                          |
| 1010  | $E$               | 78         | 0.6      | 4244.507245(3)             |                          |
| 1011  | $A_1$             | 132        | 1.8      | 4246.493439(3)             |                          |
| 1012  | $A_2$             | 142        | 1.8      | 4246.493690(4)             |                          |
| 1013  | $A_2$             | 72         | 2.0      | 4246.68553(1)              |                          |
| 1014  | $A_1$             | 72         | 2.0      | 4246.68595(1)              |                          |
| 1015  | $E$               | 74         | 2.1      | 4246.69832(1)              |                          |
| 1016  | $E$               | 72         | 2.1      | 4246.69833(1)              |                          |
| 1017  | $A_1$             | 105        | 1.6      | 4246.77392(1)              |                          |
| 1018  | $A_2$             | 94         | 1.6      | 4246.77394(2)              |                          |
| 1019  | $E$               | 109        | 0.74     | 4249.43808(1)              |                          |
| 1020  | $E$               | 133        | 0.73     | 4249.43808(1)              |                          |
| 1021  | $E$               | 108        | 0.72     | 4249.620321(7)             |                          |
| 1022  | $E$               | 108        | 0.73     | 4249.620322(7)             |                          |
| 1023  | $E$               | 61         | 0.13     | 4249.63426(1)              |                          |
| 1024  | $E$               | 62         | 0.13     | 4249.63426(1)              |                          |
| 1025  | $A_1$             | 53         | 0.7      | 4249.92600(1)              |                          |
| 1026  | $A_2$             | 52         | 0.7      | 4249.92607(2)              |                          |
| 1027  | $E$               | 78         | 0.75     | 4252.636045(1)             |                          |
| 1028  | $E$               | 65         | 0.75     | 4252.636045(6)             |                          |
| 1029  | $E$               | 90         | 0.7      | 4252.862092(2)             |                          |
| 1030  | $E$               | 87         | 0.7      | 4252.862092(2)             |                          |
| 1031  | $E$               | 84         | 0.15     | 4253.952219(1)             |                          |
| 1032  | $E$               | 84         | 0.15     | 4253.952219(1)             |                          |
| 1033  | $A_1$             | 60         | 0.16     | 4255.391740(4)             |                          |
| 1034  | $E$               | 99         | 0.29     | 4259.124062(3)             |                          |
| 1035  | $E$               | 101        | 0.29     | 4259.124062(3)             |                          |
| 1036  | $E$               | 74         | 2.2      | 4264.54443(1)              |                          |
| 1037  | $E$               | 75         | 2.2      | 4264.54443(1)              |                          |
| 1038  | $A_1$             | 75         | 2.1      | 4264.58100(1)              |                          |
| 1039  | $A_2$             | 73         | 2.1      | 4264.58484(1)              |                          |
| 1040  | $A_1$             | 48         | 0.44     | 4269.616080(3)             |                          |
| 1041  | $A_2$             | 49         | 0.44     | 4269.616084(3)             |                          |
| 1042  | $E$               | 63         | 0.5      | 4272.518998(2)             |                          |
| 1043  | $E$               | 77         | 0.5      | 4272.518998(1)             |                          |
| 1044  | $E$               | 58         | 0.47     | 4272.630855(1)             |                          |
| 1045  | $E$               | 72         | 0.47     | 4272.630857(2)             |                          |
| 1046  | $E$               | 73         | 0.082    | 4274.300666(1)             |                          |
| 1047  | $E$               | 69         | 0.082    | 4274.300667(1)             |                          |

Continued on next page.

TABLE S4 – states on Sarka/Poirier CSC PES; continued from previous page

| State | $\Gamma_{C_{3v}}$ | $D_{\max}$ | $S_{vN}$ | $\tilde{E}/\text{cm}^{-1}$ | $\Delta\text{Ref. [30]}$ |
|-------|-------------------|------------|----------|----------------------------|--------------------------|
| 1048  | $E$               | 67         | 0.27     | 4279.551950(1)             |                          |
| 1049  | $E$               | 59         | 0.27     | 4279.551950(2)             |                          |
| 1050  | $E$               | 86         | 2.0      | 4280.015257(1)             |                          |
| 1051  | $E$               | 65         | 2.0      | 4280.015257(3)             |                          |
| 1052  | $E$               | 64         | 2.0      | 4280.034057(2)             |                          |
| 1053  | $E$               | 69         | 2.0      | 4280.034057(3)             |                          |
| 1054  | $A_1$             | 74         | 0.39     | 4280.996393(1)             |                          |
| 1055  | $E$               | 64         | 2.0      | 4282.92785(1)              |                          |
| 1056  | $E$               | 63         | 2.0      | 4282.92785(1)              |                          |
| 1057  | $A_1$             | 63         | 2.0      | 4282.92885(1)              |                          |
| 1058  | $A_2$             | 60         | 2.0      | 4282.93937(1)              |                          |
| 1059  | $E$               | 94         | 2.3      | 4283.27311(1)              |                          |
| 1060  | $E$               | 104        | 2.3      | 4283.27311(1)              |                          |
| 1061  | $A_1$             | 78         | 2.2      | 4283.45961(4)              |                          |
| 1062  | $A_2$             | 79         | 2.2      | 4283.45961(5)              |                          |
| 1063  | $E$               | 145        | 2.3      | 4288.992175(2)             |                          |
| 1064  | $E$               | 106        | 2.3      | 4288.99218(1)              |                          |
| 1065  | $E$               | 105        | 2.2      | 4289.12376(1)              |                          |
| 1066  | $E$               | 105        | 2.2      | 4289.12376(1)              |                          |
| 1067  | $A_1$             | 140        | 2.4      | 4291.655406(2)             |                          |
| 1068  | $E$               | 107        | 2.3      | 4291.947125(7)             |                          |
| 1069  | $E$               | 103        | 2.3      | 4291.947125(8)             |                          |
| 1070  | $A_2$             | 90         | 2.2      | 4292.131714(3)             |                          |
| 1071  | $A_1$             | 54         | 0.62     | 4293.39100(2)              |                          |
| 1072  | $A_2$             | 56         | 0.62     | 4293.39100(1)              |                          |
| 1073  | $E$               | 81         | 0.71     | 4296.285007(2)             |                          |
| 1074  | $E$               | 66         | 0.71     | 4296.285008(6)             |                          |
| 1075  | $A_1$             | 89         | 0.26     | 4300.438549(5)             |                          |
| 1076  | $A_2$             | 119        | 0.26     | 4300.438556(4)             |                          |
| 1077  | $E$               | 127        | 2.3      | 4301.481577(2)             |                          |
| 1078  | $E$               | 125        | 2.3      | 4301.481577(3)             |                          |
| 1079  | $E$               | 96         | 3.1      | 4302.37871(2)              |                          |
| 1080  | $E$               | 108        | 3.1      | 4302.37872(2)              |                          |
| 1081  | $A_1$             | 101        | 3.2      | 4302.38852(2)              |                          |
| 1082  | $A_2$             | 106        | 3.2      | 4302.38936(1)              |                          |
| 1083  | $E$               | 102        | 2.2      | 4302.774893(4)             |                          |
| 1084  | $E$               | 117        | 2.2      | 4302.774897(7)             |                          |
| 1085  | $E$               | 111        | 2.5      | 4305.67732(1)              |                          |
| 1086  | $E$               | 125        | 2.5      | 4305.67732(1)              |                          |
| 1087  | $E$               | 107        | 2.1      | 4306.057101(4)             |                          |
| 1088  | $E$               | 119        | 2.1      | 4306.057104(6)             |                          |
| 1089  | $E$               | 116        | 0.56     | 4307.48134(1)              |                          |
| 1090  | $E$               | 148        | 0.57     | 4307.48134(1)              |                          |
| 1091  | $A_1$             | 76         | 2.3      | 4310.60473(3)              |                          |
| 1092  | $A_2$             | 76         | 2.3      | 4310.60473(2)              |                          |
| 1093  | $E$               | 101        | 2.2      | 4310.715905(8)             |                          |
| 1094  | $E$               | 100        | 2.2      | 4310.715905(8)             |                          |
| 1095  | $E$               | 120        | 1.1      | 4311.569345(8)             |                          |
| 1096  | $E$               | 146        | 1.1      | 4311.569347(8)             |                          |
| 1097  | $E$               | 163        | 2.8      | 4312.867845(3)             |                          |
| 1098  | $E$               | 150        | 2.8      | 4312.867846(5)             |                          |
| 1099  | $A_1$             | 94         | 0.62     | 4313.01261(2)              |                          |
| 1100  | $A_2$             | 112        | 2.2      | 4313.023811(5)             |                          |
| 1101  | $A_1$             | 104        | 2.2      | 4313.02388(2)              |                          |
| 1102  | $E$               | 158        | 2.4      | 4313.445332(2)             |                          |
| 1103  | $E$               | 151        | 2.4      | 4313.445332(3)             |                          |
| 1104  | $A_2$             | 148        | 2.4      | 4313.459971(4)             |                          |
| 1105  | $A_1$             | 145        | 2.4      | 4313.460037(6)             |                          |
| 1106  | $E$               | 112        | 2.4      | 4314.890112(7)             |                          |

Continued on next page.

TABLE S4 – states on Sarka/Poirier CSC PES; continued from previous page

| State | $\Gamma_{C_{3v}}$ | $D_{\max}$ | $S_{vN}$ | $\tilde{E}/\text{cm}^{-1}$ | $\Delta\text{Ref. [30]}$ |
|-------|-------------------|------------|----------|----------------------------|--------------------------|
| 1107  | $E$               | 115        | 2.4      | 4314.890112(5)             |                          |
| 1108  | $E$               | 141        | 0.52     | 4314.942686(3)             |                          |
| 1109  | $E$               | 142        | 0.53     | 4314.942686(3)             |                          |
| 1110  | $A_1$             | 108        | 2.4      | 4314.96853(1)              |                          |
| 1111  | $A_2$             | 146        | 2.4      | 4314.968669(2)             |                          |
| 1112  | $E$               | 76         | 0.53     | 4316.382330(9)             |                          |
| 1113  | $E$               | 80         | 0.53     | 4316.382331(6)             |                          |
| 1114  | $A_2$             | 126        | 2.3      | 4317.056934(9)             |                          |
| 1115  | $A_1$             | 108        | 2.4      | 4317.11578(3)              |                          |
| 1116  | $E$               | 118        | 2.2      | 4317.18390(1)              |                          |
| 1117  | $E$               | 113        | 2.2      | 4317.183907(5)             |                          |
| 1118  | $E$               | 101        | 0.29     | 4318.537016(2)             |                          |
| 1119  | $E$               | 103        | 0.29     | 4318.537016(2)             |                          |
| 1120  | $E$               | 149        | 3.3      | 4318.940611(3)             |                          |
| 1121  | $E$               | 154        | 3.3      | 4318.940611(3)             |                          |
| 1122  | $A_2$             | 145        | 3.3      | 4319.039640(5)             |                          |
| 1123  | $A_1$             | 145        | 3.3      | 4319.040348(5)             |                          |
| 1124  | $E$               | 114        | 3.3      | 4319.25119(3)              |                          |
| 1125  | $E$               | 154        | 3.2      | 4319.25119(3)              |                          |
| 1126  | $E$               | 149        | 3.0      | 4319.350323(3)             |                          |
| 1127  | $E$               | 156        | 3.0      | 4319.350324(3)             |                          |
| 1128  | $E$               | 139        | 2.2      | 4320.473126(4)             |                          |
| 1129  | $E$               | 135        | 2.2      | 4320.473126(4)             |                          |
| 1130  | $A_1$             | 110        | 2.2      | 4320.77731(2)              |                          |
| 1131  | $A_2$             | 124        | 2.2      | 4320.783802(7)             |                          |
| 1132  | $A_2$             | 62         | 2.1      | 4340.380915(6)             |                          |
| 1133  | $E$               | 86         | 2.1      | 4341.260399(2)             |                          |
| 1134  | $E$               | 68         | 2.1      | 4341.260402(6)             |                          |
| 1135  | $A_1$             | 82         | 2.1      | 4341.681637(2)             |                          |
| 1136  | $E$               | 80         | 0.13     | 4348.766813(1)             |                          |
| 1137  | $E$               | 82         | 0.13     | 4348.766813(1)             |                          |
| 1138  | $E$               | 101        | 2.1      | 4349.663706(5)             |                          |
| 1139  | $E$               | 91         | 2.1      | 4349.66371(1)              |                          |
| 1140  | $A_1$             | 88         | 2.1      | 4349.67468(1)              |                          |
| 1141  | $A_2$             | 92         | 2.1      | 4349.67468(2)              |                          |
| 1142  | $E$               | 86         | 2.2      | 4353.95471(3)              |                          |
| 1143  | $E$               | 105        | 2.2      | 4353.95471(4)              |                          |
| 1144  | $A_1$             | 91         | 2.2      | 4353.99628(2)              |                          |
| 1145  | $A_2$             | 98         | 2.2      | 4353.996442(8)             |                          |
| 1146  | $E$               | 95         | 0.35     | 4355.473584(7)             |                          |
| 1147  | $E$               | 95         | 0.37     | 4355.473584(6)             |                          |
| 1148  | $A_2$             | 56         | 0.21     | 4358.40944(1)              |                          |
| 1149  | $A_1$             | 55         | 0.21     | 4358.40944(1)              |                          |
| 1150  | $E$               | 88         | 0.25     | 4365.299730(1)             |                          |
| 1151  | $E$               | 82         | 0.25     | 4365.299730(2)             |                          |
| 1152  | $E$               | 65         | 0.24     | 4368.606788(4)             |                          |
| 1153  | $E$               | 79         | 0.24     | 4368.606788(2)             |                          |
| 1154  | $A_1$             | 90         | 0.51     | 4369.433052(1)             |                          |
| 1155  | $E$               | 81         | 0.27     | 4369.434993(2)             |                          |
| 1156  | $E$               | 95         | 0.27     | 4369.434993(1)             |                          |
| 1157  | $A_1$             | 59         | 0.16     | 4369.511358(4)             |                          |
| 1158  | $A_1$             | 80         | 0.28     | 4370.813596(2)             |                          |
| 1159  | $E$               | 122        | 2.2      | 4371.162540(9)             |                          |
| 1160  | $E$               | 122        | 2.2      | 4371.162540(8)             |                          |
| 1161  | $A_1$             | 151        | 3.2      | 4371.975089(3)             |                          |
| 1162  | $A_2$             | 127        | 3.2      | 4371.975093(3)             |                          |
| 1163  | $E$               | 97         | 3.0      | 4372.107473(7)             |                          |
| 1164  | $E$               | 132        | 3.0      | 4372.10748(1)              |                          |
| 1165  | $E$               | 134        | 2.1      | 4372.468432(2)             |                          |

Continued on next page.

TABLE S4 – states on Sarka/Poirier CSC PES; continued from previous page

| State | $\Gamma_{C_{3v}}$ | $D_{\max}$ | $S_{vN}$ | $\tilde{E}/\text{cm}^{-1}$ | $\Delta\text{Ref. [30]}$ |
|-------|-------------------|------------|----------|----------------------------|--------------------------|
| 1166  | $E$               | 134        | 2.1      | 4372.468432(2)             |                          |
| 1167  | $E$               | 80         | 0.16     | 4374.9703777(8)            |                          |
| 1168  | $E$               | 70         | 0.16     | 4374.970378(1)             |                          |
| 1169  | $E$               | 105        | 2.1      | 4376.358092(2)             |                          |
| 1170  | $E$               | 93         | 2.1      | 4376.358092(4)             |                          |
| 1171  | $E$               | 86         | 0.1      | 4376.483494(2)             |                          |
| 1172  | $E$               | 98         | 0.1      | 4376.483494(2)             |                          |
| 1173  | $E$               | 96         | 2.1      | 4376.630998(4)             |                          |
| 1174  | $E$               | 81         | 2.1      | 4376.631003(5)             |                          |
| 1175  | $A_1$             | 101        | 2.3      | 4376.84283(1)              |                          |
| 1176  | $A_2$             | 132        | 2.3      | 4376.84287(2)              |                          |
| 1177  | $E$               | 98         | 0.58     | 4376.860802(1)             |                          |
| 1178  | $E$               | 95         | 0.58     | 4376.860803(1)             |                          |
| 1179  | $E$               | 143        | 3.3      | 4377.636074(6)             |                          |
| 1180  | $E$               | 143        | 3.3      | 4377.636074(7)             |                          |
| 1181  | $E$               | 144        | 3.1      | 4377.777567(5)             |                          |
| 1182  | $E$               | 143        | 3.1      | 4377.777567(5)             |                          |
| 1183  | $A_1$             | 98         | 2.2      | 4378.14553(1)              |                          |
| 1184  | $A_2$             | 94         | 2.2      | 4378.14553(1)              |                          |
| 1185  | $E$               | 134        | 2.3      | 4379.621988(4)             |                          |
| 1186  | $E$               | 124        | 2.3      | 4379.621988(7)             |                          |
| 1187  | $A_1$             | 100        | 3.2      | 4380.61491(2)              |                          |
| 1188  | $A_2$             | 104        | 3.2      | 4380.61871(1)              |                          |
| 1189  | $E$               | 97         | 2.1      | 4380.67356(1)              |                          |
| 1190  | $E$               | 125        | 2.1      | 4380.673564(7)             |                          |
| 1191  | $E$               | 96         | 2.2      | 4380.678247(5)             |                          |
| 1192  | $E$               | 94         | 2.2      | 4380.678248(8)             |                          |
| 1193  | $E$               | 129        | 2.8      | 4380.684527(5)             |                          |
| 1194  | $E$               | 130        | 2.7      | 4380.684528(5)             |                          |
| 1195  | $E$               | 121        | 2.2      | 4381.001537(4)             |                          |
| 1196  | $E$               | 120        | 2.2      | 4381.001537(5)             |                          |
| 1197  | $A_2$             | 103        | 0.76     | 4382.365778(2)             |                          |
| 1198  | $A_1$             | 81         | 0.76     | 4382.365811(2)             |                          |
| 1199  | $A_2$             | 113        | 2.3      | 4383.366847(3)             |                          |
| 1200  | $E$               | 93         | 2.2      | 4383.578107(8)             |                          |
| 1201  | $E$               | 98         | 2.2      | 4383.578108(8)             |                          |
| 1202  | $A_1$             | 83         | 2.3      | 4383.77829(1)              |                          |
| 1203  | $E$               | 91         | 0.84     | 4385.119325(2)             |                          |
| 1204  | $E$               | 87         | 0.84     | 4385.119325(1)             |                          |
| 1205  | $A_1$             | 136        | 2.7      | 4385.615336(2)             |                          |
| 1206  | $E$               | 132        | 2.6      | 4385.738960(3)             |                          |
| 1207  | $E$               | 113        | 2.6      | 4385.738960(7)             |                          |
| 1208  | $A_2$             | 125        | 2.6      | 4385.814164(3)             |                          |
| 1209  | $A_2$             | 80         | 2.2      | 4387.26522(1)              |                          |
| 1210  | $A_1$             | 84         | 2.2      | 4387.26523(1)              |                          |
| 1211  | $E$               | 93         | 2.2      | 4387.48977(1)              |                          |
| 1212  | $E$               | 126        | 2.2      | 4387.48977(1)              |                          |
| 1213  | $E$               | 125        | 3.2      | 4392.832225(3)             |                          |
| 1214  | $E$               | 129        | 3.2      | 4392.832225(3)             |                          |
| 1215  | $A_2$             | 125        | 3.1      | 4392.840817(3)             |                          |
| 1216  | $A_1$             | 128        | 3.2      | 4392.908864(3)             |                          |
| 1217  | $E$               | 118        | 2.2      | 4393.193158(2)             |                          |
| 1218  | $E$               | 105        | 2.2      | 4393.193160(7)             |                          |
| 1219  | $E$               | 103        | 2.3      | 4393.212668(7)             |                          |
| 1220  | $E$               | 99         | 2.3      | 4393.21267(1)              |                          |
| 1221  | $E$               | 100        | 2.3      | 4395.45200(1)              |                          |
| 1222  | $E$               | 103        | 2.3      | 4395.45200(1)              |                          |
| 1223  | $A_1$             | 84         | 2.2      | 4395.632557(8)             |                          |
| 1224  | $A_2$             | 89         | 2.2      | 4395.63256(1)              |                          |

Continued on next page.

TABLE S4 – states on Sarka/Poirier CSC PES; continued from previous page

| State | $\Gamma_{C_{3v}}$ | $D_{\max}$ | $S_{vN}$ | $\tilde{E}/\text{cm}^{-1}$ | $\Delta\text{Ref. [30]}$ |
|-------|-------------------|------------|----------|----------------------------|--------------------------|
| 1225  | $E$               | 54         | 0.59     | 4400.461830(6)             |                          |
| 1226  | $E$               | 53         | 0.59     | 4400.461831(7)             |                          |
| 1227  | $E$               | 101        | 2.3      | 4400.90377(1)              |                          |
| 1228  | $E$               | 105        | 2.3      | 4400.90377(1)              |                          |
| 1229  | $E$               | 133        | 2.3      | 4401.058441(2)             |                          |
| 1230  | $E$               | 137        | 2.3      | 4401.058441(1)             |                          |
| 1231  | $A_1$             | 116        | 1.1      | 4401.559494(2)             |                          |
| 1232  | $A_1$             | 66         | 0.59     | 4401.936337(2)             |                          |
| 1233  | $A_1$             | 91         | 0.94     | 4402.038095(3)             |                          |
| 1234  | $A_1$             | 102        | 2.3      | 4403.341096(6)             |                          |
| 1235  | $E$               | 91         | 2.3      | 4403.776516(8)             |                          |
| 1236  | $E$               | 100        | 2.3      | 4403.776517(8)             |                          |
| 1237  | $A_2$             | 88         | 2.3      | 4404.062846(8)             |                          |
| 1238  | $E$               | 122        | 1.8      | 4406.964350(2)             |                          |
| 1239  | $E$               | 122        | 1.8      | 4406.964350(2)             |                          |
| 1240  | $A_1$             | 134        | 2.5      | 4408.450784(2)             |                          |
| 1241  | $A_2$             | 133        | 2.1      | 4408.628466(2)             |                          |
| 1242  | $E$               | 135        | 3.3      | 4408.670813(2)             |                          |
| 1243  | $E$               | 134        | 3.3      | 4408.670813(3)             |                          |
| 1244  | $A_1$             | 58         | 0.24     | 4414.841823(1)             |                          |
| 1245  | $A_1$             | 110        | 2.6      | 4415.768987(2)             |                          |
| 1246  | $E$               | 100        | 2.5      | 4415.853899(3)             |                          |
| 1247  | $E$               | 80         | 2.5      | 4415.85390(1)              |                          |
| 1248  | $A_2$             | 77         | 2.5      | 4415.89208(2)              |                          |
| 1249  | $E$               | 85         | 2.2      | 4418.463914(3)             |                          |
| 1250  | $E$               | 86         | 2.2      | 4418.463914(3)             |                          |
| 1251  | $E$               | 98         | 2.2      | 4418.548576(4)             |                          |
| 1252  | $E$               | 118        | 2.2      | 4418.548577(3)             |                          |
| 1253  | $E$               | 121        | 0.56     | 4419.454322(2)             |                          |
| 1254  | $E$               | 103        | 0.55     | 4419.454322(8)             |                          |
| 1255  | $E$               | 98         | 0.49     | 4419.634058(7)             |                          |
| 1256  | $E$               | 95         | 0.52     | 4419.634059(9)             |                          |
| 1257  | $A_1$             | 93         | 2.3      | 4421.264850(4)             |                          |
| 1258  | $E$               | 119        | 3.0      | 4421.429141(1)             |                          |
| 1259  | $E$               | 118        | 3.0      | 4421.429141(1)             |                          |
| 1260  | $A_2$             | 71         | 2.2      | 4421.538421(2)             |                          |
| 1261  | $E$               | 88         | 1.5      | 4421.591755(4)             |                          |
| 1262  | $E$               | 81         | 1.5      | 4421.591755(6)             |                          |
| 1263  | $A_1$             | 78         | 0.68     | 4423.057079(2)             |                          |
| 1264  | $E$               | 91         | 0.45     | 4432.378029(5)             |                          |
| 1265  | $E$               | 91         | 0.45     | 4432.378029(5)             |                          |
| 1266  | $E$               | 66         | 1.1      | 4432.528163(1)             |                          |
| 1267  | $E$               | 53         | 1.1      | 4432.528164(3)             |                          |
| 1268  | $A_2^*$           | 78         | 2.0      | 4436.285833(5)             |                          |
| 1269  | $A_1^*$           | 77         | 2.0      | 4436.285833(5)             |                          |
| 1270  | $E$               | 95         | 2.0      | 4436.324354(4)             |                          |
| 1271  | $E$               | 91         | 2.0      | 4436.324355(3)             |                          |
| 1272  | $E$               | 110        | 0.68     | 4436.654118(1)             |                          |
| 1273  | $E$               | 94         | 0.67     | 4436.65412(1)              |                          |
| 1274  | $A_1$             | 119        | 0.62     | 4438.092090(2)             |                          |
| 1275  | $A_2$             | 125        | 2.0      | 4439.373653(2)             |                          |
| 1276  | $A_1$             | 89         | 2.0      | 4439.373657(8)             |                          |
| 1277  | $E$               | 109        | 2.2      | 4439.443348(9)             |                          |
| 1278  | $E$               | 129        | 2.2      | 4439.443349(8)             |                          |
| 1279  | $E$               | 86         | 2.1      | 4443.70274(1)              |                          |
| 1280  | $E$               | 102        | 2.1      | 4443.70274(1)              |                          |
| 1281  | $A_2$             | 92         | 2.1      | 4443.716254(5)             |                          |
| 1282  | $A_1$             | 125        | 2.2      | 4443.758487(2)             |                          |
| 1283  | $E$               | 90         | 0.12     | 4445.157529(2)             |                          |

Continued on next page.

TABLE S4 – states on Sarka/Poirier CSC PES; continued from previous page

| State | $\Gamma_{C_{3v}}$ | $D_{\max}$ | $S_{vN}$ | $\tilde{E}/\text{cm}^{-1}$ | $\Delta\text{Ref. [30]}$ |
|-------|-------------------|------------|----------|----------------------------|--------------------------|
| 1284  | $E$               | 92         | 0.12     | 4445.157530(3)             |                          |
| 1285  | $E$               | 101        | 2.1      | 4445.934835(4)             |                          |
| 1286  | $E$               | 99         | 2.1      | 4445.934835(5)             |                          |
| 1287  | $E$               | 86         | 2.1      | 4445.941499(6)             |                          |
| 1288  | $E$               | 88         | 2.1      | 4445.941499(6)             |                          |
| 1289  | $E$               | 55         | 1.2      | 4447.868042(3)             |                          |
| 1290  | $E$               | 58         | 1.2      | 4447.868044(4)             |                          |
| 1291  | $E$               | 125        | 2.5      | 4450.537807(5)             |                          |
| 1292  | $E$               | 107        | 2.5      | 4450.53781(1)              |                          |
| 1293  | $E$               | 93         | 2.4      | 4450.65141(1)              |                          |
| 1294  | $E$               | 104        | 2.4      | 4450.65141(2)              |                          |
| 1295  | $A_2^*$           | 87         | 2.2      | 4452.797839(9)             |                          |
| 1296  | $A_1^*$           | 87         | 2.2      | 4452.797841(5)             |                          |
| 1297  | $E$               | 101        | 2.2      | 4452.837366(9)             |                          |
| 1298  | $E$               | 99         | 2.2      | 4452.837366(8)             |                          |
| 1299  | $A_1$             | 115        | 2.6      | 4453.321934(9)             |                          |
| 1300  | $E$               | 98         | 2.5      | 4453.52965(1)              |                          |
| 1301  | $E$               | 103        | 2.5      | 4453.52965(1)              |                          |
| 1302  | $A_2$             | 90         | 2.4      | 4453.652118(8)             |                          |
| 1303  | $E$               | 85         | 0.67     | 4454.421473(2)             |                          |
| 1304  | $E$               | 72         | 0.67     | 4454.421475(3)             |                          |
| 1305  | $E$               | 97         | 2.1      | 4455.144572(1)             |                          |
| 1306  | $E$               | 89         | 2.1      | 4455.144572(1)             |                          |
| 1307  | $A_1$             | 88         | 2.1      | 4455.148000(2)             |                          |
| 1308  | $A_2$             | 79         | 2.0      | 4455.154223(3)             |                          |
| 1309  | $E$               | 96         | 2.2      | 4456.835507(8)             |                          |
| 1310  | $E$               | 124        | 2.2      | 4456.835508(8)             |                          |
| 1311  | $A_1$             | 84         | 2.2      | 4456.997502(8)             |                          |
| 1312  | $A_2$             | 83         | 2.2      | 4456.998077(6)             |                          |
| 1313  | $A_1$             | 63         | 0.023    | 4458.068169(1)             |                          |
| 1314  | $A_2$             | 77         | 0.023    | 4458.068169(1)             |                          |
| 1315  | $E$               | 84         | 0.68     | 4458.469591(5)             |                          |
| 1316  | $E$               | 94         | 0.67     | 4458.469592(6)             |                          |
| 1317  | $E$               | 119        | 2.3      | 4460.120428(1)             |                          |
| 1318  | $E$               | 99         | 2.3      | 4460.120428(4)             |                          |
| 1319  | $A_1$             | 70         | 2.2      | 4460.17094(2)              |                          |
| 1320  | $A_2$             | 66         | 2.2      | 4460.17099(2)              |                          |
| 1321  | $E$               | 72         | 0.35     | 4461.605961(7)             |                          |
| 1322  | $E$               | 87         | 0.36     | 4461.605963(7)             |                          |
| 1323  | $E$               | 115        | 0.36     | 4463.153614(8)             |                          |
| 1324  | $E$               | 136        | 0.36     | 4463.153615(8)             |                          |
| 1325  | $E$               | 77         | 0.46     | 4465.671613(2)             |                          |
| 1326  | $E$               | 84         | 0.46     | 4465.671614(3)             |                          |
| 1327  | $E$               | 115        | 0.85     | 4467.397875(6)             |                          |
| 1328  | $E$               | 143        | 0.85     | 4467.397882(9)             |                          |
| 1329  | $A_1$             | 78         | 0.036    | 4468.335577(1)             |                          |
| 1330  | $A_2$             | 79         | 0.035    | 4468.342207(1)             |                          |
| 1331  | $E$               | 104        | 2.6      | 4468.52051(5)              |                          |
| 1332  | $E$               | 132        | 2.6      | 4468.52051(5)              |                          |
| 1333  | $A_2$             | 85         | 2.1      | 4468.70046(3)              |                          |
| 1334  | $A_1$             | 90         | 2.1      | 4468.70046(3)              |                          |
| 1335  | $A_1$             | 132        | 0.54     | 4468.840004(5)             |                          |
| 1336  | $E$               | 88         | 0.49     | 4469.982706(3)             |                          |
| 1337  | $E$               | 95         | 0.49     | 4469.982706(3)             |                          |
| 1338  | $A_1$             | 91         | 0.5      | 4471.419852(2)             |                          |
| 1339  | $E$               | 72         | 0.17     | 4472.566184(1)             |                          |
| 1340  | $E$               | 68         | 0.17     | 4472.566184(1)             |                          |
| 1341  | $A_2$             | 123        | 2.3      | 4472.82781(1)              |                          |
| 1342  | $A_1$             | 123        | 2.4      | 4472.85575(1)              |                          |

Continued on next page.



TABLE S4 – states on Sarka/Poirier CSC PES; continued from previous page

| State | $\Gamma_{C_{3v}}$ | $D_{\max}$ | $S_{vN}$ | $\tilde{E}/\text{cm}^{-1}$ | $\Delta\text{Ref. [30]}$ |
|-------|-------------------|------------|----------|----------------------------|--------------------------|
| 1343  | $E$               | 132        | 2.3      | 4472.939613(5)             |                          |
| 1344  | $E$               | 118        | 2.3      | 4472.939617(6)             |                          |
| 1345  | $A_1$             | 52         | 0.15     | 4473.872230(3)             |                          |
| 1346  | $A_2$             | 57         | 0.15     | 4473.872230(2)             |                          |
| 1347  | $E$               | 98         | 0.35     | 4474.319636(8)             |                          |
| 1348  | $E$               | 107        | 0.35     | 4474.31964(1)              |                          |
| 1349  | $E$               | 75         | 0.2      | 4480.912769(1)             |                          |
| 1350  | $E$               | 72         | 0.2      | 4480.912769(1)             |                          |
| 1351  | $E$               | 72         | 0.27     | 4484.436227(2)             |                          |
| 1352  | $E$               | 85         | 0.27     | 4484.436227(2)             |                          |
| 1353  | $E$               | 76         | 0.23     | 4485.138269(1)             |                          |
| 1354  | $E$               | 79         | 0.23     | 4485.138269(1)             |                          |
| 1355  | $A_1$             | 77         | 0.24     | 4486.546870(1)             |                          |
| 1356  | $E$               | 66         | 2.1      | 4487.03510(1)              |                          |
| 1357  | $E$               | 65         | 2.1      | 4487.03510(2)              |                          |
| 1358  | $A_2$             | 60         | 2.1      | 4487.03933(4)              |                          |
| 1359  | $A_1$             | 65         | 2.1      | 4487.03941(3)              |                          |
| 1360  | $E$               | 74         | 0.25     | 4488.530214(3)             |                          |
| 1361  | $E$               | 74         | 0.23     | 4488.530215(3)             |                          |
| 1362  | $E$               | 80         | 0.72     | 4489.246981(1)             |                          |
| 1363  | $E$               | 84         | 0.72     | 4489.246982(1)             |                          |
| 1364  | $E$               | 86         | 0.32     | 4490.951969(6)             |                          |
| 1365  | $E$               | 103        | 0.32     | 4490.951971(7)             |                          |
| 1366  | $A_2^*$           | 69         | 0.33     | 4493.673484(7)             |                          |
| 1367  | $A_1^*$           | 82         | 0.33     | 4493.673485(3)             |                          |
| 1368  | $E$               | 100        | 2.1      | 4496.491465(3)             |                          |
| 1369  | $E$               | 98         | 2.1      | 4496.491466(2)             |                          |
| 1370  | $A_1$             | 69         | 2.1      | 4496.79753(1)              |                          |
| 1371  | $A_2$             | 65         | 2.0      | 4496.80326(1)              |                          |
| 1372  | $E$               | 75         | 0.38     | 4500.274206(4)             |                          |
| 1373  | $E$               | 80         | 0.38     | 4500.274206(3)             |                          |
| 1374  | $E$               | 77         | 0.4      | 4504.235712(5)             |                          |
| 1375  | $E$               | 73         | 0.4      | 4504.235712(4)             |                          |
| 1376  | $A_1$             | 70         | 0.41     | 4505.556393(4)             |                          |
| 1377  | $A_2$             | 89         | 0.35     | 4506.022002(1)             |                          |
| 1378  | $A_1$             | 91         | 0.35     | 4506.022003(1)             |                          |
| 1379  | $E$               | 82         | 0.3      | 4507.886973(1)             |                          |
| 1380  | $E$               | 81         | 0.3      | 4507.886973(1)             |                          |
| 1381  | $E$               | 86         | 0.5      | 4513.033854(2)             |                          |
| 1382  | $E$               | 86         | 0.5      | 4513.033854(2)             |                          |
| 1383  | $A_1$             | 51         | 0.63     | 4513.48391(2)              |                          |
| 1384  | $A_2$             | 54         | 0.63     | 4513.48392(1)              |                          |
| 1385  | $E$               | 75         | 0.76     | 4516.2832190(8)            |                          |
| 1386  | $E$               | 83         | 0.76     | 4516.283220(2)             |                          |
| 1387  | $E$               | 86         | 0.57     | 4517.242191(2)             |                          |
| 1388  | $E$               | 76         | 0.57     | 4517.242191(5)             |                          |
| 1389  | $A_1$             | 85         | 0.59     | 4518.645166(2)             |                          |
| 1390  | $E$               | 144        | 2.3      | 4521.374449(2)             |                          |
| 1391  | $E$               | 111        | 2.3      | 4521.374451(9)             |                          |
| 1392  | $A_1$             | 96         | 2.3      | 4521.37901(3)              |                          |
| 1393  | $A_2$             | 84         | 2.3      | 4521.37903(4)              |                          |
| 1394  | $E$               | 93         | 0.38     | 4522.868004(7)             |                          |
| 1395  | $E$               | 90         | 0.4      | 4522.868006(5)             |                          |
| 1396  | $E$               | 55         | 0.085    | 4524.528360(5)             |                          |
| 1397  | $E$               | 55         | 0.085    | 4524.528362(3)             |                          |
| 1398  | $A_1$             | 50         | 0.13     | 4526.572353(1)             |                          |
| 1399  | $A_1$             | 81         | 2.2      | 4529.26402(1)              |                          |
| 1400  | $A_2$             | 83         | 2.2      | 4529.26402(1)              |                          |
| 1401  | $E$               | 104        | 2.2      | 4529.472200(7)             |                          |

Continued on next page.

TABLE S4 – states on Sarka/Poirier CSC PES; continued from previous page

| State | $\Gamma_{C_{3v}}$ | $D_{\max}$ | $S_{vN}$ | $\tilde{E}/\text{cm}^{-1}$ | $\Delta\text{Ref. [30]}$ |
|-------|-------------------|------------|----------|----------------------------|--------------------------|
| 1402  | $E$               | 101        | 2.2      | 4529.472200(9)             |                          |
| 1403  | $A_2$             | 92         | 2.1      | 4534.726538(3)             |                          |
| 1404  | $E$               | 77         | 2.1      | 4534.826116(1)             |                          |
| 1405  | $E$               | 106        | 2.1      | 4534.826119(4)             |                          |
| 1406  | $A_1$             | 79         | 2.1      | 4534.935648(2)             |                          |
| 1407  | $E$               | 117        | 2.4      | 4537.586986(7)             |                          |
| 1408  | $E$               | 137        | 2.4      | 4537.58699(1)              |                          |
| 1409  | $A_2$             | 87         | 2.4      | 4537.74899(2)              |                          |
| 1410  | $A_1$             | 87         | 2.4      | 4537.74899(3)              |                          |
| 1411  | $E$               | 123        | 1.8      | 4538.063393(2)             |                          |
| 1412  | $E$               | 125        | 1.8      | 4538.063393(2)             |                          |
| 1413  | $A_1$             | 109        | 2.2      | 4538.317261(6)             |                          |
| 1414  | $A_2$             | 115        | 2.2      | 4538.317269(8)             |                          |
| 1415  | $E$               | 146        | 3.2      | 4539.150103(6)             |                          |
| 1416  | $E$               | 147        | 3.2      | 4539.150104(7)             |                          |
| 1417  | $E$               | 139        | 3.1      | 4539.236483(4)             |                          |
| 1418  | $E$               | 116        | 3.1      | 4539.236488(9)             |                          |
| 1419  | $A_1$             | 101        | 2.2      | 4539.62245(1)              |                          |
| 1420  | $A_2$             | 101        | 2.2      | 4539.62245(1)              |                          |
| 1421  | $E$               | 123        | 1.6      | 4540.449638(2)             |                          |
| 1422  | $E$               | 124        | 1.6      | 4540.449638(2)             |                          |
| 1423  | $E$               | 133        | 2.3      | 4541.182809(3)             |                          |
| 1424  | $E$               | 111        | 2.3      | 4541.18281(1)              |                          |
| 1425  | $A_1$             | 108        | 3.2      | 4542.12167(1)              |                          |
| 1426  | $A_2$             | 107        | 3.2      | 4542.12373(1)              |                          |
| 1427  | $E$               | 157        | 3.0      | 4542.145840(3)             |                          |
| 1428  | $E$               | 138        | 2.9      | 4542.145841(6)             |                          |
| 1429  | $E$               | 110        | 2.2      | 4542.524023(3)             |                          |
| 1430  | $E$               | 118        | 2.2      | 4542.524024(3)             |                          |
| 1431  | $E$               | 159        | 2.5      | 4543.136473(2)             |                          |
| 1432  | $E$               | 111        | 2.5      | 4543.13647(1)              |                          |
| 1433  | $E$               | 110        | 2.5      | 4543.26331(1)              |                          |
| 1434  | $E$               | 93         | 2.5      | 4543.26331(2)              |                          |
| 1435  | $A_1$             | 101        | 2.6      | 4545.67354(1)              |                          |
| 1436  | $A_1$             | 133        | 2.5      | 4545.702088(4)             |                          |
| 1437  | $A_2$             | 137        | 2.4      | 4545.731997(2)             |                          |
| 1438  | $E$               | 142        | 2.4      | 4545.823654(2)             |                          |
| 1439  | $E$               | 125        | 2.4      | 4545.823655(5)             |                          |
| 1440  | $E$               | 133        | 2.5      | 4546.018814(2)             |                          |
| 1441  | $E$               | 139        | 2.5      | 4546.018814(2)             |                          |
| 1442  | $A_2$             | 84         | 2.5      | 4546.250313(9)             |                          |
| 1443  | $A_1$             | 125        | 0.66     | 4549.414091(2)             |                          |
| 1444  | $A_2$             | 116        | 0.59     | 4549.576138(2)             |                          |
| 1445  | $A_2$             | 84         | 2.2      | 4562.47025(3)              |                          |
| 1446  | $A_1$             | 89         | 2.2      | 4562.47403(3)              |                          |
| 1447  | $E$               | 93         | 2.1      | 4562.55173(1)              |                          |
| 1448  | $E$               | 101        | 2.1      | 4562.55173(1)              |                          |
| 1449  | $E$               | 100        | 2.2      | 4566.04294(1)              |                          |
| 1450  | $E$               | 103        | 2.2      | 4566.04294(1)              |                          |
| 1451  | $A_1$             | 138        | 2.2      | 4566.135646(1)             |                          |
| 1452  | $A_2$             | 118        | 2.1      | 4566.135705(5)             |                          |
| 1453  | $E$               | 96         | 0.24     | 4567.575545(7)             |                          |
| 1454  | $E$               | 90         | 0.23     | 4567.575546(6)             |                          |
| 1455  | $A_1$             | 57         | 1.7      | 4577.2670329(6)            |                          |
| 1456  | $E$               | 67         | 0.12     | 4584.824214(2)             |                          |
| 1457  | $E$               | 63         | 0.12     | 4584.824215(1)             |                          |
| 1458  | $A_1$             | 89         | 0.55     | 4590.35975(3)              |                          |
| 1459  | $A_2$             | 93         | 0.55     | 4590.35977(2)              |                          |
| 1460  | $A_1$             | 84         | 4.9      | 4591.076484(4)             |                          |

Continued on next page.

TABLE S4 – states on Sarka/Poirier CSC PES; continued from previous page

| State | $\Gamma_{C_{3v}}$ | $D_{\max}$ | $S_{vN}$ | $\tilde{E}/\text{cm}^{-1}$ | $\Delta\text{Ref. [30]}$ |
|-------|-------------------|------------|----------|----------------------------|--------------------------|
| 1461  | $A_1$             | 86         | 5.6      | 4591.362114(6)             |                          |
| 1462  | $E$               | 85         | 2.4      | 4591.388367(1)             |                          |
| 1463  | $E$               | 74         | 2.4      | 4591.388368(2)             |                          |
| 1464  | $A_2$             | 76         | 2.4      | 4591.429165(1)             |                          |
| 1465  | $E$               | 153        | 0.64     | 4593.256179(2)             |                          |
| 1466  | $E$               | 151        | 0.64     | 4593.256179(3)             |                          |
| 1467  | $E$               | 105        | 2.1      | 4593.480761(2)             |                          |
| 1468  | $E$               | 108        | 2.1      | 4593.480761(2)             |                          |
| 1469  | $E$               | 95         | 2.1      | 4593.505406(4)             |                          |
| 1470  | $E$               | 104        | 2.1      | 4593.505406(2)             |                          |
| 1471  | $E$               | 128        | 2.6      | 4595.760584(3)             |                          |
| 1472  | $E$               | 160        | 2.6      | 4595.76059(1)              |                          |
| 1473  | $E$               | 137        | 2.5      | 4595.931812(2)             |                          |
| 1474  | $E$               | 124        | 2.5      | 4595.931817(7)             |                          |
| 1475  | $E$               | 128        | 2.4      | 4598.737333(7)             |                          |
| 1476  | $E$               | 131        | 2.4      | 4598.737335(3)             |                          |
| 1477  | $A_1$             | 97         | 2.5      | 4598.79166(5)              |                          |
| 1478  | $A_2$             | 96         | 2.4      | 4598.80048(7)              |                          |
| 1479  | $E$               | 91         | 2.1      | 4599.013366(2)             |                          |
| 1480  | $E$               | 92         | 2.1      | 4599.013366(1)             |                          |
| 1481  | $E$               | 92         | 3.0      | 4599.504015(4)             |                          |
| 1482  | $E$               | 70         | 3.0      | 4599.50402(1)              |                          |
| 1483  | $A_1$             | 68         | 3.0      | 4599.51908(1)              |                          |
| 1484  | $A_2$             | 85         | 3.0      | 4599.523981(3)             |                          |
| 1485  | $E$               | 95         | 2.1      | 4600.0635358(8)            |                          |
| 1486  | $E$               | 94         | 2.1      | 4600.063536(1)             |                          |
| 1487  | $A_2$             | 90         | 2.3      | 4600.488781(8)             |                          |
| 1488  | $A_1$             | 82         | 2.3      | 4600.48878(2)              |                          |
| 1489  | $E$               | 85         | 2.3      | 4600.49941(1)              |                          |
| 1490  | $E$               | 80         | 2.3      | 4600.49941(2)              |                          |
| 1491  | $E$               | 78         | 0.18     | 4601.469353(1)             |                          |
| 1492  | $E$               | 78         | 0.18     | 4601.469353(1)             |                          |
| 1493  | $A_1$             | 100        | 2.4      | 4603.45590(2)              |                          |
| 1494  | $A_2$             | 99         | 2.4      | 4603.45591(2)              |                          |
| 1495  | $E$               | 144        | 2.5      | 4603.604545(2)             |                          |
| 1496  | $E$               | 130        | 2.5      | 4603.604548(5)             |                          |
| 1497  | $E$               | 102        | 0.48     | 4604.025494(2)             |                          |
| 1498  | $E$               | 103        | 0.48     | 4604.025494(2)             |                          |
| 1499  | $E$               | 108        | 2.4      | 4604.628874(7)             |                          |
| 1500  | $E$               | 140        | 2.4      | 4604.628875(6)             |                          |
| 1501  | $A_1$             | 106        | 2.4      | 4604.72387(1)              |                          |
| 1502  | $A_2$             | 104        | 2.4      | 4604.724414(9)             |                          |
| 1503  | $A_1$             | 102        | 0.56     | 4605.482079(2)             |                          |
| 1504  | $E$               | 53         | 0.17     | 4606.107927(1)             |                          |
| 1505  | $E$               | 55         | 0.17     | 4606.107927(1)             |                          |
| 1506  | $E$               | 111        | 0.73     | 4606.189529(3)             |                          |
| 1507  | $E$               | 106        | 0.75     | 4606.189529(4)             |                          |
| 1508  | $E$               | 160        | 2.4      | 4607.710412(5)             |                          |
| 1509  | $E$               | 146        | 2.4      | 4607.710415(4)             |                          |
| 1510  | $A_1$             | 105        | 2.4      | 4607.86061(5)              |                          |
| 1511  | $A_2$             | 121        | 2.4      | 4607.86160(1)              |                          |
| 1512  | $E$               | 126        | 0.64     | 4609.304298(7)             |                          |
| 1513  | $E$               | 138        | 0.62     | 4609.304298(7)             |                          |
| 1514  | $E$               | 106        | 2.1      | 4611.021007(5)             |                          |
| 1515  | $E$               | 113        | 2.1      | 4611.021007(5)             |                          |
| 1516  | $A_2$             | 89         | 2.1      | 4611.040666(9)             |                          |
| 1517  | $A_1$             | 133        | 2.1      | 4611.055337(2)             |                          |
| 1518  | $E$               | 98         | 0.12     | 4612.501917(2)             |                          |
| 1519  | $E$               | 100        | 0.12     | 4612.501918(2)             |                          |

Continued on next page.

TABLE S4 – states on Sarka/Poirier CSC PES; continued from previous page

| State | $\Gamma_{C_{3v}}$ | $D_{\max}$ | $S_{vN}$ | $\tilde{E}/\text{cm}^{-1}$ | $\Delta\text{Ref. [30]}$ |
|-------|-------------------|------------|----------|----------------------------|--------------------------|
| 1520  | $E$               | 84         | 0.5      | 4613.510449(1)             |                          |
| 1521  | $E$               | 84         | 0.5      | 4613.510450(2)             |                          |
| 1522  | $E$               | 144        | 2.0      | 4614.333874(2)             |                          |
| 1523  | $E$               | 129        | 2.0      | 4614.333876(5)             |                          |
| 1524  | $E$               | 116        | 1.8      | 4614.68826(1)              |                          |
| 1525  | $E$               | 140        | 1.8      | 4614.68826(1)              |                          |
| 1526  | $A_1$             | 108        | 2.8      | 4614.74556(1)              |                          |
| 1527  | $E$               | 102        | 2.7      | 4614.86627(2)              |                          |
| 1528  | $E$               | 102        | 2.7      | 4614.86627(2)              |                          |
| 1529  | $A_2$             | 90         | 2.6      | 4614.925963(5)             |                          |
| 1530  | $E$               | 155        | 1.4      | 4618.695123(4)             |                          |
| 1531  | $E$               | 151        | 1.4      | 4618.695123(5)             |                          |
| 1532  | $E$               | 129        | 1.4      | 4618.923406(4)             |                          |
| 1533  | $E$               | 131        | 1.3      | 4618.923407(4)             |                          |
| 1534  | $E$               | 76         | 0.13     | 4618.971732(3)             |                          |
| 1535  | $E$               | 88         | 0.13     | 4618.971732(3)             |                          |
| 1536  | $A_1$             | 123        | 0.25     | 4620.159433(6)             |                          |
| 1537  | $A_2$             | 109        | 0.24     | 4620.324798(3)             |                          |
| 1538  | $E$               | 110        | 0.39     | 4622.684869(5)             |                          |
| 1539  | $E$               | 115        | 0.39     | 4622.684869(5)             |                          |
| 1540  | $A_1$             | 58         | 0.69     | 4622.88150(2)              |                          |
| 1541  | $A_2$             | 57         | 0.69     | 4622.88150(3)              |                          |
| 1542  | $A_1$             | 111        | 0.42     | 4624.128434(4)             |                          |
| 1543  | $A_1$             | 89         | 0.17     | 4624.666086(1)             |                          |
| 1544  | $A_2$             | 77         | 0.17     | 4624.666098(4)             |                          |
| 1545  | $E$               | 83         | 0.18     | 4627.513853(4)             |                          |
| 1546  | $E$               | 60         | 0.18     | 4627.513855(4)             |                          |
| 1547  | $A_2$             | 109        | 2.1      | 4627.568622(2)             |                          |
| 1548  | $A_2$             | 87         | 2.3      | 4628.07028(2)              |                          |
| 1549  | $A_1$             | 94         | 2.3      | 4628.07796(3)              |                          |
| 1550  | $E$               | 99         | 2.1      | 4628.159763(8)             |                          |
| 1551  | $E$               | 122        | 2.1      | 4628.15977(1)              |                          |
| 1552  | $E$               | 109        | 2.1      | 4628.974050(1)             |                          |
| 1553  | $E$               | 109        | 2.1      | 4628.974050(1)             |                          |
| 1554  | $E$               | 97         | 0.28     | 4629.572926(9)             |                          |
| 1555  | $E$               | 100        | 0.28     | 4629.57293(1)              |                          |
| 1556  | $E$               | 86         | 0.82     | 4629.578176(2)             |                          |
| 1557  | $E$               | 81         | 0.82     | 4629.578177(3)             |                          |
| 1558  | $A_1$             | 109        | 2.1      | 4630.143314(2)             |                          |
| 1559  | $E$               | 77         | 0.89     | 4633.597420(1)             |                          |
| 1560  | $E$               | 80         | 0.89     | 4633.597421(3)             |                          |
| 1561  | $A_1$             | 78         | 0.91     | 4634.937374(2)             |                          |
| 1562  | $E$               | 69         | 0.46     | 4636.486304(3)             |                          |
| 1563  | $E$               | 57         | 0.46     | 4636.486304(3)             |                          |
| 1564  | $E$               | 67         | 0.48     | 4636.943374(2)             |                          |
| 1565  | $E$               | 86         | 0.48     | 4636.943378(4)             |                          |
| 1566  | $A_2$             | 99         | 2.1      | 4637.578371(1)             |                          |
| 1567  | $E$               | 119        | 2.1      | 4637.677936(2)             |                          |
| 1568  | $E$               | 103        | 2.1      | 4637.677937(2)             |                          |
| 1569  | $A_1$             | 102        | 2.1      | 4637.786440(1)             |                          |
| 1570  | $A_1$             | 78         | 0.51     | 4638.409457(2)             |                          |
| 1571  | $E$               | 98         | 1.9      | 4639.766576(3)             |                          |
| 1572  | $E$               | 93         | 2.0      | 4639.766577(3)             |                          |
| 1573  | $E$               | 105        | 1.9      | 4640.379048(2)             |                          |
| 1574  | $E$               | 105        | 1.9      | 4640.379048(1)             |                          |
| 1575  | $E$               | 69         | 0.55     | 4640.790912(2)             |                          |
| 1576  | $E$               | 80         | 0.55     | 4640.790913(1)             |                          |
| 1577  | $A_1$             | 76         | 0.57     | 4642.226007(1)             |                          |
| 1578  | $A_1$             | 48         | 0.33     | 4643.296707(5)             |                          |

Continued on next page.

TABLE S4 – states on Sarka/Poirier CSC PES; continued from previous page

| State | $\Gamma_{C_{3v}}$ | $D_{\max}$ | $S_{vN}$ | $\tilde{E}/\text{cm}^{-1}$ | $\Delta\text{Ref. [30]}$ |
|-------|-------------------|------------|----------|----------------------------|--------------------------|
| 1579  | $A_2$             | 48         | 0.33     | 4643.296710(4)             |                          |
| 1580  | $E$               | 81         | 0.56     | 4646.145427(1)             |                          |
| 1581  | $E$               | 70         | 0.56     | 4646.145427(1)             |                          |
| 1582  | $E$               | 71         | 2.0      | 4647.99376(2)              |                          |
| 1583  | $E$               | 64         | 2.0      | 4647.99376(4)              |                          |
| 1584  | $A_1$             | 61         | 2.0      | 4648.01754(5)              |                          |
| 1585  | $A_2$             | 71         | 2.0      | 4648.01755(3)              |                          |
| 1586  | $A_1$             | 79         | 2.1      | 4652.31132(1)              |                          |
| 1587  | $A_2$             | 68         | 2.1      | 4652.31239(2)              |                          |
| 1588  | $E$               | 71         | 2.1      | 4652.32374(2)              |                          |
| 1589  | $E$               | 66         | 2.1      | 4652.32374(6)              |                          |
| 1590  | $E$               | 83         | 0.069    | 4653.755419(2)             |                          |
| 1591  | $E$               | 70         | 0.07     | 4653.755419(4)             |                          |
| 1592  | $E$               | 117        | 2.3      | 4654.059112(5)             |                          |
| 1593  | $E$               | 104        | 2.3      | 4654.05911(1)              |                          |
| 1594  | $E$               | 97         | 2.2      | 4654.280742(9)             |                          |
| 1595  | $E$               | 99         | 2.2      | 4654.28074(1)              |                          |
| 1596  | $E$               | 87         | 0.65     | 4659.979931(2)             |                          |
| 1597  | $E$               | 84         | 0.65     | 4659.979931(2)             |                          |
| 1598  | $A_1$             | 102        | 2.3      | 4661.12566(2)              |                          |
| 1599  | $A_2$             | 103        | 2.3      | 4661.12566(2)              |                          |
| 1600  | $E$               | 108        | 2.3      | 4661.28984(1)              |                          |
| 1601  | $E$               | 98         | 2.3      | 4661.28985(1)              |                          |
| 1602  | $E$               | 103        | 0.79     | 4664.267481(1)             |                          |
| 1603  | $E$               | 87         | 0.79     | 4664.267481(2)             |                          |
| 1604  | $E$               | 67         | 0.36     | 4664.525979(1)             |                          |
| 1605  | $E$               | 59         | 0.36     | 4664.525981(2)             |                          |
| 1606  | $E$               | 152        | 2.3      | 4665.351223(2)             |                          |
| 1607  | $E$               | 99         | 2.4      | 4665.35123(2)              |                          |
| 1608  | $A_1$             | 90         | 2.3      | 4665.48763(4)              |                          |
| 1609  | $A_2$             | 98         | 2.3      | 4665.48789(2)              |                          |
| 1610  | $A_1$             | 91         | 0.84     | 4665.696886(2)             |                          |
| 1611  | $E$               | 139        | 2.3      | 4666.405368(5)             |                          |
| 1612  | $E$               | 139        | 2.3      | 4666.405368(5)             |                          |
| 1613  | $E$               | 99         | 0.54     | 4666.89545(1)              |                          |
| 1614  | $E$               | 104        | 0.55     | 4666.89545(1)              |                          |
| 1615  | $A_2$             | 130        | 3.7      | 4667.16649(1)              |                          |
| 1616  | $A_1$             | 145        | 3.3      | 4667.261023(7)             |                          |
| 1617  | $E$               | 147        | 3.2      | 4667.322899(4)             |                          |
| 1618  | $E$               | 152        | 3.2      | 4667.322900(5)             |                          |
| 1619  | $E$               | 152        | 2.3      | 4667.693050(2)             |                          |
| 1620  | $E$               | 141        | 2.3      | 4667.693050(5)             |                          |
| 1621  | $A_2$             | 131        | 2.8      | 4667.990008(9)             |                          |
| 1622  | $E$               | 136        | 2.3      | 4668.780935(3)             |                          |
| 1623  | $E$               | 129        | 2.3      | 4668.780939(4)             |                          |
| 1624  | $A_1$             | 121        | 2.2      | 4669.166197(4)             |                          |
| 1625  | $A_2$             | 89         | 2.0      | 4670.801097(1)             |                          |
| 1626  | $E$               | 79         | 2.0      | 4671.439550(1)             |                          |
| 1627  | $E$               | 80         | 2.0      | 4671.439550(2)             |                          |
| 1628  | $A_1$             | 79         | 2.0      | 4672.176930(2)             |                          |
| 1629  | $E$               | 109        | 0.27     | 4672.688799(6)             |                          |
| 1630  | $E$               | 117        | 0.27     | 4672.688799(5)             |                          |
| 1631  | $E$               | 125        | 2.4      | 4677.904031(7)             |                          |
| 1632  | $E$               | 147        | 2.3      | 4677.904031(6)             |                          |
| 1633  | $A_1^*$           | 97         | 2.1      | 4678.336385(8)             |                          |
| 1634  | $A_2^*$           | 99         | 2.1      | 4678.336386(7)             |                          |
| 1635  | $E$               | 101        | 2.3      | 4678.676103(9)             |                          |
| 1636  | $E$               | 129        | 2.3      | 4678.676103(9)             |                          |
| 1637  | $A_2$             | 86         | 2.2      | 4678.818095(9)             |                          |

Continued on next page.

TABLE S4 – states on Sarka/Poirier CSC PES; continued from previous page

| State | $\Gamma_{C_{3v}}$ | $D_{\max}$ | $S_{vN}$ | $\tilde{E}/\text{cm}^{-1}$ | $\Delta\text{Ref. [30]}$ |
|-------|-------------------|------------|----------|----------------------------|--------------------------|
| 1638  | $A_1$             | 82         | 2.2      | 4678.81810(1)              |                          |
| 1639  | $E$               | 170        | 2.5      | 4679.900560(4)             |                          |
| 1640  | $E$               | 172        | 2.5      | 4679.900561(4)             |                          |
| 1641  | $E$               | 164        | 2.4      | 4679.906343(4)             |                          |
| 1642  | $E$               | 165        | 2.4      | 4679.906343(4)             |                          |
| 1643  | $E$               | 122        | 0.44     | 4681.03503(1)              |                          |
| 1644  | $E$               | 159        | 0.43     | 4681.03503(1)              |                          |
| 1645  | $A_2$             | 173        | 2.6      | 4682.537848(4)             |                          |
| 1646  | $E$               | 174        | 2.4      | 4682.811511(4)             |                          |
| 1647  | $E$               | 172        | 2.5      | 4682.811512(4)             |                          |
| 1648  | $A_1$             | 158        | 2.4      | 4683.052757(7)             |                          |
| 1649  | $E$               | 143        | 2.5      | 4684.325087(2)             |                          |
| 1650  | $E$               | 93         | 2.5      | 4684.32509(2)              |                          |
| 1651  | $E$               | 107        | 2.4      | 4684.42697(1)              |                          |
| 1652  | $E$               | 94         | 2.4      | 4684.42697(2)              |                          |
| 1653  | $E$               | 129        | 3.4      | 4685.35750(2)              |                          |
| 1654  | $E$               | 170        | 3.4      | 4685.35750(2)              |                          |
| 1655  | $E$               | 174        | 3.3      | 4685.516149(5)             |                          |
| 1656  | $E$               | 166        | 3.3      | 4685.516150(4)             |                          |
| 1657  | $A_1$             | 166        | 3.3      | 4685.678019(4)             |                          |
| 1658  | $A_2$             | 163        | 3.3      | 4685.678212(4)             |                          |
| 1659  | $A_1$             | 110        | 3.1      | 4685.81926(2)              |                          |
| 1660  | $A_2$             | 98         | 3.1      | 4685.81927(5)              |                          |
| 1661  | $A_1$             | 154        | 3.5      | 4686.069864(9)             |                          |
| 1662  | $A_2$             | 152        | 3.5      | 4686.06990(1)              |                          |
| 1663  | $E$               | 127        | 2.2      | 4686.617187(9)             |                          |
| 1664  | $E$               | 171        | 2.2      | 4686.617189(9)             |                          |
| 1665  | $A_1$             | 103        | 2.7      | 4686.80717(4)              |                          |
| 1666  | $A_2$             | 111        | 2.7      | 4686.80725(5)              |                          |
| 1667  | $A_1$             | 101        | 2.6      | 4686.96961(1)              |                          |
| 1668  | $E$               | 86         | 2.5      | 4687.22546(1)              |                          |
| 1669  | $E$               | 114        | 2.5      | 4687.22546(1)              |                          |
| 1670  | $A_2$             | 85         | 2.5      | 4687.397295(2)             |                          |
| 1671  | $A_1$             | 155        | 3.3      | 4688.264187(6)             |                          |
| 1672  | $E$               | 159        | 2.8      | 4688.285594(4)             |                          |
| 1673  | $E$               | 139        | 2.8      | 4688.28560(1)              |                          |
| 1674  | $A_2$             | 159        | 3.4      | 4688.375651(4)             |                          |
| 1675  | $E$               | 137        | 3.1      | 4688.68033(1)              |                          |
| 1676  | $E$               | 149        | 3.1      | 4688.68033(1)              |                          |
| 1677  | $E$               | 129        | 2.6      | 4688.71253(2)              |                          |
| 1678  | $E$               | 131        | 2.6      | 4688.71253(1)              |                          |
| 1679  | $E$               | 124        | 0.69     | 4689.26952(1)              |                          |
| 1680  | $E$               | 120        | 0.69     | 4689.269518(8)             |                          |
| 1681  | $E$               | 82         | 0.5      | 4690.260055(3)             |                          |
| 1682  | $E$               | 78         | 0.5      | 4690.260057(2)             |                          |
| 1683  | $E$               | 130        | 2.5      | 4691.98949(1)              |                          |
| 1684  | $E$               | 143        | 2.5      | 4691.98950(1)              |                          |
| 1685  | $E$               | 128        | 2.2      | 4692.121714(7)             |                          |
| 1686  | $E$               | 172        | 2.2      | 4692.121717(7)             |                          |
| 1687  | $E$               | 93         | 2.3      | 4694.80150(1)              |                          |
| 1688  | $E$               | 111        | 2.3      | 4694.80151(1)              |                          |
| 1689  | $A_1$             | 101        | 2.3      | 4694.84222(1)              |                          |
| 1690  | $A_2$             | 104        | 2.3      | 4694.856248(7)             |                          |
| 1691  | $E$               | 115        | 2.2      | 4702.429656(2)             |                          |
| 1692  | $E$               | 115        | 2.2      | 4702.429656(2)             |                          |
| 1693  | $E$               | 91         | 3.1      | 4703.32833(1)              |                          |
| 1694  | $E$               | 88         | 3.1      | 4703.32833(1)              |                          |
| 1695  | $A_1$             | 88         | 3.1      | 4703.33175(1)              |                          |
| 1696  | $A_2$             | 88         | 3.1      | 4703.33258(1)              |                          |

Continued on next page.

TABLE S4 – states on Sarka/Poirier CSC PES; continued from previous page

| State | $\Gamma_{C_{3v}}$ | $D_{\max}$ | $S_{vN}$ | $\tilde{E}/\text{cm}^{-1}$ | $\Delta\text{Ref. [30]}$ |
|-------|-------------------|------------|----------|----------------------------|--------------------------|
| 1697  | $E$               | 94         | 2.1      | 4703.746683(4)             |                          |
| 1698  | $E$               | 90         | 2.1      | 4703.746684(6)             |                          |
| 1699  | $A_1^*$           | 99         | 2.1      | 4719.06557(1)              |                          |
| 1700  | $A_2^*$           | 95         | 2.1      | 4719.065575(9)             |                          |
| 1701  | $E$               | 102        | 2.1      | 4719.08281(1)              |                          |
| 1702  | $E$               | 90         | 2.1      | 4719.08281(2)              |                          |
| 1703  | $A_1^*$           | 53         | 0.13     | 4723.85439(1)              |                          |
| 1704  | $A_2^*$           | 54         | 0.13     | 4723.85439(1)              |                          |
| 1705  | $E$               | 76         | 0.69     | 4723.911851(2)             |                          |
| 1706  | $E$               | 79         | 0.69     | 4723.911852(3)             |                          |
| 1707  | $E$               | 129        | 2.2      | 4724.751811(3)             |                          |
| 1708  | $E$               | 109        | 2.2      | 4724.751811(6)             |                          |
| 1709  | $E$               | 110        | 2.2      | 4724.773803(5)             |                          |
| 1710  | $E$               | 130        | 2.2      | 4724.773803(3)             |                          |
| 1711  | $A_2$             | 109        | 2.2      | 4727.318772(7)             |                          |
| 1712  | $E$               | 104        | 2.2      | 4727.64619(1)              |                          |
| 1713  | $E$               | 105        | 2.2      | 4727.646190(7)             |                          |
| 1714  | $A_1$             | 105        | 2.2      | 4727.926735(9)             |                          |
| 1715  | $E$               | 87         | 0.28     | 4732.498730(4)             |                          |
| 1716  | $E$               | 95         | 0.28     | 4732.498730(3)             |                          |
| 1717  | $E$               | 112        | 0.54     | 4732.878249(2)             |                          |
| 1718  | $E$               | 113        | 0.54     | 4732.878249(2)             |                          |
| 1719  | $E$               | 91         | 0.22     | 4734.755564(1)             |                          |
| 1720  | $E$               | 95         | 0.22     | 4734.7555647(9)            |                          |
| 1721  | $E$               | 100        | 2.2      | 4737.923090(4)             |                          |
| 1722  | $E$               | 82         | 2.2      | 4737.92309(1)              |                          |
| 1723  | $A_1$             | 71         | 2.2      | 4737.96445(2)              |                          |
| 1724  | $A_2$             | 99         | 2.2      | 4737.968196(1)             |                          |
| 1725  | $A_2$             | 87         | 2.1      | 4739.92634(2)              |                          |
| 1726  | $A_1$             | 115        | 2.1      | 4739.926832(3)             |                          |
| 1727  | $E$               | 94         | 2.1      | 4739.938982(6)             |                          |
| 1728  | $E$               | 106        | 2.1      | 4739.93899(1)              |                          |
| 1729  | $E$               | 82         | 0.28     | 4741.091097(1)             |                          |
| 1730  | $E$               | 76         | 0.28     | 4741.091097(2)             |                          |
| 1731  | $A_1$             | 125        | 2.2      | 4742.027284(7)             |                          |
| 1732  | $A_2$             | 124        | 2.2      | 4742.027285(8)             |                          |
| 1733  | $E$               | 150        | 3.2      | 4742.829806(4)             |                          |
| 1734  | $E$               | 141        | 3.2      | 4742.829806(5)             |                          |
| 1735  | $E$               | 85         | 0.27     | 4742.935230(3)             |                          |
| 1736  | $E$               | 99         | 0.27     | 4742.935230(1)             |                          |
| 1737  | $E$               | 142        | 3.1      | 4742.986322(3)             |                          |
| 1738  | $E$               | 146        | 3.1      | 4742.986322(3)             |                          |
| 1739  | $A_2^*$           | 96         | 2.2      | 4743.33802(1)              |                          |
| 1740  | $A_1^*$           | 95         | 2.2      | 4743.33802(1)              |                          |
| 1741  | $E$               | 86         | 0.62     | 4744.812760(3)             |                          |
| 1742  | $E$               | 84         | 0.62     | 4744.812762(1)             |                          |
| 1743  | $E$               | 80         | 2.2      | 4747.323240(6)             |                          |
| 1744  | $E$               | 127        | 2.2      | 4747.32325(1)              |                          |
| 1745  | $A_2^*$           | 85         | 2.2      | 4747.334588(6)             |                          |
| 1746  | $A_1^*$           | 102        | 2.2      | 4747.334591(9)             |                          |
| 1747  | $A_1$             | 58         | 0.3      | 4748.39012(5)              |                          |
| 1748  | $A_2$             | 64         | 0.3      | 4748.39019(2)              |                          |
| 1749  | $E$               | 163        | 2.3      | 4749.054859(3)             |                          |
| 1750  | $E$               | 132        | 2.3      | 4749.05486(1)              |                          |
| 1751  | $E$               | 174        | 3.3      | 4749.849532(4)             |                          |
| 1752  | $E$               | 184        | 3.3      | 4749.849532(3)             |                          |
| 1753  | $A_2^*$           | 145        | 3.1      | 4750.000421(5)             |                          |
| 1754  | $A_1^*$           | 147        | 3.1      | 4750.000421(6)             |                          |
| 1755  | $E$               | 128        | 2.2      | 4750.358664(8)             |                          |

Continued on next page.

TABLE S4 – states on Sarka/Poirier CSC PES; continued from previous page

| State | $\Gamma_{C_{3v}}$ | $D_{\max}$ | $S_{vN}$ | $\tilde{E}/\text{cm}^{-1}$ | $\Delta\text{Ref. [30]}$ |
|-------|-------------------|------------|----------|----------------------------|--------------------------|
| 1756  | $E$               | 135        | 2.2      | 4750.358664(7)             |                          |
| 1757  | $A_1^*$           | 62         | 0.68     | 4750.60278(2)              |                          |
| 1758  | $A_2^*$           | 64         | 0.68     | 4750.60278(1)              |                          |
| 1759  | $E$               | 120        | 2.7      | 4750.67729(1)              |                          |
| 1760  | $E$               | 135        | 2.7      | 4750.67729(1)              |                          |
| 1761  | $A_2$             | 125        | 2.7      | 4750.741710(9)             |                          |
| 1762  | $A_1$             | 135        | 2.7      | 4750.74180(1)              |                          |
| 1763  | $E$               | 92         | 0.32     | 4751.118145(3)             |                          |
| 1764  | $E$               | 98         | 0.32     | 4751.118145(2)             |                          |
| 1765  | $E$               | 130        | 2.3      | 4751.577065(2)             |                          |
| 1766  | $E$               | 128        | 2.3      | 4751.577065(2)             |                          |
| 1767  | $A_1$             | 83         | 2.3      | 4751.61904(1)              |                          |
| 1768  | $A_2$             | 87         | 2.3      | 4751.61921(1)              |                          |
| 1769  | $E$               | 145        | 0.79     | 4752.188275(2)             |                          |
| 1770  | $E$               | 144        | 0.79     | 4752.188275(2)             |                          |
| 1771  | $A_1^*$           | 76         | 2.1      | 4752.82446(1)              |                          |
| 1772  | $A_2^*$           | 77         | 2.1      | 4752.82446(1)              |                          |
| 1773  | $E$               | 139        | 0.6      | 4753.084599(1)             |                          |
| 1774  | $E$               | 122        | 0.6      | 4753.084600(4)             |                          |
| 1775  | $E$               | 113        | 2.1      | 4753.127896(1)             |                          |
| 1776  | $E$               | 88         | 2.1      | 4753.127898(5)             |                          |
| 1777  | $E$               | 132        | 2.5      | 4753.25638(1)              |                          |
| 1778  | $E$               | 136        | 2.5      | 4753.25638(1)              |                          |
| 1779  | $A_2$             | 149        | 3.8      | 4753.758641(8)             |                          |
| 1780  | $A_1$             | 167        | 3.2      | 4754.128546(3)             |                          |
| 1781  | $E$               | 146        | 3.2      | 4754.211918(7)             |                          |
| 1782  | $E$               | 141        | 3.2      | 4754.211920(3)             |                          |
| 1783  | $E$               | 124        | 2.2      | 4754.569393(7)             |                          |
| 1784  | $E$               | 126        | 2.2      | 4754.569393(8)             |                          |
| 1785  | $A_2$             | 145        | 3.3      | 4755.070260(7)             |                          |
| 1786  | $E$               | 120        | 2.4      | 4755.644752(3)             |                          |
| 1787  | $E$               | 121        | 2.4      | 4755.644752(3)             |                          |
| 1788  | $A_1$             | 111        | 2.2      | 4755.984890(4)             |                          |
| 1789  | $E$               | 91         | 0.9      | 4757.400300(2)             |                          |
| 1790  | $E$               | 83         | 0.9      | 4757.400301(2)             |                          |
| 1791  | $A_2$             | 166        | 3.2      | 4757.808260(3)             |                          |
| 1792  | $A_1$             | 161        | 3.2      | 4757.808311(3)             |                          |
| 1793  | $E$               | 154        | 3.2      | 4757.885941(3)             |                          |
| 1794  | $E$               | 163        | 3.2      | 4757.885941(3)             |                          |
| 1795  | $E$               | 141        | 2.9      | 4758.172317(6)             |                          |
| 1796  | $E$               | 154        | 2.9      | 4758.172318(6)             |                          |
| 1797  | $E$               | 157        | 2.9      | 4758.207819(2)             |                          |
| 1798  | $E$               | 143        | 2.8      | 4758.207820(5)             |                          |
| 1799  | $E$               | 136        | 2.2      | 4759.323300(4)             |                          |
| 1800  | $E$               | 144        | 2.2      | 4759.323300(4)             |                          |
| 1801  | $A_2$             | 102        | 2.1      | 4759.65402(2)              |                          |
| 1802  | $A_1$             | 113        | 2.1      | 4759.67225(1)              |                          |
| 1803  | $E$               | 80         | 1.0      | 4761.480243(3)             |                          |
| 1804  | $E$               | 82         | 1.0      | 4761.480244(3)             |                          |
| 1805  | $A_1$             | 91         | 1.1      | 4762.840463(1)             |                          |
| 1806  | $E$               | 119        | 0.81     | 4764.229107(3)             |                          |
| 1807  | $E$               | 136        | 0.83     | 4764.229111(5)             |                          |
| 1808  | $E$               | 119        | 2.2      | 4764.960933(3)             |                          |
| 1809  | $E$               | 89         | 2.2      | 4764.96094(1)              |                          |
| 1810  | $A_2$             | 100        | 2.2      | 4765.215871(9)             |                          |
| 1811  | $A_1$             | 90         | 2.2      | 4765.215875(5)             |                          |
| 1812  | $E$               | 103        | 0.63     | 4765.450101(3)             |                          |
| 1813  | $E$               | 83         | 0.65     | 4765.45010(1)              |                          |
| 1814  | $A_1$             | 76         | 0.6      | 4766.459059(2)             |                          |

Continued on next page.



TABLE S4 – states on Sarka/Poirier CSC PES; continued from previous page

| State | $\Gamma_{C_{3v}}$ | $D_{\max}$ | $S_{vN}$ | $\tilde{E}/\text{cm}^{-1}$ | $\Delta\text{Ref. [30]}$ |
|-------|-------------------|------------|----------|----------------------------|--------------------------|
| 1815  | $A_2$             | 55         | 0.6      | 4766.459064(7)             |                          |
| 1816  | $E$               | 54         | 0.61     | 4769.374549(6)             |                          |
| 1817  | $E$               | 69         | 0.61     | 4769.374551(5)             |                          |
| 1818  | $A_1$             | 105        | 3.1      | 4769.68344(2)              |                          |
| 1819  | $E$               | 101        | 2.7      | 4769.68599(3)              |                          |
| 1820  | $E$               | 92         | 2.7      | 4769.68600(7)              |                          |
| 1821  | $A_2$             | 97         | 3.1      | 4769.68841(4)              |                          |
| 1822  | $E$               | 159        | 2.5      | 4772.750538(4)             |                          |
| 1823  | $E$               | 148        | 2.5      | 4772.750540(3)             |                          |
| 1824  | $A_1$             | 81         | 0.47     | 4772.798519(1)             |                          |
| 1825  | $A_1$             | 108        | 3.0      | 4772.88903(2)              |                          |
| 1826  | $A_2$             | 109        | 3.0      | 4772.88932(2)              |                          |
| 1827  | $E$               | 137        | 0.64     | 4774.268391(3)             |                          |
| 1828  | $E$               | 144        | 0.63     | 4774.268392(4)             |                          |
| 1829  | $E$               | 139        | 2.3      | 4774.408468(2)             |                          |
| 1830  | $E$               | 138        | 2.3      | 4774.408468(2)             |                          |
| 1831  | $E$               | 131        | 2.3      | 4774.618034(2)             |                          |
| 1832  | $E$               | 136        | 2.3      | 4774.618034(2)             |                          |
| 1833  | $E$               | 66         | 0.32     | 4774.735341(1)             |                          |
| 1834  | $E$               | 50         | 0.32     | 4774.735342(2)             |                          |
| 1835  | $A_1$             | 75         | 0.14     | 4778.941866(3)             |                          |
| 1836  | $E$               | 67         | 0.07     | 4779.788140(6)             |                          |
| 1837  | $E$               | 65         | 0.07     | 4779.788141(4)             |                          |
| 1838  | $E$               | 117        | 2.6      | 4780.774368(3)             |                          |
| 1839  | $E$               | 117        | 2.6      | 4780.774368(3)             |                          |
| 1840  | $A_1$             | 99         | 2.5      | 4780.830271(8)             |                          |
| 1841  | $A_2$             | 88         | 2.5      | 4780.83032(1)              |                          |
| 1842  | $A_1$             | 88         | 2.3      | 4781.15740(2)              |                          |
| 1843  | $A_2$             | 84         | 2.3      | 4781.15742(3)              |                          |
| 1844  | $E$               | 109        | 2.3      | 4781.332228(9)             |                          |
| 1845  | $E$               | 140        | 2.3      | 4781.332229(8)             |                          |
| 1846  | $E$               | 109        | 0.62     | 4782.277279(2)             |                          |
| 1847  | $E$               | 112        | 0.62     | 4782.277281(3)             |                          |
| 1848  | $E$               | 131        | 1.3      | 4783.656237(3)             |                          |
| 1849  | $E$               | 153        | 1.2      | 4783.656241(6)             |                          |
| 1850  | $E$               | 114        | 1.1      | 4783.871256(9)             |                          |
| 1851  | $E$               | 117        | 1.1      | 4783.87126(1)              |                          |
| 1852  | $E$               | 68         | 0.12     | 4784.388008(3)             |                          |
| 1853  | $E$               | 68         | 0.12     | 4784.388010(4)             |                          |
| 1854  | $A_1$             | 131        | 0.25     | 4785.137519(4)             |                          |
| 1855  | $E$               | 101        | 2.4      | 4785.15971(1)              |                          |
| 1856  | $E$               | 131        | 2.4      | 4785.15971(1)              |                          |
| 1857  | $A_2$             | 119        | 0.25     | 4785.306792(2)             |                          |
| 1858  | $A_1$             | 82         | 2.3      | 4785.36129(2)              |                          |
| 1859  | $A_2$             | 81         | 2.3      | 4785.36167(2)              |                          |
| 1860  | $A_2$             | 92         | 2.3      | 4785.953809(5)             |                          |
| 1861  | $A_1$             | 127        | 2.3      | 4785.953810(5)             |                          |
| 1862  | $E$               | 86         | 2.2      | 4786.069893(6)             |                          |
| 1863  | $E$               | 82         | 2.2      | 4786.069894(5)             |                          |
| 1864  | $E$               | 92         | 0.75     | 4786.749361(7)             |                          |
| 1865  | $E$               | 82         | 0.75     | 4786.74936(1)              |                          |
| 1866  | $A_1$             | 60         | 0.72     | 4787.30763(1)              |                          |
| 1867  | $A_2$             | 70         | 0.72     | 4787.30764(2)              |                          |
| 1868  | $E$               | 99         | 4.6      | 4790.177538(5)             |                          |
| 1869  | $E$               | 98         | 4.5      | 4790.177538(5)             |                          |
| 1870  | $E$               | 76         | 5.5      | 4790.31249(5)              |                          |
| 1871  | $E$               | 93         | 5.6      | 4790.31250(5)              |                          |
| 1872  | $A_1$             | 83         | 2.2      | 4790.360600(3)             |                          |
| 1873  | $A_2$             | 131        | 2.2      | 4790.36073(1)              |                          |

Continued on next page.

TABLE S4 – states on Sarka/Poirier CSC PES; continued from previous page

| State | $\Gamma_{C_{3v}}$ | $D_{\max}$ | $S_{vN}$ | $\tilde{E}/\text{cm}^{-1}$ | $\Delta\text{Ref. [30]}$ |
|-------|-------------------|------------|----------|----------------------------|--------------------------|
| 1874  | $E$               | 81         | 0.36     | 4791.786718(7)             |                          |
| 1875  | $E$               | 80         | 0.36     | 4791.786718(8)             |                          |
| 1876  | $E$               | 79         | 1.1      | 4795.681156(1)             |                          |
| 1877  | $E$               | 67         | 1.1      | 4795.681157(2)             |                          |
| 1878  | $A_1$             | 72         | 1.2      | 4797.144503(2)             |                          |
| 1879  | $E$               | 104        | 0.46     | 4801.845784(2)             |                          |
| 1880  | $E$               | 106        | 0.46     | 4801.845785(2)             |                          |
| 1881  | $A_1$             | 60         | 0.48     | 4805.38102(3)              |                          |
| 1882  | $A_2$             | 125        | 1.1      | 4807.456270(4)             |                          |
| 1883  | $A_1$             | 133        | 1.1      | 4807.456290(4)             |                          |
| 1884  | $E$               | 128        | 2.0      | 4808.835880(3)             |                          |
| 1885  | $E$               | 107        | 2.0      | 4808.83588(1)              |                          |
| 1886  | $A_1$             | 112        | 2.5      | 4808.956678(6)             |                          |
| 1887  | $A_2$             | 102        | 2.5      | 4808.956680(9)             |                          |
| 1888  | $E$               | 116        | 0.69     | 4810.322948(4)             |                          |
| 1889  | $E$               | 116        | 0.69     | 4810.322949(5)             |                          |
| 1890  | $E$               | 58         | 1.3      | 4810.73710(1)              |                          |
| 1891  | $E$               | 94         | 1.3      | 4810.73711(1)              |                          |
| 1892  | $A_2$             | 74         | 2.1      | 4810.793087(1)             |                          |
| 1893  | $E$               | 93         | 2.0      | 4811.430124(2)             |                          |
| 1894  | $E$               | 110        | 2.0      | 4811.430125(3)             |                          |
| 1895  | $E$               | 93         | 2.1      | 4811.475714(6)             |                          |
| 1896  | $E$               | 100        | 2.1      | 4811.475714(5)             |                          |
| 1897  | $E$               | 74         | 2.1      | 4811.672340(1)             |                          |
| 1898  | $E$               | 79         | 2.1      | 4811.672341(2)             |                          |
| 1899  | $A_1$             | 84         | 2.1      | 4812.088645(1)             |                          |
| 1900  | $A_1$             | 60         | 1.4      | 4812.196103(4)             |                          |
| 1901  | $E$               | 112        | 2.1      | 4814.541127(5)             |                          |
| 1902  | $E$               | 128        | 2.1      | 4814.541131(7)             |                          |
| 1903  | $E$               | 145        | 2.2      | 4814.601433(2)             |                          |
| 1904  | $E$               | 118        | 2.2      | 4814.601435(9)             |                          |
| 1905  | $A_2$             | 92         | 2.1      | 4817.403120(9)             |                          |
| 1906  | $A_1$             | 117        | 2.1      | 4817.404613(3)             |                          |
| 1907  | $E$               | 126        | 2.1      | 4817.423690(2)             |                          |
| 1908  | $E$               | 90         | 2.1      | 4817.42370(1)              |                          |
| 1909  | $A_2$             | 108        | 2.7      | 4817.741641(4)             |                          |
| 1910  | $A_2^*$           | 110        | 2.5      | 4817.74519(1)              |                          |
| 1911  | $A_1^*$           | 105        | 2.5      | 4817.74519(2)              |                          |
| 1912  | $E$               | 104        | 2.4      | 4817.89464(2)              |                          |
| 1913  | $E$               | 106        | 2.4      | 4817.89464(2)              |                          |
| 1914  | $E$               | 117        | 2.7      | 4817.934996(2)             |                          |
| 1915  | $E$               | 112        | 2.7      | 4817.934997(3)             |                          |
| 1916  | $A_1$             | 103        | 2.7      | 4818.141714(4)             |                          |
| 1917  | $A_1$             | 66         | 2.1      | 4819.46050(5)              |                          |
| 1918  | $A_2$             | 65         | 2.1      | 4819.46086(5)              |                          |
| 1919  | $E$               | 67         | 2.1      | 4819.47314(4)              |                          |
| 1920  | $E$               | 62         | 2.1      | 4819.47315(8)              |                          |
| 1921  | $E$               | 88         | 0.099    | 4820.933398(3)             |                          |
| 1922  | $E$               | 81         | 0.097    | 4820.933398(3)             |                          |
| 1923  | $E$               | 106        | 2.6      | 4822.06841(2)              |                          |
| 1924  | $E$               | 127        | 2.6      | 4822.06841(2)              |                          |
| 1925  | $A_1$             | 84         | 2.5      | 4822.17284(9)              |                          |
| 1926  | $A_2$             | 95         | 2.5      | 4822.17300(4)              |                          |
| 1927  | $E$               | 81         | 2.1      | 4822.33775(1)              |                          |
| 1928  | $E$               | 88         | 2.1      | 4822.33775(2)              |                          |
| 1929  | $A_1^*$           | 88         | 2.2      | 4822.352096(8)             |                          |
| 1930  | $A_2^*$           | 87         | 2.2      | 4822.352097(9)             |                          |
| 1931  | $E$               | 95         | 0.67     | 4823.59348(1)              |                          |
| 1932  | $E$               | 143        | 0.68     | 4823.59348(1)              |                          |

Continued on next page.

TABLE S4 – states on Sarka/Poirier CSC PES; continued from previous page

| State | $\Gamma_{C_{3v}}$ | $D_{\max}$ | $S_{vN}$ | $\tilde{E}/\text{cm}^{-1}$ | $\Delta\text{Ref. [30]}$ |
|-------|-------------------|------------|----------|----------------------------|--------------------------|
| 1933  | $E$               | 98         | 2.3      | 4824.51467(1)              |                          |
| 1934  | $E$               | 100        | 2.3      | 4824.51467(1)              |                          |
| 1935  | $E$               | 97         | 2.2      | 4824.59219(1)              |                          |
| 1936  | $E$               | 139        | 2.2      | 4824.59219(1)              |                          |
| 1937  | $A_1$             | 92         | 2.5      | 4827.27304(1)              |                          |
| 1938  | $E$               | 84         | 2.4      | 4827.439783(2)             |                          |
| 1939  | $E$               | 82         | 2.4      | 4827.439784(3)             |                          |
| 1940  | $A_2$             | 85         | 2.4      | 4827.547718(2)             |                          |
| 1941  | $E$               | 119        | 2.2      | 4830.501692(3)             |                          |
| 1942  | $E$               | 104        | 2.2      | 4830.501692(9)             |                          |
| 1943  | $A_1^*$           | 85         | 2.2      | 4830.52870(1)              |                          |
| 1944  | $A_2^*$           | 84         | 2.2      | 4830.52870(1)              |                          |
| 1945  | $E$               | 98         | 1.8      | 4831.848334(2)             |                          |
| 1946  | $E$               | 96         | 1.8      | 4831.848334(2)             |                          |
| 1947  | $E$               | 99         | 1.8      | 4831.865562(1)             |                          |
| 1948  | $E$               | 101        | 1.8      | 4831.865562(1)             |                          |
| 1949  | $E$               | 103        | 0.37     | 4831.87165(3)              |                          |
| 1950  | $E$               | 127        | 0.37     | 4831.87165(3)              |                          |
| 1951  | $E$               | 86         | 0.46     | 4835.109334(5)             |                          |
| 1952  | $E$               | 118        | 0.46     | 4835.109335(5)             |                          |
| 1953  | $E$               | 135        | 2.2      | 4835.900728(1)             |                          |
| 1954  | $E$               | 139        | 2.2      | 4835.900728(1)             |                          |
| 1955  | $E$               | 136        | 2.2      | 4836.004061(2)             |                          |
| 1956  | $E$               | 121        | 2.2      | 4836.004061(4)             |                          |
| 1957  | $A_1$             | 142        | 3.4      | 4837.06307(1)              |                          |
| 1958  | $A_2$             | 141        | 3.4      | 4837.06308(1)              |                          |
| 1959  | $E$               | 123        | 2.2      | 4837.446289(9)             |                          |
| 1960  | $E$               | 114        | 2.2      | 4837.446293(6)             |                          |
| 1961  | $A_1$             | 100        | 2.2      | 4837.6226(1)               |                          |
| 1962  | $A_2$             | 125        | 2.1      | 4837.6227(1)               |                          |
| 1963  | $A_2$             | 129        | 2.3      | 4838.210962(2)             |                          |
| 1964  | $E$               | 62         | 0.025    | 4838.654231(3)             |                          |
| 1965  | $E$               | 51         | 0.025    | 4838.654231(4)             |                          |
| 1966  | $E$               | 95         | 2.3      | 4838.782197(9)             |                          |
| 1967  | $E$               | 118        | 2.3      | 4838.782198(7)             |                          |
| 1968  | $A_1$             | 120        | 2.3      | 4839.198046(2)             |                          |
| 1969  | $E$               | 122        | 0.7      | 4840.30417(1)              |                          |
| 1970  | $E$               | 165        | 0.7      | 4840.30417(1)              |                          |
| 1971  | $A_1$             | 118        | 0.5      | 4840.795390(3)             |                          |
| 1972  | $A_2$             | 86         | 0.5      | 4840.795399(4)             |                          |
| 1973  | $E$               | 181        | 2.5      | 4842.908818(4)             |                          |
| 1974  | $E$               | 127        | 2.5      | 4842.90882(2)              |                          |
| 1975  | $E$               | 109        | 2.3      | 4843.05056(4)              |                          |
| 1976  | $E$               | 183        | 2.3      | 4843.05056(4)              |                          |
| 1977  | $E$               | 86         | 0.52     | 4843.639044(6)             |                          |
| 1978  | $E$               | 92         | 0.52     | 4843.639044(6)             |                          |
| 1979  | $A_2$             | 108        | 2.4      | 4844.877745(4)             |                          |
| 1980  | $E$               | 115        | 2.4      | 4845.752616(2)             |                          |
| 1981  | $E$               | 98         | 2.4      | 4845.752620(7)             |                          |
| 1982  | $E$               | 72         | 0.15     | 4845.7639603(8)            |                          |
| 1983  | $E$               | 57         | 0.15     | 4845.763960(2)             |                          |
| 1984  | $E$               | 100        | 2.4      | 4845.77866(1)              |                          |
| 1985  | $E$               | 95         | 2.4      | 4845.77866(3)              |                          |
| 1986  | $A_1$             | 110        | 2.4      | 4845.822400(6)             |                          |
| 1987  | $A_2$             | 95         | 2.4      | 4845.83333(4)              |                          |
| 1988  | $A_1$             | 117        | 2.4      | 4846.157068(3)             |                          |
| 1989  | $A_2$             | 121        | 2.8      | 4852.627232(3)             |                          |
| 1990  | $E$               | 125        | 2.8      | 4852.731677(2)             |                          |
| 1991  | $E$               | 125        | 2.8      | 4852.731677(2)             |                          |

Continued on next page.

TABLE S4 – states on Sarka/Poirier CSC PES; continued from previous page

| State | $\Gamma_{C_{3v}}$ | $D_{\max}$ | $S_{vN}$ | $\tilde{E}/\text{cm}^{-1}$ | $\Delta\text{Ref. [30]}$ |
|-------|-------------------|------------|----------|----------------------------|--------------------------|
| 1992  | $A_1$             | 121        | 2.8      | 4852.846503(3)             |                          |
| 1993  | $E$               | 86         | 2.1      | 4853.105604(3)             |                          |
| 1994  | $E$               | 85         | 2.1      | 4853.105604(3)             |                          |
| 1995  | $E$               | 103        | 2.2      | 4853.110137(2)             |                          |
| 1996  | $E$               | 92         | 2.2      | 4853.110137(3)             |                          |
| 1997  | $A_2$             | 165        | 2.6      | 4853.585078(4)             |                          |
| 1998  | $E$               | 126        | 2.5      | 4853.70738(1)              |                          |
| 1999  | $E$               | 146        | 2.5      | 4853.70738(2)              |                          |
| 2000  | $A_1$             | 153        | 2.5      | 4853.836690(6)             |                          |
| 2001  | $E$               | 67         | 0.22     | 4854.121486(5)             |                          |
| 2002  | $E$               | 79         | 0.22     | 4854.121486(2)             |                          |
| 2003  | $E$               | 69         | 0.2      | 4854.298331(2)             |                          |
| 2004  | $E$               | 75         | 0.2      | 4854.298331(1)             |                          |
| 2005  | $A_2$             | 99         | 2.2      | 4855.821231(3)             |                          |
| 2006  | $E$               | 96         | 2.2      | 4856.032091(5)             |                          |
| 2007  | $E$               | 95         | 2.2      | 4856.032091(4)             |                          |
| 2008  | $A_1$             | 88         | 2.2      | 4856.231558(5)             |                          |
| 2009  | $A_1$             | 146        | 3.3      | 4859.184392(4)             |                          |
| 2010  | $E$               | 137        | 3.0      | 4859.231022(7)             |                          |
| 2011  | $E$               | 100        | 3.0      | 4859.23103(4)              |                          |
| 2012  | $A_2$             | 98         | 3.3      | 4859.23452(3)              |                          |
| 2013  | $E$               | 130        | 2.8      | 4859.547164(6)             |                          |
| 2014  | $E$               | 136        | 2.8      | 4859.547165(8)             |                          |
| 2015  | $E$               | 119        | 2.9      | 4859.561366(8)             |                          |
| 2016  | $E$               | 107        | 2.9      | 4859.56137(1)              |                          |
| 2017  | $A_1$             | 53         | 0.25     | 4859.69482(3)              |                          |
| 2018  | $A_2$             | 56         | 0.25     | 4859.69484(1)              |                          |
| 2019  | $E$               | 74         | 0.27     | 4862.482113(2)             |                          |
| 2020  | $E$               | 78         | 0.27     | 4862.482113(2)             |                          |
| 2021  | $A_1$             | 82         | 0.3      | 4867.344843(2)             |                          |
| 2022  | $A_2$             | 68         | 0.3      | 4867.344844(2)             |                          |
| 2023  | $A_2$             | 50         | 0.35     | 4876.82946(1)              |                          |
| 2024  | $A_1$             | 54         | 0.35     | 4876.829461(7)             |                          |
| 2025  | $E$               | 73         | 0.37     | 4877.658021(5)             |                          |
| 2026  | $E$               | 94         | 0.37     | 4877.658022(4)             |                          |
| 2027  | $E$               | 86         | 0.38     | 4877.788475(3)             |                          |
| 2028  | $E$               | 81         | 0.38     | 4877.788475(3)             |                          |
| 2029  | $A_1$             | 103        | 0.22     | 4881.473779(2)             |                          |
| 2030  | $E$               | 81         | 0.76     | 4883.733687(2)             |                          |
| 2031  | $E$               | 80         | 0.76     | 4883.733688(1)             |                          |
| 2032  | $E$               | 78         | 0.43     | 4885.624856(2)             |                          |
| 2033  | $E$               | 88         | 0.43     | 4885.624856(3)             |                          |
| 2034  | $E$               | 85         | 0.55     | 4885.975671(3)             |                          |
| 2035  | $E$               | 94         | 0.55     | 4885.975672(1)             |                          |
| 2036  | $E$               | 106        | 0.2      | 4886.966802(2)             |                          |
| 2037  | $E$               | 107        | 0.2      | 4886.966802(2)             |                          |
| 2038  | $E$               | 99         | 2.3      | 4887.159467(9)             |                          |
| 2039  | $E$               | 124        | 2.3      | 4887.159468(6)             |                          |
| 2040  | $E$               | 104        | 2.3      | 4887.163870(7)             |                          |
| 2041  | $E$               | 115        | 2.3      | 4887.163870(6)             |                          |
| 2042  | $E$               | 82         | 0.95     | 4887.877908(2)             |                          |
| 2043  | $E$               | 79         | 0.95     | 4887.877909(4)             |                          |
| 2044  | $E$               | 42         | 0.13     | 4889.152474(3)             |                          |
| 2045  | $E$               | 45         | 0.13     | 4889.152474(2)             |                          |
| 2046  | $A_1$             | 84         | 1.0      | 4889.259595(2)             |                          |
| 2047  | $E$               | 58         | 0.096    | 4889.356110(9)             |                          |
| 2048  | $E$               | 58         | 0.096    | 4889.35611(1)              |                          |
| 2049  | $A_2$             | 107        | 2.4      | 4889.867791(5)             |                          |
| 2050  | $E$               | 105        | 2.3      | 4890.07982(1)              |                          |

Continued on next page.

TABLE S4 – states on Sarka/Poirier CSC PES; continued from previous page

| State | $\Gamma_{C_{3v}}$ | $D_{\max}$ | $S_{vN}$ | $\tilde{E}/\text{cm}^{-1}$ | $\Delta\text{Ref. [30]}$ |
|-------|-------------------|------------|----------|----------------------------|--------------------------|
| 2051  | $E$               | 103        | 2.4      | 4890.07982(1)              |                          |
| 2052  | $A_1$             | 104        | 2.3      | 4890.27982(1)              |                          |
| 2053  | $A_1$             | 60         | 0.11     | 4890.827694(7)             |                          |
| 2054  | $A_1$             | 62         | 0.47     | 4890.85084(3)              |                          |
| 2055  | $A_2$             | 62         | 0.47     | 4890.85103(2)              |                          |
| 2056  | $A_2$             | 67         | 0.65     | 4891.52318(8)              |                          |
| 2057  | $A_1$             | 67         | 0.65     | 4891.52319(6)              |                          |
| 2058  | $E$               | 80         | 0.48     | 4893.464495(2)             |                          |
| 2059  | $E$               | 86         | 0.48     | 4893.464495(3)             |                          |
| 2060  | $E$               | 97         | 0.69     | 4894.297294(1)             |                          |
| 2061  | $E$               | 81         | 0.69     | 4894.297294(5)             |                          |
| 2062  | $E$               | 79         | 2.2      | 4897.74412(1)              |                          |
| 2063  | $E$               | 95         | 2.2      | 4897.744123(7)             |                          |
| 2064  | $A_1$             | 82         | 2.2      | 4897.748700(6)             |                          |
| 2065  | $A_2$             | 97         | 2.2      | 4897.748741(3)             |                          |
| 2066  | $E$               | 95         | 0.36     | 4899.223344(3)             |                          |
| 2067  | $E$               | 82         | 0.37     | 4899.223345(6)             |                          |
| 2068  | $A_1$             | 151        | 3.3      | 4901.279830(4)             |                          |
| 2069  | $E$               | 147        | 3.3      | 4901.438000(4)             |                          |
| 2070  | $E$               | 154        | 3.3      | 4901.438001(4)             |                          |
| 2071  | $A_2$             | 151        | 2.5      | 4901.726873(3)             |                          |
| 2072  | $E$               | 126        | 2.2      | 4902.320593(2)             |                          |
| 2073  | $E$               | 99         | 2.2      | 4902.32059(1)              |                          |
| 2074  | $A_2^*$           | 86         | 2.2      | 4902.560113(9)             |                          |
| 2075  | $A_1^*$           | 85         | 2.2      | 4902.56011(1)              |                          |
| 2076  | $E$               | 135        | 1.5      | 4905.338050(3)             |                          |
| 2077  | $E$               | 137        | 1.5      | 4905.338050(4)             |                          |
| 2078  | $E$               | 129        | 2.2      | 4905.60798(1)              |                          |
| 2079  | $E$               | 130        | 2.2      | 4905.60798(1)              |                          |
| 2080  | $E$               | 147        | 3.2      | 4906.433206(4)             |                          |
| 2081  | $E$               | 147        | 3.2      | 4906.433207(5)             |                          |
| 2082  | $A_2$             | 104        | 3.1      | 4906.54000(1)              |                          |
| 2083  | $A_1$             | 105        | 3.1      | 4906.54000(1)              |                          |
| 2084  | $A_1$             | 143        | 1.0      | 4906.702890(2)             |                          |
| 2085  | $E$               | 160        | 2.2      | 4906.915598(2)             |                          |
| 2086  | $E$               | 113        | 2.2      | 4906.91560(2)              |                          |
| 2087  | $E$               | 174        | 2.4      | 4909.895449(3)             |                          |
| 2088  | $E$               | 134        | 2.4      | 4909.895452(9)             |                          |
| 2089  | $E$               | 166        | 3.4      | 4910.459489(4)             |                          |
| 2090  | $E$               | 150        | 3.4      | 4910.459493(8)             |                          |
| 2091  | $A_2$             | 155        | 3.8      | 4910.547300(6)             |                          |
| 2092  | $A_2$             | 132        | 2.6      | 4910.70530(1)              |                          |
| 2093  | $A_1$             | 156        | 2.6      | 4910.716325(5)             |                          |
| 2094  | $A_1$             | 147        | 3.3      | 4910.764011(5)             |                          |
| 2095  | $E$               | 137        | 3.2      | 4910.824227(9)             |                          |
| 2096  | $E$               | 149        | 3.2      | 4910.824228(9)             |                          |
| 2097  | $E$               | 158        | 2.3      | 4911.205417(2)             |                          |
| 2098  | $E$               | 160        | 2.3      | 4911.205417(2)             |                          |
| 2099  | $A_2$             | 141        | 3.2      | 4911.568225(9)             |                          |
| 2100  | $E$               | 159        | 3.3      | 4911.839035(3)             |                          |
| 2101  | $E$               | 163        | 3.3      | 4911.839036(3)             |                          |
| 2102  | $E$               | 149        | 2.5      | 4911.918123(2)             |                          |
| 2103  | $E$               | 114        | 2.5      | 4911.91812(1)              |                          |
| 2104  | $E$               | 111        | 2.4      | 4912.11067(1)              |                          |
| 2105  | $E$               | 102        | 2.4      | 4912.11067(1)              |                          |
| 2106  | $E$               | 130        | 2.4      | 4912.262489(2)             |                          |
| 2107  | $E$               | 122        | 2.4      | 4912.262491(4)             |                          |
| 2108  | $A_1$             | 108        | 2.3      | 4912.642801(7)             |                          |
| 2109  | $E$               | 166        | 3.1      | 4912.938713(4)             |                          |

Continued on next page.

TABLE S4 – states on Sarka/Poirier CSC PES; continued from previous page

| State | $\Gamma_{C_{3v}}$ | $D_{\max}$ | $S_{vN}$ | $\tilde{E}/\text{cm}^{-1}$ | $\Delta\text{Ref. [30]}$ |
|-------|-------------------|------------|----------|----------------------------|--------------------------|
| 2110  | $E$               | 159        | 3.2      | 4912.938714(4)             |                          |
| 2111  | $E$               | 143        | 2.7      | 4913.080283(4)             |                          |
| 2112  | $E$               | 162        | 2.6      | 4913.080287(6)             |                          |
| 2113  | $A_1$             | 81         | 2.6      | 4918.77797(9)              |                          |
| 2114  | $A_2$             | 82         | 2.6      | 4918.77798(8)              |                          |
| 2115  | $E$               | 109        | 2.6      | 4918.93001(1)              |                          |
| 2116  | $E$               | 109        | 2.6      | 4918.93001(1)              |                          |
| 2117  | $E$               | 107        | 2.7      | 4922.86537(1)              |                          |
| 2118  | $E$               | 103        | 2.7      | 4922.86537(1)              |                          |
| 2119  | $A_1$             | 94         | 2.6      | 4923.01879(1)              |                          |
| 2120  | $A_2$             | 79         | 2.6      | 4923.01915(6)              |                          |
| 2121  | $E$               | 96         | 0.99     | 4924.40723(1)              |                          |
| 2122  | $E$               | 89         | 0.97     | 4924.40723(1)              |                          |
| 2123  | $E$               | 153        | 2.4      | 4927.298279(3)             |                          |
| 2124  | $E$               | 144        | 2.4      | 4927.298279(4)             |                          |
| 2125  | $A_2$             | 109        | 2.1      | 4927.47676(1)              |                          |
| 2126  | $A_1$             | 110        | 2.1      | 4927.47677(2)              |                          |
| 2127  | $E$               | 111        | 0.23     | 4928.846491(9)             |                          |
| 2128  | $E$               | 127        | 0.24     | 4928.846492(9)             |                          |
| 2129  | $E$               | 103        | 0.65     | 4929.098391(2)             |                          |
| 2130  | $E$               | 110        | 0.65     | 4929.098392(2)             |                          |
| 2131  | $E$               | 99         | 2.2      | 4932.37527(2)              |                          |
| 2132  | $E$               | 100        | 2.2      | 4932.37527(1)              |                          |
| 2133  | $E$               | 104        | 2.2      | 4932.50593(1)              |                          |
| 2134  | $E$               | 115        | 2.2      | 4932.50594(1)              |                          |
| 2135  | $A_1$             | 103        | 2.3      | 4935.16884(1)              |                          |
| 2136  | $E$               | 129        | 2.2      | 4935.383122(3)             |                          |
| 2137  | $E$               | 129        | 2.2      | 4935.383123(3)             |                          |
| 2138  | $A_2$             | 98         | 2.2      | 4935.501052(9)             |                          |
| 2139  | $E$               | 112        | 2.1      | 4936.219133(1)             |                          |
| 2140  | $E$               | 103        | 2.1      | 4936.219134(2)             |                          |
| 2141  | $A_2$             | 67         | 2.0      | 4936.55089(2)              |                          |
| 2142  | $A_1$             | 69         | 2.1      | 4936.56946(1)              |                          |
| 2143  | $E$               | 103        | 0.1      | 4939.010714(2)             |                          |
| 2144  | $E$               | 104        | 0.1      | 4939.010714(2)             |                          |
| 2145  | $E$               | 59         | 1.8      | 4939.51411(1)              |                          |
| 2146  | $E$               | 56         | 1.8      | 4939.51412(1)              |                          |
| 2147  | $E$               | 62         | 2.1      | 4948.24546(9)              |                          |
| 2148  | $E$               | 62         | 2.1      | 4948.24546(9)              |                          |
| 2149  | $A_1$             | 65         | 2.1      | 4948.25225(7)              |                          |
| 2150  | $A_2$             | 68         | 2.1      | 4948.25251(3)              |                          |
| 2151  | $A_1$             | 105        | 0.1      | 4949.935872(1)             |                          |
| 2152  | $A_2$             | 87         | 0.083    | 4950.108755(3)             |                          |
| 2153  | $A_1$             | 71         | 2.8      | 4950.467548(1)             |                          |
| 2154  | $E$               | 84         | 1.8      | 4953.126725(3)             |                          |
| 2155  | $E$               | 83         | 1.8      | 4953.126725(2)             |                          |
| 2156  | $E$               | 116        | 2.6      | 4955.184865(2)             |                          |
| 2157  | $E$               | 93         | 2.6      | 4955.18487(1)              |                          |
| 2158  | $A_1$             | 111        | 2.5      | 4955.233439(4)             |                          |
| 2159  | $A_2$             | 113        | 2.5      | 4955.233489(3)             |                          |
| 2160  | $E$               | 79         | 0.56     | 4956.682101(3)             |                          |
| 2161  | $E$               | 76         | 0.57     | 4956.682101(6)             |                          |
| 2162  | $E$               | 129        | 0.56     | 4958.219379(9)             |                          |
| 2163  | $E$               | 125        | 0.56     | 4958.21938(1)              |                          |
| 2164  | $E$               | 84         | 0.55     | 4958.802430(1)             |                          |
| 2165  | $E$               | 82         | 0.55     | 4958.802431(1)             |                          |
| 2166  | $A_1$             | 53         | 3.0      | 4959.154249(6)             |                          |
| 2167  | $E$               | 117        | 1.2      | 4962.48783(4)              |                          |
| 2168  | $E$               | 179        | 1.2      | 4962.48783(5)              |                          |

Continued on next page.

TABLE S4 – states on Sarka/Poirier CSC PES; continued from previous page

| State | $\Gamma_{C_{3v}}$ | $D_{\max}$ | $S_{vN}$ | $\tilde{E}/\text{cm}^{-1}$ | $\Delta\text{Ref. [30]}$ |
|-------|-------------------|------------|----------|----------------------------|--------------------------|
| 2169  | $E$               | 132        | 2.9      | 4963.61245(1)              |                          |
| 2170  | $E$               | 137        | 2.9      | 4963.612447(6)             |                          |
| 2171  | $A_1$             | 117        | 2.5      | 4963.82818(1)              |                          |
| 2172  | $A_2$             | 112        | 2.5      | 4963.82818(2)              |                          |
| 2173  | $A_1$             | 128        | 0.7      | 4963.95123(1)              |                          |
| 2174  | $E$               | 104        | 2.1      | 4963.987867(3)             |                          |
| 2175  | $E$               | 98         | 2.1      | 4963.987867(3)             |                          |
| 2176  | $A_2$             | 113        | 3.2      | 4964.455414(5)             |                          |
| 2177  | $A_1$             | 122        | 3.1      | 4964.458396(2)             |                          |
| 2178  | $E$               | 105        | 3.0      | 4964.501481(3)             |                          |
| 2179  | $E$               | 105        | 3.0      | 4964.501481(5)             |                          |
| 2180  | $E$               | 99         | 2.1      | 4965.020508(2)             |                          |
| 2181  | $E$               | 103        | 2.1      | 4965.020511(5)             |                          |
| 2182  | $E$               | 118        | 2.1      | 4965.175435(3)             |                          |
| 2183  | $E$               | 100        | 2.1      | 4965.175436(9)             |                          |
| 2184  | $A_1^*$           | 83         | 2.1      | 4965.20666(1)              |                          |
| 2185  | $A_2^*$           | 84         | 2.1      | 4965.20666(1)              |                          |
| 2186  | $A_2$             | 101        | 2.1      | 4965.465501(3)             |                          |
| 2187  | $E$               | 100        | 2.1      | 4965.956470(4)             |                          |
| 2188  | $E$               | 114        | 2.1      | 4965.956471(5)             |                          |
| 2189  | $A_1$             | 101        | 2.1      | 4966.496560(4)             |                          |
| 2190  | $A_1$             | 74         | 2.4      | 4966.640878(2)             |                          |
| 2191  | $E$               | 84         | 2.2      | 4966.715424(2)             |                          |
| 2192  | $E$               | 89         | 2.2      | 4966.715426(3)             |                          |
| 2193  | $A_2$             | 69         | 2.2      | 4966.759508(2)             |                          |
| 2194  | $A_2$             | 129        | 2.5      | 4967.95434(1)              |                          |
| 2195  | $A_1$             | 146        | 2.6      | 4967.99508(1)              |                          |
| 2196  | $E$               | 141        | 2.4      | 4968.09501(1)              |                          |
| 2197  | $E$               | 142        | 2.4      | 4968.09501(1)              |                          |
| 2198  | $E$               | 124        | 0.48     | 4969.476020(5)             |                          |
| 2199  | $E$               | 152        | 0.48     | 4969.476021(5)             |                          |
| 2200  | $A_2$             | 86         | 0.5      | 4969.87394(1)              |                          |
| 2201  | $A_1$             | 87         | 0.5      | 4969.87395(1)              |                          |
| 2202  | $E$               | 109        | 0.63     | 4972.753204(7)             |                          |
| 2203  | $E$               | 111        | 0.63     | 4972.753205(5)             |                          |
| 2204  | $E$               | 158        | 2.4      | 4972.784821(4)             |                          |
| 2205  | $E$               | 166        | 2.4      | 4972.784821(4)             |                          |
| 2206  | $A_2$             | 147        | 2.4      | 4972.959251(3)             |                          |
| 2207  | $A_1$             | 165        | 2.4      | 4972.959252(3)             |                          |
| 2208  | $E$               | 96         | 2.3      | 4973.49770(1)              |                          |
| 2209  | $E$               | 90         | 2.3      | 4973.49771(2)              |                          |
| 2210  | $A_2^*$           | 89         | 2.3      | 4973.49980(2)              |                          |
| 2211  | $A_1^*$           | 89         | 2.3      | 4973.49981(1)              |                          |
| 2212  | $E$               | 131        | 2.1      | 4976.865066(3)             |                          |
| 2213  | $E$               | 103        | 2.1      | 4976.865072(8)             |                          |
| 2214  | $E$               | 114        | 2.2      | 4976.909784(4)             |                          |
| 2215  | $E$               | 137        | 2.2      | 4976.909787(5)             |                          |
| 2216  | $E$               | 116        | 2.8      | 4978.336182(9)             |                          |
| 2217  | $E$               | 111        | 2.8      | 4978.33618(2)              |                          |
| 2218  | $A_1$             | 82         | 2.7      | 4978.41253(7)              |                          |
| 2219  | $A_2$             | 88         | 2.7      | 4978.41260(4)              |                          |
| 2220  | $E$               | 154        | 2.4      | 4978.424103(5)             |                          |
| 2221  | $E$               | 158        | 2.4      | 4978.424105(6)             |                          |
| 2222  | $E$               | 152        | 2.4      | 4978.590826(3)             |                          |
| 2223  | $E$               | 152        | 2.4      | 4978.590826(3)             |                          |
| 2224  | $E$               | 75         | 0.2      | 4978.766497(2)             |                          |
| 2225  | $E$               | 86         | 0.2      | 4978.766497(2)             |                          |
| 2226  | $E$               | 112        | 2.5      | 4979.00212(1)              |                          |
| 2227  | $E$               | 132        | 2.5      | 4979.00212(1)              |                          |

Continued on next page.

TABLE S4 – states on Sarka/Poirier CSC PES; continued from previous page

| State | $\Gamma_{C_{3v}}$ | $D_{\max}$ | $S_{vN}$ | $\tilde{E}/\text{cm}^{-1}$ | $\Delta\text{Ref. [30]}$ |
|-------|-------------------|------------|----------|----------------------------|--------------------------|
| 2228  | $E$               | 161        | 2.4      | 4979.060854(2)             |                          |
| 2229  | $E$               | 109        | 2.4      | 4979.06086(1)              |                          |
| 2230  | $A_2$             | 115        | 2.2      | 4979.779861(4)             |                          |
| 2231  | $A_1$             | 90         | 2.2      | 4979.78076(1)              |                          |
| 2232  | $E$               | 88         | 2.2      | 4979.79633(1)              |                          |
| 2233  | $E$               | 90         | 2.2      | 4979.79633(1)              |                          |
| 2234  | $E$               | 93         | 0.85     | 4979.85757(1)              |                          |
| 2235  | $E$               | 94         | 0.84     | 4979.85757(1)              |                          |
| 2236  | $A_1$             | 136        | 2.5      | 4980.928752(9)             |                          |
| 2237  | $E$               | 141        | 2.3      | 4981.41647(1)              |                          |
| 2238  | $E$               | 162        | 2.3      | 4981.41648(1)              |                          |
| 2239  | $A_2$             | 109        | 2.5      | 4981.421813(8)             |                          |
| 2240  | $A_2$             | 145        | 2.3      | 4981.737307(3)             |                          |
| 2241  | $E$               | 109        | 2.5      | 4981.869928(6)             |                          |
| 2242  | $E$               | 110        | 2.5      | 4981.869928(6)             |                          |
| 2243  | $A_1$             | 103        | 2.5      | 4982.222624(4)             |                          |
| 2244  | $E$               | 128        | 0.66     | 4983.431256(2)             |                          |
| 2245  | $E$               | 131        | 0.66     | 4983.431257(2)             |                          |
| 2246  | $E$               | 143        | 2.2      | 4983.634253(4)             |                          |
| 2247  | $E$               | 143        | 2.2      | 4983.634253(5)             |                          |
| 2248  | $E$               | 142        | 1.9      | 4984.068409(3)             |                          |
| 2249  | $E$               | 122        | 1.9      | 4984.068413(9)             |                          |
| 2250  | $A_1$             | 95         | 0.43     | 4987.75731(1)              |                          |
| 2251  | $A_2$             | 89         | 0.43     | 4987.75732(3)              |                          |
| 2252  | $E$               | 69         | 0.075    | 4988.071956(2)             |                          |
| 2253  | $E$               | 64         | 0.075    | 4988.071956(1)             |                          |
| 2254  | $E$               | 140        | 2.7      | 4988.957187(3)             |                          |
| 2255  | $E$               | 133        | 2.7      | 4988.957188(3)             |                          |
| 2256  | $A_1$             | 101        | 2.7      | 4989.27670(2)              |                          |
| 2257  | $A_2$             | 94         | 2.7      | 4989.28469(2)              |                          |
| 2258  | $A_1$             | 118        | 1.9      | 4989.37515(2)              |                          |
| 2259  | $A_2$             | 136        | 1.8      | 4989.376421(7)             |                          |
| 2260  | $A_1$             | 107        | 1.7      | 4989.66842(4)              |                          |
| 2261  | $A_2$             | 127        | 1.7      | 4989.668499(9)             |                          |
| 2262  | $A_2$             | 58         | 0.13     | 4989.75870(1)              |                          |
| 2263  | $A_1$             | 58         | 0.13     | 4989.75870(1)              |                          |
| 2264  | $E$               | 112        | 0.56     | 4990.61434(2)              |                          |
| 2265  | $E$               | 145        | 0.56     | 4990.61434(2)              |                          |
| 2266  | $E$               | 150        | 2.6      | 4991.018828(3)             |                          |
| 2267  | $E$               | 155        | 2.6      | 4991.018829(2)             |                          |
| 2268  | $A_1^*$           | 62         | 0.57     | 4991.99031(4)              |                          |
| 2269  | $A_2^*$           | 59         | 0.57     | 4991.99031(5)              |                          |
| 2270  | $E$               | 164        | 0.87     | 4992.266039(2)             |                          |
| 2271  | $E$               | 112        | 0.88     | 4992.26605(1)              |                          |
| 2272  | $E$               | 152        | 3.3      | 4992.416573(6)             |                          |
| 2273  | $E$               | 158        | 3.3      | 4992.416573(6)             |                          |
| 2274  | $E$               | 134        | 0.85     | 4992.449672(3)             |                          |
| 2275  | $E$               | 131        | 0.88     | 4992.449672(3)             |                          |
| 2276  | $A_1$             | 147        | 3.7      | 4992.460385(9)             |                          |
| 2277  | $A_2$             | 171        | 3.7      | 4992.461204(3)             |                          |
| 2278  | $E$               | 128        | 2.4      | 4993.12025(1)              |                          |
| 2279  | $E$               | 133        | 2.4      | 4993.120248(5)             |                          |
| 2280  | $E$               | 111        | 2.2      | 4993.255545(9)             |                          |
| 2281  | $E$               | 129        | 2.2      | 4993.25555(1)              |                          |
| 2282  | $E$               | 124        | 2.4      | 4993.590470(6)             |                          |
| 2283  | $E$               | 138        | 2.4      | 4993.590471(6)             |                          |
| 2284  | $E$               | 96         | 2.4      | 4996.04299(2)              |                          |
| 2285  | $E$               | 91         | 2.4      | 4996.04299(3)              |                          |
| 2286  | $A_1$             | 98         | 2.4      | 4996.08511(2)              |                          |

Continued on next page.



TABLE S4 – states on Sarka/Poirier CSC PES; continued from previous page

| State | $\Gamma_{C_{3v}}$ | $D_{\max}$ | $S_{vN}$ | $\tilde{E}/\text{cm}^{-1}$ | $\Delta\text{Ref. [30]}$ |
|-------|-------------------|------------|----------|----------------------------|--------------------------|
| 2287  | $A_2$             | 95         | 2.3      | 4996.09263(2)              |                          |
| 2288  | $E$               | 85         | 0.18     | 4996.799273(3)             |                          |
| 2289  | $E$               | 106        | 0.18     | 4996.799274(2)             |                          |
| 2290  | $E$               | 70         | 0.21     | 5001.024760(7)             |                          |
| 2291  | $E$               | 79         | 0.21     | 5001.024760(6)             |                          |
| 2292  | $A_1$             | 85         | 0.28     | 5002.433068(2)             |                          |
| 2293  | $E$               | 109        | 2.1      | 5002.570950(5)             |                          |
| 2294  | $E$               | 84         | 2.1      | 5002.57096(5)              |                          |
| 2295  | $A_2$             | 102        | 2.1      | 5002.57623(1)              |                          |
| 2296  | $A_1$             | 96         | 2.2      | 5002.57659(2)              |                          |
| 2297  | $E$               | 82         | 0.79     | 5002.576720(7)             |                          |
| 2298  | $E$               | 92         | 0.79     | 5002.576721(3)             |                          |
| 2299  | $A_1$             | 67         | 0.49     | 5002.764718(4)             |                          |
| 2300  | $A_2$             | 65         | 0.49     | 5002.764721(3)             |                          |
| 2301  | $E$               | 160        | 3.2      | 5003.139582(3)             |                          |
| 2302  | $E$               | 155        | 3.2      | 5003.139582(4)             |                          |
| 2303  | $A_2$             | 110        | 3.0      | 5003.16882(3)              |                          |
| 2304  | $A_1$             | 151        | 3.2      | 5003.219869(4)             |                          |
| 2305  | $A_1$             | 156        | 3.2      | 5003.742262(3)             |                          |
| 2306  | $A_2$             | 104        | 2.9      | 5003.79484(4)              |                          |
| 2307  | $E$               | 124        | 3.0      | 5003.81420(1)              |                          |
| 2308  | $E$               | 109        | 3.0      | 5003.81420(2)              |                          |
| 2309  | $E$               | 93         | 0.21     | 5004.066959(2)             |                          |
| 2310  | $E$               | 95         | 0.22     | 5004.066960(3)             |                          |
| 2311  | $E$               | 79         | 0.48     | 5004.833900(1)             |                          |
| 2312  | $E$               | 74         | 0.48     | 5004.833901(2)             |                          |
| 2313  | $E$               | 82         | 0.56     | 5005.663564(4)             |                          |
| 2314  | $E$               | 91         | 0.56     | 5005.663564(3)             |                          |
| 2315  | $E$               | 91         | 0.39     | 5008.575211(1)             |                          |
| 2316  | $E$               | 91         | 0.39     | 5008.575211(1)             |                          |
| 2317  | $A_1$             | 91         | 0.6      | 5010.5078579(9)            |                          |
| 2318  | $A_2$             | 86         | 0.6      | 5010.507869(1)             |                          |
| 2319  | $E$               | 87         | 0.94     | 5010.520833(2)             |                          |
| 2320  | $E$               | 85         | 0.94     | 5010.520835(5)             |                          |
| 2321  | $E$               | 86         | 0.73     | 5012.787985(2)             |                          |
| 2322  | $E$               | 84         | 0.73     | 5012.787985(2)             |                          |
| 2323  | $E$               | 83         | 0.65     | 5013.345508(1)             |                          |
| 2324  | $E$               | 84         | 0.65     | 5013.345508(1)             |                          |
| 2325  | $A_1$             | 86         | 0.82     | 5014.192575(2)             |                          |
| 2326  | $A_1$             | 60         | 1.0      | 5015.81891(4)              |                          |
| 2327  | $A_2$             | 59         | 1.0      | 5015.81903(6)              |                          |
| 2328  | $A_2^*$           | 109        | 2.0      | 5017.437499(2)             |                          |
| 2329  | $A_1^*$           | 108        | 2.0      | 5017.437499(2)             |                          |
| 2330  | $E$               | 112        | 2.0      | 5017.465637(2)             |                          |
| 2331  | $E$               | 71         | 2.0      | 5017.46564(1)              |                          |
| 2332  | $E$               | 82         | 1.1      | 5018.468636(4)             |                          |
| 2333  | $E$               | 81         | 1.1      | 5018.468637(3)             |                          |
| 2334  | $E$               | 75         | 2.1      | 5023.130553(4)             |                          |
| 2335  | $E$               | 75         | 2.1      | 5023.130553(4)             |                          |
| 2336  | $E$               | 78         | 2.1      | 5023.147470(4)             |                          |
| 2337  | $E$               | 94         | 2.1      | 5023.147470(3)             |                          |
| 2338  | $A_1$             | 66         | 2.1      | 5025.97878(5)              |                          |
| 2339  | $E$               | 68         | 2.1      | 5025.98053(5)              |                          |
| 2340  | $E$               | 68         | 2.1      | 5025.98053(5)              |                          |
| 2341  | $A_2$             | 68         | 2.1      | 5025.99355(4)              |                          |
| 2342  | $A_2$             | 114        | 2.3      | 5026.277711(7)             |                          |
| 2343  | $A_1$             | 135        | 2.3      | 5026.277711(7)             |                          |
| 2344  | $E$               | 131        | 2.2      | 5026.533851(3)             |                          |
| 2345  | $E$               | 97         | 2.2      | 5026.53386(1)              |                          |

Continued on next page.

TABLE S4 – states on Sarka/Poirier CSC PES; continued from previous page

| State | $\Gamma_{C_{3v}}$ | $D_{\max}$ | $S_{vN}$ | $\tilde{E}/\text{cm}^{-1}$ | $\Delta\text{Ref. [30]}$ |
|-------|-------------------|------------|----------|----------------------------|--------------------------|
| 2346  | $A_2$             | 94         | 2.4      | 5026.772774(1)             |                          |
| 2347  | $E$               | 95         | 2.4      | 5026.871999(3)             |                          |
| 2348  | $E$               | 89         | 2.4      | 5026.872001(2)             |                          |
| 2349  | $A_1$             | 92         | 2.4      | 5026.981131(3)             |                          |
| 2350  | $E$               | 77         | 0.68     | 5028.055533(4)             |                          |
| 2351  | $E$               | 93         | 0.68     | 5028.055533(4)             |                          |
| 2352  | $A_2$             | 111        | 2.3      | 5032.82626(3)              |                          |
| 2353  | $A_1$             | 105        | 2.3      | 5032.82626(4)              |                          |
| 2354  | $E$               | 191        | 3.4      | 5033.641269(5)             |                          |
| 2355  | $E$               | 174        | 3.4      | 5033.641269(8)             |                          |
| 2356  | $A_1$             | 59         | 0.88     | 5033.70214(4)              |                          |
| 2357  | $A_2$             | 60         | 0.88     | 5033.70215(5)              |                          |
| 2358  | $E$               | 131        | 3.2      | 5033.758834(5)             |                          |
| 2359  | $E$               | 157        | 3.2      | 5033.75884(1)              |                          |
| 2360  | $A_2$             | 142        | 2.3      | 5034.115229(5)             |                          |
| 2361  | $A_1$             | 141        | 2.3      | 5034.115230(5)             |                          |
| 2362  | $E$               | 95         | 2.1      | 5034.287656(1)             |                          |
| 2363  | $E$               | 99         | 2.1      | 5034.287656(1)             |                          |
| 2364  | $E$               | 115        | 2.4      | 5034.66086(2)              |                          |
| 2365  | $E$               | 108        | 2.4      | 5034.66087(3)              |                          |
| 2366  | $A_1$             | 86         | 2.3      | 5034.85860(7)              |                          |
| 2367  | $A_2$             | 90         | 2.3      | 5034.85860(8)              |                          |
| 2368  | $A_1$             | 73         | 3.0      | 5034.92851(1)              |                          |
| 2369  | $A_2$             | 70         | 3.0      | 5034.92946(1)              |                          |
| 2370  | $E$               | 73         | 3.0      | 5034.942775(7)             |                          |
| 2371  | $E$               | 83         | 3.0      | 5034.94278(1)              |                          |
| 2372  | $E$               | 97         | 2.1      | 5035.679332(2)             |                          |
| 2373  | $E$               | 97         | 2.0      | 5035.679332(1)             |                          |
| 2374  | $E$               | 152        | 2.4      | 5035.70545(1)              |                          |
| 2375  | $E$               | 149        | 2.4      | 5035.705455(3)             |                          |
| 2376  | $E$               | 90         | 0.96     | 5036.526116(2)             |                          |
| 2377  | $E$               | 96         | 0.96     | 5036.526116(2)             |                          |
| 2378  | $A_1$             | 128        | 3.3      | 5036.65333(1)              |                          |
| 2379  | $A_2$             | 148        | 3.3      | 5036.655358(3)             |                          |
| 2380  | $E$               | 110        | 3.0      | 5036.68018(2)              |                          |
| 2381  | $E$               | 116        | 3.0      | 5036.68018(3)              |                          |
| 2382  | $E$               | 132        | 2.3      | 5037.029135(6)             |                          |
| 2383  | $E$               | 137        | 2.3      | 5037.029138(7)             |                          |
| 2384  | $E$               | 104        | 2.4      | 5040.24960(3)              |                          |
| 2385  | $E$               | 120        | 2.4      | 5040.24960(3)              |                          |
| 2386  | $E$               | 133        | 2.3      | 5040.402283(7)             |                          |
| 2387  | $E$               | 105        | 2.3      | 5040.40228(2)              |                          |
| 2388  | $A_1$             | 110        | 2.4      | 5042.79117(1)              |                          |
| 2389  | $E$               | 144        | 2.3      | 5043.171596(2)             |                          |
| 2390  | $E$               | 99         | 2.3      | 5043.17160(1)              |                          |
| 2391  | $A_2$             | 152        | 2.3      | 5043.416420(2)             |                          |
| 2392  | $E$               | 75         | 0.17     | 5044.693209(2)             |                          |
| 2393  | $E$               | 50         | 0.17     | 5044.693211(3)             |                          |
| 2394  | $E$               | 111        | 0.28     | 5046.353583(8)             |                          |
| 2395  | $E$               | 134        | 0.28     | 5046.353584(7)             |                          |
| 2396  | $A_1^*$           | 119        | 2.5      | 5047.83151(4)              |                          |
| 2397  | $A_2^*$           | 126        | 2.5      | 5047.83151(4)              |                          |
| 2398  | $E$               | 119        | 2.4      | 5047.83153(5)              |                          |
| 2399  | $E$               | 123        | 2.4      | 5047.83153(5)              |                          |
| 2400  | $E$               | 101        | 2.3      | 5048.21600(1)              |                          |
| 2401  | $E$               | 99         | 2.3      | 5048.21600(1)              |                          |
| 2402  | $E$               | 102        | 2.2      | 5048.38928(1)              |                          |
| 2403  | $E$               | 90         | 2.2      | 5048.389282(7)             |                          |
| 2404  | $A_2^*$           | 104        | 2.3      | 5051.53885(1)              |                          |

Continued on next page.

TABLE S4 – states on Sarka/Poirier CSC PES; continued from previous page

| State | $\Gamma_{C_{3v}}$ | $D_{\max}$ | $S_{vN}$ | $\tilde{E}/\text{cm}^{-1}$ | $\Delta\text{Ref. [30]}$ |
|-------|-------------------|------------|----------|----------------------------|--------------------------|
| 2405  | $A_1^*$           | 102        | 2.3      | 5051.53885(1)              |                          |
| 2406  | $E$               | 100        | 2.1      | 5052.030282(6)             |                          |
| 2407  | $E$               | 128        | 2.1      | 5052.03029(1)              |                          |
| 2408  | $E$               | 201        | 2.8      | 5052.039883(6)             |                          |
| 2409  | $E$               | 185        | 2.8      | 5052.039887(6)             |                          |
| 2410  | $A_1$             | 137        | 2.7      | 5052.12367(5)              |                          |
| 2411  | $A_2$             | 135        | 2.7      | 5052.12391(5)              |                          |
| 2412  | $A_2$             | 104        | 2.5      | 5052.19708(1)              |                          |
| 2413  | $E$               | 107        | 2.5      | 5052.297156(4)             |                          |
| 2414  | $E$               | 109        | 2.5      | 5052.297159(6)             |                          |
| 2415  | $A_1$             | 100        | 2.5      | 5052.407195(2)             |                          |
| 2416  | $A_1$             | 191        | 3.5      | 5053.262633(6)             |                          |
| 2417  | $A_2$             | 187        | 3.5      | 5053.262635(3)             |                          |
| 2418  | $E$               | 168        | 3.3      | 5053.472967(4)             |                          |
| 2419  | $E$               | 161        | 3.3      | 5053.472968(8)             |                          |
| 2420  | $E$               | 161        | 4.3      | 5053.56458(1)              |                          |
| 2421  | $E$               | 188        | 4.3      | 5053.56458(1)              |                          |
| 2422  | $E$               | 184        | 3.8      | 5053.646042(6)             |                          |
| 2423  | $E$               | 200        | 3.8      | 5053.64605(1)              |                          |
| 2424  | $E$               | 170        | 3.1      | 5053.769337(5)             |                          |
| 2425  | $E$               | 170        | 3.1      | 5053.769338(5)             |                          |
| 2426  | $A_1$             | 117        | 2.6      | 5055.19075(1)              |                          |
| 2427  | $A_2$             | 156        | 2.6      | 5055.190753(6)             |                          |
| 2428  | $E$               | 166        | 2.5      | 5055.320999(2)             |                          |
| 2429  | $E$               | 107        | 2.5      | 5055.32100(1)              |                          |
| 2430  | $A_1^*$           | 141        | 0.41     | 5055.980764(5)             |                          |
| 2431  | $A_2^*$           | 129        | 0.41     | 5055.98076(1)              |                          |
| 2432  | $E$               | 177        | 3.4      | 5057.614964(5)             |                          |
| 2433  | $E$               | 169        | 3.4      | 5057.614965(6)             |                          |
| 2434  | $A_2$             | 142        | 3.4      | 5057.70092(2)              |                          |
| 2435  | $A_1$             | 145        | 3.4      | 5057.70296(1)              |                          |
| 2436  | $E$               | 182        | 3.4      | 5057.905575(4)             |                          |
| 2437  | $E$               | 172        | 3.4      | 5057.905579(6)             |                          |
| 2438  | $E$               | 170        | 3.2      | 5058.033249(4)             |                          |
| 2439  | $E$               | 166        | 3.2      | 5058.033249(5)             |                          |
| 2440  | $E$               | 156        | 2.5      | 5059.141015(8)             |                          |
| 2441  | $E$               | 166        | 2.5      | 5059.141016(4)             |                          |
| 2442  | $A_1$             | 55         | 1.9      | 5059.2948454(6)            |                          |
| 2443  | $E$               | 154        | 2.7      | 5059.363031(2)             |                          |
| 2444  | $E$               | 136        | 2.7      | 5059.363031(4)             |                          |
| 2445  | $A_1$             | 130        | 2.3      | 5059.43680(1)              |                          |
| 2446  | $A_2$             | 131        | 2.3      | 5059.44473(1)              |                          |
| 2447  | $A_1$             | 153        | 2.7      | 5059.474853(2)             |                          |
| 2448  | $A_2$             | 144        | 2.7      | 5059.475114(3)             |                          |
| 2449  | $E$               | 85         | 0.92     | 5060.86860(1)              |                          |
| 2450  | $E$               | 98         | 0.93     | 5060.86860(1)              |                          |
| 2451  | $E$               | 136        | 2.8      | 5061.14782(1)              |                          |
| 2452  | $E$               | 174        | 2.8      | 5061.14783(1)              |                          |
| 2453  | $E$               | 166        | 2.2      | 5061.596119(2)             |                          |
| 2454  | $E$               | 128        | 2.2      | 5061.596121(9)             |                          |
| 2455  | $E$               | 117        | 0.99     | 5062.91089(2)              |                          |
| 2456  | $E$               | 179        | 0.99     | 5062.91090(2)              |                          |
| 2457  | $E$               | 128        | 2.2      | 5066.032278(7)             |                          |
| 2458  | $E$               | 128        | 2.2      | 5066.032278(7)             |                          |
| 2459  | $E$               | 137        | 1.5      | 5066.80285(1)              |                          |
| 2460  | $E$               | 127        | 1.5      | 5066.80285(1)              |                          |
| 2461  | $A_2$             | 139        | 3.6      | 5066.818814(4)             |                          |
| 2462  | $A_1$             | 143        | 3.2      | 5066.901214(6)             |                          |
| 2463  | $E$               | 133        | 3.1      | 5066.941083(8)             |                          |

Continued on next page.

TABLE S4 – states on Sarka/Poirier CSC PES; continued from previous page

| State | $\Gamma_{C_{3v}}$ | $D_{\max}$ | $S_{vN}$ | $\tilde{E}/\text{cm}^{-1}$ | $\Delta\text{Ref. [30]}$ |
|-------|-------------------|------------|----------|----------------------------|--------------------------|
| 2464  | $E$               | 134        | 3.1      | 5066.941084(4)             |                          |
| 2465  | $E$               | 117        | 2.2      | 5067.342102(6)             |                          |
| 2466  | $E$               | 128        | 2.2      | 5067.342106(8)             |                          |
| 2467  | $A_2$             | 137        | 2.8      | 5067.587758(2)             |                          |
| 2468  | $A_1$             | 105        | 0.92     | 5067.928900(4)             |                          |
| 2469  | $A_1$             | 158        | 0.75     | 5068.242712(2)             |                          |
| 2470  | $E$               | 114        | 3.0      | 5068.30054(5)              |                          |
| 2471  | $E$               | 153        | 3.0      | 5068.30055(5)              |                          |
| 2472  | $E$               | 113        | 2.3      | 5068.39462(1)              |                          |
| 2473  | $E$               | 115        | 2.3      | 5068.39463(1)              |                          |
| 2474  | $A_2$             | 119        | 2.3      | 5068.41643(2)              |                          |
| 2475  | $A_1$             | 131        | 2.3      | 5068.41645(1)              |                          |
| 2476  | $A_1$             | 120        | 2.2      | 5068.803655(2)             |                          |
| 2477  | $A_1$             | 55         | 1.9      | 5069.971564(1)             |                          |
| 2478  | $A_2$             | 113        | 2.3      | 5072.35022(3)              |                          |
| 2479  | $A_1$             | 153        | 2.6      | 5072.450195(4)             |                          |
| 2480  | $E$               | 122        | 2.3      | 5072.48938(1)              |                          |
| 2481  | $E$               | 124        | 2.3      | 5072.48938(1)              |                          |
| 2482  | $E$               | 120        | 2.0      | 5073.005825(1)             |                          |
| 2483  | $E$               | 121        | 2.0      | 5073.005825(2)             |                          |
| 2484  | $E$               | 102        | 0.4      | 5073.81559(1)              |                          |
| 2485  | $E$               | 108        | 0.4      | 5073.81559(1)              |                          |
| 2486  | $E$               | 109        | 1.7      | 5076.100454(3)             |                          |
| 2487  | $E$               | 122        | 1.7      | 5076.100454(3)             |                          |
| 2488  | $A_2$             | 95         | 2.1      | 5080.468119(4)             |                          |
| 2489  | $A_1$             | 117        | 2.4      | 5080.707023(2)             |                          |
| 2490  | $A_1$             | 98         | 0.11     | 5081.072807(5)             |                          |
| 2491  | $E$               | 99         | 2.0      | 5081.388992(4)             |                          |
| 2492  | $E$               | 91         | 2.0      | 5081.388993(6)             |                          |
| 2493  | $E$               | 114        | 0.097    | 5086.633622(2)             |                          |
| 2494  | $E$               | 113        | 0.097    | 5086.633622(2)             |                          |
| 2495  | $A_1$             | 111        | 2.8      | 5086.742210(5)             |                          |
| 2496  | $E$               | 81         | 2.7      | 5086.861641(3)             |                          |
| 2497  | $E$               | 84         | 2.7      | 5086.861644(4)             |                          |
| 2498  | $A_2$             | 83         | 2.6      | 5086.913899(1)             |                          |
| 2499  | $E$               | 107        | 2.1      | 5089.91637(1)              |                          |
| 2500  | $E$               | 97         | 2.1      | 5089.91637(1)              |                          |
| 2501  | $E$               | 107        | 2.1      | 5089.939847(7)             |                          |
| 2502  | $E$               | 102        | 2.1      | 5089.93985(1)              |                          |
| 2503  | $A_1$             | 107        | 0.68     | 5094.859184(1)             |                          |
| 2504  | $A_1^*$           | 97         | 2.2      | 5096.95900(3)              |                          |
| 2505  | $A_2^*$           | 92         | 2.2      | 5096.95901(3)              |                          |
| 2506  | $E$               | 107        | 2.2      | 5096.97019(2)              |                          |
| 2507  | $E$               | 104        | 2.2      | 5096.97019(1)              |                          |
| 2508  | $E$               | 102        | 0.35     | 5096.997723(1)             |                          |
| 2509  | $E$               | 104        | 0.35     | 5096.997724(1)             |                          |
| 2510  | $E$               | 117        | 0.56     | 5097.845438(5)             |                          |
| 2511  | $E$               | 112        | 0.56     | 5097.845438(8)             |                          |
| 2512  | $A_1$             | 103        | 0.37     | 5098.454879(9)             |                          |
| 2513  | $A_1$             | 117        | 0.6      | 5099.307409(3)             |                          |
| 2514  | $E$               | 88         | 0.13     | 5100.327737(1)             |                          |
| 2515  | $E$               | 88         | 0.13     | 5100.327737(1)             |                          |
| 2516  | $E$               | 100        | 0.64     | 5100.331208(1)             |                          |
| 2517  | $E$               | 102        | 0.64     | 5100.331208(1)             |                          |
| 2518  | $E$               | 106        | 2.2      | 5101.12072(2)              |                          |
| 2519  | $E$               | 116        | 2.2      | 5101.12072(2)              |                          |
| 2520  | $A_1$             | 111        | 2.2      | 5101.21586(1)              |                          |
| 2521  | $A_2$             | 94         | 2.2      | 5101.21613(3)              |                          |
| 2522  | $A_2$             | 109        | 2.3      | 5102.386723(6)             |                          |

Continued on next page.

TABLE S4 – states on Sarka/Poirier CSC PES; continued from previous page

| State | $\Gamma_{C_{3v}}$ | $D_{\max}$ | $S_{vN}$ | $\tilde{E}/\text{cm}^{-1}$ | $\Delta\text{Ref. [30]}$ |
|-------|-------------------|------------|----------|----------------------------|--------------------------|
| 2523  | $A_1$             | 117        | 2.3      | 5102.394680(1)             |                          |
| 2524  | $E$               | 118        | 2.2      | 5102.483404(2)             |                          |
| 2525  | $E$               | 109        | 2.2      | 5102.483406(2)             |                          |
| 2526  | $E$               | 108        | 0.58     | 5102.687730(8)             |                          |
| 2527  | $E$               | 109        | 0.59     | 5102.687730(9)             |                          |
| 2528  | $E$               | 83         | 0.069    | 5103.332500(6)             |                          |
| 2529  | $E$               | 84         | 0.069    | 5103.332500(7)             |                          |
| 2530  | $E$               | 100        | 0.26     | 5103.904042(4)             |                          |
| 2531  | $E$               | 100        | 0.26     | 5103.904043(1)             |                          |
| 2532  | $E$               | 137        | 2.1      | 5104.890353(2)             |                          |
| 2533  | $E$               | 111        | 2.1      | 5104.89036(1)              |                          |
| 2534  | $A_2$             | 102        | 2.1      | 5104.90949(1)              |                          |
| 2535  | $A_1$             | 104        | 2.2      | 5104.92409(2)              |                          |
| 2536  | $E$               | 112        | 0.15     | 5106.376665(5)             |                          |
| 2537  | $E$               | 112        | 0.15     | 5106.376666(5)             |                          |
| 2538  | $A_1$             | 106        | 2.7      | 5107.34573(1)              |                          |
| 2539  | $E$               | 73         | 2.7      | 5107.47359(8)              |                          |
| 2540  | $E$               | 89         | 2.7      | 5107.47360(7)              |                          |
| 2541  | $A_2$             | 99         | 2.6      | 5107.517999(3)             |                          |
| 2542  | $E$               | 85         | 0.24     | 5112.459184(4)             |                          |
| 2543  | $E$               | 95         | 0.24     | 5112.459184(2)             |                          |
| 2544  | $E$               | 126        | 2.2      | 5114.322496(6)             |                          |
| 2545  | $E$               | 148        | 2.2      | 5114.322497(6)             |                          |
| 2546  | $A_2$             | 80         | 0.31     | 5115.000262(3)             |                          |
| 2547  | $A_1$             | 87         | 0.31     | 5115.000262(2)             |                          |
| 2548  | $E$               | 140        | 3.2      | 5115.115264(6)             |                          |
| 2549  | $E$               | 143        | 3.2      | 5115.115265(7)             |                          |
| 2550  | $A_2$             | 103        | 3.1      | 5115.296046(6)             |                          |
| 2551  | $A_1$             | 127        | 3.1      | 5115.29605(1)              |                          |
| 2552  | $A_1$             | 86         | 2.2      | 5115.45823(1)              |                          |
| 2553  | $A_2$             | 88         | 2.2      | 5115.45823(1)              |                          |
| 2554  | $E$               | 115        | 2.2      | 5115.476012(4)             |                          |
| 2555  | $E$               | 82         | 2.2      | 5115.47602(2)              |                          |
| 2556  | $E$               | 124        | 2.2      | 5115.639190(6)             |                          |
| 2557  | $E$               | 139        | 2.2      | 5115.639190(5)             |                          |
| 2558  | $E$               | 143        | 2.7      | 5117.154886(8)             |                          |
| 2559  | $E$               | 173        | 2.7      | 5117.15489(1)              |                          |
| 2560  | $E$               | 164        | 2.7      | 5117.244492(4)             |                          |
| 2561  | $E$               | 158        | 2.7      | 5117.244493(5)             |                          |
| 2562  | $A_1$             | 156        | 2.9      | 5119.872381(7)             |                          |
| 2563  | $E$               | 177        | 2.7      | 5120.114517(3)             |                          |
| 2564  | $E$               | 164        | 2.7      | 5120.114518(4)             |                          |
| 2565  | $A_2$             | 157        | 2.7      | 5120.280864(6)             |                          |
| 2566  | $E$               | 143        | 2.4      | 5121.089923(2)             |                          |
| 2567  | $E$               | 103        | 2.4      | 5121.089926(8)             |                          |
| 2568  | $E$               | 108        | 2.4      | 5121.11205(1)              |                          |
| 2569  | $E$               | 156        | 2.4      | 5121.11205(1)              |                          |
| 2570  | $E$               | 76         | 1.1      | 5121.184157(1)             |                          |
| 2571  | $E$               | 78         | 1.1      | 5121.184157(2)             |                          |
| 2572  | $A_2^*$           | 68         | 0.3      | 5121.89977(3)              |                          |
| 2573  | $A_1^*$           | 67         | 0.3      | 5121.89977(4)              |                          |
| 2574  | $E$               | 178        | 2.3      | 5122.667259(2)             |                          |
| 2575  | $E$               | 135        | 2.3      | 5122.66726(1)              |                          |
| 2576  | $A_2^*$           | 145        | 3.3      | 5123.455531(7)             |                          |
| 2577  | $A_1^*$           | 141        | 3.3      | 5123.455532(8)             |                          |
| 2578  | $E$               | 179        | 3.1      | 5123.625285(2)             |                          |
| 2579  | $E$               | 142        | 3.1      | 5123.625288(4)             |                          |
| 2580  | $A_2$             | 106        | 2.5      | 5123.629181(7)             |                          |
| 2581  | $E$               | 134        | 2.5      | 5123.957708(2)             |                          |

Continued on next page.

TABLE S4 – states on Sarka/Poirier CSC PES; continued from previous page

| State | $\Gamma_{C_{3v}}$ | $D_{\max}$ | $S_{vN}$ | $\tilde{E}/\text{cm}^{-1}$ | $\Delta\text{Ref. [30]}$ |
|-------|-------------------|------------|----------|----------------------------|--------------------------|
| 2582  | $E$               | 101        | 2.5      | 5123.95771(1)              |                          |
| 2583  | $E$               | 128        | 2.3      | 5123.973555(9)             |                          |
| 2584  | $E$               | 129        | 2.3      | 5123.973556(9)             |                          |
| 2585  | $A_1$             | 101        | 2.5      | 5124.238798(9)             |                          |
| 2586  | $E$               | 177        | 3.2      | 5124.279142(3)             |                          |
| 2587  | $E$               | 158        | 3.2      | 5124.279144(6)             |                          |
| 2588  | $E$               | 179        | 3.3      | 5124.402200(3)             |                          |
| 2589  | $E$               | 178        | 3.3      | 5124.402200(3)             |                          |
| 2590  | $A_2$             | 170        | 3.1      | 5124.660046(5)             |                          |
| 2591  | $A_1$             | 151        | 3.1      | 5124.66081(2)              |                          |
| 2592  | $A_2$             | 165        | 2.9      | 5124.705475(8)             |                          |
| 2593  | $A_1$             | 148        | 2.9      | 5124.705505(8)             |                          |
| 2594  | $E$               | 94         | 0.78     | 5125.735677(2)             |                          |
| 2595  | $E$               | 94         | 0.78     | 5125.735678(3)             |                          |
| 2596  | $E$               | 140        | 3.1      | 5127.20052(1)              |                          |
| 2597  | $E$               | 121        | 3.1      | 5127.20052(3)              |                          |
| 2598  | $A_2$             | 144        | 3.2      | 5127.20362(1)              |                          |
| 2599  | $A_1$             | 163        | 3.3      | 5127.335720(4)             |                          |
| 2600  | $E$               | 158        | 2.5      | 5127.592881(3)             |                          |
| 2601  | $E$               | 156        | 2.5      | 5127.592882(3)             |                          |
| 2602  | $E$               | 158        | 2.4      | 5127.613834(3)             |                          |
| 2603  | $E$               | 158        | 2.4      | 5127.613834(3)             |                          |
| 2604  | $A_1$             | 130        | 2.4      | 5128.22523(2)              |                          |
| 2605  | $A_2$             | 184        | 2.4      | 5128.225306(2)             |                          |
| 2606  | $E$               | 131        | 0.81     | 5128.423496(8)             |                          |
| 2607  | $E$               | 163        | 0.81     | 5128.423499(9)             |                          |
| 2608  | $E$               | 98         | 0.34     | 5128.645726(3)             |                          |
| 2609  | $E$               | 89         | 0.34     | 5128.645727(2)             |                          |
| 2610  | $E$               | 184        | 3.5      | 5128.967834(5)             |                          |
| 2611  | $E$               | 153        | 3.5      | 5128.967837(8)             |                          |
| 2612  | $E$               | 138        | 3.2      | 5129.18076(1)              |                          |
| 2613  | $E$               | 189        | 3.2      | 5129.18076(1)              |                          |
| 2614  | $A_1$             | 124        | 2.3      | 5129.531779(3)             |                          |
| 2615  | $A_2$             | 119        | 2.3      | 5129.531785(3)             |                          |
| 2616  | $A_1$             | 180        | 0.86     | 5129.890541(2)             |                          |
| 2617  | $E$               | 106        | 0.61     | 5130.387469(4)             |                          |
| 2618  | $E$               | 120        | 0.61     | 5130.387469(5)             |                          |
| 2619  | $E$               | 93         | 2.1      | 5130.661230(7)             |                          |
| 2620  | $E$               | 99         | 2.1      | 5130.661230(6)             |                          |
| 2621  | $E$               | 144        | 2.5      | 5130.909670(4)             |                          |
| 2622  | $E$               | 144        | 2.5      | 5130.909670(4)             |                          |
| 2623  | $A_2$             | 79         | 2.1      | 5130.994771(3)             |                          |
| 2624  | $A_1$             | 76         | 2.1      | 5130.994772(4)             |                          |
| 2625  | $A_1$             | 115        | 0.62     | 5131.85996(1)              |                          |
| 2626  | $A_1$             | 121        | 3.3      | 5131.96948(3)              |                          |
| 2627  | $A_2$             | 119        | 3.3      | 5131.97543(1)              |                          |
| 2628  | $E$               | 141        | 2.5      | 5132.092472(6)             |                          |
| 2629  | $E$               | 139        | 2.5      | 5132.092473(7)             |                          |
| 2630  | $E$               | 124        | 2.4      | 5132.341581(4)             |                          |
| 2631  | $E$               | 131        | 2.3      | 5132.341583(5)             |                          |
| 2632  | $E$               | 92         | 0.37     | 5132.694385(3)             |                          |
| 2633  | $E$               | 91         | 0.37     | 5132.694385(4)             |                          |
| 2634  | $E$               | 99         | 1.0      | 5133.792209(2)             |                          |
| 2635  | $E$               | 84         | 1.0      | 5133.792210(9)             |                          |
| 2636  | $A_2$             | 143        | 2.7      | 5133.845444(2)             |                          |
| 2637  | $A_1$             | 147        | 2.7      | 5133.86186(1)              |                          |
| 2638  | $E$               | 147        | 3.3      | 5133.929114(3)             |                          |
| 2639  | $E$               | 144        | 3.3      | 5133.929119(6)             |                          |
| 2640  | $E$               | 85         | 0.96     | 5133.943415(2)             |                          |

Continued on next page.

TABLE S4 – states on Sarka/Poirier CSC PES; continued from previous page

| State | $\Gamma_{C_{3v}}$ | $D_{\max}$ | $S_{vN}$ | $\tilde{E}/\text{cm}^{-1}$ | $\Delta\text{Ref. [30]}$ |
|-------|-------------------|------------|----------|----------------------------|--------------------------|
| 2641  | $E$               | 84         | 0.96     | 5133.943415(2)             |                          |
| 2642  | $A_1$             | 94         | 0.37     | 5134.044114(3)             |                          |
| 2643  | $E$               | 102        | 0.5      | 5134.904850(2)             |                          |
| 2644  | $E$               | 104        | 0.5      | 5134.904851(3)             |                          |
| 2645  | $E$               | 130        | 0.77     | 5135.377572(3)             |                          |
| 2646  | $E$               | 130        | 0.77     | 5135.377574(3)             |                          |
| 2647  | $E$               | 92         | 1.5      | 5135.956005(9)             |                          |
| 2648  | $E$               | 79         | 1.5      | 5135.956010(5)             |                          |
| 2649  | $E$               | 80         | 0.4      | 5136.215084(1)             |                          |
| 2650  | $E$               | 74         | 0.4      | 5136.215084(1)             |                          |
| 2651  | $A_1$             | 80         | 0.56     | 5137.644388(1)             |                          |
| 2652  | $E$               | 82         | 0.63     | 5138.267461(2)             |                          |
| 2653  | $E$               | 86         | 0.63     | 5138.267461(2)             |                          |
| 2654  | $E$               | 183        | 2.5      | 5138.471625(3)             |                          |
| 2655  | $E$               | 124        | 2.5      | 5138.47163(3)              |                          |
| 2656  | $E$               | 163        | 2.8      | 5138.61572(1)              |                          |
| 2657  | $E$               | 166        | 2.8      | 5138.61572(1)              |                          |
| 2658  | $A_1$             | 67         | 1.2      | 5139.16558(4)              |                          |
| 2659  | $A_2$             | 67         | 1.2      | 5139.16565(5)              |                          |
| 2660  | $A_1$             | 80         | 0.64     | 5139.709054(3)             |                          |
| 2661  | $E$               | 96         | 0.49     | 5140.274354(8)             |                          |
| 2662  | $E$               | 103        | 0.49     | 5140.274354(7)             |                          |
| 2663  | $A_1$             | 144        | 2.7      | 5141.140459(6)             |                          |
| 2664  | $E$               | 154        | 2.5      | 5141.439297(2)             |                          |
| 2665  | $E$               | 160        | 2.5      | 5141.439300(4)             |                          |
| 2666  | $A_2$             | 152        | 2.3      | 5141.627198(3)             |                          |
| 2667  | $E$               | 86         | 1.3      | 5141.853015(4)             |                          |
| 2668  | $E$               | 87         | 1.3      | 5141.853015(3)             |                          |
| 2669  | $A_2$             | 83         | 2.1      | 5141.89200(1)              |                          |
| 2670  | $A_1$             | 82         | 2.1      | 5141.89238(1)              |                          |
| 2671  | $E$               | 81         | 2.1      | 5141.90474(1)              |                          |
| 2672  | $E$               | 80         | 2.1      | 5141.90474(1)              |                          |
| 2673  | $A_2$             | 89         | 2.0      | 5142.174377(2)             |                          |
| 2674  | $E$               | 94         | 2.1      | 5142.679912(2)             |                          |
| 2675  | $E$               | 95         | 2.1      | 5142.679912(2)             |                          |
| 2676  | $A_1$             | 95         | 2.1      | 5143.218124(2)             |                          |
| 2677  | $E$               | 107        | 2.3      | 5143.99883(1)              |                          |
| 2678  | $E$               | 110        | 2.3      | 5143.998827(8)             |                          |
| 2679  | $E$               | 107        | 2.2      | 5144.283873(8)             |                          |
| 2680  | $E$               | 110        | 2.2      | 5144.283873(7)             |                          |
| 2681  | $E$               | 115        | 2.3      | 5145.674195(4)             |                          |
| 2682  | $E$               | 101        | 2.3      | 5145.67420(1)              |                          |
| 2683  | $A_1$             | 91         | 2.2      | 5145.704963(9)             |                          |
| 2684  | $A_2$             | 95         | 2.2      | 5145.708564(4)             |                          |
| 2685  | $E$               | 129        | 2.6      | 5147.222017(5)             |                          |
| 2686  | $E$               | 132        | 2.6      | 5147.222018(4)             |                          |
| 2687  | $E$               | 130        | 2.5      | 5147.306189(3)             |                          |
| 2688  | $E$               | 131        | 2.5      | 5147.306189(3)             |                          |
| 2689  | $A_1$             | 108        | 1.8      | 5149.35022(3)              |                          |
| 2690  | $A_2$             | 105        | 1.8      | 5149.35045(5)              |                          |
| 2691  | $A_1$             | 104        | 1.6      | 5149.62340(3)              |                          |
| 2692  | $A_2$             | 112        | 1.6      | 5149.62342(2)              |                          |
| 2693  | $A_1$             | 123        | 2.7      | 5150.021935(3)             |                          |
| 2694  | $E$               | 107        | 2.6      | 5150.18613(1)              |                          |
| 2695  | $E$               | 128        | 2.6      | 5150.18613(1)              |                          |
| 2696  | $A_2$             | 117        | 2.6      | 5150.287822(6)             |                          |
| 2697  | $E$               | 141        | 0.82     | 5152.281531(3)             |                          |
| 2698  | $E$               | 166        | 0.79     | 5152.281534(4)             |                          |
| 2699  | $E$               | 127        | 0.78     | 5152.465143(4)             |                          |

Continued on next page.

TABLE S4 – states on Sarka/Poirier CSC PES; continued from previous page

| State | $\Gamma_{C_{3v}}$ | $D_{\max}$ | $S_{vN}$ | $\tilde{E}/\text{cm}^{-1}$ | $\Delta\text{Ref. [30]}$ |
|-------|-------------------|------------|----------|----------------------------|--------------------------|
| 2700  | $E$               | 131        | 0.77     | 5152.465144(5)             |                          |
| 2701  | $E$               | 87         | 1.4      | 5154.505167(7)             |                          |
| 2702  | $E$               | 92         | 1.4      | 5154.505168(6)             |                          |
| 2703  | $A_1$             | 85         | 2.3      | 5154.67847(3)              |                          |
| 2704  | $A_2$             | 86         | 2.3      | 5154.67847(2)              |                          |
| 2705  | $E$               | 107        | 2.3      | 5154.91737(1)              |                          |
| 2706  | $E$               | 103        | 2.3      | 5154.91737(1)              |                          |
| 2707  | $E$               | 104        | 2.9      | 5154.926779(6)             |                          |
| 2708  | $E$               | 134        | 3.0      | 5154.926781(6)             |                          |
| 2709  | $A_1$             | 77         | 2.2      | 5155.058601(7)             |                          |
| 2710  | $A_2$             | 75         | 2.2      | 5155.058602(8)             |                          |
| 2711  | $E$               | 95         | 0.79     | 5158.820383(2)             |                          |
| 2712  | $E$               | 92         | 0.78     | 5158.820384(3)             |                          |
| 2713  | $E$               | 68         | 0.52     | 5159.349647(1)             |                          |
| 2714  | $E$               | 68         | 0.52     | 5159.349648(2)             |                          |
| 2715  | $A_1$             | 94         | 0.79     | 5160.256628(2)             |                          |
| 2716  | $A_1$             | 83         | 1.2      | 5160.357365(1)             |                          |
| 2717  | $A_2$             | 86         | 1.2      | 5160.357368(1)             |                          |
| 2718  | $E$               | 110        | 2.3      | 5160.624375(6)             |                          |
| 2719  | $E$               | 146        | 2.3      | 5160.624376(5)             |                          |
| 2720  | $E$               | 145        | 2.2      | 5160.724274(1)             |                          |
| 2721  | $E$               | 90         | 2.2      | 5160.72428(1)              |                          |
| 2722  | $E$               | 135        | 2.4      | 5162.692256(3)             |                          |
| 2723  | $E$               | 144        | 2.4      | 5162.692256(2)             |                          |
| 2724  | $A_2$             | 87         | 2.3      | 5162.89215(4)              |                          |
| 2725  | $A_1$             | 86         | 2.3      | 5162.89215(5)              |                          |
| 2726  | $E$               | 104        | 1.3      | 5163.248616(1)             |                          |
| 2727  | $E$               | 93         | 1.3      | 5163.248617(5)             |                          |
| 2728  | $A_1$             | 100        | 2.3      | 5163.300302(7)             |                          |
| 2729  | $E$               | 90         | 2.2      | 5163.550724(6)             |                          |
| 2730  | $E$               | 92         | 2.2      | 5163.550724(6)             |                          |
| 2731  | $A_2$             | 81         | 2.2      | 5163.718941(8)             |                          |
| 2732  | $E$               | 79         | 0.51     | 5167.463828(2)             |                          |
| 2733  | $E$               | 63         | 0.51     | 5167.463832(5)             |                          |
| 2734  | $E$               | 145        | 2.4      | 5168.020686(2)             |                          |
| 2735  | $E$               | 139        | 2.4      | 5168.020686(2)             |                          |
| 2736  | $E$               | 103        | 2.4      | 5168.20840(1)              |                          |
| 2737  | $E$               | 98         | 2.4      | 5168.20840(2)              |                          |
| 2738  | $A_1$             | 115        | 2.4      | 5170.349565(4)             |                          |
| 2739  | $E$               | 114        | 2.4      | 5170.880187(4)             |                          |
| 2740  | $E$               | 118        | 2.4      | 5170.880187(3)             |                          |
| 2741  | $A_2$             | 91         | 2.4      | 5171.21842(1)              |                          |
| 2742  | $A_1$             | 111        | 0.46     | 5172.761737(4)             |                          |
| 2743  | $A_2$             | 124        | 0.46     | 5172.761737(4)             |                          |
| 2744  | $E$               | 107        | 2.2      | 5173.793906(2)             |                          |
| 2745  | $E$               | 111        | 2.2      | 5173.793907(3)             |                          |
| 2746  | $E$               | 82         | 3.1      | 5174.69177(1)              |                          |
| 2747  | $E$               | 118        | 3.1      | 5174.69178(2)              |                          |
| 2748  | $A_1$             | 84         | 3.2      | 5174.69677(1)              |                          |
| 2749  | $A_2$             | 82         | 3.1      | 5174.69766(1)              |                          |
| 2750  | $E$               | 101        | 2.2      | 5175.106120(1)             |                          |
| 2751  | $E$               | 100        | 2.2      | 5175.106120(1)             |                          |
| 2752  | $A_1$             | 57         | 1.4      | 5175.14076(2)              |                          |
| 2753  | $A_2$             | 56         | 1.4      | 5175.14076(3)              |                          |
| 2754  | $E$               | 83         | 1.5      | 5178.019775(2)             |                          |
| 2755  | $E$               | 74         | 1.5      | 5178.019776(3)             |                          |
| 2756  | $E$               | 109        | 3.3      | 5179.45615(2)              |                          |
| 2757  | $E$               | 140        | 3.3      | 5179.45615(3)              |                          |
| 2758  | $E$               | 132        | 2.0      | 5179.745878(4)             |                          |

Continued on next page.



TABLE S4 – states on Sarka/Poirier CSC PES; continued from previous page

| State | $\Gamma_{C_{3v}}$ | $D_{\max}$ | $S_{vN}$ | $\tilde{E}/\text{cm}^{-1}$ | $\Delta\text{Ref. [30]}$ |
|-------|-------------------|------------|----------|----------------------------|--------------------------|
| 2759  | $E$               | 138        | 2.0      | 5179.745878(4)             |                          |
| 2760  | $E$               | 137        | 3.3      | 5180.139120(7)             |                          |
| 2761  | $E$               | 147        | 3.3      | 5180.139123(8)             |                          |
| 2762  | $E$               | 83         | 0.52     | 5182.114858(3)             |                          |
| 2763  | $E$               | 81         | 0.52     | 5182.114859(1)             |                          |
| 2764  | $E$               | 143        | 2.7      | 5182.928523(2)             |                          |
| 2765  | $E$               | 144        | 2.7      | 5182.928523(2)             |                          |
| 2766  | $A_1$             | 120        | 2.7      | 5182.967554(7)             |                          |
| 2767  | $A_2$             | 101        | 2.7      | 5182.96774(2)              |                          |
| 2768  | $E$               | 123        | 0.93     | 5183.929010(4)             |                          |
| 2769  | $E$               | 145        | 0.93     | 5183.929011(4)             |                          |
| 2770  | $E$               | 131        | 0.94     | 5184.493070(2)             |                          |
| 2771  | $E$               | 130        | 0.96     | 5184.493070(2)             |                          |
| 2772  | $E$               | 111        | 2.1      | 5185.286218(1)             |                          |
| 2773  | $E$               | 108        | 2.1      | 5185.286218(1)             |                          |
| 2774  | $E$               | 107        | 2.1      | 5185.303986(1)             |                          |
| 2775  | $E$               | 109        | 2.1      | 5185.303986(1)             |                          |
| 2776  | $A_1$             | 105        | 0.78     | 5185.34888(1)              |                          |
| 2777  | $E$               | 111        | 2.5      | 5186.42770(2)              |                          |
| 2778  | $E$               | 111        | 2.5      | 5186.42770(2)              |                          |
| 2779  | $A_1$             | 92         | 2.4      | 5186.61291(3)              |                          |
| 2780  | $A_2$             | 95         | 2.4      | 5186.61292(3)              |                          |
| 2781  | $A_1$             | 97         | 2.1      | 5186.79734(2)              |                          |
| 2782  | $A_2$             | 96         | 2.1      | 5186.79735(1)              |                          |
| 2783  | $E$               | 161        | 2.4      | 5186.898156(3)             |                          |
| 2784  | $E$               | 148        | 2.4      | 5186.898156(6)             |                          |
| 2785  | $E$               | 101        | 2.0      | 5187.959492(6)             |                          |
| 2786  | $E$               | 106        | 2.0      | 5187.959493(6)             |                          |
| 2787  | $A_1^*$           | 83         | 2.1      | 5188.012397(6)             |                          |
| 2788  | $A_2^*$           | 82         | 2.1      | 5188.012398(5)             |                          |
| 2789  | $E$               | 78         | 2.1      | 5188.19175(1)              |                          |
| 2790  | $E$               | 70         | 2.1      | 5188.19175(3)              |                          |
| 2791  | $A_1$             | 68         | 2.1      | 5188.19195(2)              |                          |
| 2792  | $A_2$             | 104        | 2.1      | 5188.203429(4)             |                          |
| 2793  | $A_2$             | 83         | 2.4      | 5190.42200(2)              |                          |
| 2794  | $A_1$             | 74         | 2.4      | 5190.42200(4)              |                          |
| 2795  | $E$               | 101        | 2.3      | 5190.52912(1)              |                          |
| 2796  | $E$               | 83         | 2.3      | 5190.52913(1)              |                          |
| 2797  | $E$               | 132        | 2.2      | 5191.037583(4)             |                          |
| 2798  | $E$               | 103        | 2.2      | 5191.03759(1)              |                          |
| 2799  | $A_2$             | 98         | 2.1      | 5191.041727(8)             |                          |
| 2800  | $A_1$             | 113        | 2.3      | 5191.12317(1)              |                          |
| 2801  | $E$               | 174        | 2.6      | 5192.127566(2)             |                          |
| 2802  | $E$               | 109        | 2.6      | 5192.12757(3)              |                          |
| 2803  | $E$               | 109        | 2.5      | 5192.25899(3)              |                          |
| 2804  | $E$               | 111        | 2.5      | 5192.25899(3)              |                          |
| 2805  | $E$               | 103        | 0.21     | 5192.465665(3)             |                          |
| 2806  | $E$               | 113        | 0.21     | 5192.465668(4)             |                          |
| 2807  | $E$               | 130        | 2.6      | 5194.677321(5)             |                          |
| 2808  | $E$               | 107        | 2.6      | 5194.67732(1)              |                          |
| 2809  | $A_1$             | 81         | 3.0      | 5194.75359(3)              |                          |
| 2810  | $A_2$             | 80         | 2.5      | 5194.75432(2)              |                          |
| 2811  | $A_1$             | 101        | 3.1      | 5194.77960(4)              |                          |
| 2812  | $E$               | 108        | 2.6      | 5195.07367(1)              |                          |
| 2813  | $E$               | 95         | 2.6      | 5195.07367(3)              |                          |
| 2814  | $A_2$             | 102        | 2.5      | 5195.260826(8)             |                          |
| 2815  | $E$               | 91         | 0.74     | 5196.15968(1)              |                          |
| 2816  | $E$               | 78         | 0.73     | 5196.159690(8)             |                          |
| 2817  | $E$               | 104        | 2.0      | 5196.877277(7)             |                          |

Continued on next page.

TABLE S4 – states on Sarka/Poirier CSC PES; continued from previous page

| State | $\Gamma_{C_{3v}}$ | $D_{\max}$ | $S_{vN}$ | $\tilde{E}/\text{cm}^{-1}$ | $\Delta\text{Ref. [30]}$ |
|-------|-------------------|------------|----------|----------------------------|--------------------------|
| 2818  | $E$               | 135        | 2.0      | 5196.877278(7)             |                          |
| 2819  | $E$               | 129        | 2.0      | 5196.910756(3)             |                          |
| 2820  | $E$               | 112        | 2.0      | 5196.910757(6)             |                          |
| 2821  | $A_1$             | 77         | 0.065    | 5198.36127(2)              |                          |
| 2822  | $A_2$             | 74         | 0.065    | 5198.36786(2)              |                          |
| 2823  | $A_1$             | 91         | 2.1      | 5200.097583(6)             |                          |
| 2824  | $A_2$             | 95         | 2.1      | 5200.097585(7)             |                          |
| 2825  | $E$               | 87         | 2.2      | 5200.11959(1)              |                          |
| 2826  | $E$               | 86         | 2.2      | 5200.11959(1)              |                          |
| 2827  | $A_1$             | 119        | 0.39     | 5202.04526(1)              |                          |
| 2828  | $A_2$             | 127        | 0.39     | 5202.04526(1)              |                          |
| 2829  | $A_1$             | 76         | 0.46     | 5205.994953(5)             |                          |
| 2830  | $A_2$             | 94         | 0.46     | 5205.994960(6)             |                          |
| 2831  | $E$               | 141        | 2.6      | 5207.27506(1)              |                          |
| 2832  | $E$               | 140        | 2.6      | 5207.27506(1)              |                          |
| 2833  | $E$               | 122        | 2.4      | 5207.564475(8)             |                          |
| 2834  | $E$               | 141        | 2.4      | 5207.564478(9)             |                          |
| 2835  | $E$               | 113        | 2.2      | 5207.64874(2)              |                          |
| 2836  | $E$               | 167        | 2.2      | 5207.64875(2)              |                          |
| 2837  | $E$               | 116        | 3.3      | 5208.46578(1)              |                          |
| 2838  | $E$               | 133        | 3.3      | 5208.46578(2)              |                          |
| 2839  | $A_1$             | 114        | 3.4      | 5208.47339(2)              |                          |
| 2840  | $A_2$             | 103        | 3.4      | 5208.47419(3)              |                          |
| 2841  | $E$               | 129        | 2.4      | 5208.864996(2)             |                          |
| 2842  | $E$               | 130        | 2.4      | 5208.864998(3)             |                          |
| 2843  | $E$               | 131        | 0.78     | 5209.05810(1)              |                          |
| 2844  | $E$               | 177        | 0.81     | 5209.05810(1)              |                          |
| 2845  | $E$               | 98         | 2.2      | 5209.532328(8)             |                          |
| 2846  | $E$               | 96         | 2.2      | 5209.532328(9)             |                          |
| 2847  | $E$               | 100        | 2.2      | 5209.548888(6)             |                          |
| 2848  | $E$               | 98         | 2.2      | 5209.548888(7)             |                          |
| 2849  | $E$               | 101        | 0.099    | 5210.874001(2)             |                          |
| 2850  | $E$               | 106        | 0.099    | 5210.874003(2)             |                          |
| 2851  | $E$               | 75         | 0.11     | 5211.216029(1)             |                          |
| 2852  | $E$               | 76         | 0.11     | 5211.216029(1)             |                          |
| 2853  | $E$               | 95         | 0.51     | 5213.026089(7)             |                          |
| 2854  | $E$               | 128        | 0.51     | 5213.026090(8)             |                          |
| 2855  | $E$               | 187        | 1.4      | 5213.127244(4)             |                          |
| 2856  | $E$               | 136        | 1.4      | 5213.12725(2)              |                          |
| 2857  | $E$               | 142        | 3.0      | 5214.43524(1)              |                          |
| 2858  | $E$               | 131        | 3.0      | 5214.43524(3)              |                          |
| 2859  | $A_1$             | 158        | 0.85     | 5214.564257(5)             |                          |
| 2860  | $A_2$             | 104        | 2.4      | 5214.58708(5)              |                          |
| 2861  | $A_1$             | 117        | 2.4      | 5214.58713(6)              |                          |
| 2862  | $A_2$             | 89         | 2.3      | 5216.23647(2)              |                          |
| 2863  | $A_1$             | 83         | 2.3      | 5216.23648(6)              |                          |
| 2864  | $E$               | 106        | 2.3      | 5216.31257(1)              |                          |
| 2865  | $E$               | 147        | 2.3      | 5216.31257(1)              |                          |
| 2866  | $E$               | 119        | 0.54     | 5217.245926(2)             |                          |
| 2867  | $E$               | 99         | 0.54     | 5217.245926(5)             |                          |
| 2868  | $E$               | 163        | 3.7      | 5217.717729(5)             |                          |
| 2869  | $E$               | 114        | 3.7      | 5217.71773(1)              |                          |
| 2870  | $A_1$             | 160        | 3.6      | 5217.72368(1)              |                          |
| 2871  | $A_2$             | 164        | 3.6      | 5217.723782(6)             |                          |
| 2872  | $E$               | 191        | 3.6      | 5217.975722(6)             |                          |
| 2873  | $E$               | 193        | 3.6      | 5217.975724(6)             |                          |
| 2874  | $A_1$             | 140        | 3.5      | 5217.98999(3)              |                          |
| 2875  | $A_2$             | 194        | 3.5      | 5217.99005(4)              |                          |
| 2876  | $A_2$             | 131        | 2.5      | 5218.60559(1)              |                          |

Continued on next page.

TABLE S4 – states on Sarka/Poirier CSC PES; continued from previous page

| State | $\Gamma_{C_{3v}}$ | $D_{\max}$ | $S_{vN}$ | $\tilde{E}/\text{cm}^{-1}$ | $\Delta\text{Ref. [30]}$ |
|-------|-------------------|------------|----------|----------------------------|--------------------------|
| 2877  | $A_1$             | 137        | 4.0      | 5218.64727(2)              |                          |
| 2878  | $A_1$             | 131        | 5.2      | 5218.67043(4)              |                          |
| 2879  | $E$               | 130        | 2.5      | 5218.73064(4)              |                          |
| 2880  | $E$               | 133        | 2.5      | 5218.73064(4)              |                          |
| 2881  | $E$               | 69         | 0.15     | 5219.074148(2)             |                          |
| 2882  | $E$               | 83         | 0.16     | 5219.074148(1)             |                          |
| 2883  | $E$               | 149        | 1.8      | 5219.213246(4)             |                          |
| 2884  | $E$               | 147        | 1.8      | 5219.213249(5)             |                          |
| 2885  | $E$               | 170        | 1.8      | 5219.468860(4)             |                          |
| 2886  | $E$               | 156        | 1.7      | 5219.468862(8)             |                          |
| 2887  | $E$               | 120        | 0.57     | 5220.079045(9)             |                          |
| 2888  | $E$               | 118        | 0.56     | 5220.079045(7)             |                          |
| 2889  | $E$               | 104        | 2.3      | 5220.153830(8)             |                          |
| 2890  | $E$               | 101        | 2.3      | 5220.15383(1)              |                          |
| 2891  | $A_1$             | 88         | 2.3      | 5220.39595(1)              |                          |
| 2892  | $A_2$             | 84         | 2.3      | 5220.39687(1)              |                          |
| 2893  | $E$               | 77         | 0.028    | 5220.569276(1)             |                          |
| 2894  | $E$               | 72         | 0.028    | 5220.569277(3)             |                          |
| 2895  | $E$               | 88         | 2.1      | 5220.657232(6)             |                          |
| 2896  | $E$               | 94         | 2.1      | 5220.657233(4)             |                          |
| 2897  | $A_1$             | 85         | 2.2      | 5220.668722(2)             |                          |
| 2898  | $A_2$             | 109        | 2.2      | 5220.668725(4)             |                          |
| 2899  | $A_1$             | 109        | 0.11     | 5221.772316(2)             |                          |
| 2900  | $E$               | 92         | 0.89     | 5221.874062(9)             |                          |
| 2901  | $E$               | 91         | 0.95     | 5221.87406(1)              |                          |
| 2902  | $A_2$             | 103        | 0.083    | 5222.463042(2)             |                          |
| 2903  | $A_2$             | 105        | 2.1      | 5223.262966(1)             |                          |
| 2904  | $E$               | 171        | 3.4      | 5223.446059(3)             |                          |
| 2905  | $E$               | 178        | 3.4      | 5223.446061(4)             |                          |
| 2906  | $A_2$             | 160        | 3.3      | 5223.539943(8)             |                          |
| 2907  | $A_1$             | 133        | 3.3      | 5223.54066(3)              |                          |
| 2908  | $E$               | 169        | 3.3      | 5223.752871(8)             |                          |
| 2909  | $E$               | 183        | 3.3      | 5223.752872(7)             |                          |
| 2910  | $E$               | 176        | 3.1      | 5223.847146(5)             |                          |
| 2911  | $E$               | 143        | 3.1      | 5223.84715(1)              |                          |
| 2912  | $E$               | 96         | 2.1      | 5224.144541(4)             |                          |
| 2913  | $E$               | 85         | 2.1      | 5224.144544(4)             |                          |
| 2914  | $A_1$             | 104        | 2.1      | 5224.570094(3)             |                          |
| 2915  | $E$               | 72         | 2.2      | 5224.94883(3)              |                          |
| 2916  | $E$               | 98         | 2.2      | 5224.94883(3)              |                          |
| 2917  | $E$               | 162        | 2.3      | 5224.972575(4)             |                          |
| 2918  | $E$               | 160        | 2.3      | 5224.972576(4)             |                          |
| 2919  | $A_1$             | 79         | 2.2      | 5224.99009(1)              |                          |
| 2920  | $A_2$             | 99         | 2.2      | 5224.990251(9)             |                          |
| 2921  | $A_1$             | 133        | 2.3      | 5225.27310(1)              |                          |
| 2922  | $A_2$             | 123        | 2.2      | 5225.27970(2)              |                          |
| 2923  | $E$               | 88         | 0.38     | 5226.467568(4)             |                          |
| 2924  | $E$               | 101        | 0.37     | 5226.467569(4)             |                          |
| 2925  | $A_2$             | 80         | 0.23     | 5228.719144(2)             |                          |
| 2926  | $A_1$             | 78         | 0.23     | 5228.719147(5)             |                          |
| 2927  | $E$               | 84         | 0.28     | 5235.611235(1)             |                          |
| 2928  | $E$               | 76         | 0.28     | 5235.611235(6)             |                          |
| 2929  | $A_2$             | 49         | 0.22     | 5237.331351(5)             |                          |
| 2930  | $A_1$             | 52         | 0.22     | 5237.331352(4)             |                          |
| 2931  | $E$               | 82         | 0.31     | 5239.747618(1)             |                          |
| 2932  | $E$               | 76         | 0.31     | 5239.747619(1)             |                          |
| 2933  | $A_1$             | 80         | 0.32     | 5241.126601(3)             |                          |
| 2934  | $A_1$             | 78         | 0.51     | 5241.206856(1)             |                          |
| 2935  | $E$               | 99         | 0.065    | 5244.614815(2)             |                          |

Continued on next page.

TABLE S4 – states on Sarka/Poirier CSC PES; continued from previous page

| State | $\Gamma_{C_{3v}}$ | $D_{\max}$ | $S_{vN}$ | $\tilde{E}/\text{cm}^{-1}$ | $\Delta\text{Ref. [30]}$ |
|-------|-------------------|------------|----------|----------------------------|--------------------------|
| 2936  | $E$               | 89         | 0.065    | 5244.614816(3)             |                          |
| 2937  | $E$               | 119        | 0.3      | 5244.762645(4)             |                          |
| 2938  | $E$               | 118        | 0.3      | 5244.762645(3)             |                          |
| 2939  | $E$               | 97         | 0.4      | 5247.242389(1)             |                          |
| 2940  | $E$               | 79         | 0.4      | 5247.242389(2)             |                          |
| 2941  | $E$               | 78         | 0.14     | 5248.195099(2)             |                          |
| 2942  | $E$               | 81         | 0.14     | 5248.195099(1)             |                          |
| 2943  | $E$               | 131        | 2.3      | 5250.216067(6)             |                          |
| 2944  | $E$               | 133        | 2.3      | 5250.216067(6)             |                          |
| 2945  | $A_1$             | 92         | 2.2      | 5250.29312(2)              |                          |
| 2946  | $A_2$             | 93         | 2.2      | 5250.29787(1)              |                          |
| 2947  | $E$               | 94         | 0.38     | 5250.720704(2)             |                          |
| 2948  | $E$               | 82         | 0.38     | 5250.720705(6)             |                          |
| 2949  | $E$               | 84         | 0.34     | 5251.526298(3)             |                          |
| 2950  | $E$               | 71         | 0.34     | 5251.526298(4)             |                          |
| 2951  | $E$               | 64         | 0.13     | 5253.258136(1)             |                          |
| 2952  | $E$               | 51         | 0.13     | 5253.258137(2)             |                          |
| 2953  | $E$               | 89         | 2.3      | 5254.43260(6)              |                          |
| 2954  | $E$               | 105        | 2.3      | 5254.43260(7)              |                          |
| 2955  | $A_1$             | 88         | 2.3      | 5254.44338(6)              |                          |
| 2956  | $A_2$             | 96         | 2.3      | 5254.44339(7)              |                          |
| 2957  | $A_1$             | 71         | 0.14     | 5254.731849(1)             |                          |
| 2958  | $E$               | 88         | 0.9      | 5255.416876(2)             |                          |
| 2959  | $E$               | 87         | 0.89     | 5255.416878(2)             |                          |
| 2960  | $A_1$             | 59         | 0.11     | 5255.68639(1)              |                          |
| 2961  | $A_2$             | 60         | 0.11     | 5255.68640(1)              |                          |
| 2962  | $E$               | 85         | 0.13     | 5258.597047(2)             |                          |
| 2963  | $E$               | 73         | 0.13     | 5258.597047(5)             |                          |
| 2964  | $E$               | 91         | 2.4      | 5258.71133(6)              |                          |
| 2965  | $E$               | 111        | 2.4      | 5258.71134(7)              |                          |
| 2966  | $A_1$             | 89         | 2.4      | 5258.75338(8)              |                          |
| 2967  | $A_2$             | 92         | 2.4      | 5258.75354(5)              |                          |
| 2968  | $A_1$             | 72         | 0.35     | 5259.634675(1)             |                          |
| 2969  | $E$               | 99         | 0.62     | 5260.226977(6)             |                          |
| 2970  | $E$               | 102        | 0.63     | 5260.226978(7)             |                          |
| 2971  | $A_1$             | 95         | 0.61     | 5260.313453(3)             |                          |
| 2972  | $A_2$             | 97         | 0.61     | 5260.313453(3)             |                          |
| 2973  | $A_1$             | 84         | 1.1      | 5260.869323(4)             |                          |
| 2974  | $A_2$             | 82         | 1.1      | 5260.869349(2)             |                          |
| 2975  | $E$               | 99         | 2.2      | 5262.203718(3)             |                          |
| 2976  | $E$               | 120        | 2.2      | 5262.203720(3)             |                          |
| 2977  | $E$               | 95         | 2.2      | 5262.208134(5)             |                          |
| 2978  | $E$               | 100        | 2.2      | 5262.208135(9)             |                          |
| 2979  | $E$               | 94         | 0.43     | 5263.148314(2)             |                          |
| 2980  | $E$               | 91         | 0.43     | 5263.148314(4)             |                          |
| 2981  | $E$               | 92         | 1.3      | 5263.596411(2)             |                          |
| 2982  | $E$               | 91         | 1.3      | 5263.596411(2)             |                          |
| 2983  | $A_2$             | 99         | 2.4      | 5264.880256(5)             |                          |
| 2984  | $E$               | 104        | 2.4      | 5265.092680(7)             |                          |
| 2985  | $E$               | 97         | 2.4      | 5265.092681(9)             |                          |
| 2986  | $A_1$             | 91         | 2.4      | 5265.293109(2)             |                          |
| 2987  | $E$               | 169        | 3.0      | 5266.307624(5)             |                          |
| 2988  | $E$               | 123        | 3.0      | 5266.30764(2)              |                          |
| 2989  | $A_1$             | 122        | 3.2      | 5266.33304(3)              |                          |
| 2990  | $A_2$             | 119        | 3.2      | 5266.33370(4)              |                          |
| 2991  | $E$               | 96         | 0.73     | 5267.168420(3)             |                          |
| 2992  | $E$               | 105        | 0.73     | 5267.168421(2)             |                          |
| 2993  | $E$               | 163        | 1.1      | 5267.893739(5)             |                          |
| 2994  | $E$               | 156        | 1.1      | 5267.893741(4)             |                          |

Continued on next page.

TABLE S4 – states on Sarka/Poirier CSC PES; continued from previous page

| State | $\Gamma_{C_{3v}}$ | $D_{\max}$ | $S_{vN}$ | $\tilde{E}/\text{cm}^{-1}$ | $\Delta\text{Ref. [30]}$ |
|-------|-------------------|------------|----------|----------------------------|--------------------------|
| 2995  | $E$               | 87         | 0.8      | 5271.28261(1)              |                          |
| 2996  | $E$               | 93         | 0.8      | 5271.282615(8)             |                          |
| 2997  | $A_1$             | 103        | 1.3      | 5271.70080(3)              |                          |
| 2998  | $A_2$             | 102        | 1.3      | 5271.70084(4)              |                          |
| 2999  | $A_2^*$           | 61         | 0.49     | 5272.19263(3)              |                          |
| 3000  | $A_1^*$           | 59         | 0.49     | 5272.19263(4)              |                          |
| 3001  | $A_1$             | 97         | 0.82     | 5272.654215(2)             |                          |
| 3002  | $A_1$             | 97         | 0.47     | 5272.921512(3)             |                          |
| 3003  | $E$               | 138        | 2.3      | 5274.37144(1)              |                          |
| 3004  | $E$               | 131        | 2.3      | 5274.371445(7)             |                          |
| 3005  | $E$               | 158        | 1.0      | 5274.483977(4)             |                          |
| 3006  | $E$               | 153        | 1.0      | 5274.483978(3)             |                          |
| 3007  | $A_2$             | 113        | 3.2      | 5275.18692(2)              |                          |
| 3008  | $A_1$             | 123        | 3.2      | 5275.18693(2)              |                          |
| 3009  | $E$               | 181        | 3.1      | 5275.316977(2)             |                          |
| 3010  | $E$               | 177        | 3.1      | 5275.316977(2)             |                          |
| 3011  | $A_1$             | 71         | 0.56     | 5275.615510(2)             |                          |
| 3012  | $E$               | 115        | 2.2      | 5275.68264(3)              |                          |
| 3013  | $E$               | 129        | 2.2      | 5275.68265(3)              |                          |
| 3014  | $E$               | 187        | 4.8      | 5276.464042(4)             |                          |
| 3015  | $E$               | 185        | 4.8      | 5276.464043(4)             |                          |
| 3016  | $E$               | 111        | 2.3      | 5276.787806(5)             |                          |
| 3017  | $E$               | 127        | 2.3      | 5276.787806(4)             |                          |
| 3018  | $E$               | 91         | 2.2      | 5277.058402(8)             |                          |
| 3019  | $E$               | 114        | 2.2      | 5277.058408(9)             |                          |
| 3020  | $E$               | 174        | 2.7      | 5277.083795(3)             |                          |
| 3021  | $E$               | 178        | 2.7      | 5277.083796(3)             |                          |
| 3022  | $A_1$             | 100        | 0.65     | 5277.174756(2)             |                          |
| 3023  | $E$               | 184        | 3.3      | 5277.342447(6)             |                          |
| 3024  | $E$               | 164        | 3.3      | 5277.342455(9)             |                          |
| 3025  | $E$               | 175        | 4.8      | 5278.341762(4)             |                          |
| 3026  | $E$               | 181        | 4.8      | 5278.341765(6)             |                          |
| 3027  | $E$               | 98         | 0.45     | 5278.371683(4)             |                          |
| 3028  | $E$               | 94         | 0.45     | 5278.371684(1)             |                          |
| 3029  | $A_1$             | 176        | 3.0      | 5278.584461(6)             |                          |
| 3030  | $E$               | 83         | 0.54     | 5278.655493(6)             |                          |
| 3031  | $E$               | 93         | 0.54     | 5278.655493(2)             |                          |
| 3032  | $A_2$             | 178        | 3.1      | 5278.756582(4)             |                          |
| 3033  | $E$               | 97         | 0.2      | 5279.788551(2)             |                          |
| 3034  | $E$               | 100        | 0.2      | 5279.788552(1)             |                          |
| 3035  | $A_1$             | 105        | 2.4      | 5280.03166(8)              |                          |
| 3036  | $A_2$             | 104        | 2.4      | 5280.03168(8)              |                          |
| 3037  | $E$               | 165        | 3.0      | 5280.050721(3)             |                          |
| 3038  | $E$               | 180        | 3.0      | 5280.050728(8)             |                          |
| 3039  | $A_1$             | 126        | 4.1      | 5280.32596(4)              |                          |
| 3040  | $A_2$             | 123        | 4.1      | 5280.36231(4)              |                          |
| 3041  | $E$               | 156        | 3.5      | 5280.826909(6)             |                          |
| 3042  | $E$               | 153        | 3.5      | 5280.826913(4)             |                          |
| 3043  | $E$               | 166        | 3.3      | 5280.967845(8)             |                          |
| 3044  | $E$               | 147        | 3.3      | 5280.96786(1)              |                          |
| 3045  | $A_1$             | 103        | 2.3      | 5281.34004(3)              |                          |
| 3046  | $A_2$             | 106        | 2.3      | 5281.34005(2)              |                          |
| 3047  | $E$               | 78         | 0.56     | 5282.534281(5)             |                          |
| 3048  | $E$               | 88         | 0.56     | 5282.534281(3)             |                          |
| 3049  | $E$               | 144        | 2.5      | 5282.80111(1)              |                          |
| 3050  | $E$               | 138        | 2.5      | 5282.80111(1)              |                          |
| 3051  | $A_1$             | 110        | 3.4      | 5283.79605(5)              |                          |
| 3052  | $A_2$             | 106        | 3.4      | 5283.79967(4)              |                          |
| 3053  | $A_1$             | 78         | 0.57     | 5283.827388(1)             |                          |

Continued on next page.

TABLE S4 – states on Sarka/Poirier CSC PES; continued from previous page

| State | $\Gamma_{C_{3v}}$ | $D_{\max}$ | $S_{vN}$ | $\tilde{E}/\text{cm}^{-1}$ | $\Delta\text{Ref. [30]}$ |
|-------|-------------------|------------|----------|----------------------------|--------------------------|
| 3054  | $E$               | 140        | 2.9      | 5283.866553(3)             |                          |
| 3055  | $E$               | 135        | 2.9      | 5283.866553(4)             |                          |
| 3056  | $E$               | 129        | 2.4      | 5284.185990(2)             |                          |
| 3057  | $E$               | 129        | 2.4      | 5284.185991(3)             |                          |
| 3058  | $E$               | 109        | 0.24     | 5284.215362(2)             |                          |
| 3059  | $E$               | 111        | 0.24     | 5284.215362(2)             |                          |
| 3060  | $A_2$             | 113        | 2.0      | 5285.326281(2)             |                          |
| 3061  | $A_1$             | 108        | 2.0      | 5285.369714(1)             |                          |
| 3062  | $E$               | 104        | 2.0      | 5285.501813(2)             |                          |
| 3063  | $E$               | 109        | 2.0      | 5285.501813(1)             |                          |
| 3064  | $A_2$             | 84         | 2.5      | 5287.62870(5)              |                          |
| 3065  | $A_1$             | 91         | 2.5      | 5287.62870(5)              |                          |
| 3066  | $E$               | 89         | 2.5      | 5287.85183(1)              |                          |
| 3067  | $E$               | 102        | 2.5      | 5287.85184(2)              |                          |
| 3068  | $A_1$             | 150        | 2.8      | 5291.769594(3)             |                          |
| 3069  | $E$               | 149        | 2.7      | 5291.891654(4)             |                          |
| 3070  | $E$               | 152        | 2.7      | 5291.891654(4)             |                          |
| 3071  | $A_2$             | 144        | 2.6      | 5291.967745(3)             |                          |
| 3072  | $E$               | 156        | 2.4      | 5293.610803(3)             |                          |
| 3073  | $E$               | 165        | 2.4      | 5293.610806(4)             |                          |
| 3074  | $E$               | 116        | 2.1      | 5293.90013(2)              |                          |
| 3075  | $E$               | 119        | 2.1      | 5293.90013(2)              |                          |
| 3076  | $A_1$             | 118        | 1.2      | 5295.732685(2)             |                          |
| 3077  | $E$               | 103        | 2.7      | 5295.76615(3)              |                          |
| 3078  | $E$               | 102        | 2.7      | 5295.76615(3)              |                          |
| 3079  | $A_1$             | 88         | 2.7      | 5295.94619(6)              |                          |
| 3080  | $A_2$             | 88         | 2.7      | 5295.94619(7)              |                          |
| 3081  | $A_2$             | 106        | 2.3      | 5296.59171(4)              |                          |
| 3082  | $A_1$             | 102        | 2.3      | 5296.60146(5)              |                          |
| 3083  | $E$               | 139        | 2.2      | 5296.69392(1)              |                          |
| 3084  | $E$               | 108        | 2.2      | 5296.69392(6)              |                          |
| 3085  | $E$               | 151        | 3.2      | 5298.980824(3)             |                          |
| 3086  | $E$               | 139        | 3.2      | 5298.980825(5)             |                          |
| 3087  | $A_2$             | 156        | 3.2      | 5298.987738(2)             |                          |
| 3088  | $A_1$             | 152        | 3.2      | 5299.056262(4)             |                          |
| 3089  | $E$               | 127        | 2.2      | 5299.338072(7)             |                          |
| 3090  | $E$               | 134        | 2.2      | 5299.338072(5)             |                          |
| 3091  | $E$               | 146        | 2.2      | 5299.357310(3)             |                          |
| 3092  | $E$               | 138        | 2.2      | 5299.357310(5)             |                          |
| 3093  | $A_1$             | 111        | 2.3      | 5300.19085(1)              |                          |
| 3094  | $A_2$             | 107        | 2.3      | 5300.19085(1)              |                          |
| 3095  | $E$               | 105        | 2.2      | 5300.36004(2)              |                          |
| 3096  | $E$               | 106        | 2.2      | 5300.36004(2)              |                          |
| 3097  | $E$               | 150        | 4.3      | 5300.635262(3)             |                          |
| 3098  | $E$               | 148        | 4.3      | 5300.635263(2)             |                          |
| 3099  | $A_1$             | 144        | 2.8      | 5300.985637(2)             |                          |
| 3100  | $A_2$             | 142        | 2.1      | 5301.123111(2)             |                          |
| 3101  | $E$               | 101        | 2.8      | 5301.18484(3)              |                          |
| 3102  | $E$               | 160        | 2.8      | 5301.18484(3)              |                          |
| 3103  | $E$               | 159        | 2.8      | 5301.340190(2)             |                          |
| 3104  | $E$               | 138        | 2.8      | 5301.340190(5)             |                          |
| 3105  | $E$               | 140        | 3.8      | 5301.680729(3)             |                          |
| 3106  | $E$               | 142        | 3.8      | 5301.680730(3)             |                          |
| 3107  | $E$               | 77         | 1.8      | 5303.293815(5)             |                          |
| 3108  | $E$               | 79         | 1.8      | 5303.293815(5)             |                          |
| 3109  | $A_1$             | 99         | 2.9      | 5303.60402(2)              |                          |
| 3110  | $E$               | 92         | 2.8      | 5304.04291(1)              |                          |
| 3111  | $E$               | 87         | 2.8      | 5304.04291(3)              |                          |
| 3112  | $A_2$             | 92         | 2.8      | 5304.331285(5)             |                          |

Continued on next page.

TABLE S4 – states on Sarka/Poirier CSC PES; continued from previous page

| State | $\Gamma_{C_{3v}}$ | $D_{\max}$ | $S_{vN}$ | $\tilde{E}/\text{cm}^{-1}$ | $\Delta\text{Ref. [30]}$ |
|-------|-------------------|------------|----------|----------------------------|--------------------------|
| 3113  | $E$               | 104        | 2.3      | 5304.52953(2)              |                          |
| 3114  | $E$               | 105        | 2.3      | 5304.52953(2)              |                          |
| 3115  | $A_1$             | 91         | 2.2      | 5304.64404(5)              |                          |
| 3116  | $A_2$             | 98         | 2.2      | 5304.64420(2)              |                          |
| 3117  | $A_1$             | 67         | 1.8      | 5304.76501(1)              |                          |
| 3118  | $E$               | 95         | 0.36     | 5306.06389(1)              |                          |
| 3119  | $E$               | 103        | 0.38     | 5306.06390(1)              |                          |
| 3120  | $A_1$             | 90         | 0.72     | 5309.341925(1)             |                          |
| 3121  | $E$               | 81         | 2.9      | 5311.270827(2)             |                          |
| 3122  | $E$               | 60         | 2.9      | 5311.270827(6)             |                          |
| 3123  | $E$               | 119        | 0.54     | 5311.928397(8)             |                          |
| 3124  | $E$               | 131        | 0.54     | 5311.928398(8)             |                          |
| 3125  | $E$               | 108        | 0.49     | 5312.107451(6)             |                          |
| 3126  | $E$               | 99         | 0.49     | 5312.10746(1)              |                          |
| 3127  | $A_1$             | 77         | 2.1      | 5313.18795(9)              |                          |
| 3128  | $A_2$             | 74         | 2.1      | 5313.1883(1)               |                          |
| 3129  | $E$               | 88         | 2.1      | 5313.20132(4)              |                          |
| 3130  | $E$               | 79         | 2.1      | 5313.20133(7)              |                          |
| 3131  | $E$               | 86         | 0.14     | 5314.667329(5)             |                          |
| 3132  | $E$               | 74         | 0.14     | 5314.667330(8)             |                          |
| 3133  | $E$               | 85         | 1.8      | 5316.667691(3)             |                          |
| 3134  | $E$               | 97         | 1.8      | 5316.667691(3)             |                          |
| 3135  | $A_1$             | 91         | 1.8      | 5318.133867(2)             |                          |
| 3136  | $E$               | 61         | 3.0      | 5319.82560(1)              |                          |
| 3137  | $E$               | 59         | 3.0      | 5319.825606(8)             |                          |
| 3138  | $E$               | 94         | 2.6      | 5320.51280(1)              |                          |
| 3139  | $E$               | 95         | 2.6      | 5320.51281(1)              |                          |
| 3140  | $E$               | 95         | 2.5      | 5320.590611(9)             |                          |
| 3141  | $E$               | 92         | 2.5      | 5320.590614(4)             |                          |
| 3142  | $A_1$             | 118        | 2.7      | 5321.490008(4)             |                          |
| 3143  | $E$               | 118        | 2.6      | 5321.571667(2)             |                          |
| 3144  | $E$               | 102        | 2.6      | 5321.571669(6)             |                          |
| 3145  | $A_2$             | 94         | 2.6      | 5321.610446(6)             |                          |
| 3146  | $A_1$             | 121        | 2.6      | 5323.305214(4)             |                          |
| 3147  | $E$               | 93         | 2.6      | 5323.469305(7)             |                          |
| 3148  | $E$               | 102        | 2.6      | 5323.469308(7)             |                          |
| 3149  | $A_2$             | 92         | 2.5      | 5323.574495(4)             |                          |
| 3150  | $A_2$             | 109        | 2.1      | 5324.741671(2)             |                          |
| 3151  | $E$               | 114        | 2.1      | 5325.608135(1)             |                          |
| 3152  | $E$               | 113        | 2.1      | 5325.608135(1)             |                          |
| 3153  | $A_1$             | 106        | 2.1      | 5325.991213(2)             |                          |
| 3154  | $E$               | 131        | 0.57     | 5327.54479(1)              |                          |
| 3155  | $E$               | 100        | 0.57     | 5327.54480(5)              |                          |
| 3156  | $E$               | 93         | 2.4      | 5328.84444(1)              |                          |
| 3157  | $E$               | 96         | 2.4      | 5328.84444(1)              |                          |
| 3158  | $A_1$             | 133        | 2.3      | 5328.888587(2)             |                          |
| 3159  | $A_2$             | 94         | 2.3      | 5328.888639(2)             |                          |
| 3160  | $E$               | 109        | 0.5      | 5330.315364(3)             |                          |
| 3161  | $E$               | 80         | 0.49     | 5330.315369(5)             |                          |
| 3162  | $A_1$             | 79         | 2.1      | 5330.45871(3)              |                          |
| 3163  | $A_2$             | 77         | 2.1      | 5330.45873(3)              |                          |
| 3164  | $E$               | 112        | 3.1      | 5330.91485(1)              |                          |
| 3165  | $E$               | 112        | 3.1      | 5330.91485(1)              |                          |
| 3166  | $E$               | 125        | 3.0      | 5330.981582(4)             |                          |
| 3167  | $E$               | 140        | 3.0      | 5330.981582(3)             |                          |
| 3168  | $A_1$             | 80         | 2.1      | 5331.48799(1)              |                          |
| 3169  | $A_2$             | 83         | 2.1      | 5331.48803(1)              |                          |
| 3170  | $A_1$             | 114        | 3.6      | 5332.7194(2)               |                          |
| 3171  | $A_2$             | 113        | 3.6      | 5332.7194(1)               |                          |

Continued on next page.

TABLE S4 – states on Sarka/Poirier CSC PES; continued from previous page

| State | $\Gamma_{C_{3v}}$ | $D_{\max}$ | $S_{vN}$ | $\tilde{E}/\text{cm}^{-1}$ | $\Delta\text{Ref. [30]}$ |
|-------|-------------------|------------|----------|----------------------------|--------------------------|
| 3172  | $E$               | 140        | 2.4      | 5333.189123(2)             |                          |
| 3173  | $E$               | 137        | 2.4      | 5333.189125(3)             |                          |
| 3174  | $E$               | 136        | 2.2      | 5333.349767(2)             |                          |
| 3175  | $E$               | 105        | 2.2      | 5333.349768(4)             |                          |
| 3176  | $A_1$             | 137        | 2.3      | 5333.364623(5)             |                          |
| 3177  | $A_2$             | 142        | 2.3      | 5333.36466(3)              |                          |
| 3178  | $E$               | 93         | 2.9      | 5333.843538(6)             |                          |
| 3179  | $E$               | 84         | 2.9      | 5333.84354(2)              |                          |
| 3180  | $A_1$             | 84         | 3.1      | 5333.86417(5)              |                          |
| 3181  | $A_2$             | 88         | 3.1      | 5333.87343(2)              |                          |
| 3182  | $E$               | 105        | 2.1      | 5334.411658(6)             |                          |
| 3183  | $E$               | 106        | 2.1      | 5334.411658(5)             |                          |
| 3184  | $E$               | 132        | 0.82     | 5336.03815(1)              |                          |
| 3185  | $E$               | 176        | 0.81     | 5336.03816(1)              |                          |
| 3186  | $E$               | 104        | 0.51     | 5337.214089(8)             |                          |
| 3187  | $E$               | 117        | 0.51     | 5337.214093(9)             |                          |
| 3188  | $A_1$             | 89         | 2.1      | 5338.295845(5)             |                          |
| 3189  | $A_2$             | 94         | 2.1      | 5338.295850(5)             |                          |
| 3190  | $E$               | 92         | 2.2      | 5338.33382(1)              |                          |
| 3191  | $E$               | 87         | 2.2      | 5338.33382(1)              |                          |
| 3192  | $E$               | 143        | 2.7      | 5338.65504(1)              |                          |
| 3193  | $E$               | 144        | 2.7      | 5338.65504(1)              |                          |
| 3194  | $E$               | 144        | 2.4      | 5338.82837(1)              |                          |
| 3195  | $E$               | 149        | 2.4      | 5338.82838(1)              |                          |
| 3196  | $E$               | 125        | 0.8      | 5341.477815(4)             |                          |
| 3197  | $E$               | 113        | 0.8      | 5341.477823(8)             |                          |
| 3198  | $E$               | 135        | 2.4      | 5341.556183(5)             |                          |
| 3199  | $E$               | 137        | 2.4      | 5341.556188(7)             |                          |
| 3200  | $A_1$             | 114        | 2.5      | 5341.61045(3)              |                          |
| 3201  | $A_2$             | 110        | 2.4      | 5341.62286(4)              |                          |
| 3202  | $A_1$             | 112        | 0.76     | 5342.91170(1)              |                          |
| 3203  | $E$               | 106        | 2.8      | 5343.37015(3)              |                          |
| 3204  | $E$               | 110        | 2.8      | 5343.37015(3)              |                          |
| 3205  | $E$               | 107        | 2.8      | 5343.48089(3)              |                          |
| 3206  | $E$               | 106        | 2.8      | 5343.48090(2)              |                          |
| 3207  | $E$               | 148        | 2.4      | 5343.557980(2)             |                          |
| 3208  | $E$               | 148        | 2.4      | 5343.557980(2)             |                          |
| 3209  | $E$               | 146        | 2.4      | 5343.759798(6)             |                          |
| 3210  | $E$               | 154        | 2.4      | 5343.759803(8)             |                          |
| 3211  | $A_2$             | 96         | 2.1      | 5344.20021(1)              |                          |
| 3212  | $A_1$             | 92         | 2.1      | 5344.20021(1)              |                          |
| 3213  | $E$               | 136        | 2.3      | 5344.269672(9)             |                          |
| 3214  | $E$               | 135        | 2.3      | 5344.269674(3)             |                          |
| 3215  | $A_1$             | 106        | 3.0      | 5346.14130(3)              |                          |
| 3216  | $E$               | 106        | 2.8      | 5346.35122(1)              |                          |
| 3217  | $E$               | 103        | 2.8      | 5346.35122(1)              |                          |
| 3218  | $A_2$             | 97         | 2.8      | 5346.477235(2)             |                          |
| 3219  | $A_2$             | 174        | 2.8      | 5346.657893(6)             |                          |
| 3220  | $E$               | 162        | 2.7      | 5346.795772(8)             |                          |
| 3221  | $E$               | 176        | 2.7      | 5346.79577(1)              |                          |
| 3222  | $A_1$             | 170        | 2.6      | 5346.946865(7)             |                          |
| 3223  | $E$               | 105        | 2.4      | 5347.89513(1)              |                          |
| 3224  | $E$               | 92         | 2.4      | 5347.89513(1)              |                          |
| 3225  | $E$               | 101        | 2.4      | 5347.90124(1)              |                          |
| 3226  | $E$               | 110        | 2.4      | 5347.90124(1)              |                          |
| 3227  | $E$               | 109        | 2.2      | 5348.51706(1)              |                          |
| 3228  | $E$               | 102        | 2.2      | 5348.51706(2)              |                          |
| 3229  | $A_2$             | 94         | 2.2      | 5348.53038(2)              |                          |
| 3230  | $A_1$             | 140        | 2.3      | 5348.572841(2)             |                          |

Continued on next page.



TABLE S4 – states on Sarka/Poirier CSC PES; continued from previous page

| State | $\Gamma_{C_{3v}}$ | $D_{\max}$ | $S_{vN}$ | $\tilde{E}/\text{cm}^{-1}$ | $\Delta\text{Ref. [30]}$ |
|-------|-------------------|------------|----------|----------------------------|--------------------------|
| 3231  | $E$               | 117        | 0.26     | 5349.967763(4)             |                          |
| 3232  | $E$               | 115        | 0.26     | 5349.967763(4)             |                          |
| 3233  | $E$               | 65         | 2.1      | 5350.15739(4)              |                          |
| 3234  | $E$               | 68         | 2.1      | 5350.15740(4)              |                          |
| 3235  | $A_1$             | 73         | 2.1      | 5350.16060(2)              |                          |
| 3236  | $A_2$             | 63         | 2.1      | 5350.16747(5)              |                          |
| 3237  | $A_1$             | 119        | 2.5      | 5350.53730(8)              |                          |
| 3238  | $A_2$             | 189        | 2.5      | 5350.53734(9)              |                          |
| 3239  | $E$               | 153        | 2.4      | 5350.736292(8)             |                          |
| 3240  | $E$               | 161        | 2.4      | 5350.73630(1)              |                          |
| 3241  | $A_1$             | 176        | 3.6      | 5352.277314(4)             |                          |
| 3242  | $E$               | 186        | 3.6      | 5352.336673(4)             |                          |
| 3243  | $E$               | 187        | 3.6      | 5352.336673(6)             |                          |
| 3244  | $A_2$             | 122        | 3.6      | 5352.35183(5)              |                          |
| 3245  | $E$               | 165        | 2.9      | 5352.665367(4)             |                          |
| 3246  | $E$               | 175        | 2.9      | 5352.665369(5)             |                          |
| 3247  | $E$               | 177        | 3.1      | 5352.677581(3)             |                          |
| 3248  | $E$               | 157        | 3.1      | 5352.677586(8)             |                          |
| 3249  | $E$               | 118        | 0.46     | 5354.32772(1)              |                          |
| 3250  | $E$               | 122        | 0.47     | 5354.32772(1)              |                          |
| 3251  | $A_1$             | 110        | 2.3      | 5354.37969(9)              |                          |
| 3252  | $A_2$             | 120        | 2.3      | 5354.37969(8)              |                          |
| 3253  | $E$               | 157        | 2.5      | 5354.66994(1)              |                          |
| 3254  | $E$               | 149        | 2.5      | 5354.66994(1)              |                          |
| 3255  | $A_2$             | 86         | 2.5      | 5354.72219(6)              |                          |
| 3256  | $A_1$             | 87         | 2.5      | 5354.72220(5)              |                          |
| 3257  | $E$               | 108        | 2.5      | 5354.76251(1)              |                          |
| 3258  | $E$               | 108        | 2.5      | 5354.76251(1)              |                          |
| 3259  | $A_1$             | 140        | 2.2      | 5354.895901(3)             |                          |
| 3260  | $A_2$             | 148        | 2.2      | 5354.895936(3)             |                          |
| 3261  | $A_1$             | 135        | 2.6      | 5354.92958(4)              |                          |
| 3262  | $A_2$             | 130        | 2.6      | 5354.93166(5)              |                          |
| 3263  | $E$               | 186        | 2.6      | 5355.950636(3)             |                          |
| 3264  | $E$               | 171        | 2.6      | 5355.950639(6)             |                          |
| 3265  | $E$               | 156        | 0.89     | 5356.393328(9)             |                          |
| 3266  | $E$               | 149        | 0.9      | 5356.393332(4)             |                          |
| 3267  | $A_2$             | 175        | 4.1      | 5357.04791(1)              |                          |
| 3268  | $A_1$             | 173        | 3.4      | 5357.325771(9)             |                          |
| 3269  | $E$               | 164        | 3.7      | 5357.40573(1)              |                          |
| 3270  | $E$               | 192        | 3.7      | 5357.40574(1)              |                          |
| 3271  | $A_1$             | 78         | 0.23     | 5357.432371(1)             |                          |
| 3272  | $A_2$             | 96         | 0.22     | 5357.432372(1)             |                          |
| 3273  | $A_2$             | 178        | 3.6      | 5357.68916(1)              |                          |
| 3274  | $E$               | 177        | 2.5      | 5358.526378(3)             |                          |
| 3275  | $E$               | 171        | 2.5      | 5358.526379(3)             |                          |
| 3276  | $E$               | 128        | 1.0      | 5358.54987(1)              |                          |
| 3277  | $E$               | 173        | 1.1      | 5358.54987(1)              |                          |
| 3278  | $E$               | 104        | 2.6      | 5358.73820(1)              |                          |
| 3279  | $E$               | 141        | 2.6      | 5358.73820(1)              |                          |
| 3280  | $E$               | 164        | 2.4      | 5358.827318(4)             |                          |
| 3281  | $E$               | 163        | 2.4      | 5358.827319(5)             |                          |
| 3282  | $A_1$             | 91         | 2.6      | 5358.90183(3)              |                          |
| 3283  | $A_2$             | 85         | 2.6      | 5358.90239(5)              |                          |
| 3284  | $E$               | 130        | 2.7      | 5359.681130(8)             |                          |
| 3285  | $E$               | 138        | 2.7      | 5359.68113(1)              |                          |
| 3286  | $A_1^*$           | 101        | 2.2      | 5359.85288(5)              |                          |
| 3287  | $A_2^*$           | 103        | 2.2      | 5359.85288(5)              |                          |
| 3288  | $A_1$             | 171        | 2.5      | 5359.973223(3)             |                          |
| 3289  | $A_1$             | 110        | 0.87     | 5359.98429(2)              |                          |

Continued on next page.

TABLE S4 – states on Sarka/Poirier CSC PES; continued from previous page

| State | $\Gamma_{C_{3v}}$ | $D_{\max}$ | $S_{vN}$ | $\tilde{E}/\text{cm}^{-1}$ | $\Delta\text{Ref. [30]}$ |
|-------|-------------------|------------|----------|----------------------------|--------------------------|
| 3290  | $E$               | 132        | 1.1      | 5360.367584(3)             |                          |
| 3291  | $E$               | 103        | 1.1      | 5360.36759(1)              |                          |
| 3292  | $E$               | 134        | 2.1      | 5361.46946(1)              |                          |
| 3293  | $E$               | 155        | 2.1      | 5361.46947(1)              |                          |
| 3294  | $E$               | 153        | 1.9      | 5361.834951(6)             |                          |
| 3295  | $E$               | 170        | 1.9      | 5361.834957(9)             |                          |
| 3296  | $E$               | 63         | 0.14     | 5361.97862(1)              |                          |
| 3297  | $E$               | 66         | 0.14     | 5361.97862(1)              |                          |
| 3298  | $E$               | 100        | 0.69     | 5362.230660(1)             |                          |
| 3299  | $E$               | 96         | 0.69     | 5362.230661(2)             |                          |
| 3300  | $A_2$             | 165        | 2.5      | 5363.965918(6)             |                          |
| 3301  | $A_1$             | 124        | 2.6      | 5363.993756(4)             |                          |
| 3302  | $E$               | 117        | 2.4      | 5364.073701(5)             |                          |
| 3303  | $E$               | 137        | 2.4      | 5364.07372(2)              |                          |
| 3304  | $E$               | 109        | 0.53     | 5365.448887(5)             |                          |
| 3305  | $E$               | 118        | 0.53     | 5365.448893(8)             |                          |
| 3306  | $E$               | 123        | 1.6      | 5365.74476(2)              |                          |
| 3307  | $E$               | 150        | 1.6      | 5365.74476(2)              |                          |
| 3308  | $E$               | 146        | 1.5      | 5365.976905(2)             |                          |
| 3309  | $E$               | 153        | 1.5      | 5365.976911(6)             |                          |
| 3310  | $A_1$             | 129        | 0.34     | 5367.181633(6)             |                          |
| 3311  | $A_2$             | 128        | 0.33     | 5367.346063(6)             |                          |
| 3312  | $A_2$             | 169        | 3.3      | 5368.018073(7)             |                          |
| 3313  | $A_1$             | 172        | 3.3      | 5368.019564(6)             |                          |
| 3314  | $E$               | 154        | 3.1      | 5368.15736(2)              |                          |
| 3315  | $E$               | 170        | 3.1      | 5368.15736(2)              |                          |
| 3316  | $E$               | 176        | 3.3      | 5368.622200(7)             |                          |
| 3317  | $E$               | 185        | 3.3      | 5368.622201(8)             |                          |
| 3318  | $A_2$             | 123        | 3.0      | 5368.76659(3)              |                          |
| 3319  | $A_1$             | 173        | 3.0      | 5368.76660(4)              |                          |
| 3320  | $E$               | 139        | 2.1      | 5368.976680(5)             |                          |
| 3321  | $E$               | 94         | 2.1      | 5368.976682(9)             |                          |
| 3322  | $E$               | 94         | 2.1      | 5368.97971(1)              |                          |
| 3323  | $E$               | 96         | 2.1      | 5368.97971(1)              |                          |
| 3324  | $E$               | 132        | 2.2      | 5369.57213(3)              |                          |
| 3325  | $E$               | 169        | 2.2      | 5369.57213(4)              |                          |
| 3326  | $E$               | 95         | 0.51     | 5370.077087(4)             |                          |
| 3327  | $E$               | 101        | 0.51     | 5370.077088(4)             |                          |
| 3328  | $E$               | 130        | 2.1      | 5370.17322(4)              |                          |
| 3329  | $E$               | 126        | 2.1      | 5370.17323(4)              |                          |
| 3330  | $E$               | 92         | 0.2      | 5370.336026(2)             |                          |
| 3331  | $E$               | 75         | 0.2      | 5370.336026(6)             |                          |
| 3332  | $A_2$             | 101        | 2.1      | 5371.69164(2)              |                          |
| 3333  | $E$               | 84         | 0.64     | 5371.807939(6)             |                          |
| 3334  | $E$               | 98         | 0.64     | 5371.807940(3)             |                          |
| 3335  | $E$               | 109        | 2.1      | 5371.90304(1)              |                          |
| 3336  | $E$               | 110        | 2.1      | 5371.90304(1)              |                          |
| 3337  | $A_1$             | 107        | 2.1      | 5372.102014(2)             |                          |
| 3338  | $E$               | 91         | 0.6      | 5374.376124(5)             |                          |
| 3339  | $E$               | 98         | 0.6      | 5374.376125(5)             |                          |
| 3340  | $A_2$             | 55         | 0.5      | 5374.64221(2)              |                          |
| 3341  | $A_1$             | 54         | 0.5      | 5374.64221(3)              |                          |
| 3342  | $E$               | 81         | 0.46     | 5375.373005(2)             |                          |
| 3343  | $E$               | 92         | 0.46     | 5375.373006(2)             |                          |
| 3344  | $A_1$             | 98         | 0.63     | 5375.809354(5)             |                          |
| 3345  | $A_1$             | 87         | 0.23     | 5375.909304(3)             |                          |
| 3346  | $A_2$             | 83         | 0.23     | 5375.909333(4)             |                          |
| 3347  | $A_1$             | 92         | 0.051    | 5376.125183(2)             |                          |
| 3348  | $A_2$             | 96         | 0.051    | 5376.131510(1)             |                          |

Continued on next page.

TABLE S4 – states on Sarka/Poirier CSC PES; continued from previous page

| State | $\Gamma_{C_{3v}}$ | $D_{\max}$ | $S_{vN}$ | $\tilde{E}/\text{cm}^{-1}$ | $\Delta\text{Ref. [30]}$ |
|-------|-------------------|------------|----------|----------------------------|--------------------------|
| 3349  | $E$               | 99         | 0.25     | 5378.696546(1)             |                          |
| 3350  | $E$               | 87         | 0.25     | 5378.696546(3)             |                          |
| 3351  | $A_1$             | 57         | 0.91     | 5380.90919(4)              |                          |
| 3352  | $A_2$             | 59         | 0.91     | 5380.90921(5)              |                          |
| 3353  | $E$               | 95         | 0.65     | 5381.653680(1)             |                          |
| 3354  | $E$               | 87         | 0.65     | 5381.653680(1)             |                          |
| 3355  | $E$               | 88         | 0.9      | 5383.578967(7)             |                          |
| 3356  | $E$               | 93         | 0.9      | 5383.578967(3)             |                          |
| 3357  | $E$               | 77         | 1.1      | 5383.678288(3)             |                          |
| 3358  | $E$               | 78         | 1.1      | 5383.678288(2)             |                          |
| 3359  | $E$               | 120        | 0.31     | 5385.144472(2)             |                          |
| 3360  | $E$               | 117        | 0.31     | 5385.144473(2)             |                          |
| 3361  | $E$               | 81         | 0.73     | 5385.861876(2)             |                          |
| 3362  | $E$               | 91         | 0.73     | 5385.861876(2)             |                          |
| 3363  | $A_1$             | 83         | 0.75     | 5387.264821(2)             |                          |
| 3364  | $E$               | 74         | 2.0      | 5388.329595(4)             |                          |
| 3365  | $E$               | 70         | 2.0      | 5388.329595(5)             |                          |
| 3366  | $E$               | 68         | 2.0      | 5388.361424(7)             |                          |
| 3367  | $E$               | 72         | 2.0      | 5388.361424(5)             |                          |
| 3368  | $E$               | 110        | 2.1      | 5390.680348(2)             |                          |
| 3369  | $E$               | 107        | 2.1      | 5390.680348(3)             |                          |
| 3370  | $E$               | 68         | 2.4      | 5390.74450(5)              |                          |
| 3371  | $E$               | 97         | 2.4      | 5390.74451(4)              |                          |
| 3372  | $A_1$             | 80         | 2.4      | 5390.74889(1)              |                          |
| 3373  | $A_2$             | 76         | 2.4      | 5390.74892(1)              |                          |
| 3374  | $A_1$             | 106        | 2.1      | 5390.982570(4)             |                          |
| 3375  | $A_2$             | 93         | 2.1      | 5390.988396(8)             |                          |
| 3376  | $E$               | 79         | 0.52     | 5392.236867(3)             |                          |
| 3377  | $E$               | 106        | 0.5      | 5392.236873(7)             |                          |
| 3378  | $A_1^*$           | 65         | 1.1      | 5392.73995(6)              |                          |
| 3379  | $A_2^*$           | 67         | 1.1      | 5392.73995(4)              |                          |
| 3380  | $E$               | 81         | 2.1      | 5395.36770(5)              |                          |
| 3381  | $E$               | 115        | 2.1      | 5395.36770(6)              |                          |
| 3382  | $A_1^*$           | 75         | 2.1      | 5395.38900(6)              |                          |
| 3383  | $A_2^*$           | 75         | 2.1      | 5395.38900(5)              |                          |
| 3384  | $E$               | 79         | 0.7      | 5396.623665(1)             |                          |
| 3385  | $E$               | 86         | 0.7      | 5396.623666(2)             |                          |
| 3386  | $A_2$             | 85         | 0.72     | 5397.601465(3)             |                          |
| 3387  | $A_1$             | 73         | 0.72     | 5397.601465(8)             |                          |
| 3388  | $E$               | 90         | 1.2      | 5399.286555(7)             |                          |
| 3389  | $E$               | 93         | 1.2      | 5399.286555(6)             |                          |
| 3390  | $E$               | 104        | 2.1      | 5399.305306(2)             |                          |
| 3391  | $E$               | 92         | 2.1      | 5399.305306(7)             |                          |
| 3392  | $A_1$             | 74         | 2.1      | 5399.59283(5)              |                          |
| 3393  | $A_2$             | 73         | 2.1      | 5399.59490(4)              |                          |
| 3394  | $E$               | 85         | 2.1      | 5399.60449(1)              |                          |
| 3395  | $E$               | 89         | 2.1      | 5399.60449(2)              |                          |
| 3396  | $E$               | 103        | 2.3      | 5399.91290(1)              |                          |
| 3397  | $E$               | 121        | 2.3      | 5399.91290(1)              |                          |
| 3398  | $A_2$             | 92         | 3.2      | 5399.934550(7)             |                          |
| 3399  | $E$               | 101        | 3.0      | 5399.937475(6)             |                          |
| 3400  | $E$               | 105        | 3.0      | 5399.937476(5)             |                          |
| 3401  | $A_1$             | 85         | 3.1      | 5399.951900(7)             |                          |
| 3402  | $A_2$             | 98         | 2.2      | 5400.20287(1)              |                          |
| 3403  | $A_1$             | 103        | 2.2      | 5400.20287(1)              |                          |
| 3404  | $E$               | 102        | 2.2      | 5400.673418(2)             |                          |
| 3405  | $E$               | 108        | 2.2      | 5400.673420(2)             |                          |
| 3406  | $E$               | 145        | 2.4      | 5400.729534(6)             |                          |
| 3407  | $E$               | 149        | 2.4      | 5400.729537(7)             |                          |

Continued on next page.

TABLE S4 – states on Sarka/Poirier CSC PES; continued from previous page

| State | $\Gamma_{C_{3v}}$ | $D_{\max}$ | $S_{vN}$ | $\tilde{E}/\text{cm}^{-1}$ | $\Delta\text{Ref. [30]}$ |
|-------|-------------------|------------|----------|----------------------------|--------------------------|
| 3408  | $A_2$             | 116        | 2.3      | 5400.806506(3)             |                          |
| 3409  | $E$               | 70         | 0.13     | 5401.006514(4)             |                          |
| 3410  | $E$               | 95         | 0.12     | 5401.006516(4)             |                          |
| 3411  | $E$               | 108        | 2.2      | 5401.437274(2)             |                          |
| 3412  | $E$               | 110        | 2.2      | 5401.437275(2)             |                          |
| 3413  | $E$               | 152        | 3.4      | 5401.535193(3)             |                          |
| 3414  | $E$               | 161        | 3.4      | 5401.535195(5)             |                          |
| 3415  | $A_2$             | 113        | 3.2      | 5401.67834(3)              |                          |
| 3416  | $A_1$             | 132        | 3.2      | 5401.67835(4)              |                          |
| 3417  | $E$               | 140        | 2.3      | 5402.021980(2)             |                          |
| 3418  | $E$               | 143        | 2.3      | 5402.021983(4)             |                          |
| 3419  | $A_1$             | 100        | 2.1      | 5402.165269(1)             |                          |
| 3420  | $E$               | 94         | 1.3      | 5403.215755(5)             |                          |
| 3421  | $E$               | 82         | 1.3      | 5403.215756(5)             |                          |
| 3422  | $A_1$             | 86         | 1.3      | 5404.525693(5)             |                          |
| 3423  | $E$               | 85         | 0.97     | 5404.573125(5)             |                          |
| 3424  | $E$               | 107        | 0.97     | 5404.573126(4)             |                          |
| 3425  | $E$               | 195        | 2.5      | 5405.042649(4)             |                          |
| 3426  | $E$               | 151        | 2.5      | 5405.04266(1)              |                          |
| 3427  | $A_2$             | 96         | 2.2      | 5405.236446(6)             |                          |
| 3428  | $E$               | 108        | 2.2      | 5405.336483(3)             |                          |
| 3429  | $E$               | 111        | 2.2      | 5405.336483(3)             |                          |
| 3430  | $A_1$             | 74         | 2.2      | 5405.446374(4)             |                          |
| 3431  | $A_2$             | 167        | 3.9      | 5405.668015(8)             |                          |
| 3432  | $A_1$             | 151        | 3.3      | 5405.903113(5)             |                          |
| 3433  | $E$               | 166        | 3.3      | 5405.97996(1)              |                          |
| 3434  | $E$               | 160        | 3.3      | 5405.97997(1)              |                          |
| 3435  | $E$               | 153        | 2.3      | 5406.33587(1)              |                          |
| 3436  | $E$               | 143        | 2.3      | 5406.335878(5)             |                          |
| 3437  | $A_2$             | 155        | 3.2      | 5406.743901(4)             |                          |
| 3438  | $E$               | 149        | 2.4      | 5407.419986(6)             |                          |
| 3439  | $E$               | 147        | 2.4      | 5407.419987(2)             |                          |
| 3440  | $A_1$             | 134        | 2.3      | 5407.777947(2)             |                          |
| 3441  | $E$               | 91         | 1.1      | 5408.757499(3)             |                          |
| 3442  | $E$               | 108        | 1.1      | 5408.757499(2)             |                          |
| 3443  | $E$               | 100        | 2.4      | 5409.58261(4)              |                          |
| 3444  | $E$               | 101        | 2.4      | 5409.58262(4)              |                          |
| 3445  | $E$               | 123        | 2.3      | 5409.81388(1)              |                          |
| 3446  | $E$               | 154        | 2.3      | 5409.81389(1)              |                          |
| 3447  | $A_1$             | 96         | 1.1      | 5410.152517(2)             |                          |
| 3448  | $E$               | 96         | 0.18     | 5412.233863(1)             |                          |
| 3449  | $E$               | 98         | 0.18     | 5412.233864(1)             |                          |
| 3450  | $E$               | 101        | 2.6      | 5415.86937(2)              |                          |
| 3451  | $E$               | 103        | 2.6      | 5415.86937(2)              |                          |
| 3452  | $A_1$             | 100        | 2.6      | 5415.87407(2)              |                          |
| 3453  | $A_2$             | 88         | 2.6      | 5415.87411(7)              |                          |
| 3454  | $A_1$             | 91         | 2.4      | 5416.4941(1)               |                          |
| 3455  | $A_2$             | 93         | 2.4      | 5416.49410(8)              |                          |
| 3456  | $E$               | 108        | 2.3      | 5416.67475(2)              |                          |
| 3457  | $E$               | 108        | 2.3      | 5416.67475(2)              |                          |
| 3458  | $A_2^*$           | 130        | 2.5      | 5417.21905(3)              |                          |
| 3459  | $A_1^*$           | 129        | 2.5      | 5417.21905(3)              |                          |
| 3460  | $E$               | 128        | 2.5      | 5417.22392(3)              |                          |
| 3461  | $E$               | 158        | 2.5      | 5417.22393(4)              |                          |
| 3462  | $E$               | 107        | 0.69     | 5417.359076(7)             |                          |
| 3463  | $E$               | 98         | 0.71     | 5417.35908(1)              |                          |
| 3464  | $A_1$             | 89         | 2.4      | 5419.20930(2)              |                          |
| 3465  | $A_2$             | 89         | 2.4      | 5419.20931(2)              |                          |
| 3466  | $E$               | 102        | 2.3      | 5419.41407(1)              |                          |

Continued on next page.

TABLE S4 – states on Sarka/Poirier CSC PES; continued from previous page

| State | $\Gamma_{C_{3v}}$ | $D_{\max}$ | $S_{vN}$ | $\tilde{E}/\text{cm}^{-1}$ | $\Delta\text{Ref. [30]}$ |
|-------|-------------------|------------|----------|----------------------------|--------------------------|
| 3467  | $E$               | 136        | 2.3      | 5419.41408(1)              |                          |
| 3468  | $E$               | 106        | 2.4      | 5420.60931(2)              |                          |
| 3469  | $E$               | 162        | 2.4      | 5420.60931(2)              |                          |
| 3470  | $A_1$             | 96         | 2.4      | 5420.78701(5)              |                          |
| 3471  | $A_2$             | 93         | 2.4      | 5420.78739(5)              |                          |
| 3472  | $A_2$             | 92         | 0.28     | 5421.417660(4)             |                          |
| 3473  | $A_1$             | 97         | 0.28     | 5421.417662(8)             |                          |
| 3474  | $E$               | 136        | 0.82     | 5421.551440(3)             |                          |
| 3475  | $E$               | 117        | 0.82     | 5421.551440(4)             |                          |
| 3476  | $E$               | 57         | 2.0      | 5422.167816(7)             |                          |
| 3477  | $E$               | 93         | 2.0      | 5422.167819(6)             |                          |
| 3478  | $E$               | 98         | 0.71     | 5422.18499(2)              |                          |
| 3479  | $E$               | 96         | 0.69     | 5422.18499(2)              |                          |
| 3480  | $E$               | 162        | 4.4      | 5422.52231(1)              |                          |
| 3481  | $E$               | 184        | 4.4      | 5422.52232(2)              |                          |
| 3482  | $E$               | 202        | 4.7      | 5422.633552(6)             |                          |
| 3483  | $E$               | 195        | 4.7      | 5422.633556(8)             |                          |
| 3484  | $A_2$             | 129        | 3.3      | 5422.89335(5)              |                          |
| 3485  | $A_1$             | 128        | 3.3      | 5422.89336(5)              |                          |
| 3486  | $E$               | 195        | 3.8      | 5422.977529(4)             |                          |
| 3487  | $E$               | 210        | 3.7      | 5422.97754(1)              |                          |
| 3488  | $E$               | 208        | 4.7      | 5423.143518(9)             |                          |
| 3489  | $E$               | 201        | 4.7      | 5423.143520(6)             |                          |
| 3490  | $A_1$             | 204        | 0.18     | 5423.16308(1)              |                          |
| 3491  | $E$               | 100        | 3.1      | 5423.183120(4)             |                          |
| 3492  | $E$               | 172        | 3.1      | 5423.183124(6)             |                          |
| 3493  | $A_2$             | 109        | 0.17     | 5423.328972(1)             |                          |
| 3494  | $A_2$             | 183        | 2.7      | 5425.312445(5)             |                          |
| 3495  | $E$               | 178        | 2.6      | 5425.749210(3)             |                          |
| 3496  | $E$               | 191        | 2.6      | 5425.749217(8)             |                          |
| 3497  | $A_1$             | 197        | 2.6      | 5426.083944(7)             |                          |
| 3498  | $E$               | 126        | 2.3      | 5426.571190(6)             |                          |
| 3499  | $E$               | 127        | 2.3      | 5426.571191(7)             |                          |
| 3500  | $E$               | 130        | 2.1      | 5427.123307(5)             |                          |
| 3501  | $E$               | 125        | 2.1      | 5427.123308(7)             |                          |
| 3502  | $E$               | 115        | 2.7      | 5427.47512(2)              |                          |
| 3503  | $E$               | 99         | 2.7      | 5427.47512(4)              |                          |
| 3504  | $A_1$             | 88         | 2.6      | 5427.63523(3)              |                          |
| 3505  | $A_2$             | 92         | 2.6      | 5427.63523(4)              |                          |
| 3506  | $E$               | 180        | 3.5      | 5428.354762(6)             |                          |
| 3507  | $E$               | 184        | 3.5      | 5428.354765(7)             |                          |
| 3508  | $E$               | 190        | 3.4      | 5428.501103(9)             |                          |
| 3509  | $E$               | 197        | 3.4      | 5428.50111(1)              |                          |
| 3510  | $A_1$             | 177        | 3.5      | 5428.666194(9)             |                          |
| 3511  | $A_2$             | 145        | 3.4      | 5428.66741(2)              |                          |
| 3512  | $E$               | 132        | 2.2      | 5428.711919(3)             |                          |
| 3513  | $E$               | 114        | 2.2      | 5428.711921(5)             |                          |
| 3514  | $A_1$             | 130        | 3.2      | 5428.81959(5)              |                          |
| 3515  | $A_2$             | 179        | 3.2      | 5428.81961(5)              |                          |
| 3516  | $A_2$             | 129        | 2.2      | 5429.061754(3)             |                          |
| 3517  | $A_1$             | 121        | 2.2      | 5429.078589(4)             |                          |
| 3518  | $A_1$             | 65         | 0.31     | 5429.3456318(3)            |                          |
| 3519  | $A_1$             | 138        | 2.3      | 5431.14941(1)              |                          |
| 3520  | $A_2$             | 130        | 2.3      | 5431.149419(8)             |                          |
| 3521  | $E$               | 184        | 2.7      | 5431.152500(7)             |                          |
| 3522  | $E$               | 161        | 2.7      | 5431.15250(1)              |                          |
| 3523  | $A_1$             | 153        | 3.4      | 5431.17813(1)              |                          |
| 3524  | $A_2$             | 178        | 3.5      | 5431.348531(9)             |                          |
| 3525  | $E$               | 159        | 1.0      | 5431.383284(3)             |                          |

Continued on next page.

TABLE S4 – states on Sarka/Poirier CSC PES; continued from previous page

| State | $\Gamma_{C_{3v}}$ | $D_{\max}$ | $S_{vN}$ | $\tilde{E}/\text{cm}^{-1}$ | $\Delta\text{Ref. [30]}$ |
|-------|-------------------|------------|----------|----------------------------|--------------------------|
| 3526  | $E$               | 152        | 1.0      | 5431.383285(4)             |                          |
| 3527  | $E$               | 183        | 3.2      | 5431.624201(4)             |                          |
| 3528  | $E$               | 185        | 3.2      | 5431.624203(4)             |                          |
| 3529  | $E$               | 177        | 2.6      | 5431.712372(5)             |                          |
| 3530  | $E$               | 167        | 2.6      | 5431.71237(1)              |                          |
| 3531  | $E$               | 148        | 3.3      | 5431.985414(2)             |                          |
| 3532  | $E$               | 152        | 3.3      | 5431.985420(7)             |                          |
| 3533  | $E$               | 144        | 3.2      | 5432.069068(4)             |                          |
| 3534  | $E$               | 167        | 3.2      | 5432.069073(7)             |                          |
| 3535  | $E$               | 116        | 0.42     | 5432.29934(2)              |                          |
| 3536  | $E$               | 152        | 0.42     | 5432.29935(2)              |                          |
| 3537  | $A_2$             | 111        | 2.2      | 5432.46029(1)              |                          |
| 3538  | $A_1$             | 108        | 2.2      | 5432.46030(1)              |                          |
| 3539  | $E$               | 60         | 2.0      | 5432.633000(9)             |                          |
| 3540  | $E$               | 61         | 2.0      | 5432.633000(9)             |                          |
| 3541  | $E$               | 158        | 2.9      | 5432.986006(4)             |                          |
| 3542  | $E$               | 106        | 2.9      | 5432.98601(3)              |                          |
| 3543  | $E$               | 152        | 2.8      | 5433.112352(4)             |                          |
| 3544  | $E$               | 101        | 2.8      | 5433.11235(2)              |                          |
| 3545  | $E$               | 176        | 2.4      | 5434.004013(4)             |                          |
| 3546  | $E$               | 136        | 2.4      | 5434.004017(6)             |                          |
| 3547  | $A_1$             | 116        | 3.3      | 5434.94398(3)              |                          |
| 3548  | $A_2$             | 109        | 3.3      | 5434.94604(7)              |                          |
| 3549  | $E$               | 114        | 3.1      | 5434.96948(1)              |                          |
| 3550  | $E$               | 107        | 3.1      | 5434.96948(2)              |                          |
| 3551  | $E$               | 127        | 2.4      | 5435.350875(2)             |                          |
| 3552  | $E$               | 125        | 2.4      | 5435.350877(3)             |                          |
| 3553  | $A_1$             | 118        | 3.0      | 5435.50284(1)              |                          |
| 3554  | $E$               | 149        | 2.9      | 5435.850524(3)             |                          |
| 3555  | $E$               | 98         | 2.9      | 5435.85053(2)              |                          |
| 3556  | $A_2$             | 93         | 2.9      | 5436.08407(3)              |                          |
| 3557  | $E$               | 155        | 4.0      | 5436.440883(8)             |                          |
| 3558  | $E$               | 131        | 4.0      | 5436.44089(2)              |                          |
| 3559  | $A_1$             | 160        | 4.0      | 5436.472548(7)             |                          |
| 3560  | $A_2$             | 119        | 4.0      | 5436.47334(4)              |                          |
| 3561  | $E$               | 157        | 2.6      | 5437.464591(8)             |                          |
| 3562  | $E$               | 133        | 2.6      | 5437.464597(8)             |                          |
| 3563  | $A_1^*$           | 110        | 2.2      | 5437.945859(9)             |                          |
| 3564  | $A_2^*$           | 109        | 2.2      | 5437.94586(1)              |                          |
| 3565  | $E$               | 122        | 3.8      | 5439.55260(3)              |                          |
| 3566  | $E$               | 129        | 3.8      | 5439.55260(4)              |                          |
| 3567  | $A_1$             | 134        | 3.8      | 5439.55522(2)              |                          |
| 3568  | $A_2$             | 127        | 3.8      | 5439.55708(3)              |                          |
| 3569  | $E$               | 113        | 0.68     | 5440.48903(3)              |                          |
| 3570  | $E$               | 143        | 0.69     | 5440.48904(3)              |                          |
| 3571  | $E$               | 148        | 3.2      | 5442.821331(3)             |                          |
| 3572  | $E$               | 150        | 3.2      | 5442.821332(3)             |                          |
| 3573  | $E$               | 145        | 2.3      | 5443.914889(3)             |                          |
| 3574  | $E$               | 131        | 2.3      | 5443.914889(8)             |                          |
| 3575  | $E$               | 130        | 2.5      | 5444.158932(7)             |                          |
| 3576  | $E$               | 149        | 2.5      | 5444.158934(7)             |                          |
| 3577  | $E$               | 147        | 3.1      | 5444.339746(3)             |                          |
| 3578  | $E$               | 151        | 3.1      | 5444.339746(3)             |                          |
| 3579  | $A_1$             | 137        | 3.1      | 5444.81742(1)              |                          |
| 3580  | $A_2$             | 132        | 3.1      | 5444.81826(1)              |                          |
| 3581  | $E$               | 164        | 3.1      | 5444.853730(3)             |                          |
| 3582  | $E$               | 160        | 3.1      | 5444.853730(3)             |                          |
| 3583  | $A_1$             | 114        | 3.5      | 5445.33116(6)              |                          |
| 3584  | $A_2$             | 121        | 3.5      | 5445.33125(7)              |                          |

Continued on next page.

TABLE S4 – states on Sarka/Poirier CSC PES; continued from previous page

| State | $\Gamma_{C_{3v}}$ | $D_{\max}$ | $S_{vN}$ | $\tilde{E}/\text{cm}^{-1}$ | $\Delta\text{Ref. [30]}$ |
|-------|-------------------|------------|----------|----------------------------|--------------------------|
| 3585  | $E$               | 132        | 2.3      | 5446.05329(1)              |                          |
| 3586  | $E$               | 136        | 2.3      | 5446.05329(1)              |                          |
| 3587  | $A_1$             | 183        | 3.2      | 5446.271730(6)             |                          |
| 3588  | $A_2$             | 110        | 3.2      | 5446.27187(6)              |                          |
| 3589  | $E$               | 119        | 0.93     | 5448.477399(7)             |                          |
| 3590  | $E$               | 115        | 0.93     | 5448.47740(1)              |                          |
| 3591  | $A_1$             | 169        | 2.4      | 5449.250670(3)             |                          |
| 3592  | $A_2$             | 165        | 2.3      | 5449.276988(3)             |                          |
| 3593  | $E$               | 170        | 2.6      | 5449.373786(3)             |                          |
| 3594  | $E$               | 159        | 2.6      | 5449.373788(4)             |                          |
| 3595  | $E$               | 118        | 0.8      | 5450.877846(2)             |                          |
| 3596  | $E$               | 115        | 0.8      | 5450.877846(2)             |                          |
| 3597  | $E$               | 93         | 2.8      | 5451.25818(3)              |                          |
| 3598  | $E$               | 99         | 2.8      | 5451.25818(4)              |                          |
| 3599  | $E$               | 125        | 2.7      | 5451.33051(2)              |                          |
| 3600  | $E$               | 124        | 2.7      | 5451.33051(2)              |                          |
| 3601  | $A_1$             | 94         | 2.7      | 5451.336866(3)             |                          |
| 3602  | $A_2$             | 92         | 2.7      | 5451.336935(2)             |                          |
| 3603  | $E$               | 126        | 2.4      | 5451.443131(4)             |                          |
| 3604  | $E$               | 133        | 2.4      | 5451.443134(6)             |                          |
| 3605  | $E$               | 88         | 0.78     | 5452.787793(5)             |                          |
| 3606  | $E$               | 86         | 0.79     | 5452.787795(3)             |                          |
| 3607  | $E$               | 102        | 2.4      | 5454.07224(1)              |                          |
| 3608  | $E$               | 109        | 2.4      | 5454.07225(1)              |                          |
| 3609  | $A_1$             | 105        | 2.4      | 5454.10638(1)              |                          |
| 3610  | $A_2$             | 107        | 2.4      | 5454.12335(1)              |                          |
| 3611  | $A_1$             | 136        | 0.64     | 5454.498799(2)             |                          |
| 3612  | $A_2$             | 137        | 0.61     | 5454.667516(2)             |                          |
| 3613  | $E$               | 63         | 0.14     | 5457.858226(1)             |                          |
| 3614  | $E$               | 81         | 0.14     | 5457.858226(1)             |                          |
| 3615  | $E$               | 130        | 0.84     | 5458.299002(2)             |                          |
| 3616  | $E$               | 131        | 0.84     | 5458.299002(2)             |                          |
| 3617  | $E$               | 107        | 2.1      | 5462.19956(1)              |                          |
| 3618  | $E$               | 137        | 2.1      | 5462.19957(1)              |                          |
| 3619  | $A_1$             | 92         | 2.2      | 5462.22940(2)              |                          |
| 3620  | $A_2$             | 109        | 2.2      | 5462.22941(3)              |                          |
| 3621  | $A_1$             | 84         | 0.38     | 5462.99407(1)              |                          |
| 3622  | $A_2$             | 84         | 0.38     | 5462.99408(1)              |                          |
| 3623  | $E$               | 52         | 0.26     | 5463.379956(2)             |                          |
| 3624  | $E$               | 55         | 0.26     | 5463.379957(2)             |                          |
| 3625  | $E$               | 129        | 2.7      | 5463.733447(7)             |                          |
| 3626  | $E$               | 108        | 2.7      | 5463.73345(2)              |                          |
| 3627  | $A_1$             | 109        | 2.7      | 5463.77309(2)              |                          |
| 3628  | $A_2$             | 111        | 2.6      | 5463.77697(1)              |                          |
| 3629  | $A_2$             | 91         | 0.57     | 5464.31497(2)              |                          |
| 3630  | $A_1$             | 94         | 0.57     | 5464.31498(3)              |                          |
| 3631  | $E$               | 107        | 0.44     | 5465.87794(1)              |                          |
| 3632  | $E$               | 111        | 0.45     | 5465.87794(1)              |                          |
| 3633  | $A_2$             | 99         | 2.3      | 5465.97459(3)              |                          |
| 3634  | $A_1$             | 95         | 2.3      | 5465.97798(4)              |                          |
| 3635  | $E$               | 125        | 2.1      | 5466.04502(1)              |                          |
| 3636  | $E$               | 107        | 2.1      | 5466.04503(2)              |                          |
| 3637  | $E$               | 129        | 0.65     | 5467.206082(2)             |                          |
| 3638  | $E$               | 122        | 0.65     | 5467.206086(4)             |                          |
| 3639  | $A_1$             | 82         | 3.3      | 5467.577127(1)             |                          |
| 3640  | $E$               | 136        | 2.4      | 5468.359129(7)             |                          |
| 3641  | $E$               | 122        | 2.4      | 5468.359133(4)             |                          |
| 3642  | $E$               | 115        | 2.2      | 5468.502998(2)             |                          |
| 3643  | $E$               | 114        | 2.2      | 5468.503000(3)             |                          |

Continued on next page.

TABLE S4 – states on Sarka/Poirier CSC PES; continued from previous page

| State | $\Gamma_{C_{3v}}$ | $D_{\max}$ | $S_{vN}$ | $\tilde{E}/\text{cm}^{-1}$ | $\Delta\text{Ref. [30]}$ |
|-------|-------------------|------------|----------|----------------------------|--------------------------|
| 3644  | $E$               | 110        | 2.2      | 5470.56658(2)              |                          |
| 3645  | $E$               | 91         | 2.2      | 5470.56659(7)              |                          |
| 3646  | $A_1^*$           | 99         | 2.2      | 5470.56984(3)              |                          |
| 3647  | $A_2^*$           | 97         | 2.2      | 5470.56984(4)              |                          |
| 3648  | $E$               | 119        | 2.3      | 5471.308067(3)             |                          |
| 3649  | $E$               | 114        | 2.3      | 5471.30807(1)              |                          |
| 3650  | $A_1$             | 99         | 2.9      | 5471.34850(4)              |                          |
| 3651  | $A_2$             | 103        | 2.9      | 5471.35567(3)              |                          |
| 3652  | $E$               | 145        | 2.1      | 5471.355850(4)             |                          |
| 3653  | $E$               | 134        | 2.1      | 5471.355851(8)             |                          |
| 3654  | $E$               | 167        | 2.2      | 5471.399830(4)             |                          |
| 3655  | $E$               | 134        | 2.2      | 5471.399838(9)             |                          |
| 3656  | $E$               | 167        | 2.8      | 5471.572959(2)             |                          |
| 3657  | $E$               | 118        | 2.8      | 5471.57296(2)              |                          |
| 3658  | $A_1$             | 94         | 3.3      | 5471.66970(8)              |                          |
| 3659  | $A_2$             | 100        | 3.3      | 5471.66990(6)              |                          |
| 3660  | $E$               | 108        | 0.85     | 5473.10334(1)              |                          |
| 3661  | $E$               | 100        | 0.85     | 5473.10334(1)              |                          |
| 3662  | $A_2$             | 109        | 2.2      | 5474.281989(6)             |                          |
| 3663  | $A_1$             | 124        | 2.2      | 5474.28299(1)              |                          |
| 3664  | $E$               | 105        | 2.2      | 5474.297400(5)             |                          |
| 3665  | $E$               | 105        | 2.2      | 5474.29741(1)              |                          |
| 3666  | $E$               | 137        | 2.2      | 5476.102943(9)             |                          |
| 3667  | $E$               | 154        | 2.2      | 5476.102944(9)             |                          |
| 3668  | $E$               | 102        | 2.2      | 5476.16112(1)              |                          |
| 3669  | $E$               | 116        | 2.2      | 5476.16113(2)              |                          |
| 3670  | $A_1$             | 85         | 3.4      | 5477.746798(1)             |                          |
| 3671  | $E$               | 87         | 0.14     | 5478.172202(3)             |                          |
| 3672  | $E$               | 67         | 0.14     | 5478.172202(8)             |                          |
| 3673  | $A_2$             | 129        | 2.3      | 5478.537159(5)             |                          |
| 3674  | $E$               | 107        | 2.2      | 5478.98496(1)              |                          |
| 3675  | $E$               | 152        | 2.2      | 5478.98496(1)              |                          |
| 3676  | $A_1$             | 109        | 2.2      | 5479.33751(1)              |                          |
| 3677  | $A_1$             | 127        | 3.3      | 5482.695914(2)             |                          |
| 3678  | $E$               | 94         | 3.2      | 5482.774490(7)             |                          |
| 3679  | $E$               | 96         | 3.2      | 5482.774491(5)             |                          |
| 3680  | $A_2$             | 82         | 3.2      | 5482.816491(2)             |                          |
| 3681  | $E$               | 106        | 2.2      | 5485.06236(1)              |                          |
| 3682  | $E$               | 104        | 2.2      | 5485.06236(1)              |                          |
| 3683  | $E$               | 107        | 2.2      | 5485.086571(7)             |                          |
| 3684  | $E$               | 146        | 2.2      | 5485.086573(8)             |                          |
| 3685  | $A_2$             | 179        | 2.7      | 5485.111633(3)             |                          |
| 3686  | $A_1$             | 178        | 2.7      | 5485.111633(3)             |                          |
| 3687  | $E$               | 149        | 2.7      | 5485.22947(1)              |                          |
| 3688  | $E$               | 139        | 2.7      | 5485.22947(1)              |                          |
| 3689  | $E$               | 153        | 2.2      | 5488.032394(3)             |                          |
| 3690  | $E$               | 158        | 2.2      | 5488.032394(2)             |                          |
| 3691  | $A_2$             | 119        | 3.2      | 5488.815905(7)             |                          |
| 3692  | $A_1$             | 119        | 3.2      | 5488.815909(8)             |                          |
| 3693  | $E$               | 125        | 3.1      | 5489.020773(5)             |                          |
| 3694  | $E$               | 138        | 3.1      | 5489.020779(8)             |                          |
| 3695  | $E$               | 127        | 2.2      | 5489.356115(6)             |                          |
| 3696  | $E$               | 127        | 2.2      | 5489.356115(7)             |                          |
| 3697  | $E$               | 181        | 2.9      | 5489.381501(5)             |                          |
| 3698  | $E$               | 177        | 2.9      | 5489.381503(6)             |                          |
| 3699  | $A_2$             | 135        | 2.8      | 5489.48993(4)              |                          |
| 3700  | $A_1$             | 134        | 2.8      | 5489.49024(4)              |                          |
| 3701  | $E$               | 82         | 0.35     | 5490.320733(3)             |                          |
| 3702  | $E$               | 86         | 0.35     | 5490.320733(5)             |                          |

Continued on next page.



TABLE S4 – states on Sarka/Poirier CSC PES; continued from previous page

| State | $\Gamma_{C_{3v}}$ | $D_{\max}$ | $S_{vN}$ | $\tilde{E}/\text{cm}^{-1}$ | $\Delta\text{Ref. [30]}$ |
|-------|-------------------|------------|----------|----------------------------|--------------------------|
| 3703  | $E$               | 170        | 1.0      | 5490.929270(4)             |                          |
| 3704  | $E$               | 168        | 1.0      | 5490.929271(5)             |                          |
| 3705  | $A_1^*$           | 88         | 0.26     | 5491.505819(3)             |                          |
| 3706  | $A_2^*$           | 89         | 0.26     | 5491.505819(3)             |                          |
| 3707  | $A_2^*$           | 87         | 2.5      | 5492.02957(3)              |                          |
| 3708  | $A_1^*$           | 82         | 2.5      | 5492.02958(3)              |                          |
| 3709  | $E$               | 96         | 2.5      | 5492.04079(2)              |                          |
| 3710  | $E$               | 92         | 2.5      | 5492.04079(3)              |                          |
| 3711  | $E$               | 182        | 3.3      | 5492.230465(3)             |                          |
| 3712  | $E$               | 153        | 3.3      | 5492.230469(9)             |                          |
| 3713  | $E$               | 89         | 0.27     | 5492.338900(5)             |                          |
| 3714  | $E$               | 94         | 0.27     | 5492.338901(5)             |                          |
| 3715  | $A_2$             | 186        | 3.3      | 5492.403830(3)             |                          |
| 3716  | $A_1$             | 191        | 3.3      | 5492.403835(3)             |                          |
| 3717  | $E$               | 174        | 3.2      | 5492.633931(3)             |                          |
| 3718  | $E$               | 186        | 3.2      | 5492.633938(8)             |                          |
| 3719  | $E$               | 167        | 3.0      | 5492.685006(5)             |                          |
| 3720  | $E$               | 179        | 3.0      | 5492.685009(5)             |                          |
| 3721  | $A_1$             | 104        | 0.82     | 5494.12792(8)              |                          |
| 3722  | $A_2$             | 106        | 0.82     | 5494.12794(6)              |                          |
| 3723  | $E$               | 111        | 2.6      | 5496.14515(1)              |                          |
| 3724  | $E$               | 124        | 2.6      | 5496.14515(1)              |                          |
| 3725  | $A_1$             | 96         | 2.6      | 5496.24154(1)              |                          |
| 3726  | $A_2$             | 87         | 2.6      | 5496.24192(3)              |                          |
| 3727  | $A_2$             | 133        | 3.4      | 5496.57541(4)              |                          |
| 3728  | $A_1$             | 133        | 3.4      | 5496.57550(3)              |                          |
| 3729  | $E$               | 167        | 3.3      | 5496.66537(1)              |                          |
| 3730  | $E$               | 192        | 3.3      | 5496.66537(1)              |                          |
| 3731  | $A_2$             | 95         | 0.66     | 5496.82785(1)              |                          |
| 3732  | $A_1$             | 121        | 0.66     | 5496.82785(1)              |                          |
| 3733  | $E$               | 183        | 3.1      | 5496.944352(3)             |                          |
| 3734  | $E$               | 157        | 3.1      | 5496.944356(9)             |                          |
| 3735  | $E$               | 145        | 3.0      | 5496.98471(1)              |                          |
| 3736  | $E$               | 164        | 3.0      | 5496.98472(1)              |                          |
| 3737  | $E$               | 186        | 0.94     | 5497.019708(4)             |                          |
| 3738  | $E$               | 139        | 0.94     | 5497.019716(9)             |                          |
| 3739  | $A_1$             | 107        | 3.6      | 5497.13731(2)              |                          |
| 3740  | $E$               | 128        | 3.5      | 5497.255016(5)             |                          |
| 3741  | $E$               | 103        | 3.5      | 5497.25502(1)              |                          |
| 3742  | $A_2$             | 96         | 3.4      | 5497.325186(1)             |                          |
| 3743  | $A_2$             | 124        | 2.3      | 5497.665226(5)             |                          |
| 3744  | $A_1$             | 122        | 2.3      | 5497.66523(1)              |                          |
| 3745  | $E$               | 91         | 1.0      | 5497.69954(1)              |                          |
| 3746  | $E$               | 105        | 1.0      | 5497.69954(1)              |                          |
| 3747  | $E$               | 158        | 2.3      | 5498.081381(3)             |                          |
| 3748  | $E$               | 132        | 2.3      | 5498.08138(2)              |                          |
| 3749  | $A_2$             | 117        | 2.2      | 5498.40526(3)              |                          |
| 3750  | $A_1$             | 137        | 2.2      | 5498.423072(9)             |                          |
| 3751  | $E$               | 148        | 3.3      | 5498.445750(2)             |                          |
| 3752  | $E$               | 143        | 3.3      | 5498.445757(7)             |                          |
| 3753  | $E$               | 112        | 0.53     | 5498.549944(4)             |                          |
| 3754  | $E$               | 111        | 0.53     | 5498.549945(3)             |                          |
| 3755  | $E$               | 139        | 3.2      | 5498.636225(2)             |                          |
| 3756  | $E$               | 145        | 3.2      | 5498.636227(4)             |                          |
| 3757  | $A_1$             | 107        | 2.3      | 5498.97634(1)              |                          |
| 3758  | $A_2$             | 109        | 2.3      | 5498.976342(9)             |                          |
| 3759  | $A_1$             | 103        | 0.48     | 5499.266356(4)             |                          |
| 3760  | $A_2$             | 108        | 0.48     | 5499.266360(3)             |                          |
| 3761  | $E$               | 151        | 2.8      | 5499.52687(1)              |                          |

Continued on next page.

TABLE S4 – states on Sarka/Poirier CSC PES; continued from previous page

| State | $\Gamma_{C_{3v}}$ | $D_{\max}$ | $S_{vN}$ | $\tilde{E}/\text{cm}^{-1}$ | $\Delta\text{Ref. [30]}$ |
|-------|-------------------|------------|----------|----------------------------|--------------------------|
| 3762  | $E$               | 149        | 2.8      | 5499.52687(1)              |                          |
| 3763  | $E$               | 141        | 2.8      | 5499.677901(3)             |                          |
| 3764  | $E$               | 144        | 2.8      | 5499.677903(4)             |                          |
| 3765  | $E$               | 145        | 0.65     | 5499.739406(1)             |                          |
| 3766  | $E$               | 128        | 0.65     | 5499.739407(3)             |                          |
| 3767  | $A_1$             | 110        | 0.64     | 5500.001779(2)             |                          |
| 3768  | $E$               | 82         | 0.79     | 5502.080481(2)             |                          |
| 3769  | $E$               | 86         | 0.79     | 5502.080481(2)             |                          |
| 3770  | $E$               | 100        | 0.33     | 5502.179121(4)             |                          |
| 3771  | $E$               | 106        | 0.33     | 5502.179121(3)             |                          |
| 3772  | $E$               | 86         | 0.89     | 5502.245840(8)             |                          |
| 3773  | $E$               | 104        | 0.89     | 5502.245840(4)             |                          |
| 3774  | $E$               | 115        | 2.7      | 5502.49524(4)              |                          |
| 3775  | $E$               | 115        | 2.7      | 5502.49524(4)              |                          |
| 3776  | $A_1$             | 124        | 2.8      | 5502.54371(2)              |                          |
| 3777  | $A_2$             | 142        | 2.7      | 5502.552744(5)             |                          |
| 3778  | $E$               | 90         | 0.63     | 5502.896639(2)             |                          |
| 3779  | $E$               | 106        | 0.63     | 5502.896639(2)             |                          |
| 3780  | $E$               | 117        | 0.59     | 5503.127157(7)             |                          |
| 3781  | $E$               | 115        | 0.59     | 5503.127158(8)             |                          |
| 3782  | $E$               | 141        | 2.4      | 5504.54451(1)              |                          |
| 3783  | $E$               | 134        | 2.4      | 5504.544522(8)             |                          |
| 3784  | $A_1$             | 118        | 0.66     | 5504.55686(1)              |                          |
| 3785  | $E$               | 101        | 2.1      | 5504.939560(4)             |                          |
| 3786  | $E$               | 124        | 2.1      | 5504.939561(4)             |                          |
| 3787  | $E$               | 150        | 3.4      | 5505.30315(1)              |                          |
| 3788  | $E$               | 160        | 3.4      | 5505.30316(1)              |                          |
| 3789  | $E$               | 94         | 3.1      | 5505.435978(6)             |                          |
| 3790  | $E$               | 95         | 3.1      | 5505.435978(9)             |                          |
| 3791  | $A_1$             | 83         | 3.1      | 5505.45076(3)              |                          |
| 3792  | $A_2$             | 85         | 3.1      | 5505.453946(9)             |                          |
| 3793  | $A_2$             | 188        | 3.2      | 5505.507512(3)             |                          |
| 3794  | $A_1$             | 188        | 3.2      | 5505.507512(3)             |                          |
| 3795  | $E$               | 147        | 2.1      | 5505.533674(4)             |                          |
| 3796  | $E$               | 97         | 2.1      | 5505.533681(8)             |                          |
| 3797  | $A_2$             | 104        | 2.1      | 5505.553203(4)             |                          |
| 3798  | $A_1$             | 108        | 2.2      | 5505.567990(6)             |                          |
| 3799  | $A_2^*$           | 120        | 2.5      | 5505.67370(2)              |                          |
| 3800  | $A_1^*$           | 124        | 2.5      | 5505.67370(2)              |                          |
| 3801  | $E$               | 168        | 2.7      | 5505.83336(1)              |                          |
| 3802  | $E$               | 167        | 2.7      | 5505.833361(3)             |                          |
| 3803  | $E$               | 129        | 2.3      | 5505.850165(3)             |                          |
| 3804  | $E$               | 131        | 2.3      | 5505.850166(2)             |                          |
| 3805  | $E$               | 132        | 2.1      | 5505.981092(2)             |                          |
| 3806  | $E$               | 106        | 2.1      | 5505.981092(9)             |                          |
| 3807  | $A_2$             | 115        | 2.8      | 5506.380498(2)             |                          |
| 3808  | $E$               | 112        | 0.2      | 5507.010065(4)             |                          |
| 3809  | $E$               | 101        | 0.2      | 5507.010069(4)             |                          |
| 3810  | $E$               | 109        | 2.8      | 5507.766013(2)             |                          |
| 3811  | $E$               | 118        | 2.8      | 5507.766013(2)             |                          |
| 3812  | $A_2$             | 94         | 2.4      | 5508.49425(5)              |                          |
| 3813  | $A_1$             | 91         | 2.4      | 5508.50143(8)              |                          |
| 3814  | $E$               | 107        | 2.2      | 5508.575109(8)             |                          |
| 3815  | $E$               | 131        | 2.2      | 5508.57512(1)              |                          |
| 3816  | $A_1$             | 60         | 0.66     | 5508.59831(1)              |                          |
| 3817  | $A_2$             | 59         | 0.66     | 5508.59832(1)              |                          |
| 3818  | $E$               | 143        | 2.7      | 5508.647416(7)             |                          |
| 3819  | $E$               | 146        | 2.7      | 5508.647420(8)             |                          |
| 3820  | $A_1$             | 119        | 2.8      | 5508.865773(2)             |                          |

Continued on next page.

TABLE S4 – states on Sarka/Poirier CSC PES; continued from previous page

| State | $\Gamma_{C_{3v}}$ | $D_{\max}$ | $S_{vN}$ | $\tilde{E}/\text{cm}^{-1}$ | $\Delta\text{Ref. [30]}$ |
|-------|-------------------|------------|----------|----------------------------|--------------------------|
| 3821  | $A_2$             | 132        | 3.9      | 5508.99454(1)              |                          |
| 3822  | $A_1$             | 182        | 3.3      | 5509.528226(3)             |                          |
| 3823  | $E$               | 143        | 3.3      | 5509.639050(3)             |                          |
| 3824  | $E$               | 148        | 3.3      | 5509.639052(4)             |                          |
| 3825  | $E$               | 88         | 2.1      | 5509.85428(1)              |                          |
| 3826  | $E$               | 90         | 2.1      | 5509.854284(3)             |                          |
| 3827  | $E$               | 170        | 2.6      | 5509.910660(3)             |                          |
| 3828  | $E$               | 160        | 2.6      | 5509.910668(9)             |                          |
| 3829  | $E$               | 127        | 2.3      | 5509.971925(3)             |                          |
| 3830  | $E$               | 126        | 2.3      | 5509.971925(2)             |                          |
| 3831  | $E$               | 107        | 0.41     | 5509.983852(4)             |                          |
| 3832  | $E$               | 141        | 0.41     | 5509.983858(7)             |                          |
| 3833  | $A_1$             | 124        | 2.6      | 5510.06320(9)              |                          |
| 3834  | $A_2$             | 121        | 2.6      | 5510.0642(1)               |                          |
| 3835  | $E$               | 97         | 0.38     | 5510.187842(6)             |                          |
| 3836  | $E$               | 97         | 0.38     | 5510.187842(7)             |                          |
| 3837  | $E$               | 95         | 2.1      | 5510.217365(7)             |                          |
| 3838  | $E$               | 83         | 2.1      | 5510.217374(9)             |                          |
| 3839  | $A_2$             | 148        | 3.5      | 5510.612617(2)             |                          |
| 3840  | $E$               | 135        | 2.6      | 5511.070173(2)             |                          |
| 3841  | $E$               | 136        | 2.6      | 5511.070174(2)             |                          |
| 3842  | $A_1$             | 125        | 2.3      | 5511.362433(1)             |                          |
| 3843  | $E$               | 74         | 0.67     | 5511.449700(5)             |                          |
| 3844  | $E$               | 92         | 0.67     | 5511.449700(3)             |                          |
| 3845  | $E$               | 144        | 0.81     | 5511.497103(6)             |                          |
| 3846  | $E$               | 168        | 0.84     | 5511.497109(9)             |                          |
| 3847  | $A_2$             | 73         | 1.2      | 5511.52758(3)              |                          |
| 3848  | $A_1$             | 89         | 1.2      | 5511.52759(1)              |                          |
| 3849  | $A_1^*$           | 133        | 2.6      | 5515.148979(2)             |                          |
| 3850  | $A_2^*$           | 132        | 2.6      | 5515.148979(3)             |                          |
| 3851  | $E$               | 117        | 2.5      | 5515.263629(3)             |                          |
| 3852  | $E$               | 128        | 2.5      | 5515.263631(6)             |                          |
| 3853  | $A_1$             | 65         | 0.41     | 5515.52872(4)              |                          |
| 3854  | $A_2$             | 66         | 0.41     | 5515.52884(3)              |                          |
| 3855  | $E$               | 164        | 2.1      | 5516.525159(5)             |                          |
| 3856  | $E$               | 155        | 2.1      | 5516.525166(7)             |                          |
| 3857  | $E$               | 154        | 1.8      | 5516.870274(3)             |                          |
| 3858  | $E$               | 150        | 1.8      | 5516.870276(4)             |                          |
| 3859  | $E$               | 100        | 1.4      | 5518.160961(3)             |                          |
| 3860  | $E$               | 92         | 1.4      | 5518.16096(1)              |                          |
| 3861  | $E$               | 72         | 0.43     | 5518.19977(1)              |                          |
| 3862  | $E$               | 99         | 0.43     | 5518.199773(5)             |                          |
| 3863  | $E$               | 115        | 2.6      | 5519.46820(2)              |                          |
| 3864  | $E$               | 132        | 2.6      | 5519.46820(1)              |                          |
| 3865  | $A_1$             | 119        | 2.6      | 5519.54674(1)              |                          |
| 3866  | $A_2$             | 160        | 2.6      | 5519.546865(2)             |                          |
| 3867  | $E$               | 116        | 1.6      | 5520.86759(7)              |                          |
| 3868  | $E$               | 163        | 1.6      | 5520.86761(7)              |                          |
| 3869  | $E$               | 95         | 0.79     | 5520.96921(2)              |                          |
| 3870  | $E$               | 125        | 0.77     | 5520.96921(2)              |                          |
| 3871  | $E$               | 144        | 1.5      | 5521.094386(5)             |                          |
| 3872  | $E$               | 146        | 1.4      | 5521.094388(5)             |                          |
| 3873  | $A_1$             | 75         | 0.073    | 5521.546154(1)             |                          |
| 3874  | $E$               | 114        | 2.1      | 5521.614037(2)             |                          |
| 3875  | $E$               | 105        | 2.1      | 5521.614037(2)             |                          |
| 3876  | $E$               | 83         | 1.5      | 5522.14242(1)              |                          |
| 3877  | $E$               | 84         | 1.5      | 5522.14243(1)              |                          |
| 3878  | $E$               | 98         | 2.0      | 5522.211500(2)             |                          |
| 3879  | $E$               | 110        | 2.0      | 5522.211501(3)             |                          |

Continued on next page.

TABLE S4 – states on Sarka/Poirier CSC PES; continued from previous page

| State | $\Gamma_{C_{3v}}$ | $D_{\max}$ | $S_{vN}$ | $\tilde{E}/\text{cm}^{-1}$ | $\Delta\text{Ref. [30]}$ |
|-------|-------------------|------------|----------|----------------------------|--------------------------|
| 3880  | $A_2$             | 99         | 2.5      | 5522.231795(5)             |                          |
| 3881  | $A_1$             | 162        | 0.42     | 5522.324768(3)             |                          |
| 3882  | $E$               | 93         | 2.5      | 5522.331541(2)             |                          |
| 3883  | $E$               | 94         | 2.5      | 5522.331544(4)             |                          |
| 3884  | $A_1$             | 89         | 2.5      | 5522.441015(2)             |                          |
| 3885  | $A_2$             | 125        | 0.41     | 5522.49320(1)              |                          |
| 3886  | $E$               | 87         | 0.73     | 5523.202078(4)             |                          |
| 3887  | $E$               | 78         | 0.73     | 5523.202078(8)             |                          |
| 3888  | $A_1$             | 84         | 1.5      | 5523.469816(8)             |                          |
| 3889  | $A_1$             | 81         | 2.3      | 5524.36484(2)              |                          |
| 3890  | $A_2$             | 86         | 2.3      | 5524.36484(3)              |                          |
| 3891  | $E$               | 100        | 2.2      | 5524.67961(1)              |                          |
| 3892  | $E$               | 89         | 2.2      | 5524.679616(8)             |                          |
| 3893  | $E$               | 101        | 2.3      | 5525.326041(8)             |                          |
| 3894  | $E$               | 97         | 2.3      | 5525.326041(8)             |                          |
| 3895  | $E$               | 93         | 2.2      | 5525.497705(1)             |                          |
| 3896  | $E$               | 132        | 2.2      | 5525.497710(5)             |                          |
| 3897  | $E$               | 87         | 1.2      | 5526.539408(1)             |                          |
| 3898  | $E$               | 92         | 1.2      | 5526.539409(1)             |                          |
| 3899  | $A_1$             | 63         | 0.81     | 5528.87866(3)              |                          |
| 3900  | $A_2$             | 61         | 0.81     | 5528.87868(5)              |                          |
| 3901  | $E$               | 82         | 1.4      | 5530.823648(1)             |                          |
| 3902  | $E$               | 89         | 1.4      | 5530.823648(2)             |                          |
| 3903  | $E$               | 71         | 0.54     | 5531.084067(3)             |                          |
| 3904  | $E$               | 91         | 0.54     | 5531.084073(7)             |                          |
| 3905  | $E$               | 102        | 0.85     | 5531.717361(2)             |                          |
| 3906  | $E$               | 98         | 0.85     | 5531.717361(1)             |                          |
| 3907  | $A_1$             | 97         | 1.4      | 5532.251979(2)             |                          |
| 3908  | $A_1$             | 86         | 2.3      | 5532.37970(1)              |                          |
| 3909  | $A_2$             | 82         | 2.3      | 5532.37970(3)              |                          |
| 3910  | $E$               | 96         | 2.2      | 5532.50852(1)              |                          |
| 3911  | $E$               | 101        | 2.2      | 5532.50852(1)              |                          |
| 3912  | $A_1$             | 98         | 0.59     | 5532.545731(2)             |                          |
| 3913  | $A_2$             | 130        | 2.1      | 5532.749007(3)             |                          |
| 3914  | $E$               | 130        | 2.1      | 5534.157946(2)             |                          |
| 3915  | $E$               | 127        | 2.1      | 5534.157947(3)             |                          |
| 3916  | $A_1$             | 133        | 2.1      | 5535.335103(3)             |                          |
| 3917  | $E$               | 93         | 2.4      | 5536.24821(4)              |                          |
| 3918  | $E$               | 131        | 2.4      | 5536.24821(3)              |                          |
| 3919  | $A_2^*$           | 87         | 2.3      | 5536.51648(2)              |                          |
| 3920  | $A_1^*$           | 87         | 2.3      | 5536.51648(2)              |                          |
| 3921  | $E$               | 98         | 2.3      | 5536.60051(1)              |                          |
| 3922  | $E$               | 103        | 2.3      | 5536.60051(1)              |                          |
| 3923  | $A_1$             | 83         | 2.3      | 5536.70936(3)              |                          |
| 3924  | $A_2$             | 84         | 2.3      | 5536.70959(2)              |                          |
| 3925  | $E$               | 103        | 0.5      | 5538.117324(9)             |                          |
| 3926  | $E$               | 90         | 0.51     | 5538.11733(2)              |                          |
| 3927  | $E$               | 121        | 2.3      | 5538.333776(4)             |                          |
| 3928  | $E$               | 120        | 2.3      | 5538.333776(4)             |                          |
| 3929  | $A_2$             | 100        | 2.8      | 5538.600037(2)             |                          |
| 3930  | $A_2$             | 159        | 3.6      | 5539.120566(3)             |                          |
| 3931  | $A_1$             | 136        | 3.2      | 5539.201273(4)             |                          |
| 3932  | $E$               | 135        | 3.2      | 5539.243603(2)             |                          |
| 3933  | $E$               | 135        | 3.2      | 5539.243604(1)             |                          |
| 3934  | $E$               | 105        | 2.8      | 5539.533365(2)             |                          |
| 3935  | $E$               | 109        | 2.8      | 5539.533365(1)             |                          |
| 3936  | $E$               | 118        | 2.2      | 5539.638751(7)             |                          |
| 3937  | $E$               | 121        | 2.2      | 5539.638752(7)             |                          |
| 3938  | $A_2$             | 132        | 2.8      | 5539.897779(2)             |                          |

Continued on next page.

TABLE S4 – states on Sarka/Poirier CSC PES; continued from previous page

| State | $\Gamma_{C_{3v}}$ | $D_{\max}$ | $S_{vN}$ | $\tilde{E}/\text{cm}^{-1}$ | $\Delta\text{Ref. [30]}$ |
|-------|-------------------|------------|----------|----------------------------|--------------------------|
| 3939  | $A_1$             | 108        | 2.8      | 5539.982378(2)             |                          |
| 3940  | $E$               | 119        | 2.2      | 5540.706019(4)             |                          |
| 3941  | $E$               | 114        | 2.3      | 5540.706020(3)             |                          |
| 3942  | $E$               | 89         | 1.4      | 5541.061819(3)             |                          |
| 3943  | $E$               | 93         | 1.4      | 5541.061819(3)             |                          |
| 3944  | $A_1$             | 105        | 2.2      | 5541.110450(3)             |                          |
| 3945  | $A_2$             | 112        | 2.5      | 5544.706396(7)             |                          |
| 3946  | $E$               | 107        | 2.5      | 5544.80631(1)              |                          |
| 3947  | $E$               | 109        | 2.5      | 5544.80631(1)              |                          |
| 3948  | $A_1$             | 105        | 2.5      | 5544.915140(4)             |                          |
| 3949  | $E$               | 135        | 2.0      | 5544.935570(2)             |                          |
| 3950  | $E$               | 133        | 2.0      | 5544.935570(2)             |                          |
| 3951  | $E$               | 106        | 0.47     | 5545.109475(3)             |                          |
| 3952  | $E$               | 106        | 0.47     | 5545.109480(5)             |                          |
| 3953  | $E$               | 90         | 1.6      | 5545.323115(3)             |                          |
| 3954  | $E$               | 84         | 1.6      | 5545.323116(3)             |                          |
| 3955  | $E$               | 99         | 2.4      | 5545.49721(2)              |                          |
| 3956  | $E$               | 108        | 2.4      | 5545.49721(2)              |                          |
| 3957  | $E$               | 123        | 1.9      | 5545.544831(3)             |                          |
| 3958  | $E$               | 120        | 1.9      | 5545.544832(3)             |                          |
| 3959  | $E$               | 107        | 2.4      | 5545.72405(1)              |                          |
| 3960  | $E$               | 107        | 2.4      | 5545.72405(1)              |                          |
| 3961  | $A_1$             | 93         | 1.7      | 5546.743788(3)             |                          |
| 3962  | $E$               | 155        | 2.7      | 5549.480139(3)             |                          |
| 3963  | $E$               | 155        | 2.7      | 5549.480140(3)             |                          |
| 3964  | $E$               | 142        | 2.7      | 5549.500921(4)             |                          |
| 3965  | $E$               | 156        | 2.7      | 5549.500923(5)             |                          |
| 3966  | $A_2$             | 155        | 2.7      | 5552.019134(2)             |                          |
| 3967  | $E$               | 133        | 2.7      | 5552.066242(2)             |                          |
| 3968  | $E$               | 138        | 2.7      | 5552.066244(3)             |                          |
| 3969  | $A_2$             | 97         | 2.0      | 5552.087270(9)             |                          |
| 3970  | $A_1$             | 98         | 2.0      | 5552.08727(1)              |                          |
| 3971  | $A_1$             | 87         | 2.5      | 5552.09993(8)              |                          |
| 3972  | $A_2$             | 88         | 2.5      | 5552.09997(5)              |                          |
| 3973  | $E$               | 95         | 2.4      | 5552.30089(6)              |                          |
| 3974  | $E$               | 110        | 2.4      | 5552.30089(4)              |                          |
| 3975  | $E$               | 154        | 2.7      | 5552.448733(3)             |                          |
| 3976  | $E$               | 149        | 2.7      | 5552.448734(2)             |                          |
| 3977  | $E$               | 76         | 2.1      | 5552.60342(8)              |                          |
| 3978  | $E$               | 143        | 2.1      | 5552.60343(7)              |                          |
| 3979  | $A_1$             | 77         | 2.1      | 5552.62584(6)              |                          |
| 3980  | $A_2$             | 83         | 2.1      | 5552.62585(6)              |                          |
| 3981  | $A_1$             | 142        | 2.7      | 5552.808637(3)             |                          |
| 3982  | $E$               | 129        | 1.3      | 5553.546093(2)             |                          |
| 3983  | $E$               | 169        | 1.3      | 5553.546103(9)             |                          |
| 3984  | $E$               | 136        | 2.5      | 5555.992949(2)             |                          |
| 3985  | $E$               | 104        | 2.5      | 5555.99295(1)              |                          |
| 3986  | $A_1$             | 87         | 2.5      | 5556.25215(4)              |                          |
| 3987  | $A_2$             | 80         | 2.5      | 5556.25254(6)              |                          |
| 3988  | $E$               | 118        | 2.5      | 5556.56879(1)              |                          |
| 3989  | $E$               | 106        | 2.5      | 5556.56879(2)              |                          |
| 3990  | $E$               | 120        | 2.4      | 5556.78925(1)              |                          |
| 3991  | $E$               | 111        | 2.4      | 5556.78925(1)              |                          |
| 3992  | $A_1$             | 91         | 2.2      | 5556.90860(3)              |                          |
| 3993  | $A_2$             | 84         | 2.2      | 5556.90968(4)              |                          |
| 3994  | $E$               | 82         | 2.2      | 5556.92037(5)              |                          |
| 3995  | $E$               | 79         | 2.2      | 5556.92037(7)              |                          |
| 3996  | $E$               | 92         | 0.99     | 5557.63750(2)              |                          |
| 3997  | $E$               | 88         | 1.0      | 5557.63750(2)              |                          |

Continued on next page.

TABLE S4 – states on Sarka/Poirier CSC PES; continued from previous page

| State | $\Gamma_{C_{3v}}$ | $D_{\max}$ | $S_{vN}$ | $\tilde{E}/\text{cm}^{-1}$ | $\Delta\text{Ref. [30]}$ |
|-------|-------------------|------------|----------|----------------------------|--------------------------|
| 3998  | $E$               | 73         | 0.94     | 5557.716281(1)             |                          |
| 3999  | $E$               | 76         | 0.94     | 5557.716281(2)             |                          |
| 4000  | $E$               | 112        | 2.4      | 5557.827924(8)             |                          |
| 4001  | $E$               | 122        | 2.4      | 5557.827926(9)             |                          |
| 4002  | $A_2^*$           | 82         | 2.3      | 5557.96589(2)              |                          |
| 4003  | $A_1^*$           | 83         | 2.3      | 5557.96589(3)              |                          |
| 4004  | $E$               | 120        | 0.22     | 5558.348386(2)             |                          |
| 4005  | $E$               | 118        | 0.22     | 5558.348386(2)             |                          |
| 4006  | $A_2$             | 113        | 1.5      | 5558.86524(1)              |                          |
| 4007  | $A_1$             | 103        | 1.5      | 5558.86529(3)              |                          |
| 4008  | $E$               | 150        | 2.1      | 5560.455485(5)             |                          |
| 4009  | $E$               | 137        | 2.1      | 5560.455489(5)             |                          |
| 4010  | $A_2$             | 119        | 2.8      | 5560.64119(1)              |                          |
| 4011  | $A_1$             | 115        | 2.8      | 5560.64120(2)              |                          |
| 4012  | $E$               | 124        | 0.87     | 5561.710169(3)             |                          |
| 4013  | $E$               | 148        | 0.87     | 5561.710170(3)             |                          |
| 4014  | $A_2^*$           | 113        | 2.0      | 5563.405896(7)             |                          |
| 4015  | $A_1^*$           | 129        | 2.0      | 5563.405897(7)             |                          |
| 4016  | $E$               | 103        | 2.7      | 5563.43247(2)              |                          |
| 4017  | $E$               | 94         | 2.7      | 5563.43247(3)              |                          |
| 4018  | $A_2$             | 145        | 2.1      | 5563.457154(5)             |                          |
| 4019  | $A_1$             | 123        | 2.1      | 5563.457714(7)             |                          |
| 4020  | $E$               | 119        | 2.7      | 5563.53254(1)              |                          |
| 4021  | $E$               | 167        | 2.7      | 5563.53254(1)              |                          |
| 4022  | $A_2$             | 93         | 2.7      | 5563.60752(8)              |                          |
| 4023  | $A_1$             | 108        | 2.7      | 5563.60753(9)              |                          |
| 4024  | $E$               | 113        | 2.6      | 5563.77153(3)              |                          |
| 4025  | $E$               | 104        | 2.6      | 5563.77154(4)              |                          |
| 4026  | $A_2^*$           | 89         | 2.0      | 5565.859336(7)             |                          |
| 4027  | $A_1^*$           | 88         | 2.0      | 5565.859336(6)             |                          |
| 4028  | $E$               | 88         | 2.1      | 5565.91979(1)              |                          |
| 4029  | $E$               | 95         | 2.1      | 5565.91979(1)              |                          |
| 4030  | $E$               | 124        | 2.2      | 5566.04351(1)              |                          |
| 4031  | $E$               | 123        | 2.2      | 5566.04351(1)              |                          |
| 4032  | $A_1$             | 110        | 2.9      | 5566.05363(1)              |                          |
| 4033  | $E$               | 144        | 2.5      | 5566.120471(3)             |                          |
| 4034  | $E$               | 138        | 2.5      | 5566.120477(7)             |                          |
| 4035  | $E$               | 94         | 2.8      | 5566.31055(1)              |                          |
| 4036  | $E$               | 102        | 2.8      | 5566.31055(1)              |                          |
| 4037  | $E$               | 149        | 1.9      | 5566.331062(2)             |                          |
| 4038  | $E$               | 142        | 1.9      | 5566.331063(2)             |                          |
| 4039  | $E$               | 145        | 2.1      | 5566.352189(3)             |                          |
| 4040  | $E$               | 128        | 2.1      | 5566.35219(1)              |                          |
| 4041  | $A_2$             | 90         | 2.8      | 5566.484280(1)             |                          |
| 4042  | $E$               | 116        | 2.7      | 5567.81573(2)              |                          |
| 4043  | $E$               | 113        | 2.7      | 5567.81573(3)              |                          |
| 4044  | $A_1$             | 127        | 2.7      | 5567.95335(1)              |                          |
| 4045  | $A_2$             | 92         | 2.7      | 5567.9537(1)               |                          |
| 4046  | $A_2$             | 127        | 2.2      | 5568.848794(3)             |                          |
| 4047  | $A_1$             | 105        | 2.2      | 5568.850817(8)             |                          |
| 4048  | $E$               | 123        | 2.2      | 5568.875478(3)             |                          |
| 4049  | $E$               | 120        | 2.2      | 5568.875480(4)             |                          |
| 4050  | $E$               | 113        | 0.93     | 5569.35681(1)              |                          |
| 4051  | $E$               | 114        | 0.93     | 5569.35681(1)              |                          |
| 4052  | $E$               | 148        | 2.5      | 5571.806906(3)             |                          |
| 4053  | $E$               | 127        | 2.5      | 5571.80691(2)              |                          |
| 4054  | $A_1$             | 137        | 4.0      | 5572.432850(5)             |                          |
| 4055  | $A_2$             | 162        | 3.9      | 5572.569066(6)             |                          |
| 4056  | $A_1$             | 181        | 3.4      | 5572.666027(6)             |                          |

Continued on next page.

TABLE S4 – states on Sarka/Poirier CSC PES; continued from previous page

| State | $\Gamma_{C_{3v}}$ | $D_{\max}$ | $S_{vN}$ | $\tilde{E}/\text{cm}^{-1}$ | $\Delta\text{Ref. [30]}$ |
|-------|-------------------|------------|----------|----------------------------|--------------------------|
| 4057  | $E$               | 149        | 3.4      | 5572.725927(5)             |                          |
| 4058  | $E$               | 195        | 3.4      | 5572.72594(1)              |                          |
| 4059  | $E$               | 166        | 2.4      | 5573.101493(5)             |                          |
| 4060  | $E$               | 172        | 2.4      | 5573.101494(5)             |                          |
| 4061  | $A_2$             | 163        | 3.0      | 5573.392210(3)             |                          |
| 4062  | $E$               | 120        | 0.41     | 5573.65895(1)              |                          |
| 4063  | $E$               | 120        | 0.41     | 5573.658955(4)             |                          |
| 4064  | $E$               | 157        | 2.5      | 5574.079767(3)             |                          |
| 4065  | $E$               | 152        | 2.5      | 5574.079768(3)             |                          |
| 4066  | $E$               | 146        | 2.5      | 5574.18325(1)              |                          |
| 4067  | $E$               | 144        | 2.5      | 5574.183257(6)             |                          |
| 4068  | $E$               | 114        | 1.1      | 5574.323104(1)             |                          |
| 4069  | $E$               | 79         | 1.1      | 5574.323107(3)             |                          |
| 4070  | $A_1$             | 101        | 2.2      | 5574.376407(2)             |                          |
| 4071  | $A_2$             | 145        | 2.1      | 5574.411501(2)             |                          |
| 4072  | $E$               | 98         | 2.1      | 5574.506610(6)             |                          |
| 4073  | $E$               | 101        | 2.1      | 5574.506611(6)             |                          |
| 4074  | $A_2$             | 96         | 2.1      | 5574.547302(8)             |                          |
| 4075  | $A_1$             | 129        | 2.4      | 5574.572554(5)             |                          |
| 4076  | $A_1$             | 159        | 4.2      | 5575.071393(3)             |                          |
| 4077  | $E$               | 68         | 0.13     | 5577.642874(2)             |                          |
| 4078  | $E$               | 58         | 0.13     | 5577.642875(2)             |                          |
| 4079  | $E$               | 90         | 0.46     | 5578.311966(5)             |                          |
| 4080  | $E$               | 89         | 0.46     | 5578.311967(6)             |                          |
| 4081  | $A_2$             | 101        | 2.0      | 5578.364736(1)             |                          |
| 4082  | $E$               | 154        | 2.5      | 5578.86547(1)              |                          |
| 4083  | $E$               | 143        | 2.5      | 5578.86547(1)              |                          |
| 4084  | $E$               | 98         | 2.0      | 5579.015270(1)             |                          |
| 4085  | $E$               | 96         | 2.0      | 5579.015270(2)             |                          |
| 4086  | $E$               | 147        | 1.1      | 5579.106906(3)             |                          |
| 4087  | $E$               | 148        | 1.1      | 5579.106906(3)             |                          |
| 4088  | $E$               | 91         | 2.2      | 5579.19997(1)              |                          |
| 4089  | $E$               | 105        | 2.2      | 5579.199966(7)             |                          |
| 4090  | $E$               | 91         | 2.2      | 5579.22965(1)              |                          |
| 4091  | $E$               | 97         | 2.2      | 5579.229648(7)             |                          |
| 4092  | $A_1^*$           | 119        | 2.2      | 5579.291758(7)             |                          |
| 4093  | $A_2^*$           | 117        | 2.2      | 5579.291759(6)             |                          |
| 4094  | $A_1$             | 102        | 2.0      | 5579.768373(1)             |                          |
| 4095  | $E$               | 163        | 0.7      | 5581.964351(9)             |                          |
| 4096  | $E$               | 150        | 0.71     | 5581.96435(1)              |                          |
| 4097  | $E$               | 189        | 2.9      | 5583.730689(4)             |                          |
| 4098  | $E$               | 174        | 2.8      | 5583.730696(8)             |                          |
| 4099  | $E$               | 165        | 2.8      | 5583.736397(4)             |                          |
| 4100  | $E$               | 187        | 2.8      | 5583.736401(7)             |                          |
| 4101  | $E$               | 177        | 3.0      | 5584.254771(3)             |                          |
| 4102  | $E$               | 147        | 3.0      | 5584.254776(5)             |                          |
| 4103  | $E$               | 151        | 3.0      | 5584.258580(2)             |                          |
| 4104  | $E$               | 156        | 3.0      | 5584.258581(3)             |                          |
| 4105  | $E$               | 117        | 2.2      | 5584.593703(2)             |                          |
| 4106  | $E$               | 140        | 2.2      | 5584.593705(3)             |                          |
| 4107  | $E$               | 148        | 0.58     | 5585.156978(3)             |                          |
| 4108  | $E$               | 139        | 0.57     | 5585.156978(5)             |                          |
| 4109  | $E$               | 97         | 3.1      | 5585.49471(1)              |                          |
| 4110  | $E$               | 98         | 3.1      | 5585.49471(1)              |                          |
| 4111  | $A_1$             | 95         | 3.2      | 5585.49629(1)              |                          |
| 4112  | $A_2$             | 95         | 3.2      | 5585.49708(1)              |                          |
| 4113  | $E$               | 149        | 0.54     | 5585.837128(3)             |                          |
| 4114  | $E$               | 149        | 0.54     | 5585.837129(3)             |                          |
| 4115  | $E$               | 112        | 2.2      | 5585.916544(2)             |                          |

Continued on next page.

TABLE S4 – states on Sarka/Poirier CSC PES; continued from previous page

| State | $\Gamma_{C_{3v}}$ | $D_{\max}$ | $S_{vN}$ | $\tilde{E}/\text{cm}^{-1}$ | $\Delta\text{Ref. [30]}$ |
|-------|-------------------|------------|----------|----------------------------|--------------------------|
| 4116  | $E$               | 104        | 2.2      | 5585.916547(4)             |                          |
| 4117  | $A_2$             | 202        | 2.9      | 5586.359491(5)             |                          |
| 4118  | $E$               | 201        | 2.9      | 5586.632784(9)             |                          |
| 4119  | $E$               | 207        | 2.9      | 5586.63279(1)              |                          |
| 4120  | $E$               | 95         | 0.53     | 5586.659000(8)             |                          |
| 4121  | $E$               | 113        | 0.53     | 5586.659000(9)             |                          |
| 4122  | $A_1$             | 187        | 3.0      | 5586.87272(1)              |                          |
| 4123  | $A_2$             | 149        | 3.0      | 5586.953693(3)             |                          |
| 4124  | $A_2$             | 114        | 3.8      | 5586.9822(1)               |                          |
| 4125  | $A_1$             | 122        | 3.9      | 5586.9827(1)               |                          |
| 4126  | $E$               | 149        | 3.0      | 5587.177708(3)             |                          |
| 4127  | $E$               | 139        | 3.0      | 5587.177710(7)             |                          |
| 4128  | $A_1$             | 156        | 3.0      | 5587.387950(4)             |                          |
| 4129  | $E$               | 135        | 2.4      | 5587.53321(1)              |                          |
| 4130  | $E$               | 138        | 2.4      | 5587.53321(1)              |                          |
| 4131  | $A_1$             | 141        | 3.1      | 5587.71720(7)              |                          |
| 4132  | $A_2$             | 129        | 3.1      | 5587.71722(6)              |                          |
| 4133  | $E$               | 194        | 3.5      | 5589.189432(3)             |                          |
| 4134  | $E$               | 192        | 3.5      | 5589.189434(4)             |                          |
| 4135  | $E$               | 199        | 3.3      | 5589.342206(8)             |                          |
| 4136  | $E$               | 179        | 3.3      | 5589.34222(1)              |                          |
| 4137  | $A_1$             | 156        | 3.4      | 5589.50670(1)              |                          |
| 4138  | $A_2$             | 159        | 3.4      | 5589.50689(1)              |                          |
| 4139  | $A_1^*$           | 129        | 3.1      | 5589.64168(3)              |                          |
| 4140  | $A_2^*$           | 127        | 3.1      | 5589.64168(3)              |                          |
| 4141  | $A_1^*$           | 98         | 2.2      | 5589.676707(6)             |                          |
| 4142  | $A_2^*$           | 81         | 2.2      | 5589.676708(9)             |                          |
| 4143  | $E$               | 93         | 2.2      | 5589.694606(6)             |                          |
| 4144  | $E$               | 95         | 2.2      | 5589.694607(7)             |                          |
| 4145  | $A_2$             | 90         | 2.3      | 5589.87660(1)              |                          |
| 4146  | $A_1$             | 90         | 2.3      | 5589.876602(7)             |                          |
| 4147  | $E$               | 92         | 2.3      | 5589.883730(6)             |                          |
| 4148  | $E$               | 95         | 2.3      | 5589.88373(1)              |                          |
| 4149  | $E$               | 158        | 1.1      | 5590.157481(7)             |                          |
| 4150  | $E$               | 130        | 1.1      | 5590.157487(6)             |                          |
| 4151  | $A_1$             | 138        | 3.5      | 5592.08608(3)              |                          |
| 4152  | $E$               | 136        | 2.9      | 5592.10484(2)              |                          |
| 4153  | $E$               | 143        | 2.9      | 5592.10484(4)              |                          |
| 4154  | $A_2$             | 182        | 3.5      | 5592.197522(5)             |                          |
| 4155  | $A_1$             | 78         | 0.56     | 5592.22545(1)              |                          |
| 4156  | $A_2$             | 78         | 0.57     | 5592.22548(1)              |                          |
| 4157  | $E$               | 168        | 3.2      | 5592.496819(7)             |                          |
| 4158  | $E$               | 157        | 3.2      | 5592.496820(7)             |                          |
| 4159  | $E$               | 167        | 2.8      | 5592.530907(7)             |                          |
| 4160  | $E$               | 153        | 2.8      | 5592.530909(9)             |                          |
| 4161  | $E$               | 199        | 2.9      | 5592.883375(6)             |                          |
| 4162  | $E$               | 135        | 2.9      | 5592.88339(1)              |                          |
| 4163  | $E$               | 171        | 2.6      | 5593.012590(8)             |                          |
| 4164  | $E$               | 112        | 2.6      | 5593.01261(8)              |                          |
| 4165  | $A_1^*$           | 52         | 0.16     | 5593.78727(2)              |                          |
| 4166  | $A_2^*$           | 51         | 0.16     | 5593.78728(2)              |                          |
| 4167  | $E$               | 128        | 0.58     | 5595.009199(1)             |                          |
| 4168  | $E$               | 84         | 0.58     | 5595.009204(5)             |                          |
| 4169  | $E$               | 96         | 2.2      | 5595.364305(5)             |                          |
| 4170  | $E$               | 96         | 2.2      | 5595.364306(5)             |                          |
| 4171  | $E$               | 122        | 2.2      | 5595.385865(3)             |                          |
| 4172  | $E$               | 92         | 2.2      | 5595.385866(6)             |                          |
| 4173  | $E$               | 120        | 2.6      | 5595.680941(4)             |                          |
| 4174  | $E$               | 107        | 2.6      | 5595.68095(2)              |                          |

Continued on next page.



TABLE S4 – states on Sarka/Poirier CSC PES; continued from previous page

| State | $\Gamma_{C_{3v}}$ | $D_{\max}$ | $S_{vN}$ | $\tilde{E}/\text{cm}^{-1}$ | $\Delta\text{Ref. [30]}$ |
|-------|-------------------|------------|----------|----------------------------|--------------------------|
| 4175  | $A_1$             | 112        | 2.7      | 5595.72058(3)              |                          |
| 4176  | $A_2$             | 119        | 2.6      | 5595.73475(1)              |                          |
| 4177  | $E$               | 104        | 0.41     | 5595.815467(9)             |                          |
| 4178  | $E$               | 136        | 0.42     | 5595.815470(9)             |                          |
| 4179  | $E$               | 131        | 2.3      | 5597.850146(4)             |                          |
| 4180  | $E$               | 92         | 2.3      | 5597.85016(3)              |                          |
| 4181  | $A_2$             | 91         | 2.3      | 5597.90851(3)              |                          |
| 4182  | $A_1$             | 91         | 2.3      | 5597.90852(4)              |                          |
| 4183  | $A_2$             | 93         | 2.2      | 5597.931590(9)             |                          |
| 4184  | $E$               | 96         | 2.2      | 5598.258846(3)             |                          |
| 4185  | $E$               | 96         | 2.2      | 5598.258847(1)             |                          |
| 4186  | $A_1$             | 97         | 2.2      | 5598.539526(2)             |                          |
| 4187  | $E$               | 104        | 2.4      | 5603.11879(1)              |                          |
| 4188  | $E$               | 105        | 2.4      | 5603.11879(1)              |                          |
| 4189  | $E$               | 148        | 2.4      | 5603.277257(2)             |                          |
| 4190  | $E$               | 103        | 2.4      | 5603.27726(2)              |                          |
| 4191  | $A_1$             | 72         | 0.03     | 5603.800178(1)             |                          |
| 4192  | $A_2$             | 59         | 0.03     | 5603.800181(1)             |                          |
| 4193  | $E$               | 98         | 0.52     | 5604.263357(1)             |                          |
| 4194  | $E$               | 100        | 0.52     | 5604.263357(2)             |                          |
| 4195  | $E$               | 87         | 0.25     | 5604.691083(2)             |                          |
| 4196  | $E$               | 82         | 0.25     | 5604.691083(4)             |                          |
| 4197  | $A_2$             | 100        | 2.4      | 5605.316780(4)             |                          |
| 4198  | $E$               | 98         | 2.4      | 5606.01615(1)              |                          |
| 4199  | $E$               | 96         | 2.4      | 5606.016154(6)             |                          |
| 4200  | $A_1$             | 116        | 2.4      | 5606.487703(3)             |                          |
| 4201  | $E$               | 128        | 2.3      | 5607.919848(7)             |                          |
| 4202  | $E$               | 108        | 2.3      | 5607.91985(2)              |                          |
| 4203  | $A_2$             | 94         | 2.1      | 5608.00666(3)              |                          |
| 4204  | $A_1$             | 92         | 2.1      | 5608.00684(4)              |                          |
| 4205  | $E$               | 129        | 0.36     | 5609.574886(2)             |                          |
| 4206  | $E$               | 128        | 0.36     | 5609.574886(2)             |                          |
| 4207  | $A_1$             | 153        | 0.43     | 5611.037835(4)             |                          |
| 4208  | $A_2$             | 80         | 2.1      | 5611.249153(6)             |                          |
| 4209  | $A_1$             | 78         | 2.1      | 5611.249626(7)             |                          |
| 4210  | $E$               | 77         | 2.1      | 5611.26185(1)              |                          |
| 4211  | $E$               | 75         | 2.1      | 5611.26185(1)              |                          |
| 4212  | $E$               | 87         | 0.31     | 5612.872850(5)             |                          |
| 4213  | $E$               | 87         | 0.31     | 5612.872850(5)             |                          |
| 4214  | $A_2$             | 142        | 2.3      | 5614.981803(2)             |                          |
| 4215  | $A_1$             | 139        | 2.4      | 5614.996900(3)             |                          |
| 4216  | $E$               | 146        | 2.3      | 5615.146144(4)             |                          |
| 4217  | $E$               | 144        | 2.3      | 5615.146149(5)             |                          |
| 4218  | $E$               | 121        | 0.31     | 5616.541985(2)             |                          |
| 4219  | $E$               | 119        | 0.31     | 5616.541986(2)             |                          |
| 4220  | $A_1$             | 62         | 0.34     | 5618.32921(6)              |                          |
| 4221  | $A_2$             | 62         | 0.34     | 5618.32927(4)              |                          |
| 4222  | $E$               | 60         | 0.45     | 5618.793647(3)             |                          |
| 4223  | $E$               | 67         | 0.46     | 5618.793647(1)             |                          |
| 4224  | $A_1$             | 51         | 0.13     | 5618.870583(3)             |                          |
| 4225  | $A_2$             | 50         | 0.13     | 5618.870586(4)             |                          |
| 4226  | $E$               | 83         | 0.45     | 5619.112251(2)             |                          |
| 4227  | $E$               | 74         | 0.45     | 5619.112251(6)             |                          |
| 4228  | $E$               | 87         | 0.36     | 5621.057969(2)             |                          |
| 4229  | $E$               | 90         | 0.36     | 5621.057969(2)             |                          |
| 4230  | $E$               | 84         | 0.24     | 5621.651820(2)             |                          |
| 4231  | $E$               | 80         | 0.24     | 5621.651820(2)             |                          |
| 4232  | $E$               | 79         | 0.15     | 5621.7853770(6)            |                          |
| 4233  | $E$               | 69         | 0.15     | 5621.785377(1)             |                          |

Continued on next page.

TABLE S4 – states on Sarka/Poirier CSC PES; continued from previous page

| State | $\Gamma_{C_{3v}}$ | $D_{\max}$ | $S_{vN}$ | $\tilde{E}/\text{cm}^{-1}$ | $\Delta\text{Ref. [30]}$ |
|-------|-------------------|------------|----------|----------------------------|--------------------------|
| 4234  | $A_1$             | 97         | 2.3      | 5623.18094(4)              |                          |
| 4235  | $A_2$             | 91         | 2.3      | 5623.18094(8)              |                          |
| 4236  | $E$               | 92         | 2.3      | 5623.19794(7)              |                          |
| 4237  | $E$               | 90         | 2.3      | 5623.19794(9)              |                          |
| 4238  | $E$               | 63         | 0.11     | 5623.50109(1)              |                          |
| 4239  | $E$               | 64         | 0.11     | 5623.50109(1)              |                          |
| 4240  | $A_2$             | 66         | 0.4      | 5625.19485(1)              |                          |
| 4241  | $A_1$             | 59         | 0.4      | 5625.19486(2)              |                          |
| 4242  | $E$               | 86         | 1.9      | 5627.406493(6)             |                          |
| 4243  | $E$               | 96         | 1.9      | 5627.406495(7)             |                          |
| 4244  | $E$               | 86         | 0.15     | 5627.819203(2)             |                          |
| 4245  | $E$               | 86         | 0.15     | 5627.819204(2)             |                          |
| 4246  | $E$               | 79         | 2.3      | 5628.17446(1)              |                          |
| 4247  | $E$               | 124        | 2.3      | 5628.17447(2)              |                          |
| 4248  | $A_2^*$           | 88         | 2.3      | 5628.18456(1)              |                          |
| 4249  | $A_1^*$           | 87         | 2.3      | 5628.18456(1)              |                          |
| 4250  | $A_2$             | 70         | 1.1      | 5628.52057(5)              |                          |
| 4251  | $A_1$             | 74         | 1.1      | 5628.52057(6)              |                          |
| 4252  | $E$               | 106        | 2.5      | 5628.84807(2)              |                          |
| 4253  | $E$               | 97         | 2.5      | 5628.84808(2)              |                          |
| 4254  | $E$               | 99         | 2.4      | 5628.87046(2)              |                          |
| 4255  | $E$               | 122        | 2.4      | 5628.87047(2)              |                          |
| 4256  | $A_1$             | 62         | 0.15     | 5629.258781(9)             |                          |
| 4257  | $A_2$             | 120        | 2.5      | 5631.40514(1)              |                          |
| 4258  | $E$               | 109        | 2.5      | 5631.73366(1)              |                          |
| 4259  | $E$               | 127        | 2.5      | 5631.73366(1)              |                          |
| 4260  | $A_1$             | 107        | 2.5      | 5632.01472(1)              |                          |
| 4261  | $E$               | 92         | 2.5      | 5632.400316(4)             |                          |
| 4262  | $E$               | 131        | 2.5      | 5632.40033(1)              |                          |
| 4263  | $A_1$             | 89         | 2.5      | 5632.443138(7)             |                          |
| 4264  | $A_2$             | 101        | 2.5      | 5632.443296(7)             |                          |
| 4265  | $E$               | 179        | 2.9      | 5632.663112(9)             |                          |
| 4266  | $E$               | 186        | 2.9      | 5632.663112(9)             |                          |
| 4267  | $E$               | 162        | 3.1      | 5632.723909(4)             |                          |
| 4268  | $E$               | 167        | 3.1      | 5632.723913(6)             |                          |
| 4269  | $E$               | 102        | 0.79     | 5633.899965(5)             |                          |
| 4270  | $E$               | 94         | 0.79     | 5633.899965(6)             |                          |
| 4271  | $A_2$             | 101        | 2.3      | 5634.527765(1)             |                          |
| 4272  | $E$               | 106        | 2.3      | 5635.030603(3)             |                          |
| 4273  | $E$               | 107        | 2.3      | 5635.030603(1)             |                          |
| 4274  | $E$               | 137        | 0.64     | 5635.210171(1)             |                          |
| 4275  | $E$               | 110        | 0.64     | 5635.210172(3)             |                          |
| 4276  | $E$               | 94         | 1.4      | 5635.243324(5)             |                          |
| 4277  | $E$               | 109        | 1.4      | 5635.243324(4)             |                          |
| 4278  | $A_1$             | 166        | 3.1      | 5635.278317(6)             |                          |
| 4279  | $A_1$             | 112        | 2.2      | 5635.587037(3)             |                          |
| 4280  | $E$               | 177        | 2.8      | 5635.686827(8)             |                          |
| 4281  | $E$               | 168        | 2.8      | 5635.686834(7)             |                          |
| 4282  | $A_2$             | 138        | 2.5      | 5636.00088(1)              |                          |
| 4283  | $E$               | 93         | 0.66     | 5636.031755(3)             |                          |
| 4284  | $E$               | 90         | 0.66     | 5636.031755(8)             |                          |
| 4285  | $E$               | 103        | 0.38     | 5636.966986(1)             |                          |
| 4286  | $E$               | 105        | 0.38     | 5636.966987(1)             |                          |
| 4287  | $E$               | 95         | 0.57     | 5638.645192(1)             |                          |
| 4288  | $E$               | 87         | 0.57     | 5638.645193(3)             |                          |
| 4289  | $E$               | 90         | 1.5      | 5639.279131(4)             |                          |
| 4290  | $E$               | 99         | 1.5      | 5639.279131(3)             |                          |
| 4291  | $E$               | 162        | 1.1      | 5639.538154(6)             |                          |
| 4292  | $E$               | 164        | 1.1      | 5639.538155(7)             |                          |

Continued on next page.

TABLE S4 – states on Sarka/Poirier CSC PES; continued from previous page

| State | $\Gamma_{C_{3v}}$ | $D_{\max}$ | $S_{vN}$ | $\tilde{E}/\text{cm}^{-1}$ | $\Delta\text{Ref. [30]}$ |
|-------|-------------------|------------|----------|----------------------------|--------------------------|
| 4293  | $E$               | 122        | 0.7      | 5639.930684(2)             |                          |
| 4294  | $E$               | 119        | 0.7      | 5639.930684(8)             |                          |
| 4295  | $E$               | 121        | 6.3      | 5640.483790(9)             |                          |
| 4296  | $E$               | 156        | 6.2      | 5640.483791(9)             |                          |
| 4297  | $A_1$             | 93         | 1.6      | 5640.624688(2)             |                          |
| 4298  | $A_1$             | 128        | 2.5      | 5640.666571(4)             |                          |
| 4299  | $A_2$             | 124        | 2.5      | 5640.670352(2)             |                          |
| 4300  | $E$               | 140        | 6.4      | 5640.743711(5)             |                          |
| 4301  | $E$               | 126        | 6.4      | 5640.743711(6)             |                          |
| 4302  | $A_2$             | 105        | 2.4      | 5643.220919(7)             |                          |
| 4303  | $E$               | 129        | 2.3      | 5643.229706(2)             |                          |
| 4304  | $E$               | 106        | 2.3      | 5643.229710(7)             |                          |
| 4305  | $A_1$             | 94         | 2.3      | 5643.24901(1)              |                          |
| 4306  | $A_1$             | 162        | 4.0      | 5643.43564(1)              |                          |
| 4307  | $A_2$             | 138        | 4.1      | 5643.43579(4)              |                          |
| 4308  | $E$               | 149        | 1.6      | 5643.680323(7)             |                          |
| 4309  | $E$               | 181        | 1.6      | 5643.68033(1)              |                          |
| 4310  | $A_1$             | 156        | 2.8      | 5643.69893(1)              |                          |
| 4311  | $A_2$             | 158        | 2.9      | 5643.699675(9)             |                          |
| 4312  | $E$               | 97         | 0.82     | 5644.163681(6)             |                          |
| 4313  | $E$               | 96         | 0.82     | 5644.163682(8)             |                          |
| 4314  | $A_1$             | 120        | 2.3      | 5644.591124(7)             |                          |
| 4315  | $A_2$             | 124        | 2.3      | 5644.591128(7)             |                          |
| 4316  | $E$               | 131        | 3.1      | 5644.96177(6)              |                          |
| 4317  | $E$               | 192        | 3.0      | 5644.96178(6)              |                          |
| 4318  | $A_1$             | 164        | 1.0      | 5645.117585(9)             |                          |
| 4319  | $E$               | 148        | 3.3      | 5645.396524(3)             |                          |
| 4320  | $E$               | 148        | 3.3      | 5645.396525(3)             |                          |
| 4321  | $E$               | 128        | 3.1      | 5645.550832(3)             |                          |
| 4322  | $E$               | 150        | 3.1      | 5645.55084(1)              |                          |
| 4323  | $A_2$             | 130        | 4.8      | 5645.61915(8)              |                          |
| 4324  | $A_1$             | 132        | 4.8      | 5645.61916(8)              |                          |
| 4325  | $A_1^*$           | 110        | 2.3      | 5645.907092(7)             |                          |
| 4326  | $A_2^*$           | 116        | 2.3      | 5645.90709(2)              |                          |
| 4327  | $E$               | 171        | 1.5      | 5646.54594(1)              |                          |
| 4328  | $E$               | 173        | 1.5      | 5646.545940(4)             |                          |
| 4329  | $E$               | 167        | 1.5      | 5646.728838(5)             |                          |
| 4330  | $E$               | 175        | 1.5      | 5646.728845(8)             |                          |
| 4331  | $A_2$             | 109        | 2.3      | 5646.96882(1)              |                          |
| 4332  | $A_1$             | 137        | 2.3      | 5646.969265(3)             |                          |
| 4333  | $E$               | 125        | 2.3      | 5646.981534(3)             |                          |
| 4334  | $E$               | 113        | 2.3      | 5646.98154(1)              |                          |
| 4335  | $A_1$             | 96         | 0.2      | 5648.312185(3)             |                          |
| 4336  | $E$               | 94         | 0.079    | 5648.553129(3)             |                          |
| 4337  | $E$               | 82         | 0.078    | 5648.553130(2)             |                          |
| 4338  | $E$               | 128        | 2.7      | 5648.746524(3)             |                          |
| 4339  | $E$               | 125        | 2.7      | 5648.746525(3)             |                          |
| 4340  | $E$               | 132        | 2.6      | 5648.803793(2)             |                          |
| 4341  | $E$               | 135        | 2.6      | 5648.803793(2)             |                          |
| 4342  | $A_1$             | 107        | 3.2      | 5648.881227(9)             |                          |
| 4343  | $A_2$             | 96         | 3.2      | 5648.92529(1)              |                          |
| 4344  | $E$               | 101        | 3.1      | 5648.95382(1)              |                          |
| 4345  | $E$               | 94         | 3.1      | 5648.95383(2)              |                          |
| 4346  | $A_2$             | 157        | 2.7      | 5649.22285(1)              |                          |
| 4347  | $A_1$             | 175        | 2.8      | 5649.286077(7)             |                          |
| 4348  | $E$               | 177        | 3.6      | 5649.50385(2)              |                          |
| 4349  | $E$               | 182        | 3.6      | 5649.50386(1)              |                          |
| 4350  | $A_1$             | 121        | 0.91     | 5649.586957(3)             |                          |
| 4351  | $A_2$             | 105        | 0.91     | 5649.587022(4)             |                          |

Continued on next page.

TABLE S4 – states on Sarka/Poirier CSC PES; continued from previous page

| State | $\Gamma_{C_{3v}}$ | $D_{\max}$ | $S_{vN}$ | $\tilde{E}/\text{cm}^{-1}$ | $\Delta\text{Ref. [30]}$ |
|-------|-------------------|------------|----------|----------------------------|--------------------------|
| 4352  | $A_1$             | 104        | 0.48     | 5649.739335(4)             |                          |
| 4353  | $A_2$             | 92         | 0.48     | 5649.739335(2)             |                          |
| 4354  | $E$               | 145        | 0.99     | 5650.762498(5)             |                          |
| 4355  | $E$               | 151        | 0.98     | 5650.762501(7)             |                          |
| 4356  | $E$               | 148        | 2.5      | 5651.59003(1)              |                          |
| 4357  | $E$               | 155        | 2.5      | 5651.59004(1)              |                          |
| 4358  | $E$               | 98         | 0.96     | 5652.299252(4)             |                          |
| 4359  | $E$               | 102        | 0.96     | 5652.299253(5)             |                          |
| 4360  | $E$               | 154        | 3.5      | 5652.386970(3)             |                          |
| 4361  | $E$               | 158        | 3.5      | 5652.386978(9)             |                          |
| 4362  | $A_1$             | 114        | 3.3      | 5652.53717(4)              |                          |
| 4363  | $A_2$             | 129        | 3.3      | 5652.53718(5)              |                          |
| 4364  | $A_2^*$           | 84         | 2.3      | 5652.65126(3)              |                          |
| 4365  | $A_1^*$           | 83         | 2.3      | 5652.65127(3)              |                          |
| 4366  | $E$               | 133        | 2.4      | 5652.899554(2)             |                          |
| 4367  | $E$               | 134        | 2.4      | 5652.899557(4)             |                          |
| 4368  | $E$               | 96         | 2.2      | 5652.952582(8)             |                          |
| 4369  | $E$               | 110        | 2.2      | 5652.95259(1)              |                          |
| 4370  | $E$               | 69         | 0.19     | 5653.744536(4)             |                          |
| 4371  | $E$               | 108        | 0.19     | 5653.744542(7)             |                          |
| 4372  | $E$               | 148        | 2.8      | 5655.774404(2)             |                          |
| 4373  | $E$               | 147        | 2.8      | 5655.774406(3)             |                          |
| 4374  | $E$               | 166        | 2.8      | 5656.150087(6)             |                          |
| 4375  | $E$               | 171        | 2.8      | 5656.150088(4)             |                          |
| 4376  | $A_2$             | 127        | 2.8      | 5656.21238(2)              |                          |
| 4377  | $A_1$             | 136        | 2.7      | 5656.21268(3)              |                          |
| 4378  | $A_2$             | 156        | 4.1      | 5656.275169(4)             |                          |
| 4379  | $A_1$             | 151        | 3.5      | 5656.649309(3)             |                          |
| 4380  | $A_1$             | 90         | 0.51     | 5656.727816(1)             |                          |
| 4381  | $E$               | 149        | 3.5      | 5656.732073(3)             |                          |
| 4382  | $E$               | 152        | 3.5      | 5656.732074(4)             |                          |
| 4383  | $E$               | 128        | 2.5      | 5657.09334(1)              |                          |
| 4384  | $E$               | 130        | 2.5      | 5657.093341(3)             |                          |
| 4385  | $A_2$             | 157        | 3.6      | 5657.58721(1)              |                          |
| 4386  | $E$               | 156        | 0.86     | 5657.657366(4)             |                          |
| 4387  | $E$               | 141        | 0.86     | 5657.657369(9)             |                          |
| 4388  | $E$               | 94         | 1.2      | 5657.70199(6)              |                          |
| 4389  | $E$               | 135        | 1.2      | 5657.70200(6)              |                          |
| 4390  | $E$               | 142        | 2.7      | 5658.160123(2)             |                          |
| 4391  | $E$               | 138        | 2.7      | 5658.160124(4)             |                          |
| 4392  | $A_1$             | 138        | 2.5      | 5658.503208(3)             |                          |
| 4393  | $E$               | 95         | 0.56     | 5659.963572(1)             |                          |
| 4394  | $E$               | 95         | 0.56     | 5659.963573(2)             |                          |
| 4395  | $A_2$             | 116        | 2.5      | 5661.39632(4)              |                          |
| 4396  | $A_1$             | 117        | 2.5      | 5661.39632(3)              |                          |
| 4397  | $E$               | 159        | 2.1      | 5661.803858(3)             |                          |
| 4398  | $E$               | 143        | 2.1      | 5661.803862(8)             |                          |
| 4399  | $A_1$             | 120        | 4.5      | 5663.01543(4)              |                          |
| 4400  | $A_2$             | 112        | 4.5      | 5663.02029(6)              |                          |
| 4401  | $E$               | 177        | 3.2      | 5663.139851(3)             |                          |
| 4402  | $E$               | 148        | 3.2      | 5663.139856(5)             |                          |
| 4403  | $A_2$             | 124        | 3.3      | 5663.27574(3)              |                          |
| 4404  | $A_1$             | 126        | 3.3      | 5663.27577(4)              |                          |
| 4405  | $E$               | 157        | 3.2      | 5663.35126(1)              |                          |
| 4406  | $E$               | 166        | 3.2      | 5663.351263(7)             |                          |
| 4407  | $E$               | 161        | 3.0      | 5663.636620(4)             |                          |
| 4408  | $E$               | 153        | 3.0      | 5663.636621(4)             |                          |
| 4409  | $E$               | 147        | 2.9      | 5663.670501(4)             |                          |
| 4410  | $E$               | 158        | 2.9      | 5663.670502(4)             |                          |

Continued on next page.

TABLE S4 – states on Sarka/Poirier CSC PES; continued from previous page

| State | $\Gamma_{C_{3v}}$ | $D_{\max}$ | $S_{vN}$ | $\tilde{E}/\text{cm}^{-1}$ | $\Delta\text{Ref. [30]}$ |
|-------|-------------------|------------|----------|----------------------------|--------------------------|
| 4411  | $E$               | 76         | 0.13     | 5663.703066(2)             |                          |
| 4412  | $E$               | 106        | 0.14     | 5663.703067(3)             |                          |
| 4413  | $E$               | 184        | 2.6      | 5664.572865(5)             |                          |
| 4414  | $E$               | 161        | 2.6      | 5664.572869(5)             |                          |
| 4415  | $E$               | 149        | 2.6      | 5664.704614(3)             |                          |
| 4416  | $E$               | 114        | 2.6      | 5664.70462(1)              |                          |
| 4417  | $E$               | 150        | 2.2      | 5664.786577(3)             |                          |
| 4418  | $E$               | 160        | 2.2      | 5664.786579(5)             |                          |
| 4419  | $A_1$             | 169        | 4.2      | 5664.837310(3)             |                          |
| 4420  | $A_2$             | 158        | 4.2      | 5664.837865(2)             |                          |
| 4421  | $E$               | 128        | 0.53     | 5664.905083(2)             |                          |
| 4422  | $E$               | 125        | 0.53     | 5664.905083(2)             |                          |
| 4423  | $A_1^*$           | 85         | 2.5      | 5664.95826(5)              |                          |
| 4424  | $A_2^*$           | 92         | 2.5      | 5664.95826(4)              |                          |
| 4425  | $A_2$             | 152        | 2.2      | 5665.114334(3)             |                          |
| 4426  | $A_1$             | 158        | 2.2      | 5665.132672(3)             |                          |
| 4427  | $E$               | 154        | 2.4      | 5665.788741(4)             |                          |
| 4428  | $E$               | 176        | 2.4      | 5665.788743(7)             |                          |
| 4429  | $A_2$             | 122        | 2.2      | 5665.99428(4)              |                          |
| 4430  | $A_1$             | 121        | 2.2      | 5665.99429(4)              |                          |
| 4431  | $E$               | 151        | 1.0      | 5666.091133(2)             |                          |
| 4432  | $E$               | 148        | 1.0      | 5666.091134(2)             |                          |
| 4433  | $E$               | 123        | 0.32     | 5667.32223(1)              |                          |
| 4434  | $E$               | 143        | 0.32     | 5667.322235(8)             |                          |
| 4435  | $E$               | 112        | 0.61     | 5667.635462(1)             |                          |
| 4436  | $E$               | 101        | 0.61     | 5667.635463(1)             |                          |
| 4437  | $A_1$             | 105        | 1.9      | 5668.5873775(8)            |                          |
| 4438  | $A_2$             | 99         | 1.9      | 5668.587380(2)             |                          |
| 4439  | $E$               | 107        | 2.3      | 5669.47317(2)              |                          |
| 4440  | $E$               | 105        | 2.3      | 5669.47317(1)              |                          |
| 4441  | $A_1$             | 104        | 2.2      | 5669.68032(2)              |                          |
| 4442  | $A_2$             | 104        | 2.2      | 5669.680324(1)             |                          |
| 4443  | $A_2$             | 83         | 2.1      | 5671.01741(2)              |                          |
| 4444  | $A_1$             | 87         | 2.1      | 5671.05046(2)              |                          |
| 4445  | $E$               | 130        | 2.1      | 5671.095766(2)             |                          |
| 4446  | $E$               | 130        | 2.1      | 5671.095766(2)             |                          |
| 4447  | $E$               | 70         | 1.9      | 5671.494678(9)             |                          |
| 4448  | $E$               | 94         | 1.9      | 5671.494678(7)             |                          |
| 4449  | $E$               | 93         | 0.74     | 5672.07195(1)              |                          |
| 4450  | $E$               | 98         | 0.74     | 5672.071948(3)             |                          |
| 4451  | $A_1$             | 97         | 0.64     | 5672.751683(1)             |                          |
| 4452  | $A_2$             | 104        | 0.64     | 5672.751966(1)             |                          |
| 4453  | $E$               | 97         | 3.0      | 5673.627234(1)             |                          |
| 4454  | $E$               | 93         | 3.0      | 5673.627234(1)             |                          |
| 4455  | $E$               | 163        | 2.8      | 5674.088074(2)             |                          |
| 4456  | $E$               | 164        | 2.8      | 5674.088074(2)             |                          |
| 4457  | $E$               | 113        | 2.7      | 5674.29714(1)              |                          |
| 4458  | $E$               | 99         | 2.7      | 5674.29714(4)              |                          |
| 4459  | $A_1$             | 85         | 3.1      | 5675.081115(2)             |                          |
| 4460  | $E$               | 108        | 2.3      | 5675.19592(3)              |                          |
| 4461  | $E$               | 115        | 2.3      | 5675.19592(4)              |                          |
| 4462  | $E$               | 93         | 0.66     | 5675.310536(2)             |                          |
| 4463  | $E$               | 82         | 0.66     | 5675.310538(3)             |                          |
| 4464  | $E$               | 109        | 2.2      | 5675.34060(2)              |                          |
| 4465  | $E$               | 108        | 2.2      | 5675.34060(2)              |                          |
| 4466  | $E$               | 163        | 1.2      | 5675.436173(5)             |                          |
| 4467  | $E$               | 162        | 1.3      | 5675.436173(6)             |                          |
| 4468  | $E$               | 116        | 1.1      | 5675.64521(1)              |                          |
| 4469  | $E$               | 117        | 1.1      | 5675.64521(1)              |                          |

Continued on next page.

TABLE S4 – states on Sarka/Poirier CSC PES; continued from previous page

| State | $\Gamma_{C_{3v}}$ | $D_{\max}$ | $S_{vN}$ | $\tilde{E}/\text{cm}^{-1}$ | $\Delta\text{Ref. [30]}$ |
|-------|-------------------|------------|----------|----------------------------|--------------------------|
| 4470  | $A_1$             | 133        | 0.36     | 5676.906954(2)             |                          |
| 4471  | $A_2$             | 98         | 0.35     | 5677.07831(6)              |                          |
| 4472  | $A_1$             | 107        | 2.3      | 5677.85787(2)              |                          |
| 4473  | $E$               | 104        | 2.3      | 5678.16062(1)              |                          |
| 4474  | $E$               | 123        | 2.3      | 5678.16062(2)              |                          |
| 4475  | $A_2$             | 103        | 2.2      | 5678.346651(1)             |                          |
| 4476  | $E$               | 87         | 2.1      | 5679.63332(1)              |                          |
| 4477  | $E$               | 90         | 2.1      | 5679.633321(9)             |                          |
| 4478  | $E$               | 90         | 2.1      | 5679.652154(6)             |                          |
| 4479  | $E$               | 90         | 2.1      | 5679.65215(1)              |                          |
| 4480  | $A_1$             | 167        | 2.9      | 5680.791321(2)             |                          |
| 4481  | $A_2$             | 167        | 2.9      | 5680.791343(2)             |                          |
| 4482  | $E$               | 165        | 2.9      | 5680.966640(2)             |                          |
| 4483  | $E$               | 94         | 2.9      | 5680.9667(1)               |                          |
| 4484  | $A_1$             | 103        | 1.9      | 5681.729290(4)             |                          |
| 4485  | $A_2$             | 84         | 1.9      | 5681.729294(4)             |                          |
| 4486  | $E$               | 95         | 3.1      | 5682.065921(1)             |                          |
| 4487  | $E$               | 77         | 3.1      | 5682.065923(6)             |                          |
| 4488  | $E$               | 77         | 2.2      | 5682.55154(8)              |                          |
| 4489  | $E$               | 76         | 2.2      | 5682.55154(8)              |                          |
| 4490  | $A_1$             | 79         | 2.2      | 5682.55669(6)              |                          |
| 4491  | $A_2$             | 75         | 2.2      | 5682.55894(8)              |                          |
| 4492  | $A_1$             | 93         | 3.2      | 5683.517623(1)             |                          |
| 4493  | $E$               | 113        | 1.9      | 5684.624662(1)             |                          |
| 4494  | $E$               | 93         | 1.9      | 5684.624663(3)             |                          |
| 4495  | $E$               | 158        | 3.0      | 5684.765145(2)             |                          |
| 4496  | $E$               | 145        | 3.0      | 5684.765145(3)             |                          |
| 4497  | $A_1$             | 105        | 3.0      | 5684.96932(2)              |                          |
| 4498  | $A_2$             | 100        | 2.9      | 5684.96977(2)              |                          |
| 4499  | $E$               | 100        | 2.7      | 5685.81470(2)              |                          |
| 4500  | $E$               | 138        | 2.7      | 5685.81471(3)              |                          |
| 4501  | $A_1$             | 135        | 2.6      | 5685.867631(1)             |                          |
| 4502  | $A_2$             | 99         | 2.6      | 5685.86769(1)              |                          |
| 4503  | $E$               | 93         | 1.4      | 5686.35006(2)              |                          |
| 4504  | $E$               | 97         | 1.4      | 5686.35006(1)              |                          |
| 4505  | $A_1$             | 79         | 2.1      | 5687.21118(1)              |                          |
| 4506  | $A_2$             | 78         | 2.1      | 5687.26511(1)              |                          |
| 4507  | $E$               | 121        | 0.68     | 5687.312803(1)             |                          |
| 4508  | $E$               | 92         | 0.69     | 5687.31281(3)              |                          |
| 4509  | $A_2^*$           | 83         | 2.6      | 5687.33390(3)              |                          |
| 4510  | $A_1^*$           | 83         | 2.6      | 5687.33391(3)              |                          |
| 4511  | $E$               | 93         | 2.5      | 5687.44195(1)              |                          |
| 4512  | $E$               | 142        | 2.5      | 5687.44195(2)              |                          |
| 4513  | $E$               | 136        | 2.2      | 5688.063233(2)             |                          |
| 4514  | $E$               | 138        | 2.2      | 5688.063235(3)             |                          |
| 4515  | $E$               | 123        | 2.1      | 5688.084340(2)             |                          |
| 4516  | $E$               | 124        | 2.1      | 5688.084340(2)             |                          |
| 4517  | $E$               | 107        | 3.1      | 5688.95105(2)              |                          |
| 4518  | $E$               | 128        | 3.1      | 5688.95105(2)              |                          |
| 4519  | $A_1$             | 118        | 3.2      | 5688.96837(1)              |                          |
| 4520  | $A_2$             | 119        | 3.1      | 5688.96920(1)              |                          |
| 4521  | $A_1$             | 60         | 0.53     | 5688.976125(1)             |                          |
| 4522  | $E$               | 121        | 2.2      | 5689.334599(2)             |                          |
| 4523  | $E$               | 131        | 2.2      | 5689.334602(4)             |                          |
| 4524  | $E$               | 97         | 2.7      | 5691.64347(1)              |                          |
| 4525  | $E$               | 115        | 2.7      | 5691.64347(2)              |                          |
| 4526  | $A_1$             | 79         | 2.6      | 5691.71970(3)              |                          |
| 4527  | $A_2$             | 81         | 2.6      | 5691.71984(3)              |                          |
| 4528  | $E$               | 123        | 2.5      | 5692.540604(4)             |                          |

Continued on next page.

TABLE S4 – states on Sarka/Poirier CSC PES; continued from previous page

| State | $\Gamma_{C_{3v}}$ | $D_{\max}$ | $S_{vN}$ | $\tilde{E}/\text{cm}^{-1}$ | $\Delta\text{Ref. [30]}$ |
|-------|-------------------|------------|----------|----------------------------|--------------------------|
| 4529  | $E$               | 137        | 2.5      | 5692.540606(4)             |                          |
| 4530  | $E$               | 99         | 2.4      | 5692.61113(1)              |                          |
| 4531  | $E$               | 98         | 2.4      | 5692.61113(1)              |                          |
| 4532  | $E$               | 87         | 0.74     | 5693.141740(9)             |                          |
| 4533  | $E$               | 88         | 0.76     | 5693.14174(1)              |                          |
| 4534  | $A_1$             | 145        | 2.7      | 5695.271815(2)             |                          |
| 4535  | $E$               | 95         | 2.6      | 5695.43621(1)              |                          |
| 4536  | $E$               | 141        | 2.6      | 5695.43621(1)              |                          |
| 4537  | $A_2$             | 91         | 2.6      | 5695.546078(1)             |                          |
| 4538  | $A_2$             | 127        | 0.57     | 5698.318757(4)             |                          |
| 4539  | $A_1$             | 157        | 0.57     | 5698.318762(4)             |                          |
| 4540  | $E$               | 106        | 2.1      | 5698.40971(1)              |                          |
| 4541  | $E$               | 104        | 2.1      | 5698.40971(1)              |                          |
| 4542  | $E$               | 114        | 3.1      | 5698.85183(2)              |                          |
| 4543  | $E$               | 168        | 3.1      | 5698.85183(2)              |                          |
| 4544  | $A_1^*$           | 90         | 3.0      | 5698.94386(1)              |                          |
| 4545  | $A_2^*$           | 89         | 3.1      | 5698.94386(1)              |                          |
| 4546  | $E$               | 109        | 2.1      | 5699.43607(1)              |                          |
| 4547  | $E$               | 110        | 2.1      | 5699.43607(1)              |                          |
| 4548  | $E$               | 106        | 2.2      | 5702.71672(2)              |                          |
| 4549  | $E$               | 106        | 2.2      | 5702.71672(2)              |                          |
| 4550  | $A_2$             | 160        | 3.3      | 5703.159504(3)             |                          |
| 4551  | $A_1$             | 116        | 3.2      | 5703.17011(1)              |                          |
| 4552  | $E$               | 146        | 3.1      | 5703.234245(6)             |                          |
| 4553  | $E$               | 113        | 3.1      | 5703.23425(3)              |                          |
| 4554  | $E$               | 145        | 2.8      | 5703.53725(1)              |                          |
| 4555  | $E$               | 166        | 2.8      | 5703.53726(1)              |                          |
| 4556  | $E$               | 112        | 2.3      | 5703.73007(2)              |                          |
| 4557  | $E$               | 111        | 2.3      | 5703.73008(1)              |                          |
| 4558  | $E$               | 132        | 2.4      | 5703.997463(7)             |                          |
| 4559  | $E$               | 161        | 2.4      | 5703.99748(1)              |                          |
| 4560  | $A_2$             | 109        | 2.3      | 5704.18502(1)              |                          |
| 4561  | $E$               | 107        | 2.3      | 5704.66676(1)              |                          |
| 4562  | $E$               | 110        | 2.3      | 5704.66676(1)              |                          |
| 4563  | $A_1$             | 142        | 2.2      | 5705.194054(2)             |                          |
| 4564  | $E$               | 135        | 0.89     | 5705.397685(6)             |                          |
| 4565  | $E$               | 183        | 0.89     | 5705.39770(1)              |                          |
| 4566  | $E$               | 119        | 0.53     | 5706.028547(8)             |                          |
| 4567  | $E$               | 153        | 0.53     | 5706.02855(1)              |                          |
| 4568  | $E$               | 138        | 1.5      | 5709.468420(7)             |                          |
| 4569  | $E$               | 140        | 1.6      | 5709.468422(3)             |                          |
| 4570  | $A_2$             | 99         | 2.9      | 5709.90611(5)              |                          |
| 4571  | $A_1$             | 98         | 2.9      | 5709.90611(6)              |                          |
| 4572  | $E$               | 113        | 2.8      | 5710.05286(1)              |                          |
| 4573  | $E$               | 141        | 2.8      | 5710.05287(2)              |                          |
| 4574  | $E$               | 151        | 3.1      | 5710.79705(1)              |                          |
| 4575  | $E$               | 146        | 3.1      | 5710.797055(9)             |                          |
| 4576  | $A_1$             | 139        | 0.86     | 5710.92860(1)              |                          |
| 4577  | $A_2$             | 122        | 2.4      | 5710.97950(9)              |                          |
| 4578  | $A_1$             | 127        | 2.4      | 5710.9795(1)               |                          |
| 4579  | $A_2$             | 107        | 1.2      | 5711.62009(2)              |                          |
| 4580  | $A_1$             | 117        | 1.3      | 5711.62011(3)              |                          |
| 4581  | $E$               | 160        | 2.7      | 5711.66700(2)              |                          |
| 4582  | $E$               | 168        | 2.8      | 5711.66700(3)              |                          |
| 4583  | $A_2$             | 200        | 2.7      | 5711.68311(1)              |                          |
| 4584  | $A_1$             | 169        | 2.7      | 5711.68314(1)              |                          |
| 4585  | $E$               | 110        | 2.2      | 5712.826943(7)             |                          |
| 4586  | $E$               | 102        | 2.2      | 5712.82695(1)              |                          |
| 4587  | $E$               | 106        | 2.2      | 5712.871886(7)             |                          |

Continued on next page.

TABLE S4 – states on Sarka/Poirier CSC PES; continued from previous page

| State | $\Gamma_{C_{3v}}$ | $D_{\max}$ | $S_{vN}$ | $\tilde{E}/\text{cm}^{-1}$ | $\Delta\text{Ref. [30]}$ |
|-------|-------------------|------------|----------|----------------------------|--------------------------|
| 4588  | $E$               | 107        | 2.2      | 5712.871886(8)             |                          |
| 4589  | $E$               | 159        | 2.1      | 5713.009194(3)             |                          |
| 4590  | $E$               | 124        | 2.1      | 5713.009202(9)             |                          |
| 4591  | $A_2^*$           | 111        | 2.6      | 5713.12949(4)              |                          |
| 4592  | $A_1^*$           | 117        | 2.6      | 5713.12949(5)              |                          |
| 4593  | $E$               | 173        | 0.85     | 5713.183929(7)             |                          |
| 4594  | $E$               | 172        | 0.86     | 5713.183931(7)             |                          |
| 4595  | $A_1$             | 89         | 2.1      | 5713.78072(5)              |                          |
| 4596  | $A_2$             | 106        | 2.1      | 5713.78108(2)              |                          |
| 4597  | $E$               | 93         | 2.1      | 5713.79349(3)              |                          |
| 4598  | $E$               | 89         | 2.1      | 5713.79349(3)              |                          |
| 4599  | $E$               | 108        | 3.0      | 5714.21039(6)              |                          |
| 4600  | $E$               | 110        | 3.0      | 5714.21040(7)              |                          |
| 4601  | $A_1$             | 100        | 2.9      | 5714.31459(8)              |                          |
| 4602  | $A_2$             | 97         | 2.9      | 5714.31476(7)              |                          |
| 4603  | $E$               | 130        | 0.88     | 5714.476971(7)             |                          |
| 4604  | $E$               | 160        | 0.88     | 5714.476972(6)             |                          |
| 4605  | $A_2$             | 145        | 2.5      | 5714.989743(2)             |                          |
| 4606  | $A_1$             | 189        | 2.7      | 5715.065681(5)             |                          |
| 4607  | $E$               | 151        | 2.5      | 5715.14403(1)              |                          |
| 4608  | $E$               | 146        | 2.5      | 5715.14403(1)              |                          |
| 4609  | $A_2$             | 112        | 2.4      | 5715.184377(2)             |                          |
| 4610  | $E$               | 103        | 0.18     | 5715.249210(2)             |                          |
| 4611  | $E$               | 75         | 0.18     | 5715.24922(1)              |                          |
| 4612  | $E$               | 107        | 1.1      | 5715.73072(2)              |                          |
| 4613  | $E$               | 100        | 1.1      | 5715.73072(2)              |                          |
| 4614  | $A_1^*$           | 136        | 2.4      | 5715.760087(5)             |                          |
| 4615  | $A_2^*$           | 116        | 2.4      | 5715.76009(2)              |                          |
| 4616  | $E$               | 152        | 2.4      | 5715.990384(9)             |                          |
| 4617  | $E$               | 156        | 2.4      | 5715.99039(1)              |                          |
| 4618  | $E$               | 98         | 2.4      | 5716.065483(1)             |                          |
| 4619  | $E$               | 110        | 2.4      | 5716.065484(1)             |                          |
| 4620  | $A_1$             | 120        | 2.4      | 5716.485627(2)             |                          |
| 4621  | $E$               | 130        | 0.54     | 5716.492014(7)             |                          |
| 4622  | $E$               | 139        | 0.55     | 5716.49202(1)              |                          |
| 4623  | $E$               | 175        | 3.6      | 5717.16781(1)              |                          |
| 4624  | $E$               | 200        | 3.6      | 5717.167810(6)             |                          |
| 4625  | $A_2$             | 187        | 3.7      | 5717.27830(1)              |                          |
| 4626  | $A_1$             | 195        | 3.7      | 5717.279098(9)             |                          |
| 4627  | $E$               | 191        | 3.5      | 5717.496003(6)             |                          |
| 4628  | $E$               | 200        | 3.5      | 5717.496010(9)             |                          |
| 4629  | $E$               | 195        | 3.6      | 5717.598746(4)             |                          |
| 4630  | $E$               | 207        | 3.6      | 5717.598753(9)             |                          |
| 4631  | $E$               | 145        | 2.3      | 5718.695395(2)             |                          |
| 4632  | $E$               | 147        | 2.3      | 5718.695397(3)             |                          |
| 4633  | $E$               | 176        | 2.6      | 5718.721840(5)             |                          |
| 4634  | $E$               | 191        | 2.6      | 5718.72185(1)              |                          |
| 4635  | $E$               | 110        | 2.4      | 5718.75559(3)              |                          |
| 4636  | $E$               | 137        | 2.4      | 5718.75559(3)              |                          |
| 4637  | $A_1$             | 140        | 2.5      | 5719.03799(3)              |                          |
| 4638  | $A_2$             | 168        | 2.5      | 5719.047266(9)             |                          |
| 4639  | $A_2$             | 113        | 2.3      | 5721.54805(2)              |                          |
| 4640  | $A_1$             | 99         | 2.3      | 5721.54935(2)              |                          |
| 4641  | $E$               | 112        | 2.3      | 5721.56847(1)              |                          |
| 4642  | $E$               | 98         | 2.3      | 5721.56847(2)              |                          |
| 4643  | $E$               | 116        | 2.2      | 5722.089386(1)             |                          |
| 4644  | $E$               | 105        | 2.2      | 5722.089387(3)             |                          |
| 4645  | $A_2$             | 161        | 2.6      | 5722.37040(3)              |                          |
| 4646  | $A_1$             | 147        | 2.6      | 5722.37042(2)              |                          |

Continued on next page.



TABLE S4 – states on Sarka/Poirier CSC PES; continued from previous page

| State | $\Gamma_{C_{3v}}$ | $D_{\max}$ | $S_{vN}$ | $\tilde{E}/\text{cm}^{-1}$ | $\Delta\text{Ref. [30]}$ |
|-------|-------------------|------------|----------|----------------------------|--------------------------|
| 4647  | $E$               | 118        | 2.1      | 5722.372641(1)             |                          |
| 4648  | $E$               | 118        | 2.1      | 5722.372641(1)             |                          |
| 4649  | $E$               | 170        | 0.5      | 5722.381072(3)             |                          |
| 4650  | $E$               | 165        | 0.5      | 5722.381072(3)             |                          |
| 4651  | $A_2$             | 86         | 3.0      | 5722.95701(1)              |                          |
| 4652  | $A_1$             | 89         | 3.0      | 5722.96795(1)              |                          |
| 4653  | $E$               | 119        | 2.4      | 5723.67065(1)              |                          |
| 4654  | $E$               | 104        | 2.4      | 5723.67065(2)              |                          |
| 4655  | $E$               | 94         | 3.7      | 5723.68430(1)              |                          |
| 4656  | $E$               | 90         | 3.7      | 5723.68430(3)              |                          |
| 4657  | $A_2$             | 198        | 2.5      | 5723.68431(2)              |                          |
| 4658  | $A_1$             | 192        | 2.5      | 5723.68431(3)              |                          |
| 4659  | $E$               | 216        | 3.6      | 5723.835823(5)             |                          |
| 4660  | $E$               | 199        | 3.6      | 5723.835829(9)             |                          |
| 4661  | $E$               | 180        | 2.7      | 5724.03809(1)              |                          |
| 4662  | $E$               | 165        | 2.7      | 5724.03810(1)              |                          |
| 4663  | $E$               | 127        | 2.0      | 5724.107532(1)             |                          |
| 4664  | $E$               | 132        | 2.0      | 5724.107532(3)             |                          |
| 4665  | $A_2$             | 145        | 2.4      | 5724.28209(1)              |                          |
| 4666  | $A_1$             | 129        | 2.4      | 5724.28210(7)              |                          |
| 4667  | $A_2$             | 139        | 2.7      | 5724.861610(3)             |                          |
| 4668  | $A_1$             | 147        | 2.5      | 5724.94976(3)              |                          |
| 4669  | $A_2$             | 135        | 2.5      | 5724.94976(1)              |                          |
| 4670  | $E$               | 129        | 2.7      | 5725.055472(4)             |                          |
| 4671  | $E$               | 126        | 2.7      | 5725.055473(5)             |                          |
| 4672  | $E$               | 218        | 2.7      | 5725.240179(5)             |                          |
| 4673  | $E$               | 220        | 2.7      | 5725.240179(5)             |                          |
| 4674  | $A_1$             | 123        | 2.7      | 5725.262666(5)             |                          |
| 4675  | $E$               | 163        | 2.5      | 5726.566640(6)             |                          |
| 4676  | $E$               | 175        | 2.5      | 5726.566644(7)             |                          |
| 4677  | $A_1$             | 159        | 3.5      | 5726.69466(4)              |                          |
| 4678  | $A_2$             | 144        | 3.5      | 5726.69559(6)              |                          |
| 4679  | $E$               | 191        | 3.3      | 5726.72055(1)              |                          |
| 4680  | $E$               | 167        | 3.3      | 5726.72055(3)              |                          |
| 4681  | $E$               | 167        | 2.0      | 5727.155366(3)             |                          |
| 4682  | $E$               | 137        | 2.0      | 5727.15537(1)              |                          |
| 4683  | $A_1$             | 132        | 3.6      | 5727.55601(5)              |                          |
| 4684  | $A_2$             | 127        | 3.6      | 5727.55601(4)              |                          |
| 4685  | $E$               | 169        | 2.4      | 5727.824365(5)             |                          |
| 4686  | $E$               | 170        | 2.4      | 5727.824366(6)             |                          |
| 4687  | $E$               | 156        | 2.3      | 5727.935035(7)             |                          |
| 4688  | $E$               | 184        | 2.3      | 5727.93504(1)              |                          |
| 4689  | $A_1$             | 126        | 2.4      | 5728.10408(3)              |                          |
| 4690  | $A_2$             | 141        | 2.4      | 5728.10411(2)              |                          |
| 4691  | $E$               | 144        | 2.6      | 5729.56299(1)              |                          |
| 4692  | $E$               | 199        | 2.6      | 5729.56301(2)              |                          |
| 4693  | $E$               | 201        | 2.4      | 5729.815291(6)             |                          |
| 4694  | $E$               | 166        | 2.4      | 5729.815299(8)             |                          |
| 4695  | $E$               | 123        | 0.94     | 5730.76499(1)              |                          |
| 4696  | $E$               | 129        | 0.94     | 5730.76499(1)              |                          |
| 4697  | $E$               | 96         | 2.6      | 5731.78630(5)              |                          |
| 4698  | $E$               | 135        | 2.6      | 5731.78632(5)              |                          |
| 4699  | $A_2^*$           | 98         | 2.6      | 5731.81419(3)              |                          |
| 4700  | $A_1^*$           | 98         | 2.6      | 5731.81419(3)              |                          |
| 4701  | $A_1$             | 146        | 2.6      | 5731.913369(5)             |                          |
| 4702  | $E$               | 150        | 2.4      | 5732.608398(4)             |                          |
| 4703  | $E$               | 192        | 2.4      | 5732.608405(8)             |                          |
| 4704  | $A_2$             | 159        | 2.4      | 5733.032070(3)             |                          |
| 4705  | $E$               | 142        | 2.7      | 5733.37362(1)              |                          |

Continued on next page.

TABLE S4 – states on Sarka/Poirier CSC PES; continued from previous page

| State | $\Gamma_{C_{3v}}$ | $D_{\max}$ | $S_{vN}$ | $\tilde{E}/\text{cm}^{-1}$ | $\Delta\text{Ref. [30]}$ |
|-------|-------------------|------------|----------|----------------------------|--------------------------|
| 4706  | $E$               | 141        | 2.7      | 5733.37362(1)              |                          |
| 4707  | $E$               | 140        | 2.5      | 5733.510380(1)             |                          |
| 4708  | $E$               | 141        | 2.5      | 5733.510382(2)             |                          |
| 4709  | $E$               | 207        | 3.4      | 5734.389934(5)             |                          |
| 4710  | $E$               | 178        | 3.4      | 5734.38994(1)              |                          |
| 4711  | $E$               | 162        | 3.1      | 5734.61398(2)              |                          |
| 4712  | $E$               | 207        | 3.1      | 5734.61399(2)              |                          |
| 4713  | $E$               | 210        | 3.1      | 5734.96193(2)              |                          |
| 4714  | $E$               | 162        | 3.1      | 5734.96193(2)              |                          |
| 4715  | $E$               | 205        | 4.0      | 5735.009451(5)             |                          |
| 4716  | $E$               | 215        | 3.9      | 5735.00947(1)              |                          |
| 4717  | $E$               | 172        | 3.1      | 5735.217681(6)             |                          |
| 4718  | $E$               | 192        | 3.1      | 5735.21768(1)              |                          |
| 4719  | $E$               | 152        | 2.0      | 5735.40516(2)              |                          |
| 4720  | $E$               | 156        | 2.0      | 5735.40517(2)              |                          |
| 4721  | $E$               | 66         | 0.14     | 5735.61545(1)              |                          |
| 4722  | $E$               | 100        | 0.14     | 5735.61546(1)              |                          |
| 4723  | $E$               | 114        | 2.6      | 5736.22642(4)              |                          |
| 4724  | $E$               | 109        | 2.6      | 5736.22642(4)              |                          |
| 4725  | $A_1$             | 128        | 2.7      | 5736.26853(5)              |                          |
| 4726  | $A_2$             | 100        | 2.6      | 5736.2796(1)               |                          |
| 4727  | $E$               | 102        | 2.1      | 5736.86120(2)              |                          |
| 4728  | $E$               | 104        | 2.1      | 5736.86121(3)              |                          |
| 4729  | $A_2^*$           | 98         | 2.1      | 5736.87064(4)              |                          |
| 4730  | $A_1^*$           | 97         | 2.1      | 5736.87065(4)              |                          |
| 4731  | $E$               | 168        | 2.7      | 5737.153537(2)             |                          |
| 4732  | $E$               | 168        | 2.7      | 5737.15355(1)              |                          |
| 4733  | $E$               | 137        | 2.7      | 5737.258240(6)             |                          |
| 4734  | $E$               | 170        | 2.7      | 5737.258242(8)             |                          |
| 4735  | $A_2$             | 182        | 2.9      | 5737.34687(1)              |                          |
| 4736  | $E$               | 207        | 3.3      | 5737.373606(6)             |                          |
| 4737  | $E$               | 195        | 3.3      | 5737.37361(1)              |                          |
| 4738  | $A_1$             | 182        | 3.2      | 5737.436533(8)             |                          |
| 4739  | $E$               | 84         | 0.25     | 5737.453917(1)             |                          |
| 4740  | $E$               | 84         | 0.25     | 5737.453918(2)             |                          |
| 4741  | $A_1$             | 133        | 3.1      | 5737.98082(6)              |                          |
| 4742  | $E$               | 147        | 3.1      | 5738.05218(5)              |                          |
| 4743  | $E$               | 144        | 3.1      | 5738.05218(5)              |                          |
| 4744  | $A_2$             | 140        | 2.8      | 5738.07349(4)              |                          |
| 4745  | $E$               | 109        | 0.52     | 5738.863319(4)             |                          |
| 4746  | $E$               | 109        | 0.52     | 5738.863324(6)             |                          |
| 4747  | $E$               | 116        | 1.9      | 5738.949099(1)             |                          |
| 4748  | $E$               | 94         | 1.9      | 5738.949100(4)             |                          |
| 4749  | $E$               | 110        | 1.9      | 5738.966186(2)             |                          |
| 4750  | $E$               | 110        | 1.9      | 5738.966187(3)             |                          |
| 4751  | $A_2$             | 103        | 2.8      | 5739.44791(1)              |                          |
| 4752  | $E$               | 97         | 2.8      | 5740.02112(1)              |                          |
| 4753  | $E$               | 97         | 2.8      | 5740.02112(2)              |                          |
| 4754  | $A_2$             | 123        | 2.7      | 5740.038932(2)             |                          |
| 4755  | $A_1$             | 107        | 2.8      | 5740.43719(1)              |                          |
| 4756  | $A_1$             | 147        | 2.0      | 5740.58639(1)              |                          |
| 4757  | $A_2$             | 126        | 2.0      | 5740.58994(6)              |                          |
| 4758  | $A_1$             | 125        | 1.9      | 5740.88437(3)              |                          |
| 4759  | $A_2$             | 135        | 1.9      | 5740.88461(3)              |                          |
| 4760  | $E$               | 124        | 2.7      | 5740.916286(2)             |                          |
| 4761  | $E$               | 123        | 2.7      | 5740.916286(2)             |                          |
| 4762  | $E$               | 168        | 2.2      | 5741.151537(2)             |                          |
| 4763  | $E$               | 137        | 2.2      | 5741.151538(8)             |                          |
| 4764  | $A_1$             | 107        | 2.2      | 5741.19380(3)              |                          |

Continued on next page.

TABLE S4 – states on Sarka/Poirier CSC PES; continued from previous page

| State | $\Gamma_{C_{3v}}$ | $D_{\max}$ | $S_{vN}$ | $\tilde{E}/\text{cm}^{-1}$ | $\Delta\text{Ref. [30]}$ |
|-------|-------------------|------------|----------|----------------------------|--------------------------|
| 4765  | $A_2$             | 101        | 2.2      | 5741.19395(4)              |                          |
| 4766  | $A_1$             | 124        | 2.7      | 5741.326366(3)             |                          |
| 4767  | $E$               | 104        | 0.37     | 5742.67078(1)              |                          |
| 4768  | $E$               | 105        | 0.39     | 5742.670787(7)             |                          |
| 4769  | $E$               | 140        | 0.98     | 5743.420886(3)             |                          |
| 4770  | $E$               | 150        | 0.97     | 5743.420889(4)             |                          |
| 4771  | $E$               | 148        | 0.94     | 5743.604419(2)             |                          |
| 4772  | $E$               | 150        | 1.0      | 5743.604420(3)             |                          |
| 4773  | $A_2$             | 62         | 0.52     | 5743.67663(3)              |                          |
| 4774  | $A_1$             | 61         | 0.52     | 5743.67664(3)              |                          |
| 4775  | $A_1$             | 82         | 0.65     | 5744.53059(1)              |                          |
| 4776  | $A_2$             | 75         | 0.65     | 5744.53061(1)              |                          |
| 4777  | $A_1$             | 64         | 0.22     | 5745.26042(3)              |                          |
| 4778  | $A_2$             | 60         | 0.22     | 5745.26043(4)              |                          |
| 4779  | $E$               | 87         | 0.53     | 5745.8950917(7)            |                          |
| 4780  | $E$               | 96         | 0.53     | 5745.895093(2)             |                          |
| 4781  | $A_2$             | 155        | 2.6      | 5747.076422(6)             |                          |
| 4782  | $E$               | 175        | 2.5      | 5747.197818(3)             |                          |
| 4783  | $E$               | 175        | 2.5      | 5747.197819(3)             |                          |
| 4784  | $A_1$             | 176        | 2.4      | 5747.325069(4)             |                          |
| 4785  | $E$               | 98         | 0.71     | 5747.364855(4)             |                          |
| 4786  | $E$               | 110        | 0.71     | 5747.364859(7)             |                          |
| 4787  | $E$               | 93         | 1.1      | 5750.494887(3)             |                          |
| 4788  | $E$               | 91         | 1.1      | 5750.494887(3)             |                          |
| 4789  | $E$               | 94         | 0.26     | 5752.1524040(9)            |                          |
| 4790  | $E$               | 114        | 0.26     | 5752.152406(3)             |                          |
| 4791  | $A_1$             | 167        | 3.4      | 5752.671048(3)             |                          |
| 4792  | $E$               | 124        | 3.1      | 5752.712222(8)             |                          |
| 4793  | $E$               | 161        | 3.1      | 5752.71224(2)              |                          |
| 4794  | $A_2$             | 127        | 3.4      | 5752.71933(1)              |                          |
| 4795  | $E$               | 91         | 0.72     | 5752.949887(3)             |                          |
| 4796  | $E$               | 88         | 0.72     | 5752.949891(4)             |                          |
| 4797  | $E$               | 138        | 2.7      | 5753.028785(9)             |                          |
| 4798  | $E$               | 139        | 2.7      | 5753.02879(1)              |                          |
| 4799  | $E$               | 111        | 2.8      | 5753.03939(2)              |                          |
| 4800  | $E$               | 146        | 2.8      | 5753.03940(1)              |                          |
| 4801  | $E$               | 100        | 0.71     | 5754.21257(5)              |                          |
| 4802  | $E$               | 100        | 0.71     | 5754.212567(3)             |                          |
| 4803  | $E$               | 97         | 1.3      | 5754.587856(1)             |                          |
| 4804  | $E$               | 97         | 1.3      | 5754.587859(3)             |                          |
| 4805  | $A_1$             | 87         | 1.4      | 5755.952518(3)             |                          |
| 4806  | $E$               | 102        | 2.4      | 5756.138147(5)             |                          |
| 4807  | $E$               | 89         | 2.4      | 5756.138149(9)             |                          |
| 4808  | $E$               | 122        | 2.4      | 5756.142764(6)             |                          |
| 4809  | $E$               | 103        | 2.4      | 5756.142765(8)             |                          |
| 4810  | $E$               | 89         | 0.29     | 5756.288702(3)             |                          |
| 4811  | $E$               | 89         | 0.29     | 5756.288705(5)             |                          |
| 4812  | $A_1$             | 108        | 0.52     | 5756.940008(1)             |                          |
| 4813  | $A_1$             | 86         | 0.29     | 5757.667650(5)             |                          |
| 4814  | $A_2$             | 120        | 2.5      | 5758.845733(4)             |                          |
| 4815  | $E$               | 102        | 2.5      | 5759.05741(1)              |                          |
| 4816  | $E$               | 95         | 2.5      | 5759.05741(1)              |                          |
| 4817  | $A_1$             | 102        | 2.5      | 5759.25697(1)              |                          |
| 4818  | $A_2$             | 120        | 2.7      | 5759.318026(3)             |                          |
| 4819  | $E$               | 111        | 2.7      | 5759.422754(6)             |                          |
| 4820  | $E$               | 120        | 2.7      | 5759.422755(3)             |                          |
| 4821  | $A_1$             | 122        | 2.7      | 5759.537817(3)             |                          |
| 4822  | $A_2$             | 64         | 0.82     | 5759.76011(7)              |                          |
| 4823  | $A_1$             | 67         | 0.83     | 5759.76024(6)              |                          |

Continued on next page.

TABLE S4 – states on Sarka/Poirier CSC PES; continued from previous page

| State | $\Gamma_{C_{3v}}$ | $D_{\max}$ | $S_{vN}$ | $\tilde{E}/\text{cm}^{-1}$ | $\Delta\text{Ref. [30]}$ |
|-------|-------------------|------------|----------|----------------------------|--------------------------|
| 4824  | $E$               | 78         | 2.0      | 5760.65366(2)              |                          |
| 4825  | $E$               | 75         | 2.0      | 5760.65367(3)              |                          |
| 4826  | $A_2$             | 73         | 2.0      | 5760.68851(3)              |                          |
| 4827  | $A_1$             | 75         | 2.0      | 5760.68851(3)              |                          |
| 4828  | $E$               | 96         | 0.86     | 5762.534134(2)             |                          |
| 4829  | $E$               | 89         | 0.86     | 5762.534137(4)             |                          |
| 4830  | $E$               | 107        | 0.092    | 5764.033465(3)             |                          |
| 4831  | $E$               | 106        | 0.091    | 5764.033466(2)             |                          |
| 4832  | $A_2^*$           | 90         | 2.1      | 5765.820488(1)             |                          |
| 4833  | $A_1^*$           | 104        | 2.1      | 5765.82050(8)              |                          |
| 4834  | $A_1^*$           | 66         | 1.0      | 5765.87445(5)              |                          |
| 4835  | $A_2^*$           | 67         | 1.0      | 5765.87445(5)              |                          |
| 4836  | $E$               | 113        | 3.0      | 5766.446572(4)             |                          |
| 4837  | $E$               | 113        | 3.0      | 5766.446575(4)             |                          |
| 4838  | $E$               | 110        | 3.1      | 5766.46971(5)              |                          |
| 4839  | $E$               | 113        | 3.1      | 5766.469711(6)             |                          |
| 4840  | $A_2$             | 97         | 2.1      | 5767.194582(3)             |                          |
| 4841  | $A_1$             | 98         | 2.1      | 5767.1946(1)               |                          |
| 4842  | $E$               | 88         | 2.3      | 5767.54038(1)              |                          |
| 4843  | $E$               | 82         | 2.3      | 5767.540384(9)             |                          |
| 4844  | $A_1$             | 83         | 2.3      | 5767.54529(1)              |                          |
| 4845  | $A_2$             | 87         | 2.3      | 5767.54533(1)              |                          |
| 4846  | $A_1$             | 106        | 1.0      | 5767.58095(4)              |                          |
| 4847  | $E$               | 89         | 0.75     | 5768.602073(1)             |                          |
| 4848  | $E$               | 108        | 0.75     | 5768.602076(4)             |                          |
| 4849  | $E$               | 142        | 2.1      | 5768.705171(1)             |                          |
| 4850  | $E$               | 112        | 2.1      | 5768.705176(7)             |                          |
| 4851  | $A_1^*$           | 83         | 2.1      | 5769.00760(6)              |                          |
| 4852  | $A_2^*$           | 82         | 2.1      | 5769.00760(7)              |                          |
| 4853  | $E$               | 117        | 0.48     | 5769.009897(5)             |                          |
| 4854  | $E$               | 103        | 0.5      | 5769.00993(4)              |                          |
| 4855  | $E$               | 81         | 2.1      | 5769.03260(6)              |                          |
| 4856  | $E$               | 85         | 2.1      | 5769.03260(4)              |                          |
| 4857  | $A_1$             | 101        | 3.1      | 5769.37525(1)              |                          |
| 4858  | $A_2$             | 101        | 3.1      | 5769.37716(1)              |                          |
| 4859  | $E$               | 109        | 2.8      | 5769.38362(1)              |                          |
| 4860  | $E$               | 103        | 2.8      | 5769.38364(1)              |                          |
| 4861  | $E$               | 148        | 2.4      | 5770.0980(1)               |                          |
| 4862  | $E$               | 150        | 2.4      | 5770.097957(6)             |                          |
| 4863  | $E$               | 133        | 2.1      | 5770.138606(2)             |                          |
| 4864  | $E$               | 101        | 2.1      | 5770.13861(1)              |                          |
| 4865  | $A_1^*$           | 133        | 3.4      | 5770.89223(4)              |                          |
| 4866  | $A_2^*$           | 130        | 3.4      | 5770.89224(4)              |                          |
| 4867  | $E$               | 155        | 3.2      | 5771.06348(1)              |                          |
| 4868  | $E$               | 155        | 3.2      | 5771.063486(9)             |                          |
| 4869  | $E$               | 146        | 2.3      | 5771.3953(1)               |                          |
| 4870  | $E$               | 143        | 2.3      | 5771.3953(1)               |                          |
| 4871  | $E$               | 118        | 1.6      | 5773.002501(1)             |                          |
| 4872  | $E$               | 116        | 1.6      | 5773.00250(4)              |                          |
| 4873  | $E$               | 110        | 2.1      | 5774.580380(8)             |                          |
| 4874  | $E$               | 79         | 2.1      | 5774.58039(1)              |                          |
| 4875  | $E$               | 77         | 2.1      | 5774.59540(2)              |                          |
| 4876  | $E$               | 96         | 2.1      | 5774.59541(1)              |                          |
| 4877  | $E$               | 113        | 2.3      | 5774.94915(1)              |                          |
| 4878  | $E$               | 109        | 2.3      | 5774.94915(1)              |                          |
| 4879  | $A_1$             | 131        | 2.6      | 5775.11821(5)              |                          |
| 4880  | $E$               | 106        | 2.2      | 5775.27221(1)              |                          |
| 4881  | $E$               | 106        | 2.2      | 5775.27221(1)              |                          |
| 4882  | $E$               | 127        | 3.0      | 5775.30106(7)              |                          |

Continued on next page.

TABLE S4 – states on Sarka/Poirier CSC PES; continued from previous page

| State | $\Gamma_{C_{3v}}$ | $D_{\max}$ | $S_{vN}$ | $\tilde{E}/\text{cm}^{-1}$ | $\Delta\text{Ref. [30]}$ |
|-------|-------------------|------------|----------|----------------------------|--------------------------|
| 4883  | $E$               | 118        | 3.0      | 5775.3011(1)               |                          |
| 4884  | $A_2$             | 127        | 2.2      | 5775.30238(3)              |                          |
| 4885  | $A_1$             | 122        | 2.5      | 5775.79323(9)              |                          |
| 4886  | $A_2$             | 130        | 2.5      | 5775.79325(3)              |                          |
| 4887  | $E$               | 102        | 1.2      | 5776.221443(3)             |                          |
| 4888  | $E$               | 103        | 1.2      | 5776.221443(4)             |                          |
| 4889  | $E$               | 162        | 3.5      | 5776.5703(3)               |                          |
| 4890  | $E$               | 177        | 3.5      | 5776.57036(3)              |                          |
| 4891  | $E$               | 203        | 3.3      | 5776.740430(6)             |                          |
| 4892  | $E$               | 170        | 3.3      | 5776.74043(1)              |                          |
| 4893  | $E$               | 92         | 1.1      | 5776.865004(3)             |                          |
| 4894  | $E$               | 101        | 1.1      | 5776.865007(5)             |                          |
| 4895  | $A_1$             | 125        | 2.3      | 5777.084045(5)             |                          |
| 4896  | $A_2$             | 137        | 2.3      | 5777.08406(1)              |                          |
| 4897  | $A_1$             | 119        | 2.2      | 5777.365534(9)             |                          |
| 4898  | $E$               | 74         | 2.2      | 5777.36989(3)              |                          |
| 4899  | $E$               | 78         | 2.2      | 5777.36991(3)              |                          |
| 4900  | $A_2$             | 72         | 2.2      | 5777.38425(5)              |                          |
| 4901  | $E$               | 165        | 2.5      | 5778.57329(1)              |                          |
| 4902  | $E$               | 173        | 2.5      | 5778.57329(1)              |                          |
| 4903  | $A_1$             | 126        | 3.4      | 5779.57875(8)              |                          |
| 4904  | $A_2$             | 125        | 3.3      | 5779.58237(4)              |                          |
| 4905  | $E$               | 150        | 2.8      | 5779.6573(1)               |                          |
| 4906  | $E$               | 156        | 2.8      | 5779.657335(8)             |                          |
| 4907  | $E$               | 152        | 2.4      | 5779.9398(1)               |                          |
| 4908  | $E$               | 146        | 2.4      | 5779.93982(1)              |                          |
| 4909  | $E$               | 110        | 2.6      | 5780.97232(1)              |                          |
| 4910  | $E$               | 105        | 2.6      | 5780.97232(1)              |                          |
| 4911  | $E$               | 101        | 2.6      | 5780.97644(1)              |                          |
| 4912  | $E$               | 131        | 2.6      | 5780.97645(1)              |                          |
| 4913  | $A_2^*$           | 82         | 1.2      | 5782.37590(2)              |                          |
| 4914  | $A_1^*$           | 86         | 1.2      | 5782.37592(2)              |                          |
| 4915  | $A_2$             | 117        | 2.7      | 5783.67004(1)              |                          |
| 4916  | $E$               | 105        | 2.7      | 5783.8826(2)               |                          |
| 4917  | $E$               | 113        | 2.7      | 5783.882563(4)             |                          |
| 4918  | $E$               | 101        | 1.4      | 5783.985999(5)             |                          |
| 4919  | $E$               | 122        | 1.4      | 5783.986000(4)             |                          |
| 4920  | $A_1$             | 105        | 2.7      | 5784.0835(2)               |                          |
| 4921  | $A_1$             | 138        | 2.9      | 5784.82716(2)              |                          |
| 4922  | $E$               | 160        | 2.8      | 5784.978713(6)             |                          |
| 4923  | $E$               | 160        | 2.8      | 5784.97872(7)              |                          |
| 4924  | $A_2$             | 180        | 2.8      | 5785.06397(2)              |                          |
| 4925  | $E$               | 122        | 1.3      | 5785.132282(1)             |                          |
| 4926  | $E$               | 98         | 1.3      | 5785.132287(5)             |                          |
| 4927  | $A_1$             | 93         | 2.4      | 5785.87657(8)              |                          |
| 4928  | $A_2$             | 96         | 2.4      | 5785.87658(7)              |                          |
| 4929  | $E$               | 123        | 0.68     | 5786.10787(7)              |                          |
| 4930  | $E$               | 131        | 0.7      | 5786.107872(3)             |                          |
| 4931  | $E$               | 107        | 2.3      | 5786.14101(2)              |                          |
| 4932  | $E$               | 109        | 2.3      | 5786.14102(2)              |                          |
| 4933  | $E$               | 116        | 0.65     | 5786.28367(6)              |                          |
| 4934  | $E$               | 115        | 0.63     | 5786.28367(5)              |                          |
| 4935  | $E$               | 102        | 2.1      | 5786.563898(1)             |                          |
| 4936  | $E$               | 88         | 2.1      | 5786.563901(3)             |                          |
| 4937  | $A_1$             | 125        | 0.85     | 5787.68545(4)              |                          |
| 4938  | $A_1$             | 84         | 2.1      | 5788.03742(2)              |                          |
| 4939  | $E$               | 161        | 2.5      | 5788.052625(3)             |                          |
| 4940  | $E$               | 157        | 2.5      | 5788.052627(3)             |                          |
| 4941  | $E$               | 156        | 2.5      | 5788.062203(4)             |                          |

Continued on next page.

TABLE S4 – states on Sarka/Poirier CSC PES; continued from previous page

| State | $\Gamma_{C_{3v}}$ | $D_{\max}$ | $S_{vN}$ | $\tilde{E}/\text{cm}^{-1}$ | $\Delta\text{Ref. [30]}$ |
|-------|-------------------|------------|----------|----------------------------|--------------------------|
| 4942  | $E$               | 161        | 2.5      | 5788.062206(3)             |                          |
| 4943  | $A_1$             | 113        | 0.65     | 5788.707723(4)             |                          |
| 4944  | $A_1$             | 100        | 1.4      | 5789.164332(3)             |                          |
| 4945  | $A_2$             | 93         | 1.4      | 5789.164526(4)             |                          |
| 4946  | $E$               | 81         | 0.33     | 5791.2289969(5)            |                          |
| 4947  | $E$               | 80         | 0.33     | 5791.229000(7)             |                          |
| 4948  | $E$               | 103        | 2.4      | 5791.641447(7)             |                          |
| 4949  | $E$               | 112        | 2.4      | 5791.64145(1)              |                          |
| 4950  | $E$               | 99         | 1.5      | 5791.75425(2)              |                          |
| 4951  | $E$               | 106        | 1.5      | 5791.754255(4)             |                          |
| 4952  | $A_2^*$           | 93         | 2.3      | 5791.87769(2)              |                          |
| 4953  | $A_1^*$           | 86         | 2.3      | 5791.87770(2)              |                          |
| 4954  | $E$               | 170        | 3.3      | 5792.092174(5)             |                          |
| 4955  | $E$               | 169        | 3.3      | 5792.092174(4)             |                          |
| 4956  | $A_2$             | 184        | 3.3      | 5792.116453(4)             |                          |
| 4957  | $A_1$             | 179        | 3.4      | 5792.183137(4)             |                          |
| 4958  | $E$               | 175        | 2.6      | 5792.480383(3)             |                          |
| 4959  | $E$               | 168        | 2.6      | 5792.480383(3)             |                          |
| 4960  | $E$               | 154        | 2.6      | 5792.499865(7)             |                          |
| 4961  | $E$               | 162        | 2.6      | 5792.49987(5)              |                          |
| 4962  | $E$               | 120        | 0.73     | 5793.17350(3)              |                          |
| 4963  | $E$               | 120        | 0.73     | 5793.17350(3)              |                          |
| 4964  | $E$               | 181        | 3.6      | 5793.376495(5)             |                          |
| 4965  | $E$               | 191        | 3.6      | 5793.376501(8)             |                          |
| 4966  | $A_2$             | 143        | 3.7      | 5793.66684(3)              |                          |
| 4967  | $A_1$             | 158        | 3.7      | 5793.66685(4)              |                          |
| 4968  | $E$               | 176        | 3.3      | 5793.760687(6)             |                          |
| 4969  | $E$               | 172        | 3.3      | 5793.760689(6)             |                          |
| 4970  | $A_2^*$           | 133        | 3.1      | 5794.04363(2)              |                          |
| 4971  | $A_1^*$           | 134        | 3.1      | 5794.04364(2)              |                          |
| 4972  | $E$               | 109        | 2.4      | 5794.07886(3)              |                          |
| 4973  | $E$               | 111        | 2.4      | 5794.07887(3)              |                          |
| 4974  | $A_1^*$           | 109        | 2.4      | 5794.29028(3)              |                          |
| 4975  | $A_2^*$           | 112        | 2.4      | 5794.29028(3)              |                          |
| 4976  | $E$               | 205        | 2.7      | 5795.09984(1)              |                          |
| 4977  | $E$               | 187        | 2.7      | 5795.0999(2)               |                          |
| 4978  | $A_2$             | 160        | 2.9      | 5795.10295(4)              |                          |
| 4979  | $A_1$             | 154        | 2.9      | 5795.10295(4)              |                          |
| 4980  | $E$               | 172        | 1.1      | 5796.349740(3)             |                          |
| 4981  | $E$               | 183        | 1.1      | 5796.349743(5)             |                          |
| 4982  | $E$               | 62         | 2.1      | 5796.825906(6)             |                          |
| 4983  | $E$               | 91         | 2.1      | 5796.82591(1)              |                          |
| 4984  | $E$               | 160        | 2.3      | 5797.766492(7)             |                          |
| 4985  | $E$               | 135        | 2.3      | 5797.7665(1)               |                          |
| 4986  | $A_1$             | 184        | 1.2      | 5797.78858(6)              |                          |
| 4987  | $E$               | 143        | 0.29     | 5797.866105(2)             |                          |
| 4988  | $E$               | 113        | 0.29     | 5797.86611(1)              |                          |
| 4989  | $A_1$             | 68         | 2.1      | 5798.295404(9)             |                          |
| 4990  | $E$               | 156        | 3.3      | 5798.59488(1)              |                          |
| 4991  | $E$               | 158        | 3.3      | 5798.59488(2)              |                          |
| 4992  | $A_2$             | 143        | 3.2      | 5798.6987(1)               |                          |
| 4993  | $A_1$             | 156        | 3.2      | 5798.698758(4)             |                          |
| 4994  | $E$               | 141        | 2.8      | 5799.0795(1)               |                          |
| 4995  | $E$               | 175        | 2.8      | 5799.07953(1)              |                          |
| 4996  | $E$               | 206        | 3.6      | 5799.08186(1)              |                          |
| 4997  | $E$               | 204        | 3.6      | 5799.081863(5)             |                          |
| 4998  | $A_1$             | 205        | 2.9      | 5799.261459(4)             |                          |
| 4999  | $A_2$             | 206        | 2.9      | 5799.26194(1)              |                          |
